# Supplementary material for: ZipIR: Latent Pyramid Diffusion Transformer for High-Resolution Image Restoration
Source: arXiv:2504.08591 source file (2025-04-11)

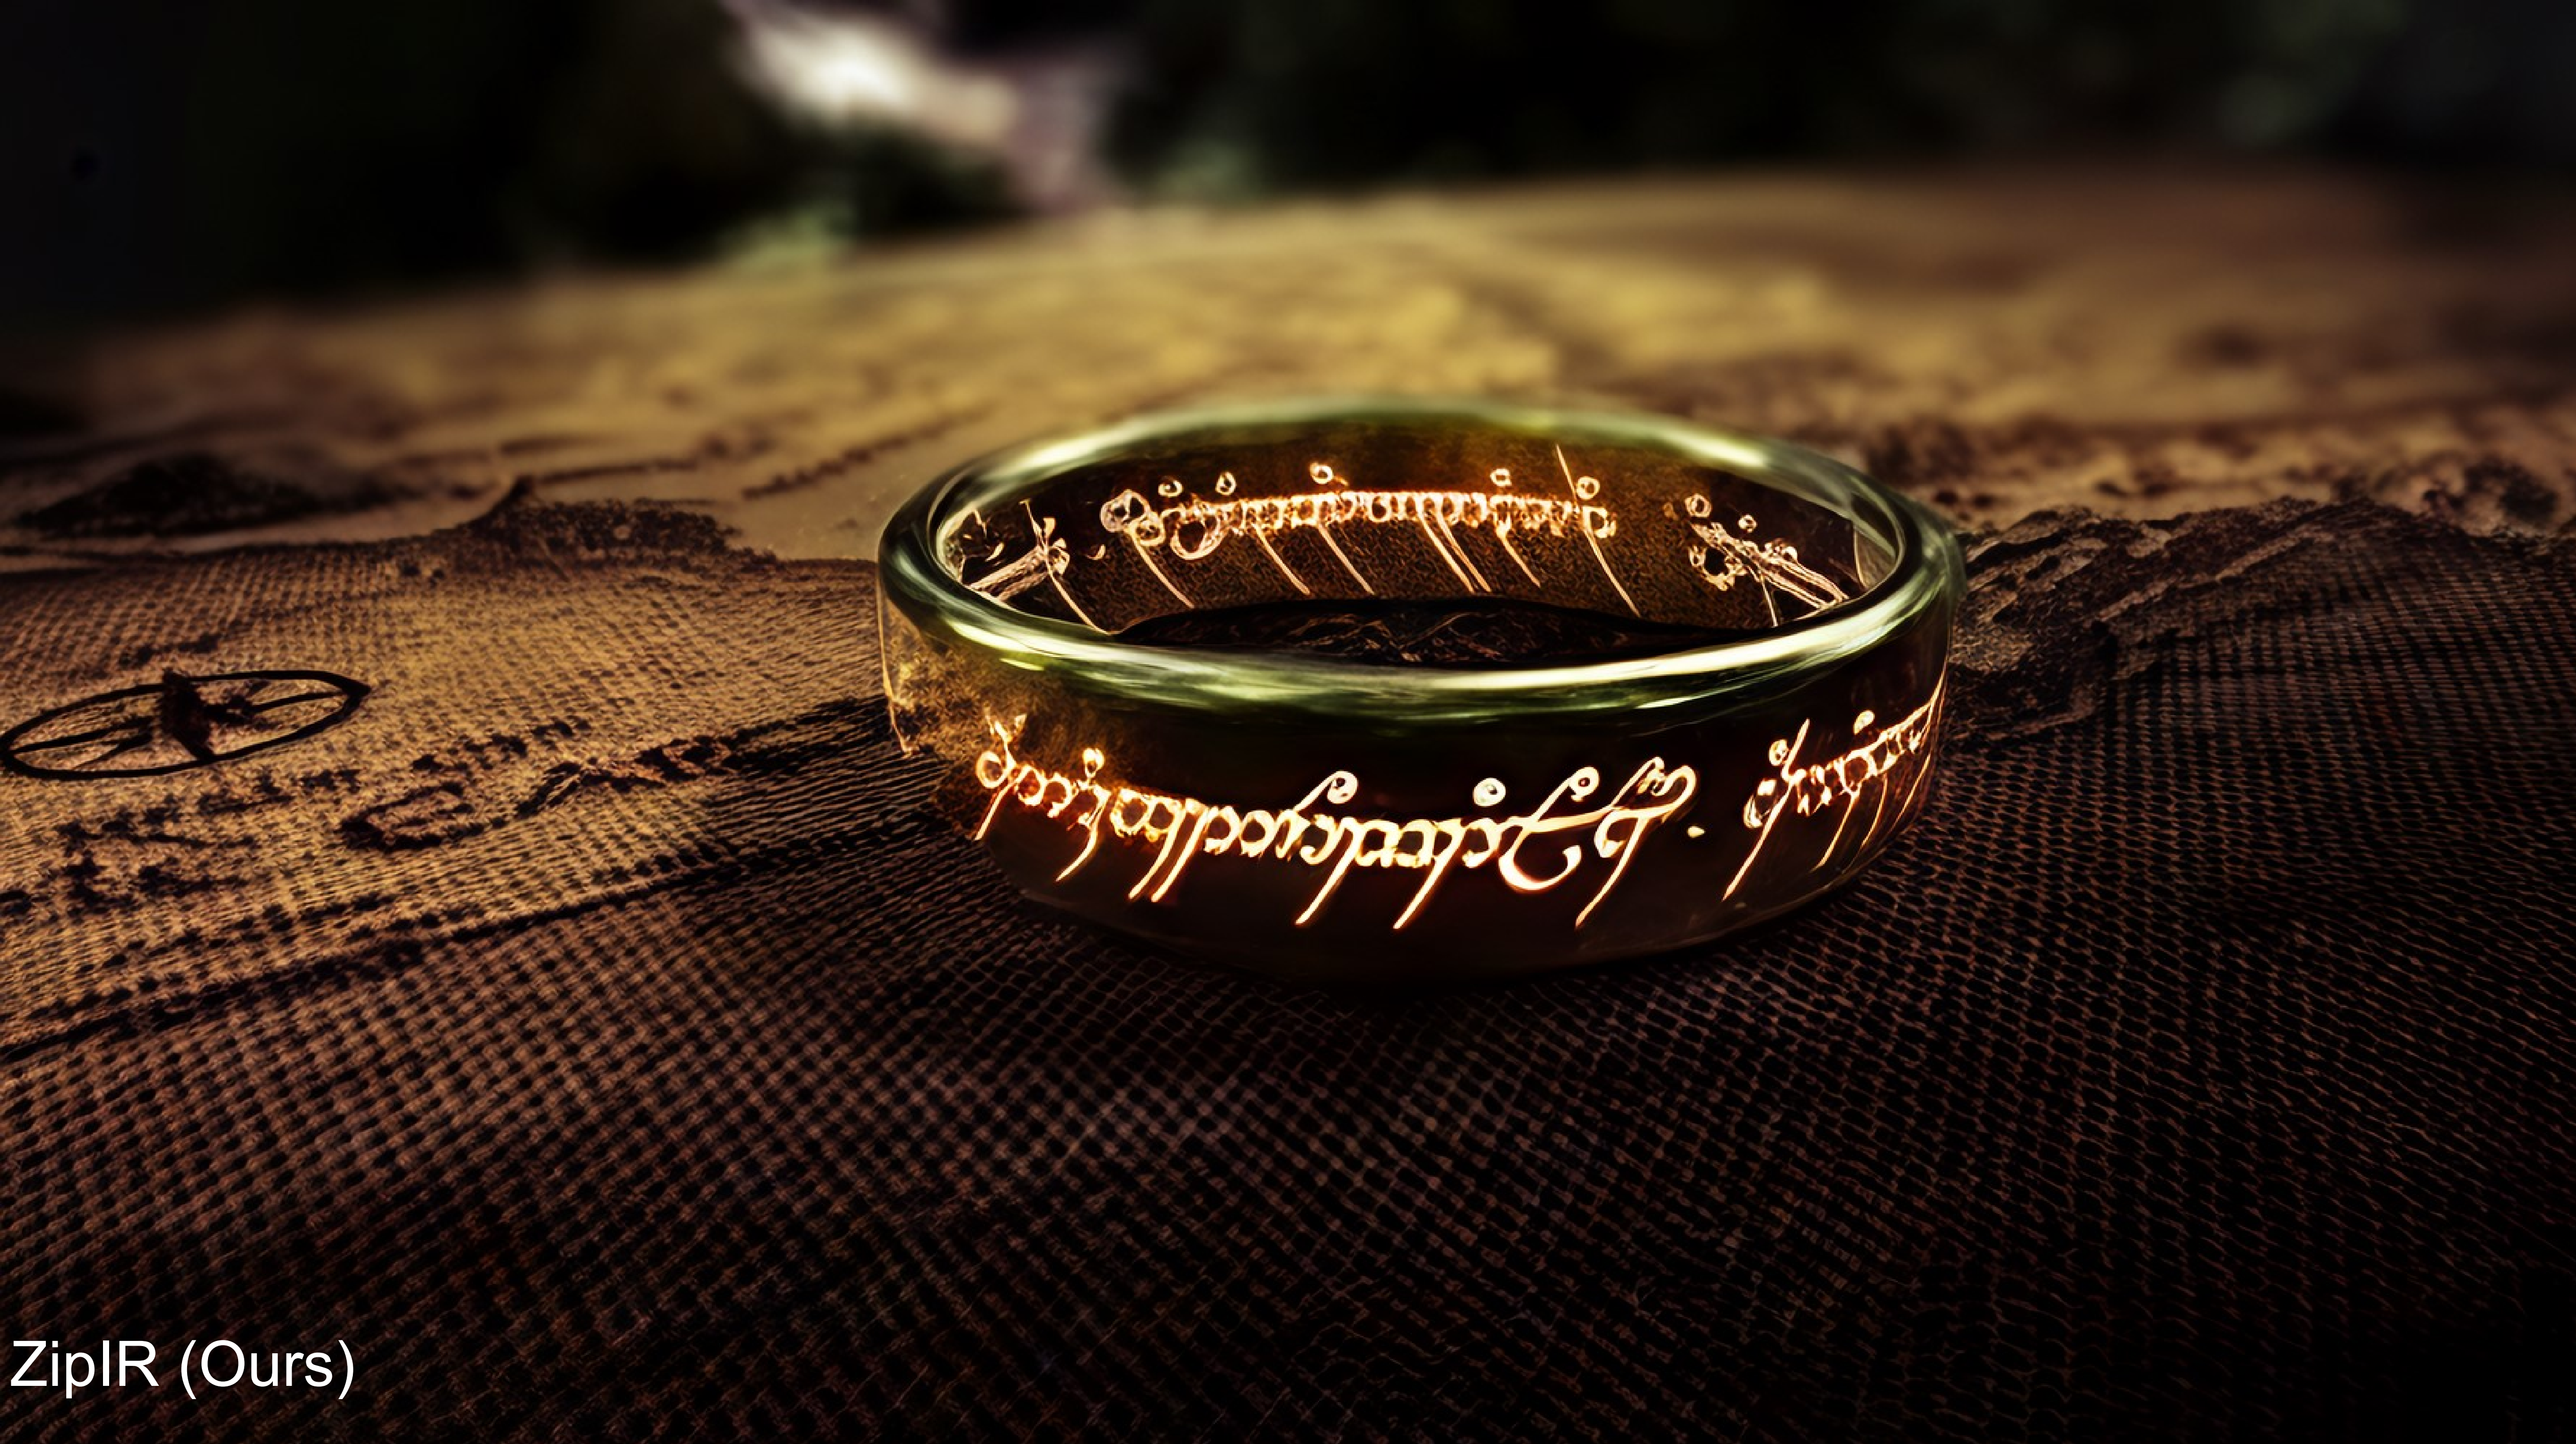

ZipIR (Ours)

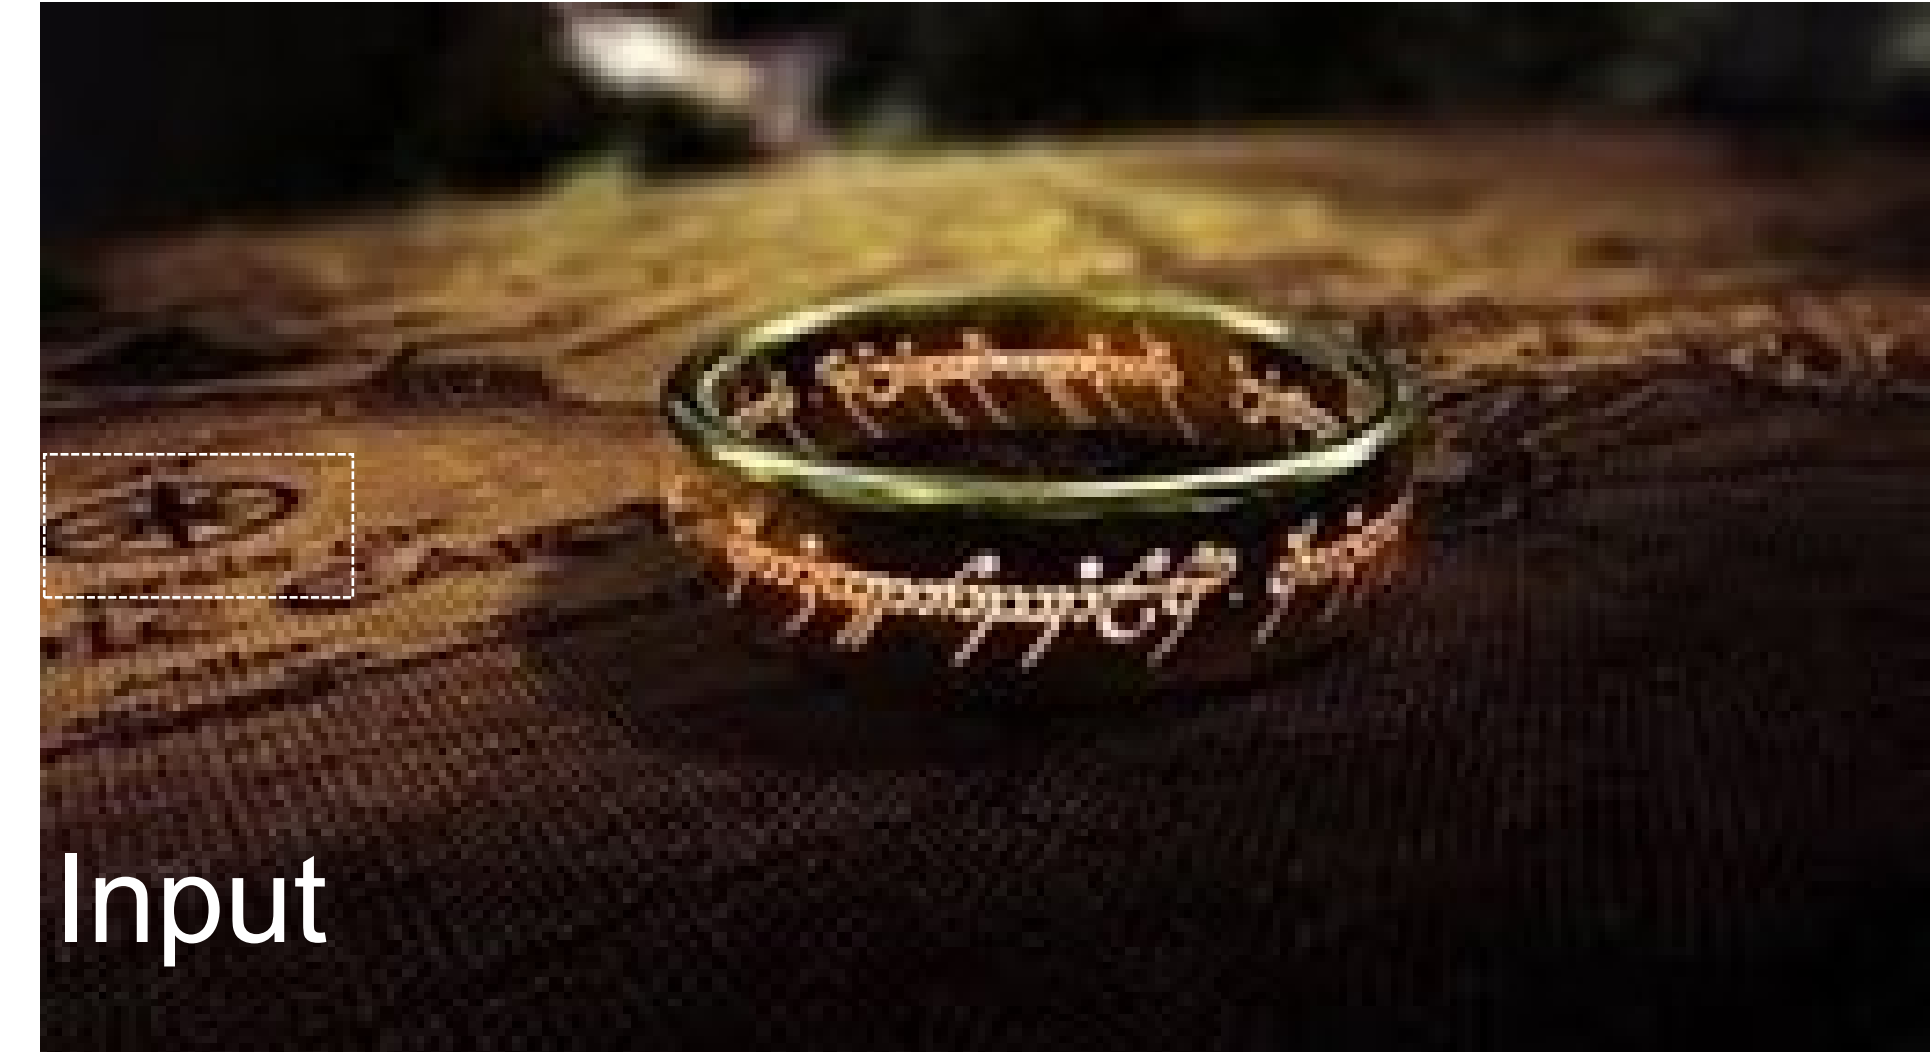

Input

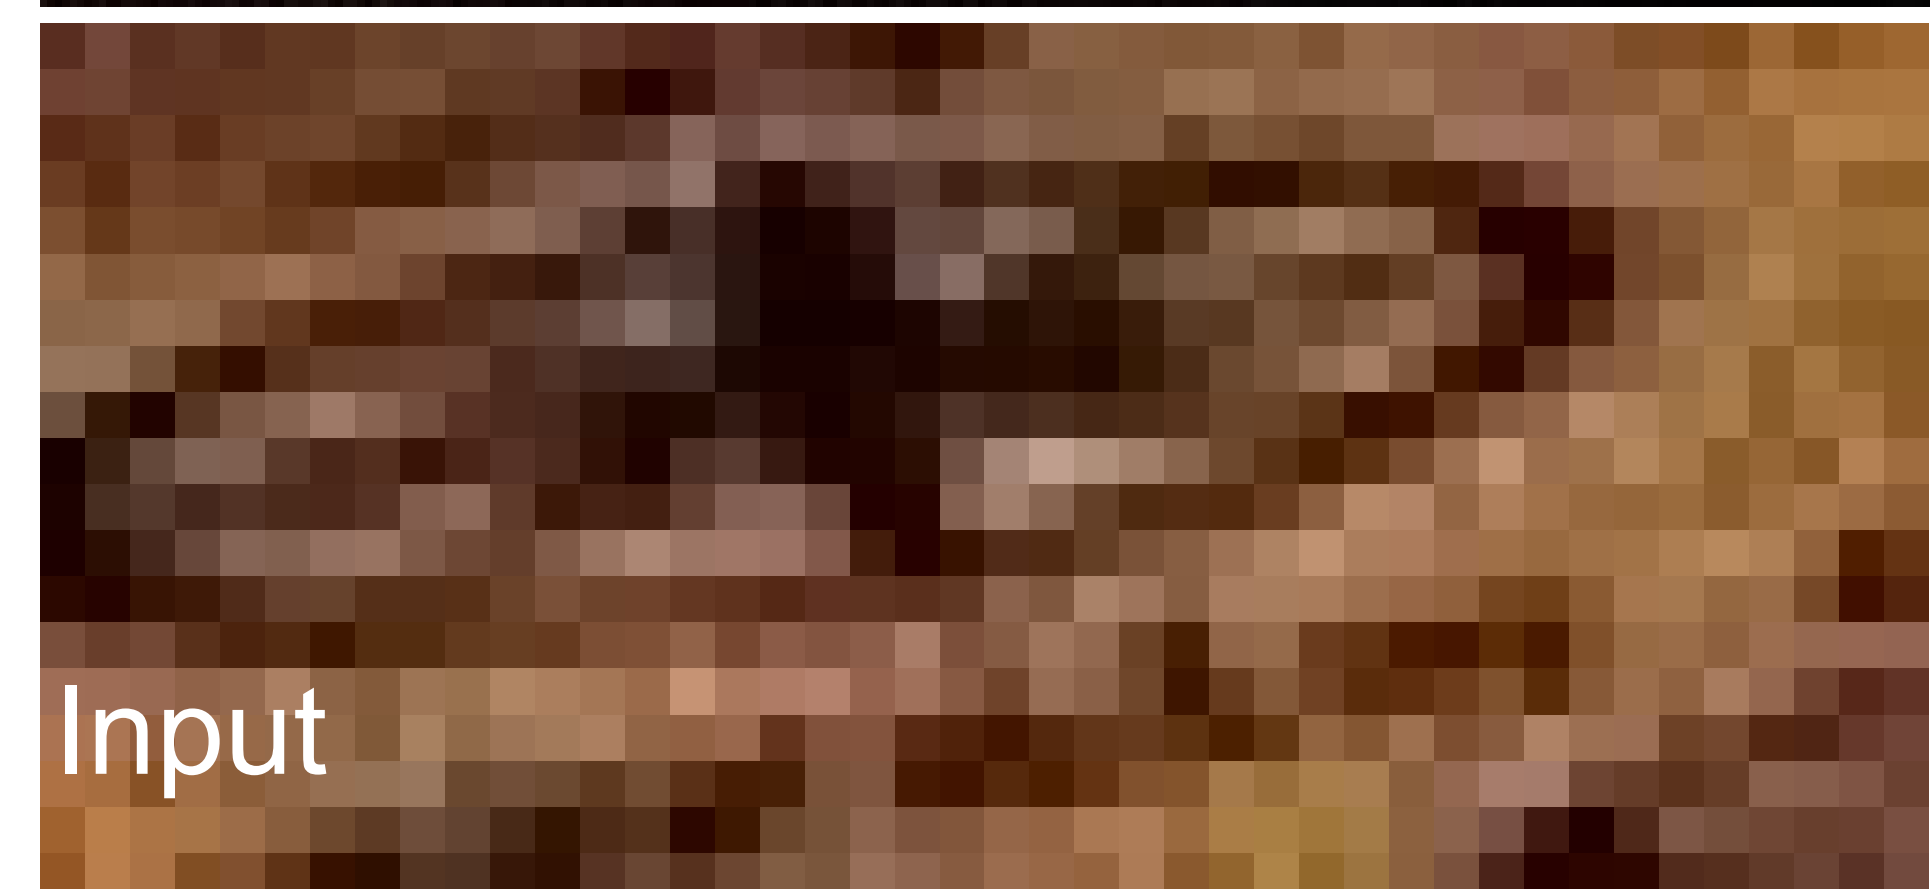

Input

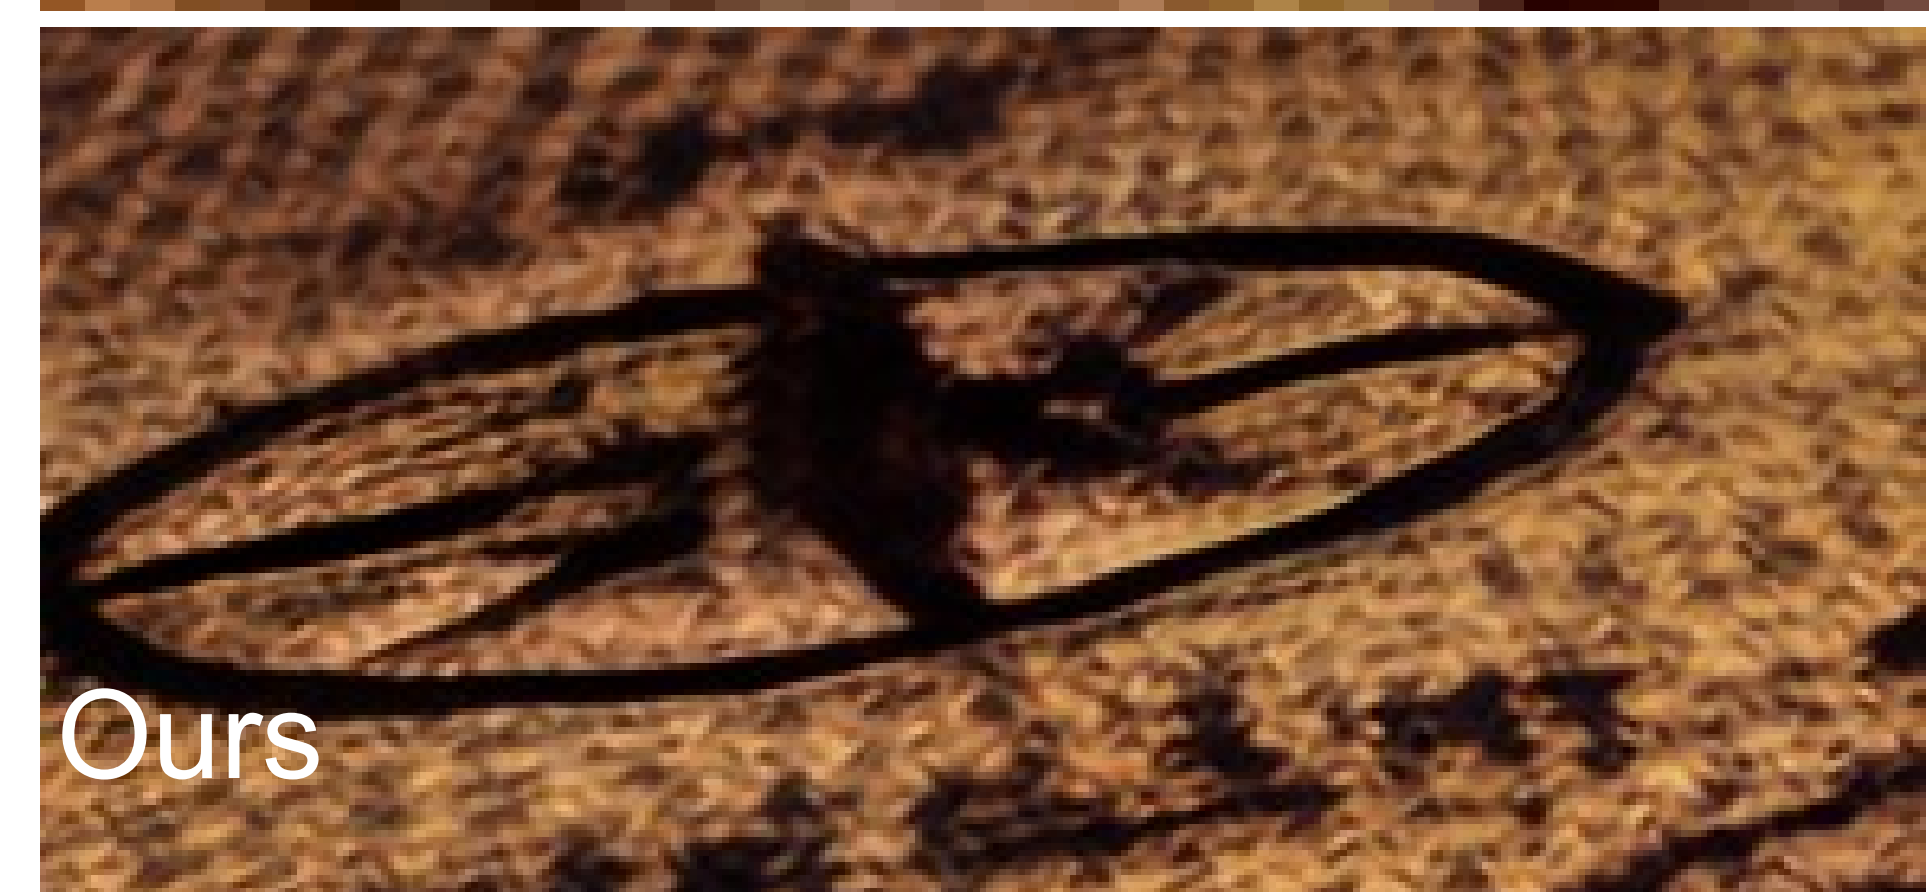

Ours

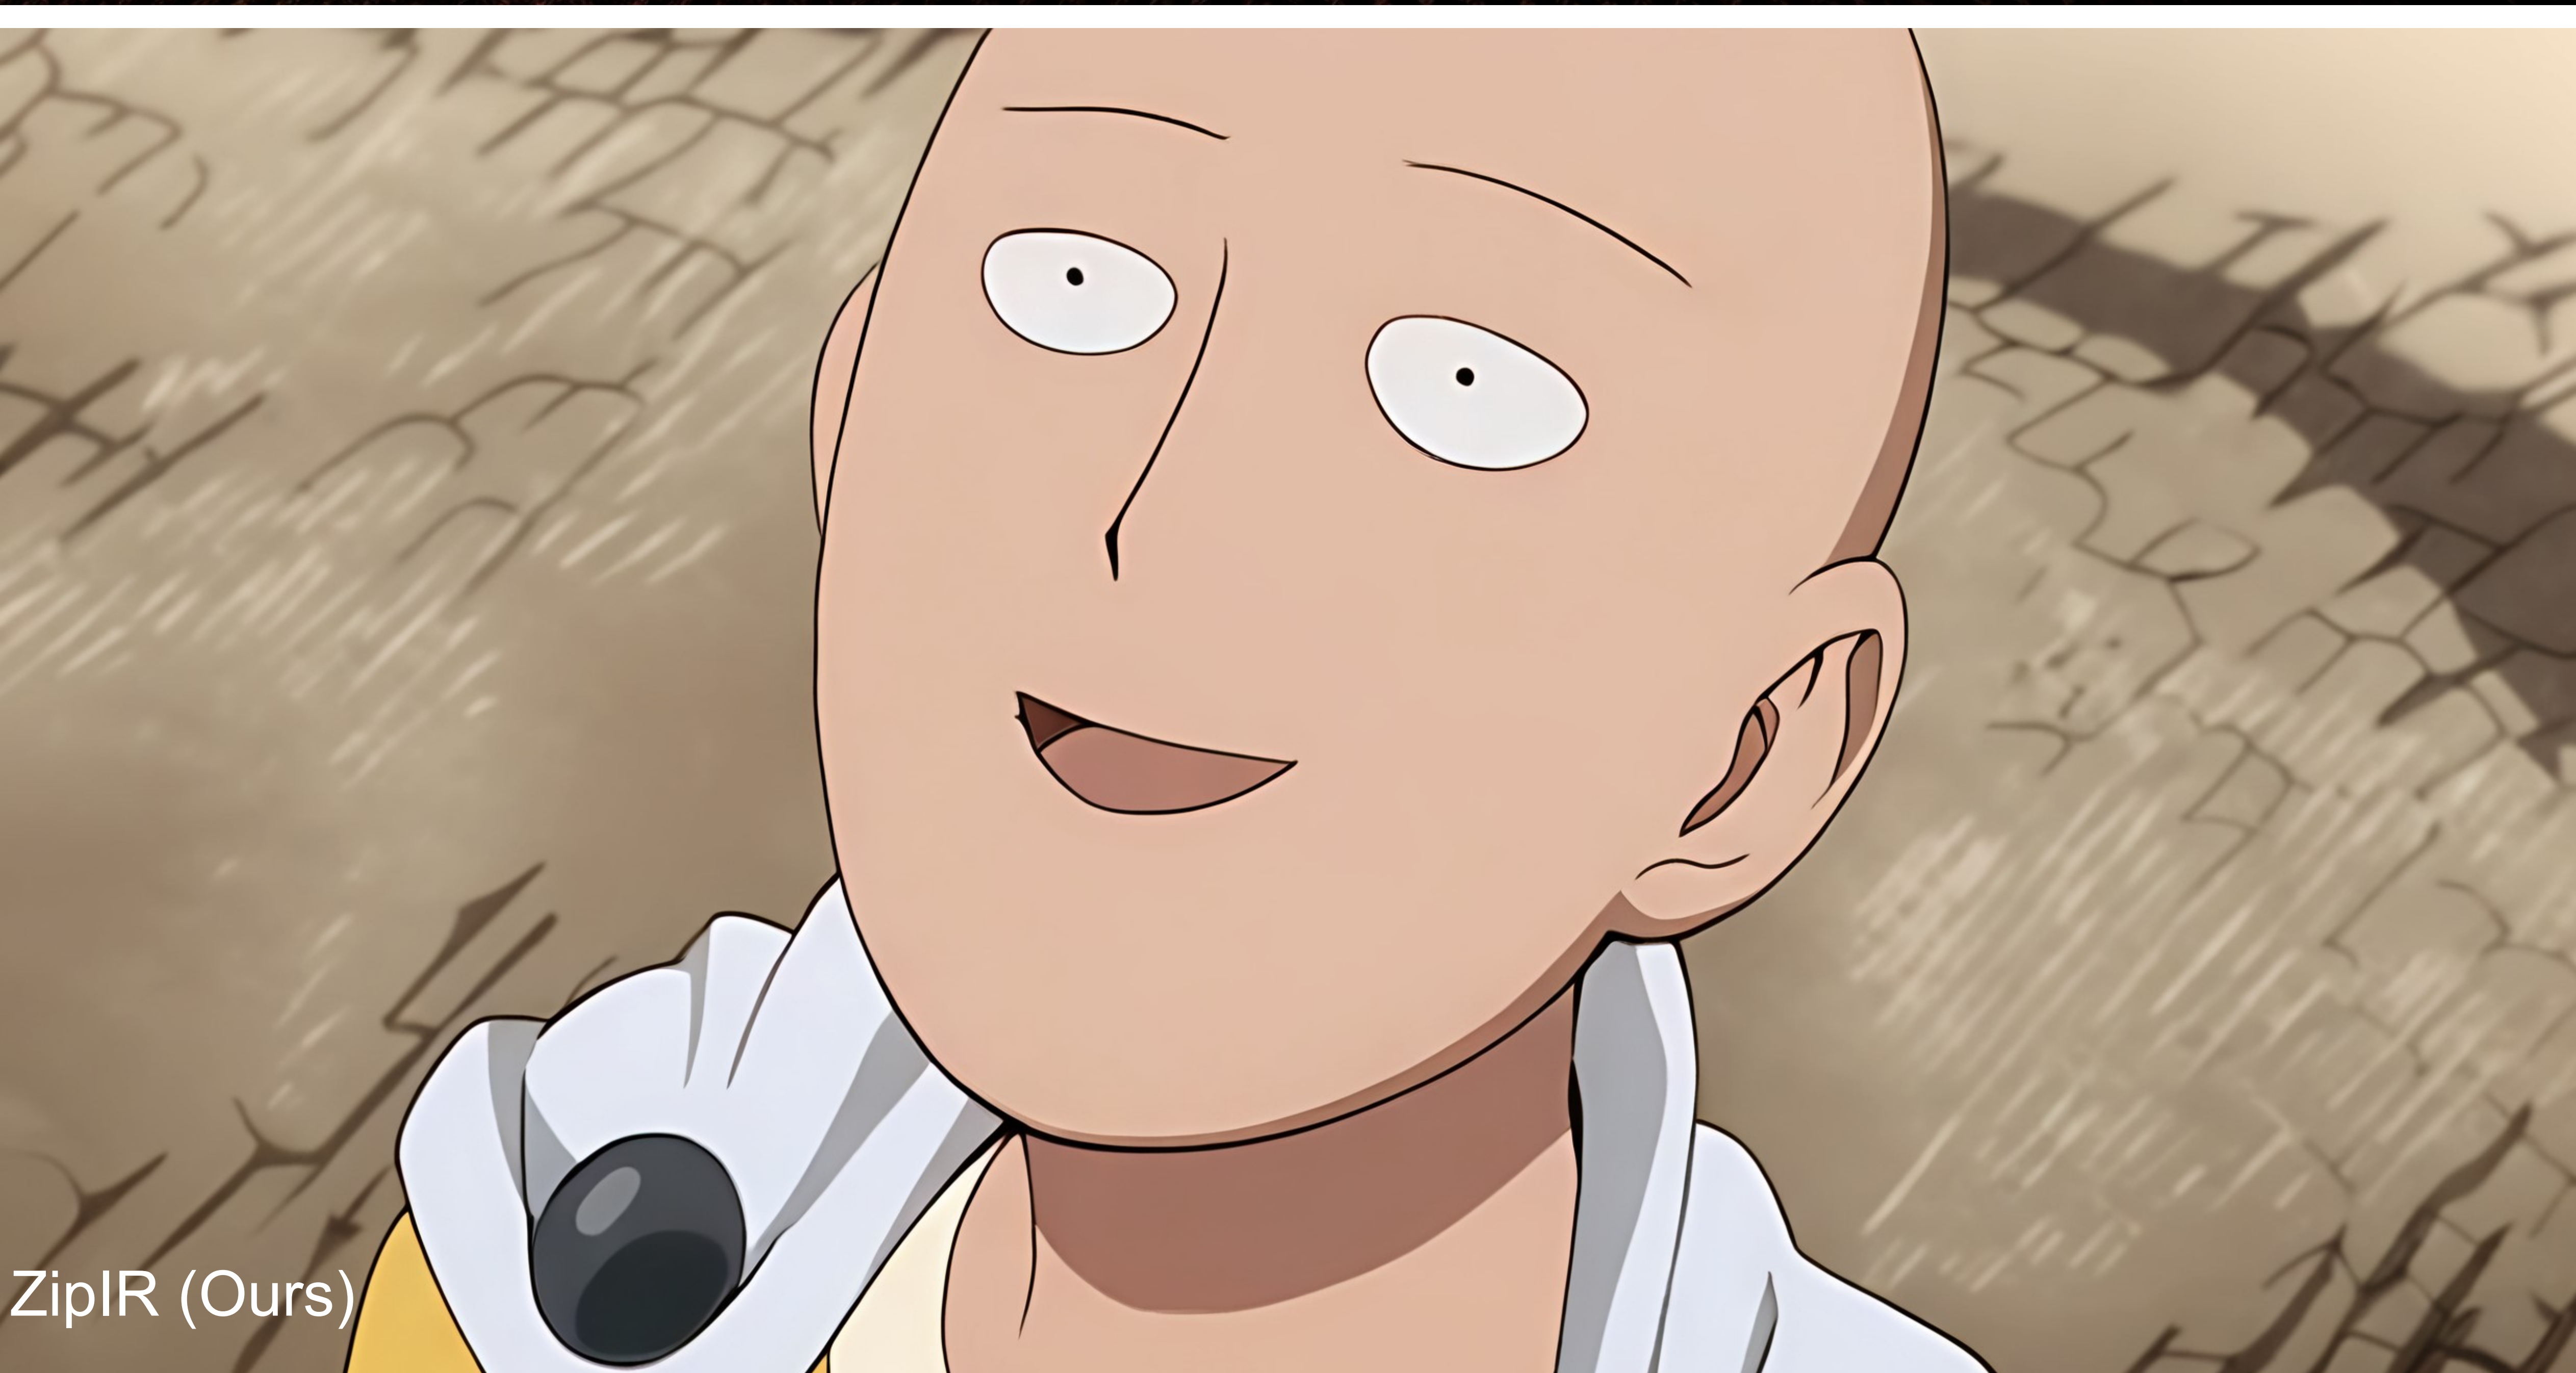

ZipIR (Ours)

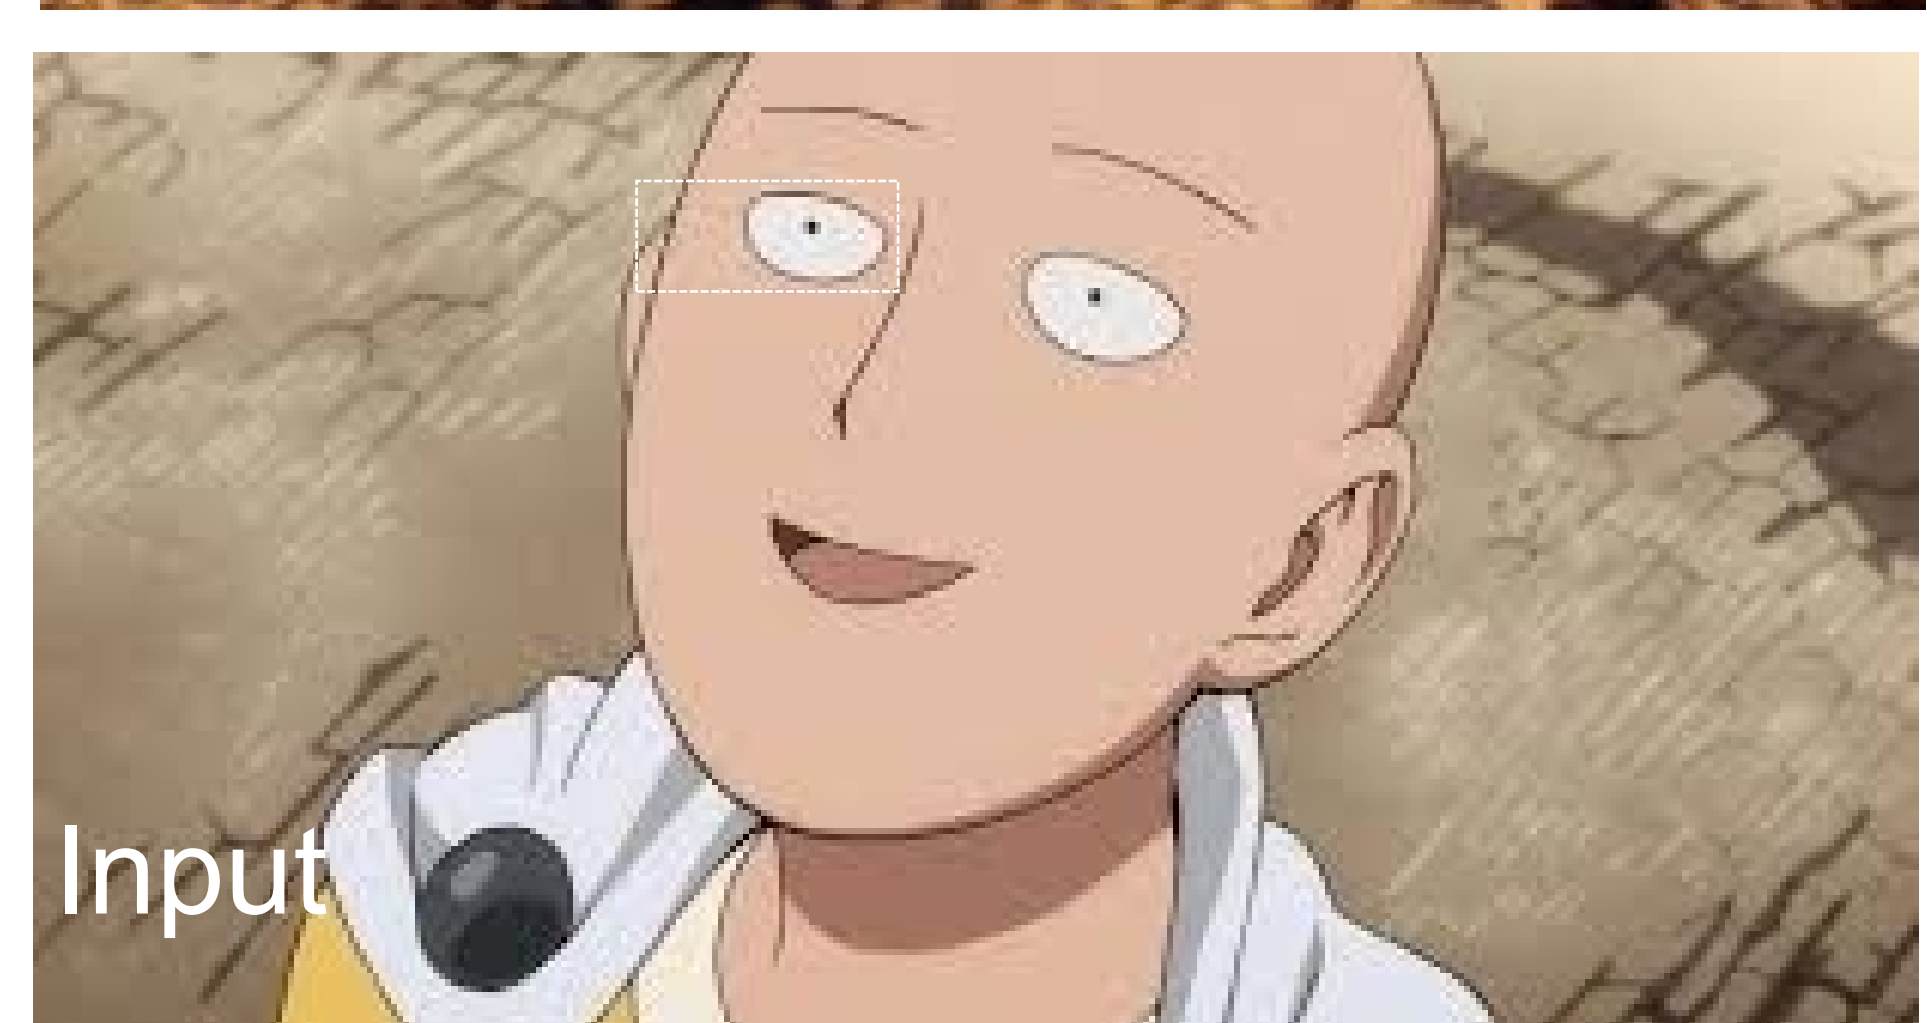

Input

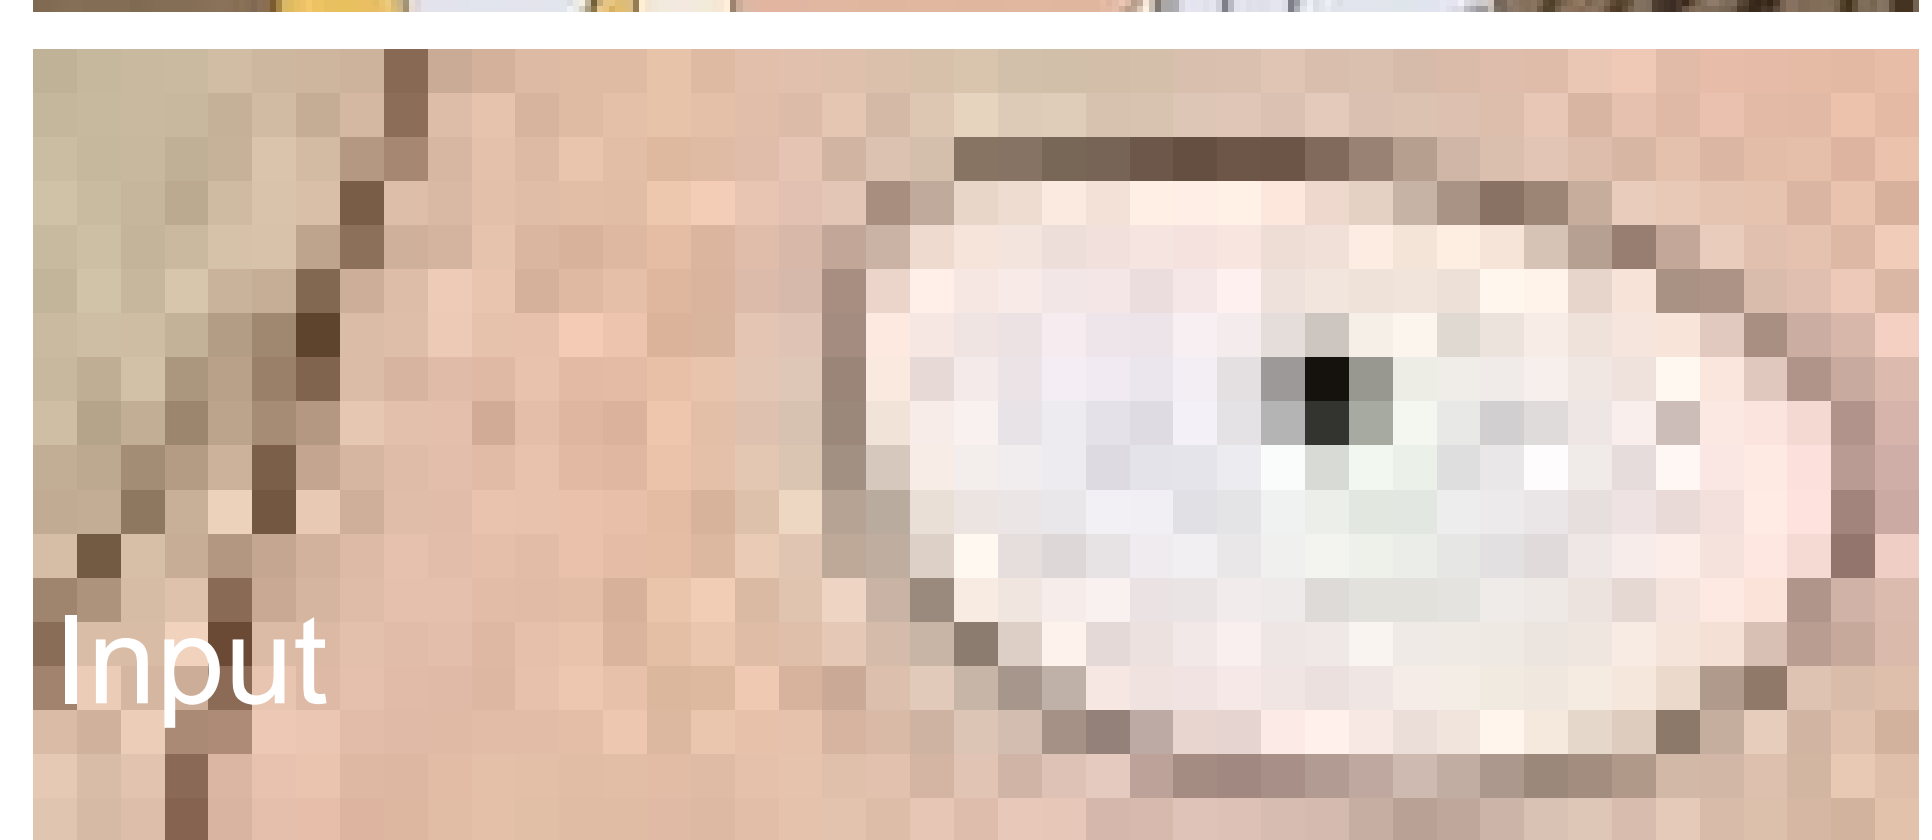

Input

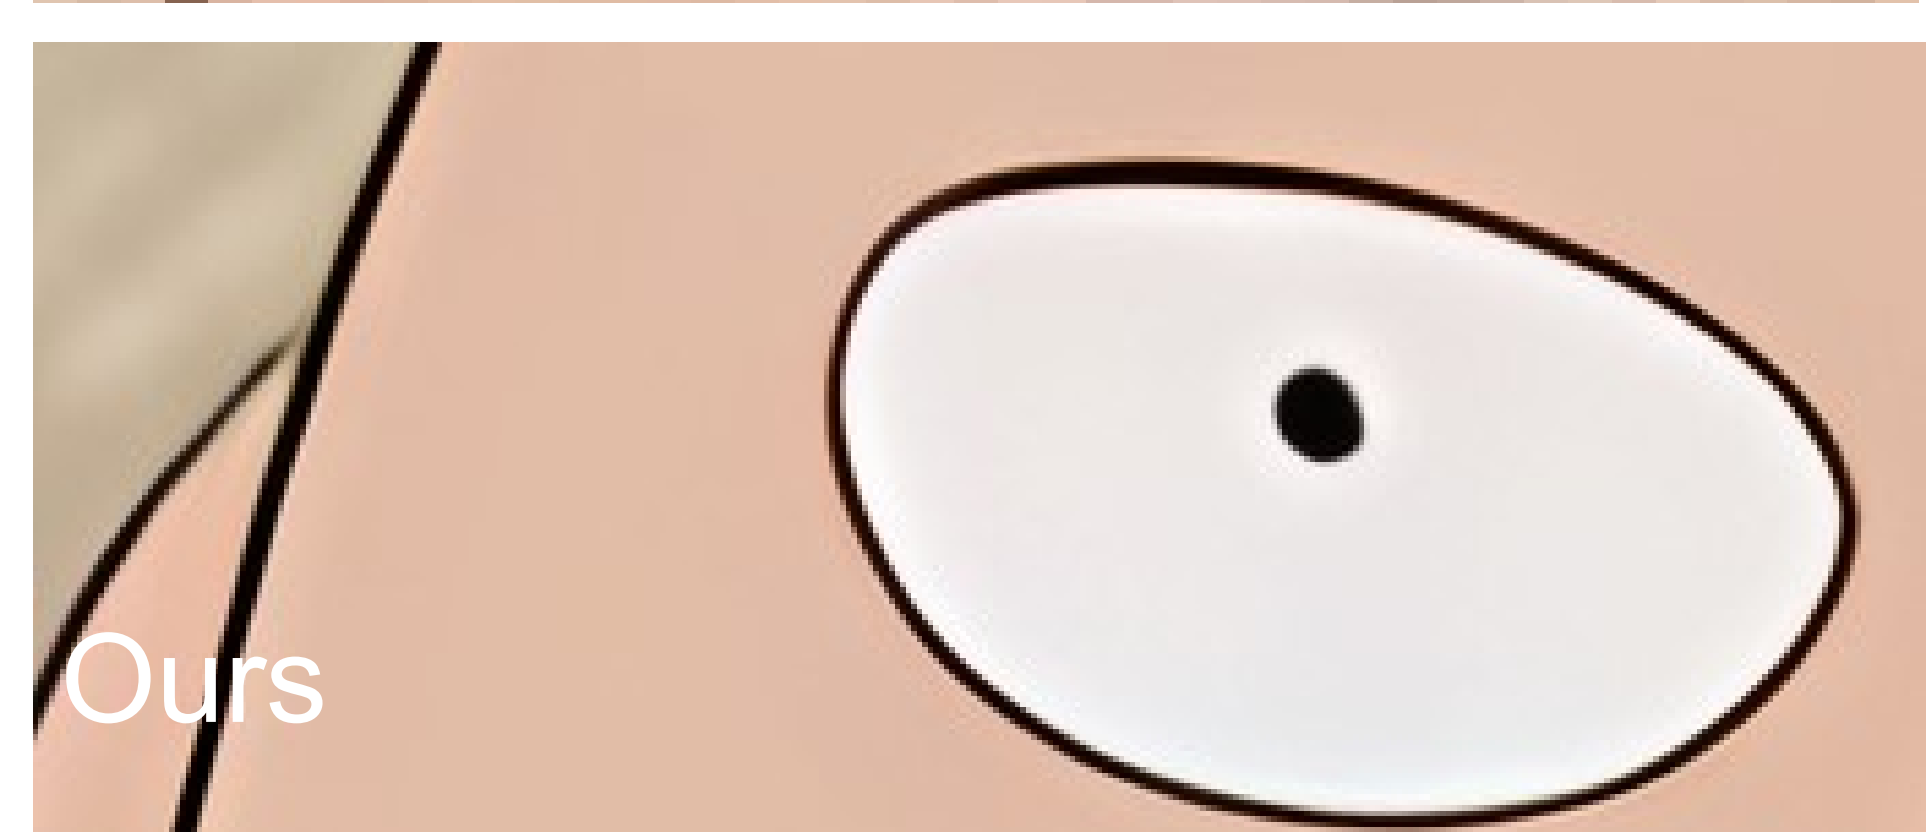

Ours

**ME ALL DAY**

**ME AT 3AM**

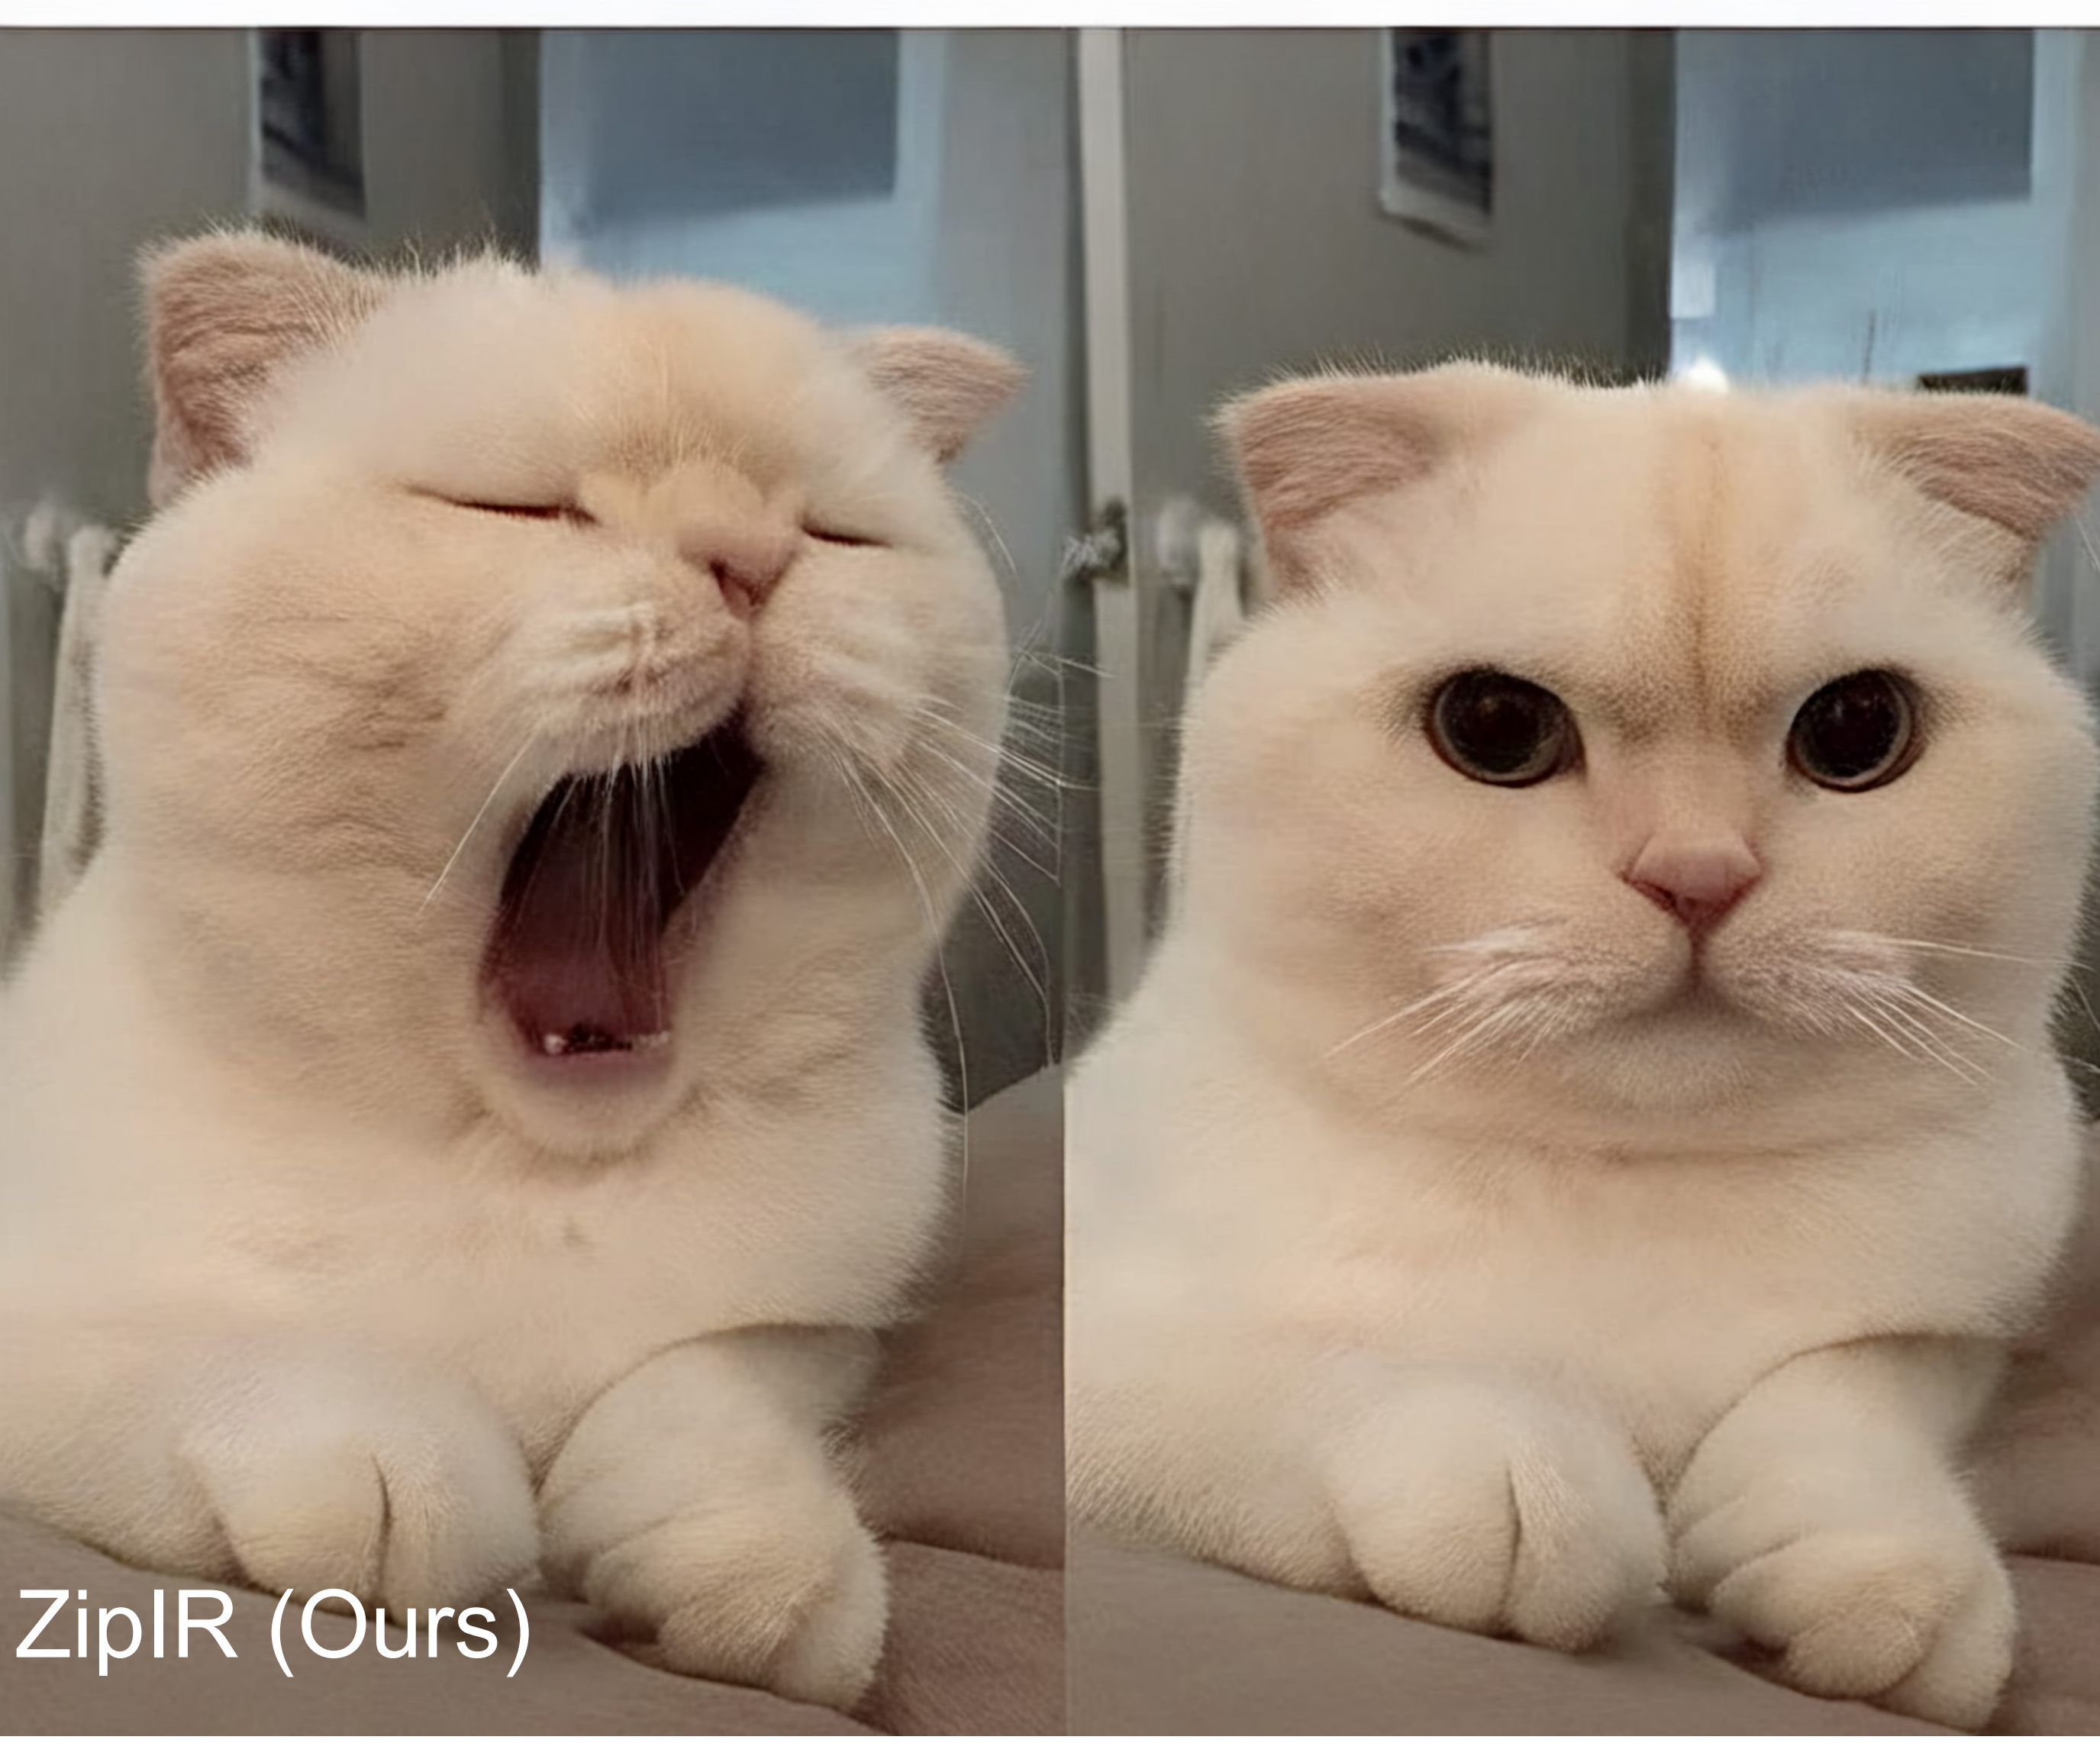

ZipIR (Ours)

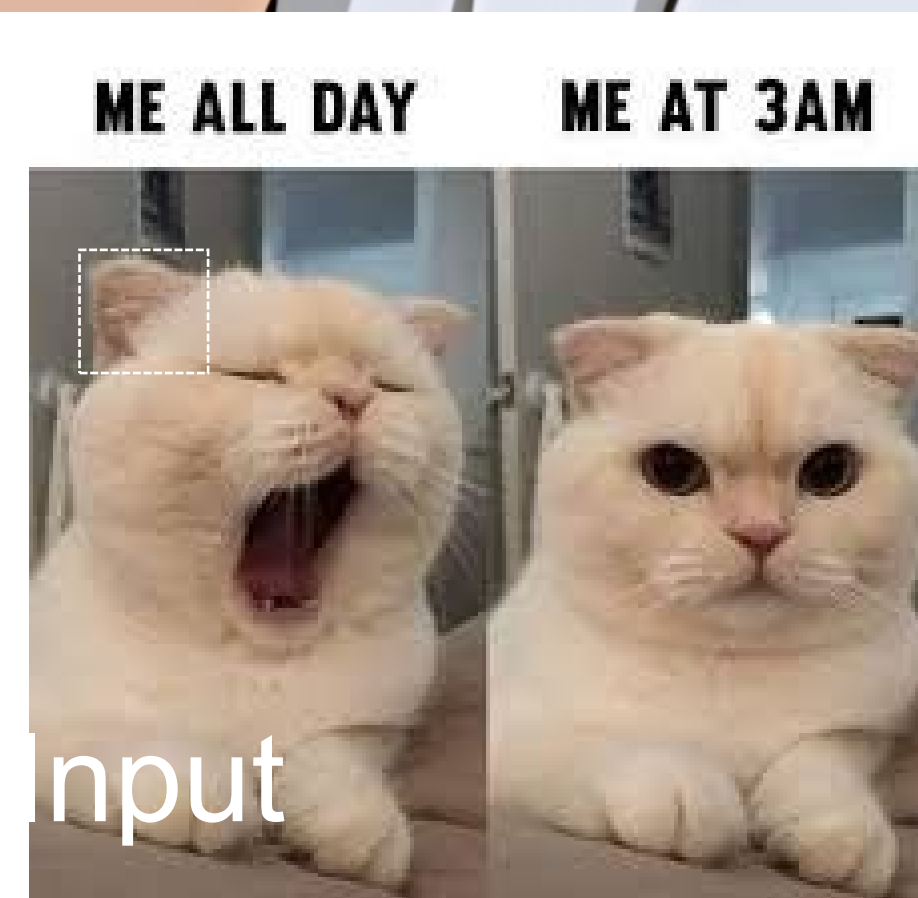

Input

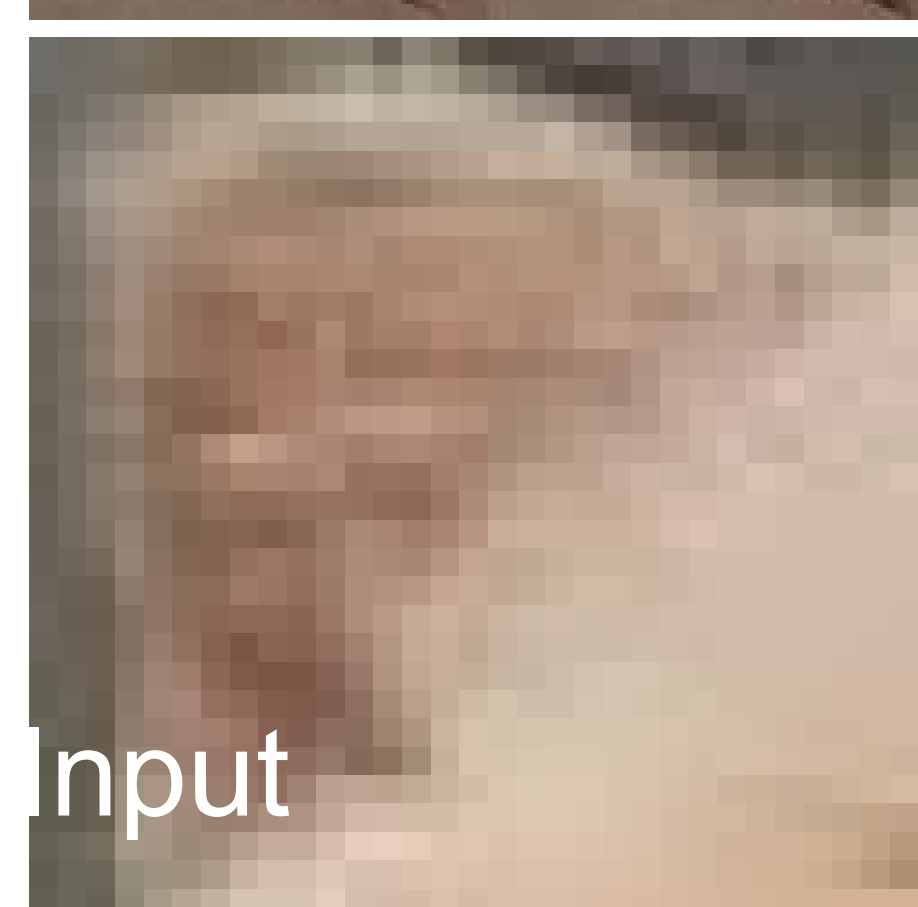

Input

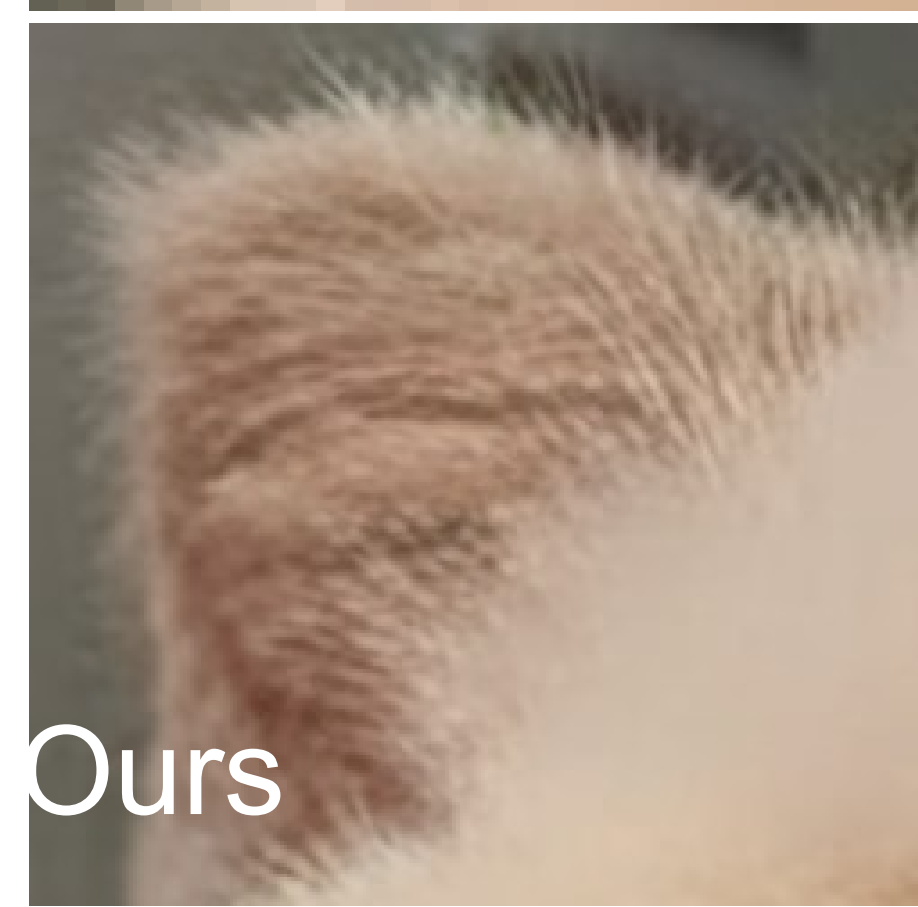

Ours

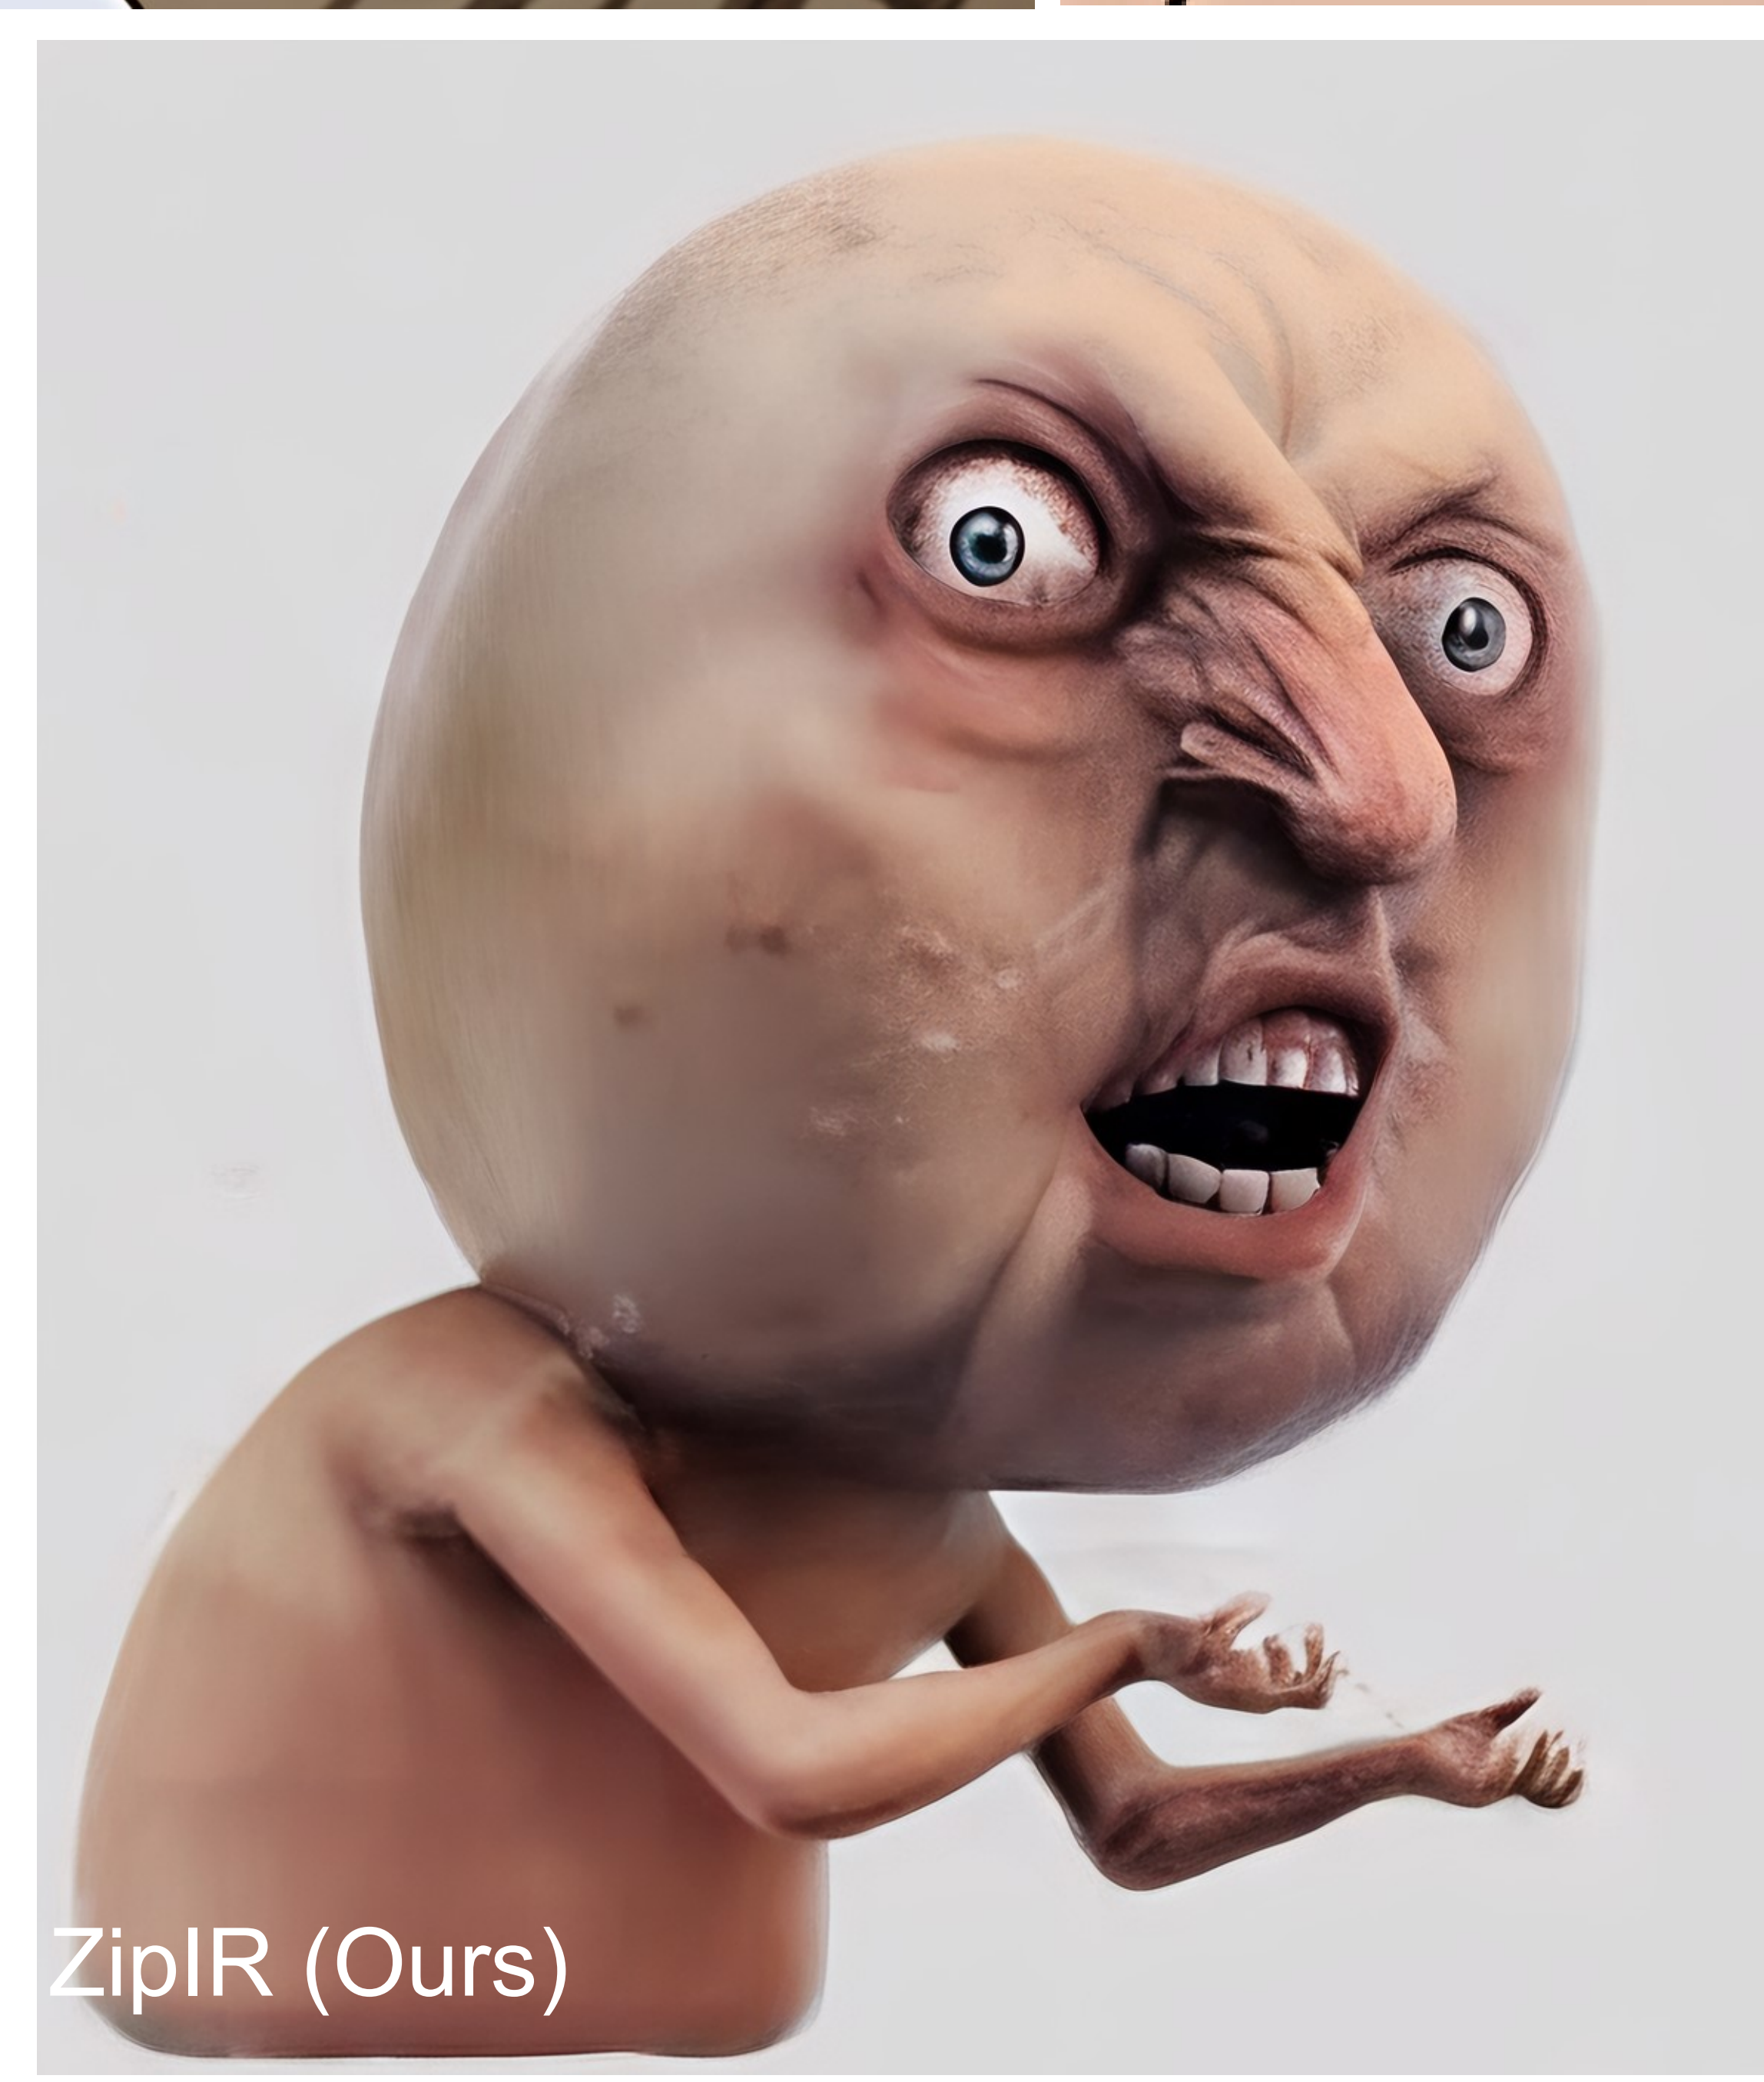

ZipIR (Ours)

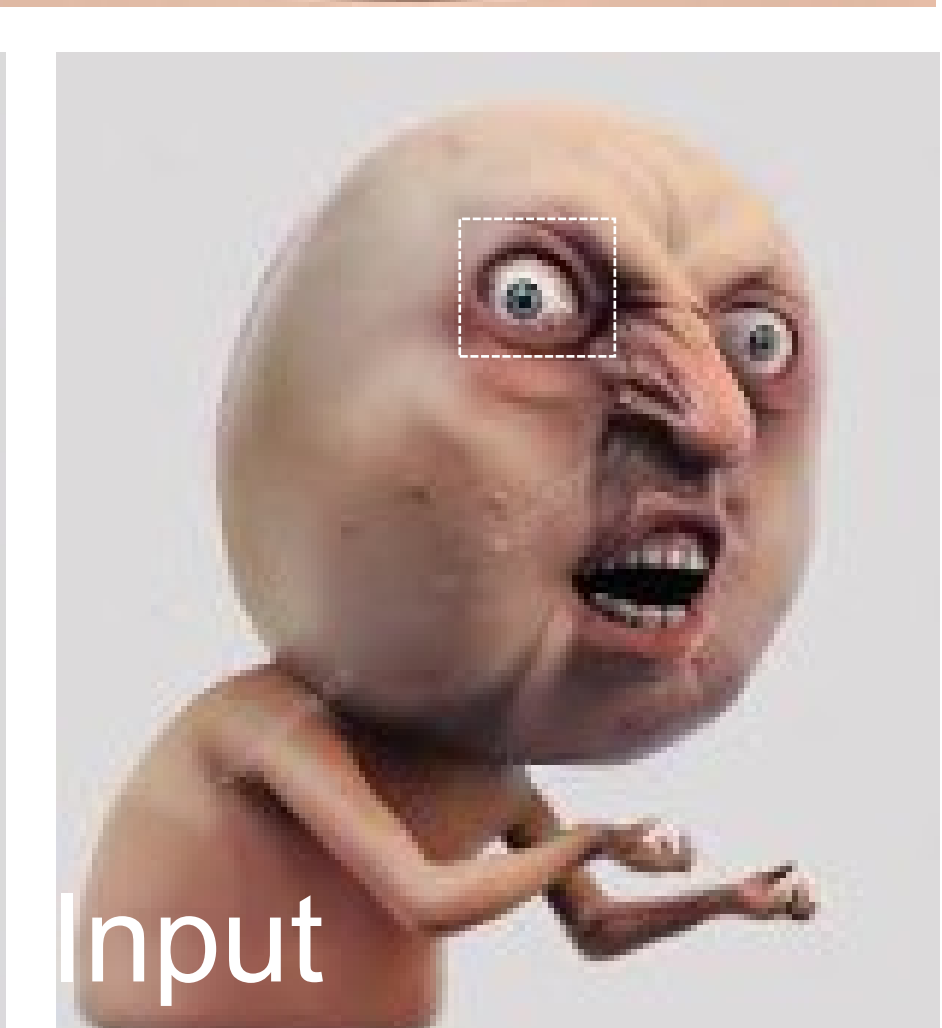

Input

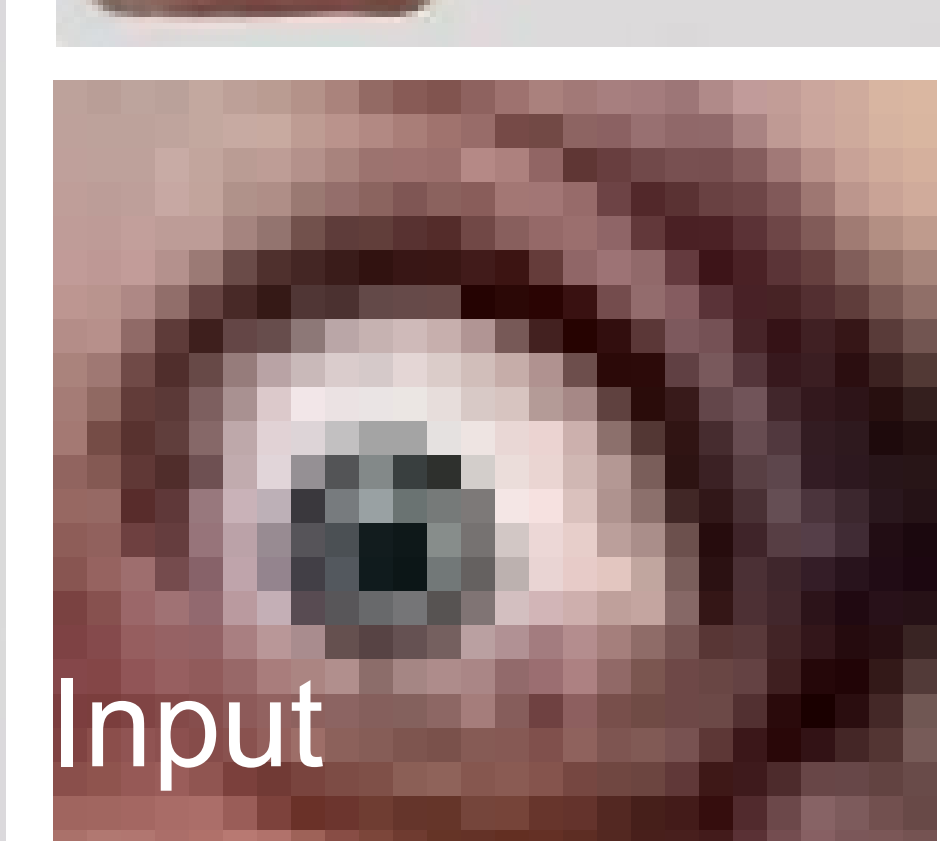

Input

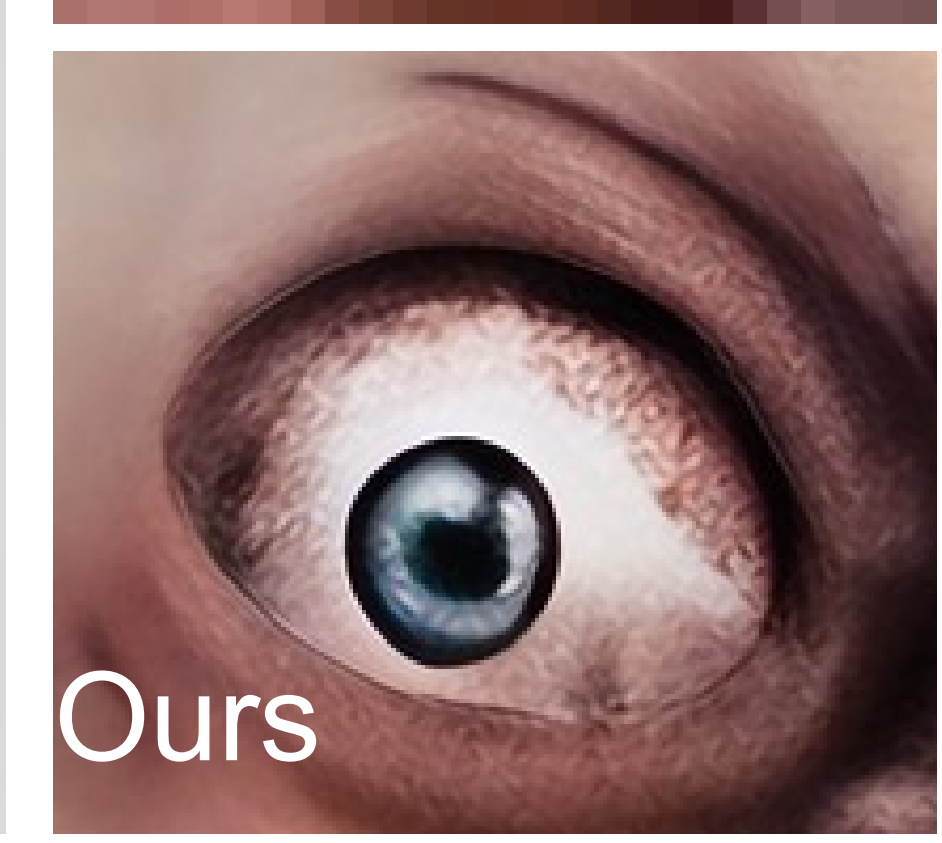

Ours



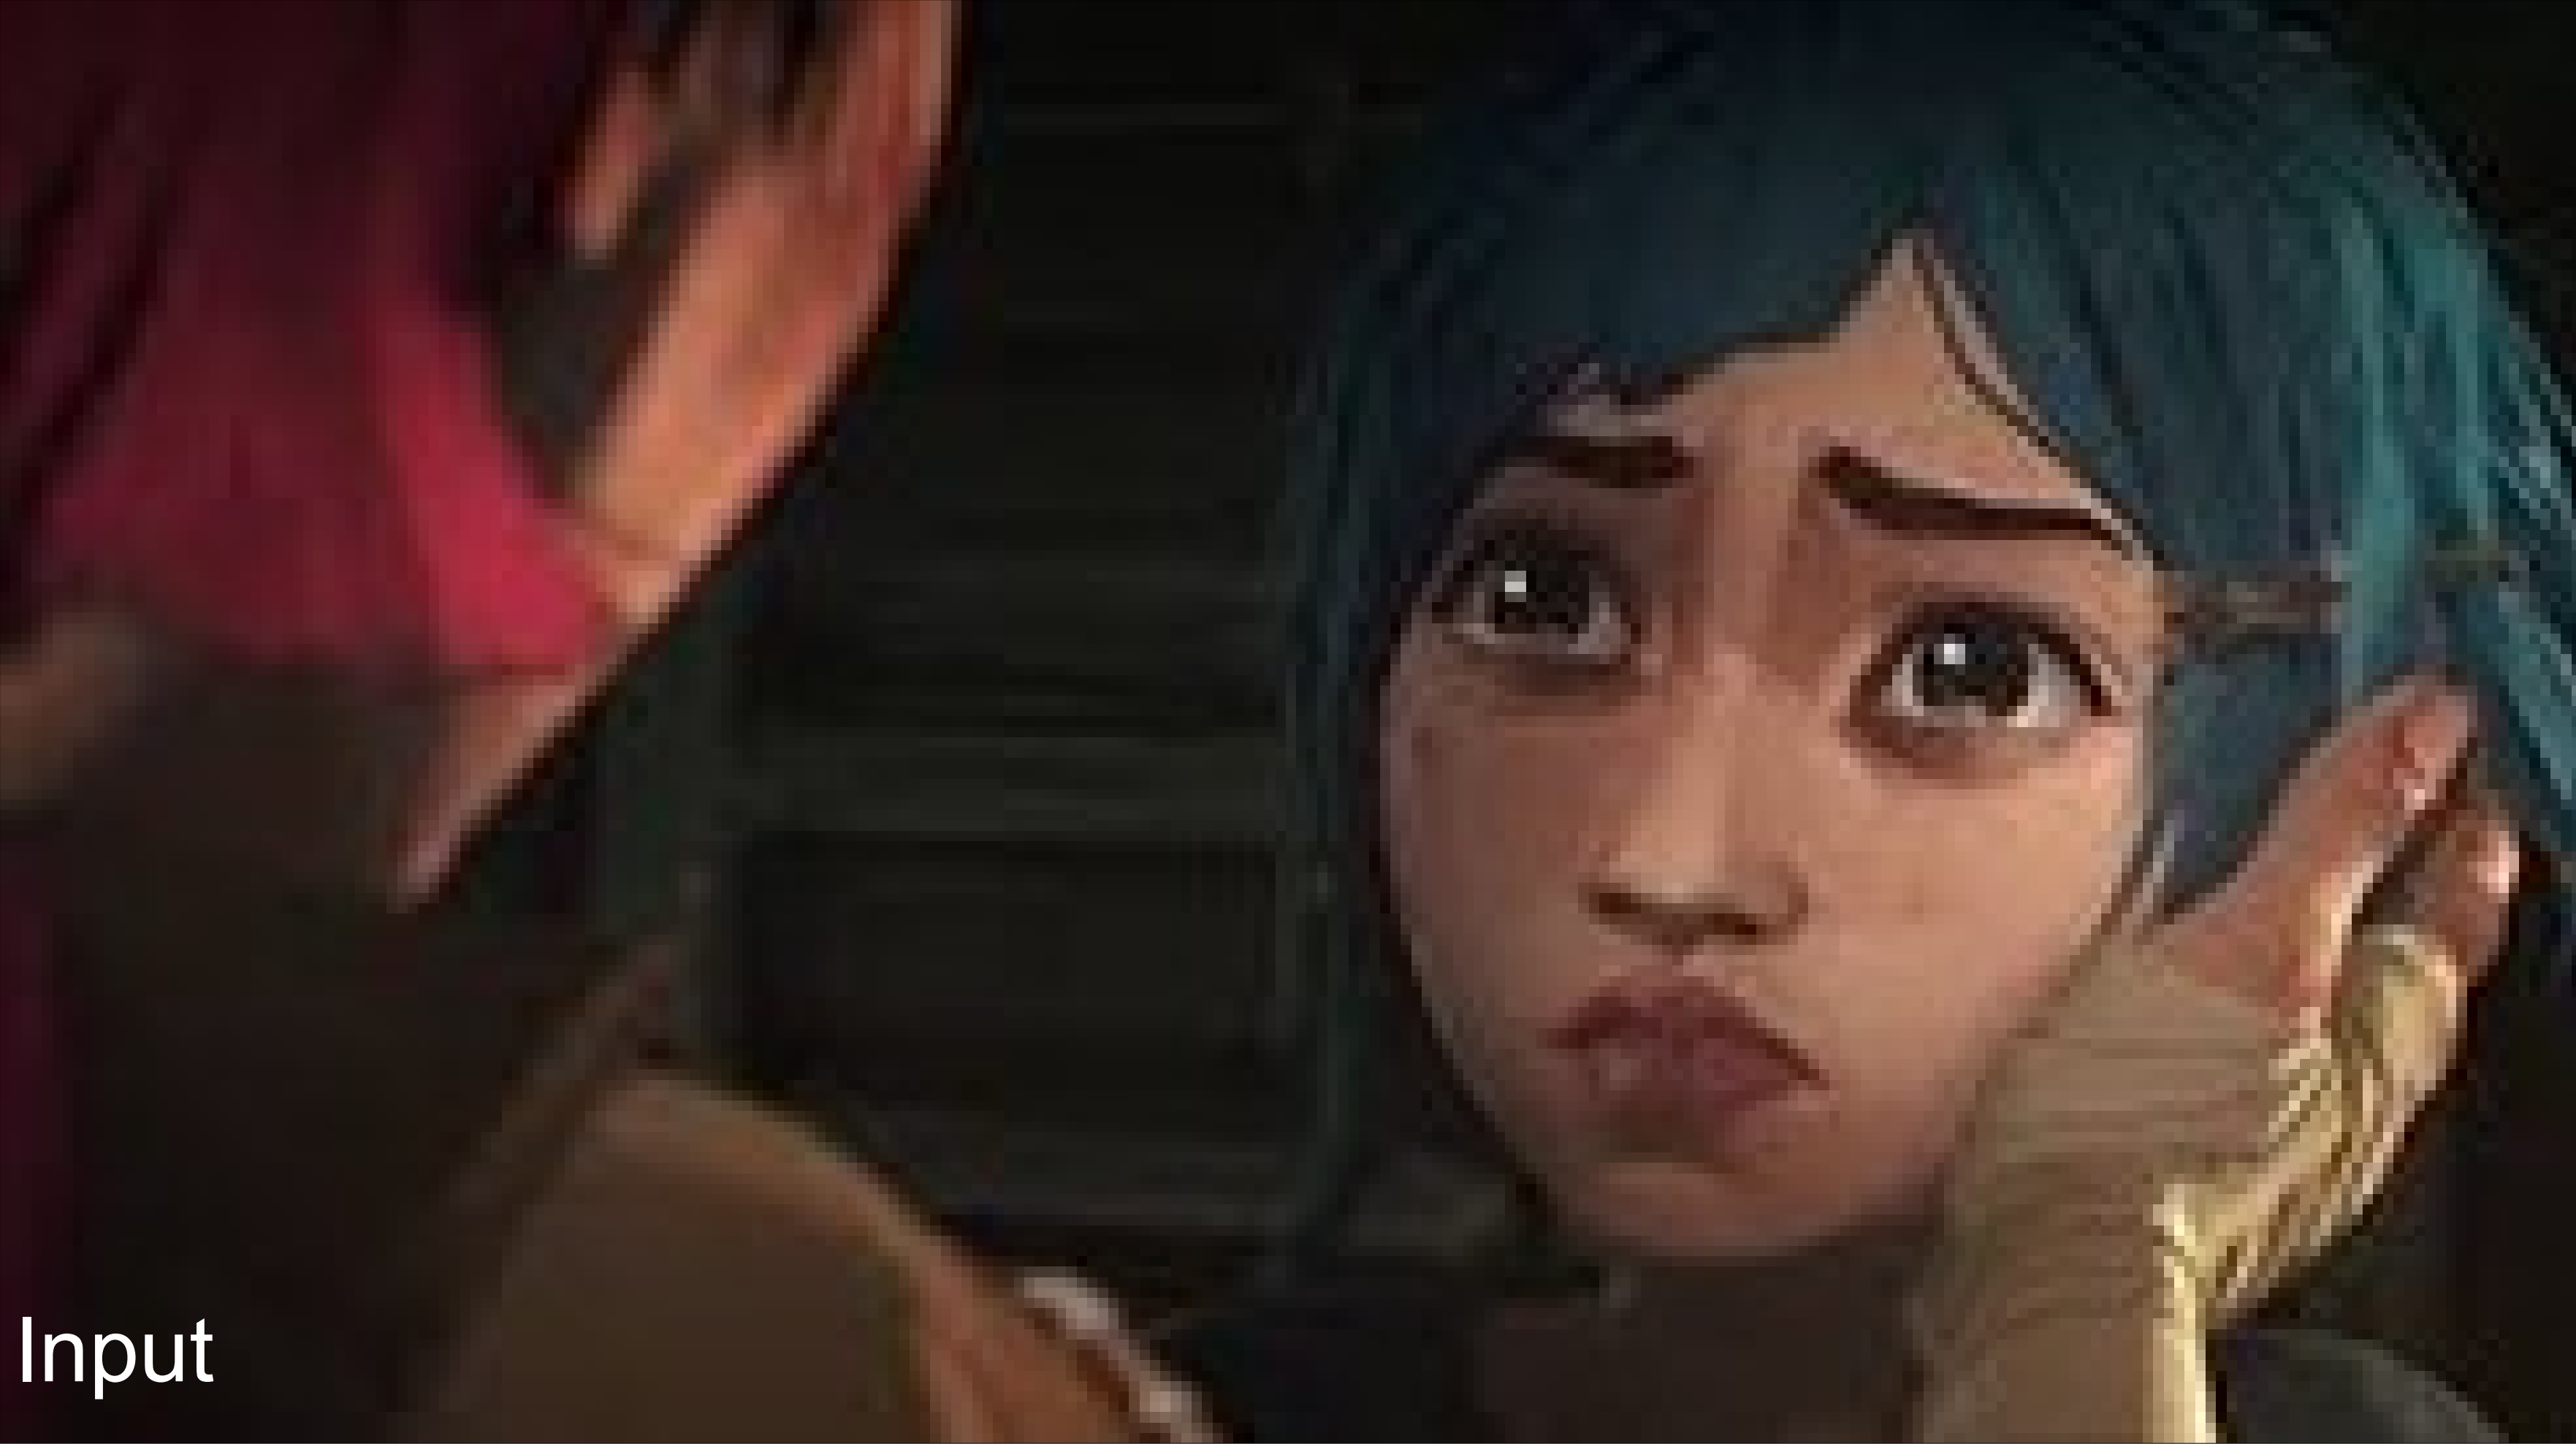

Input

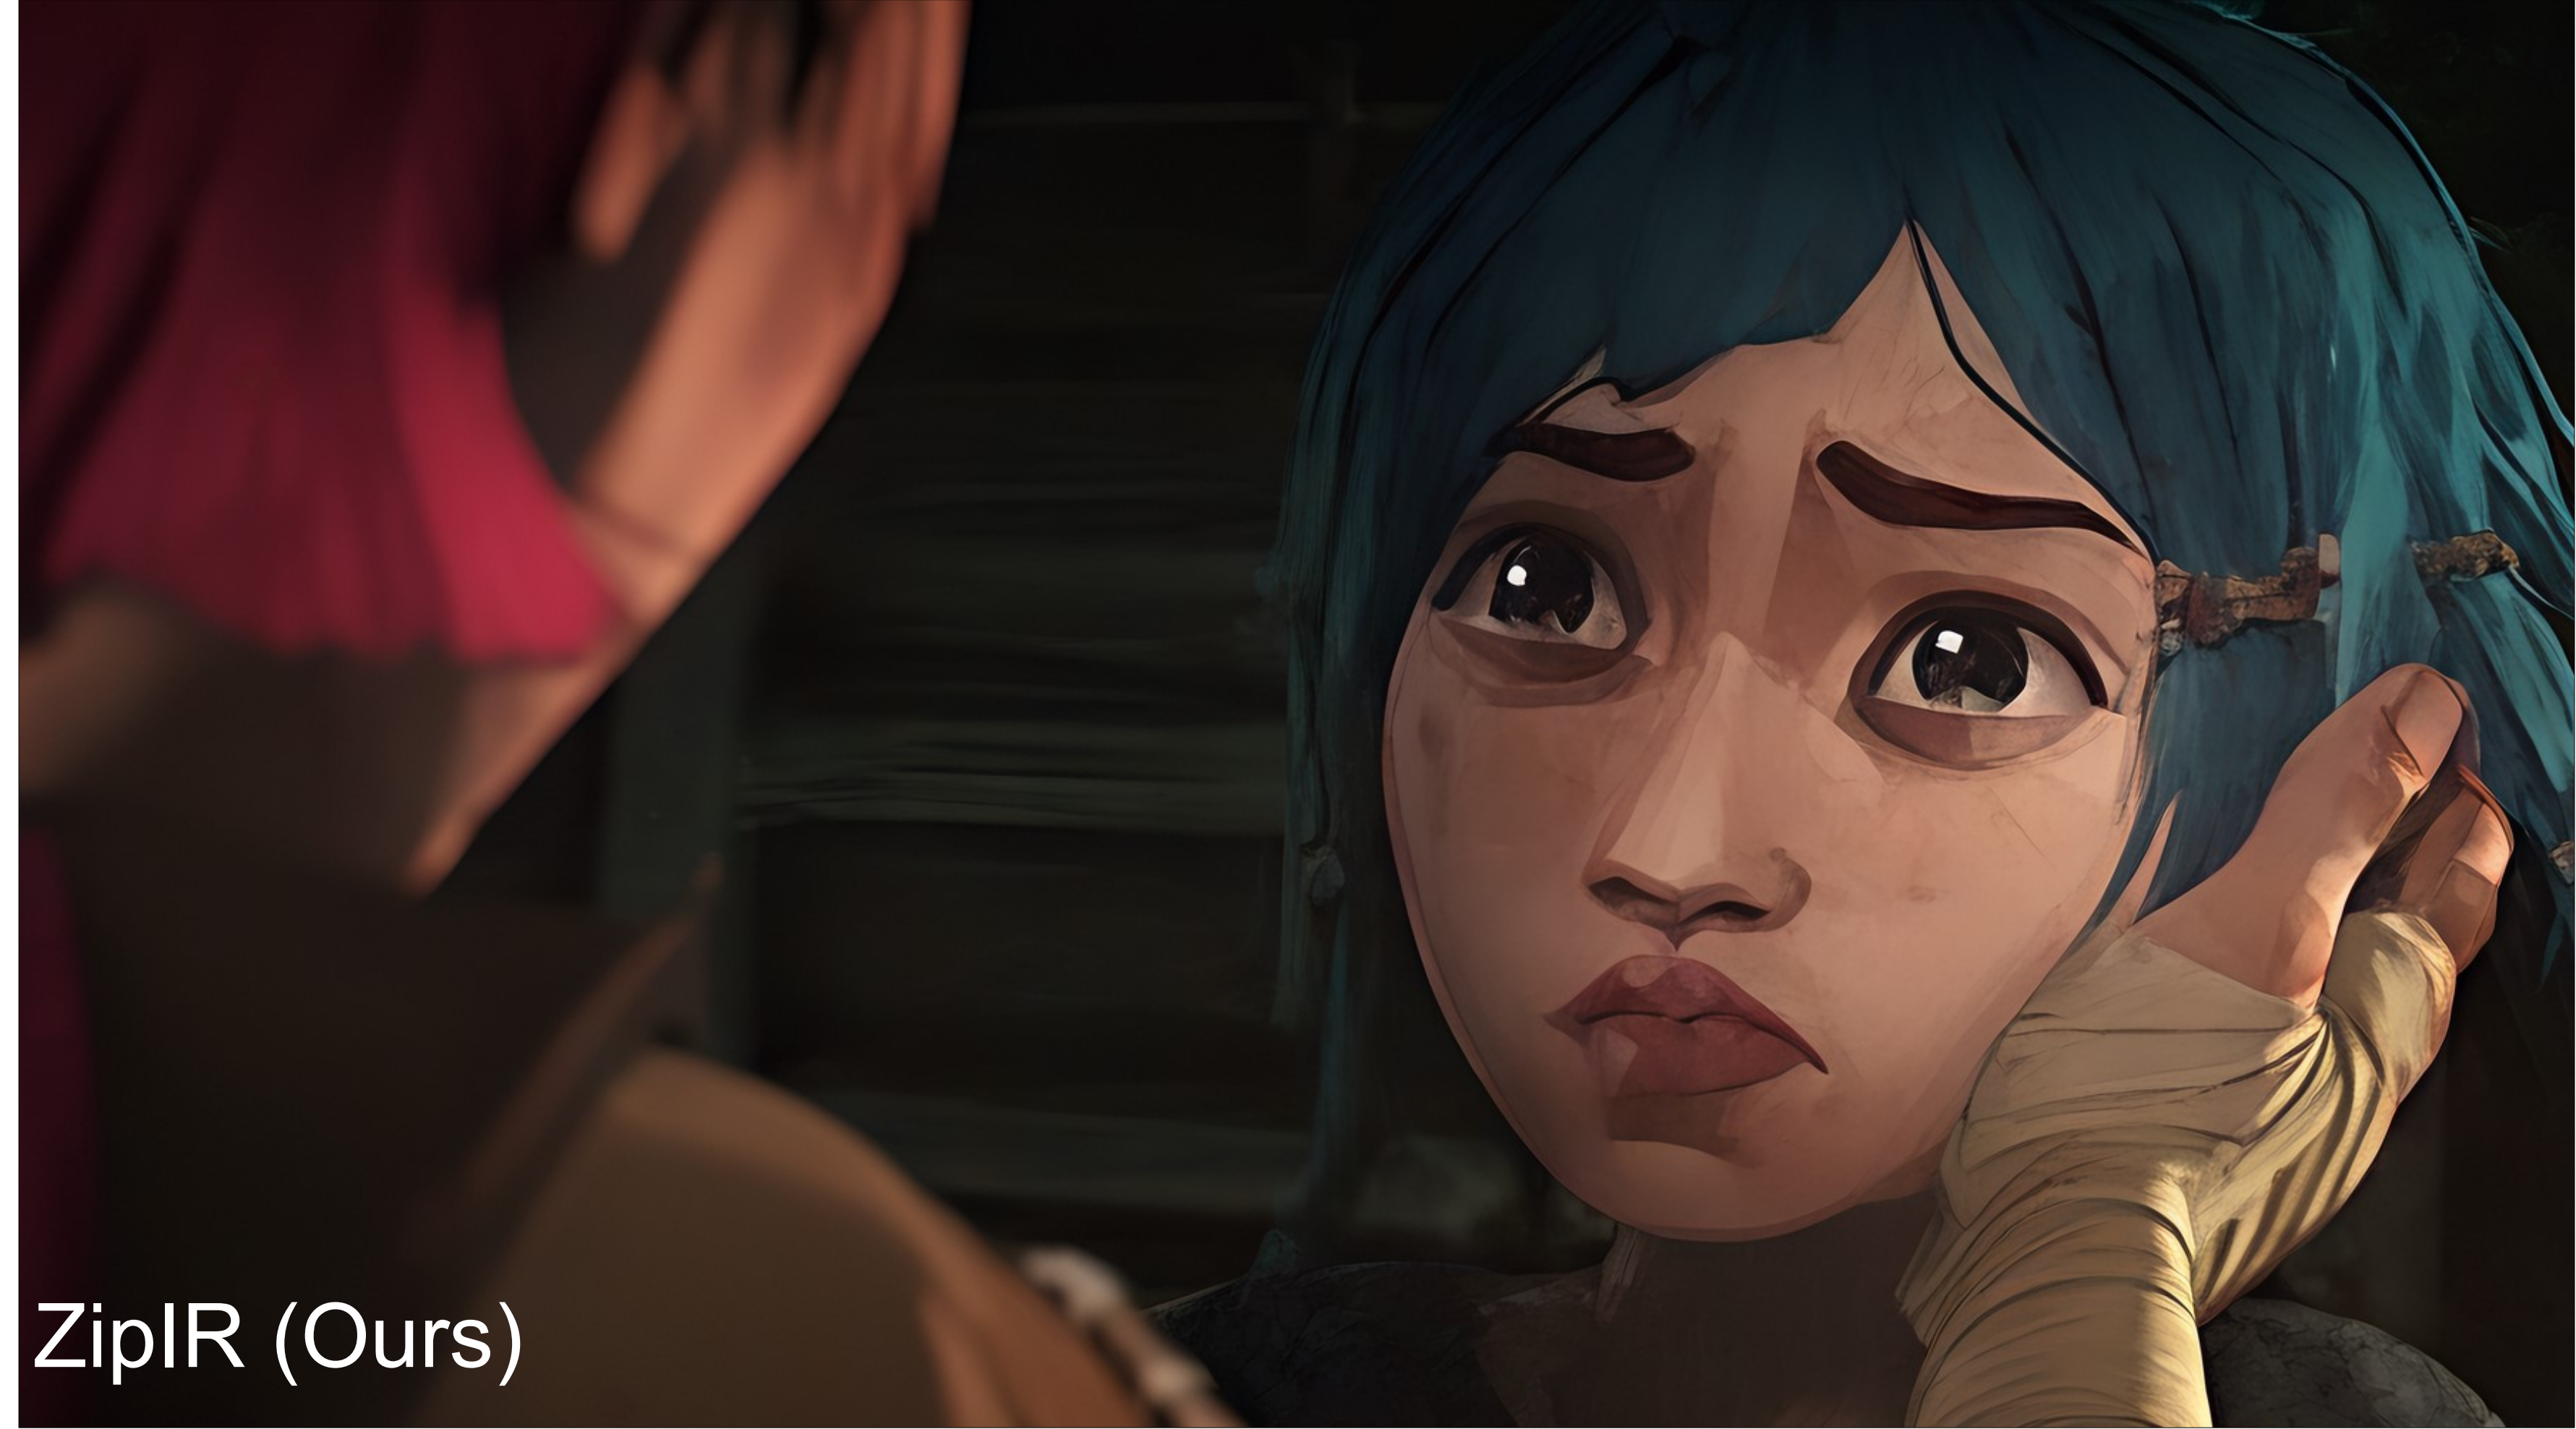

ZipIR (Ours)

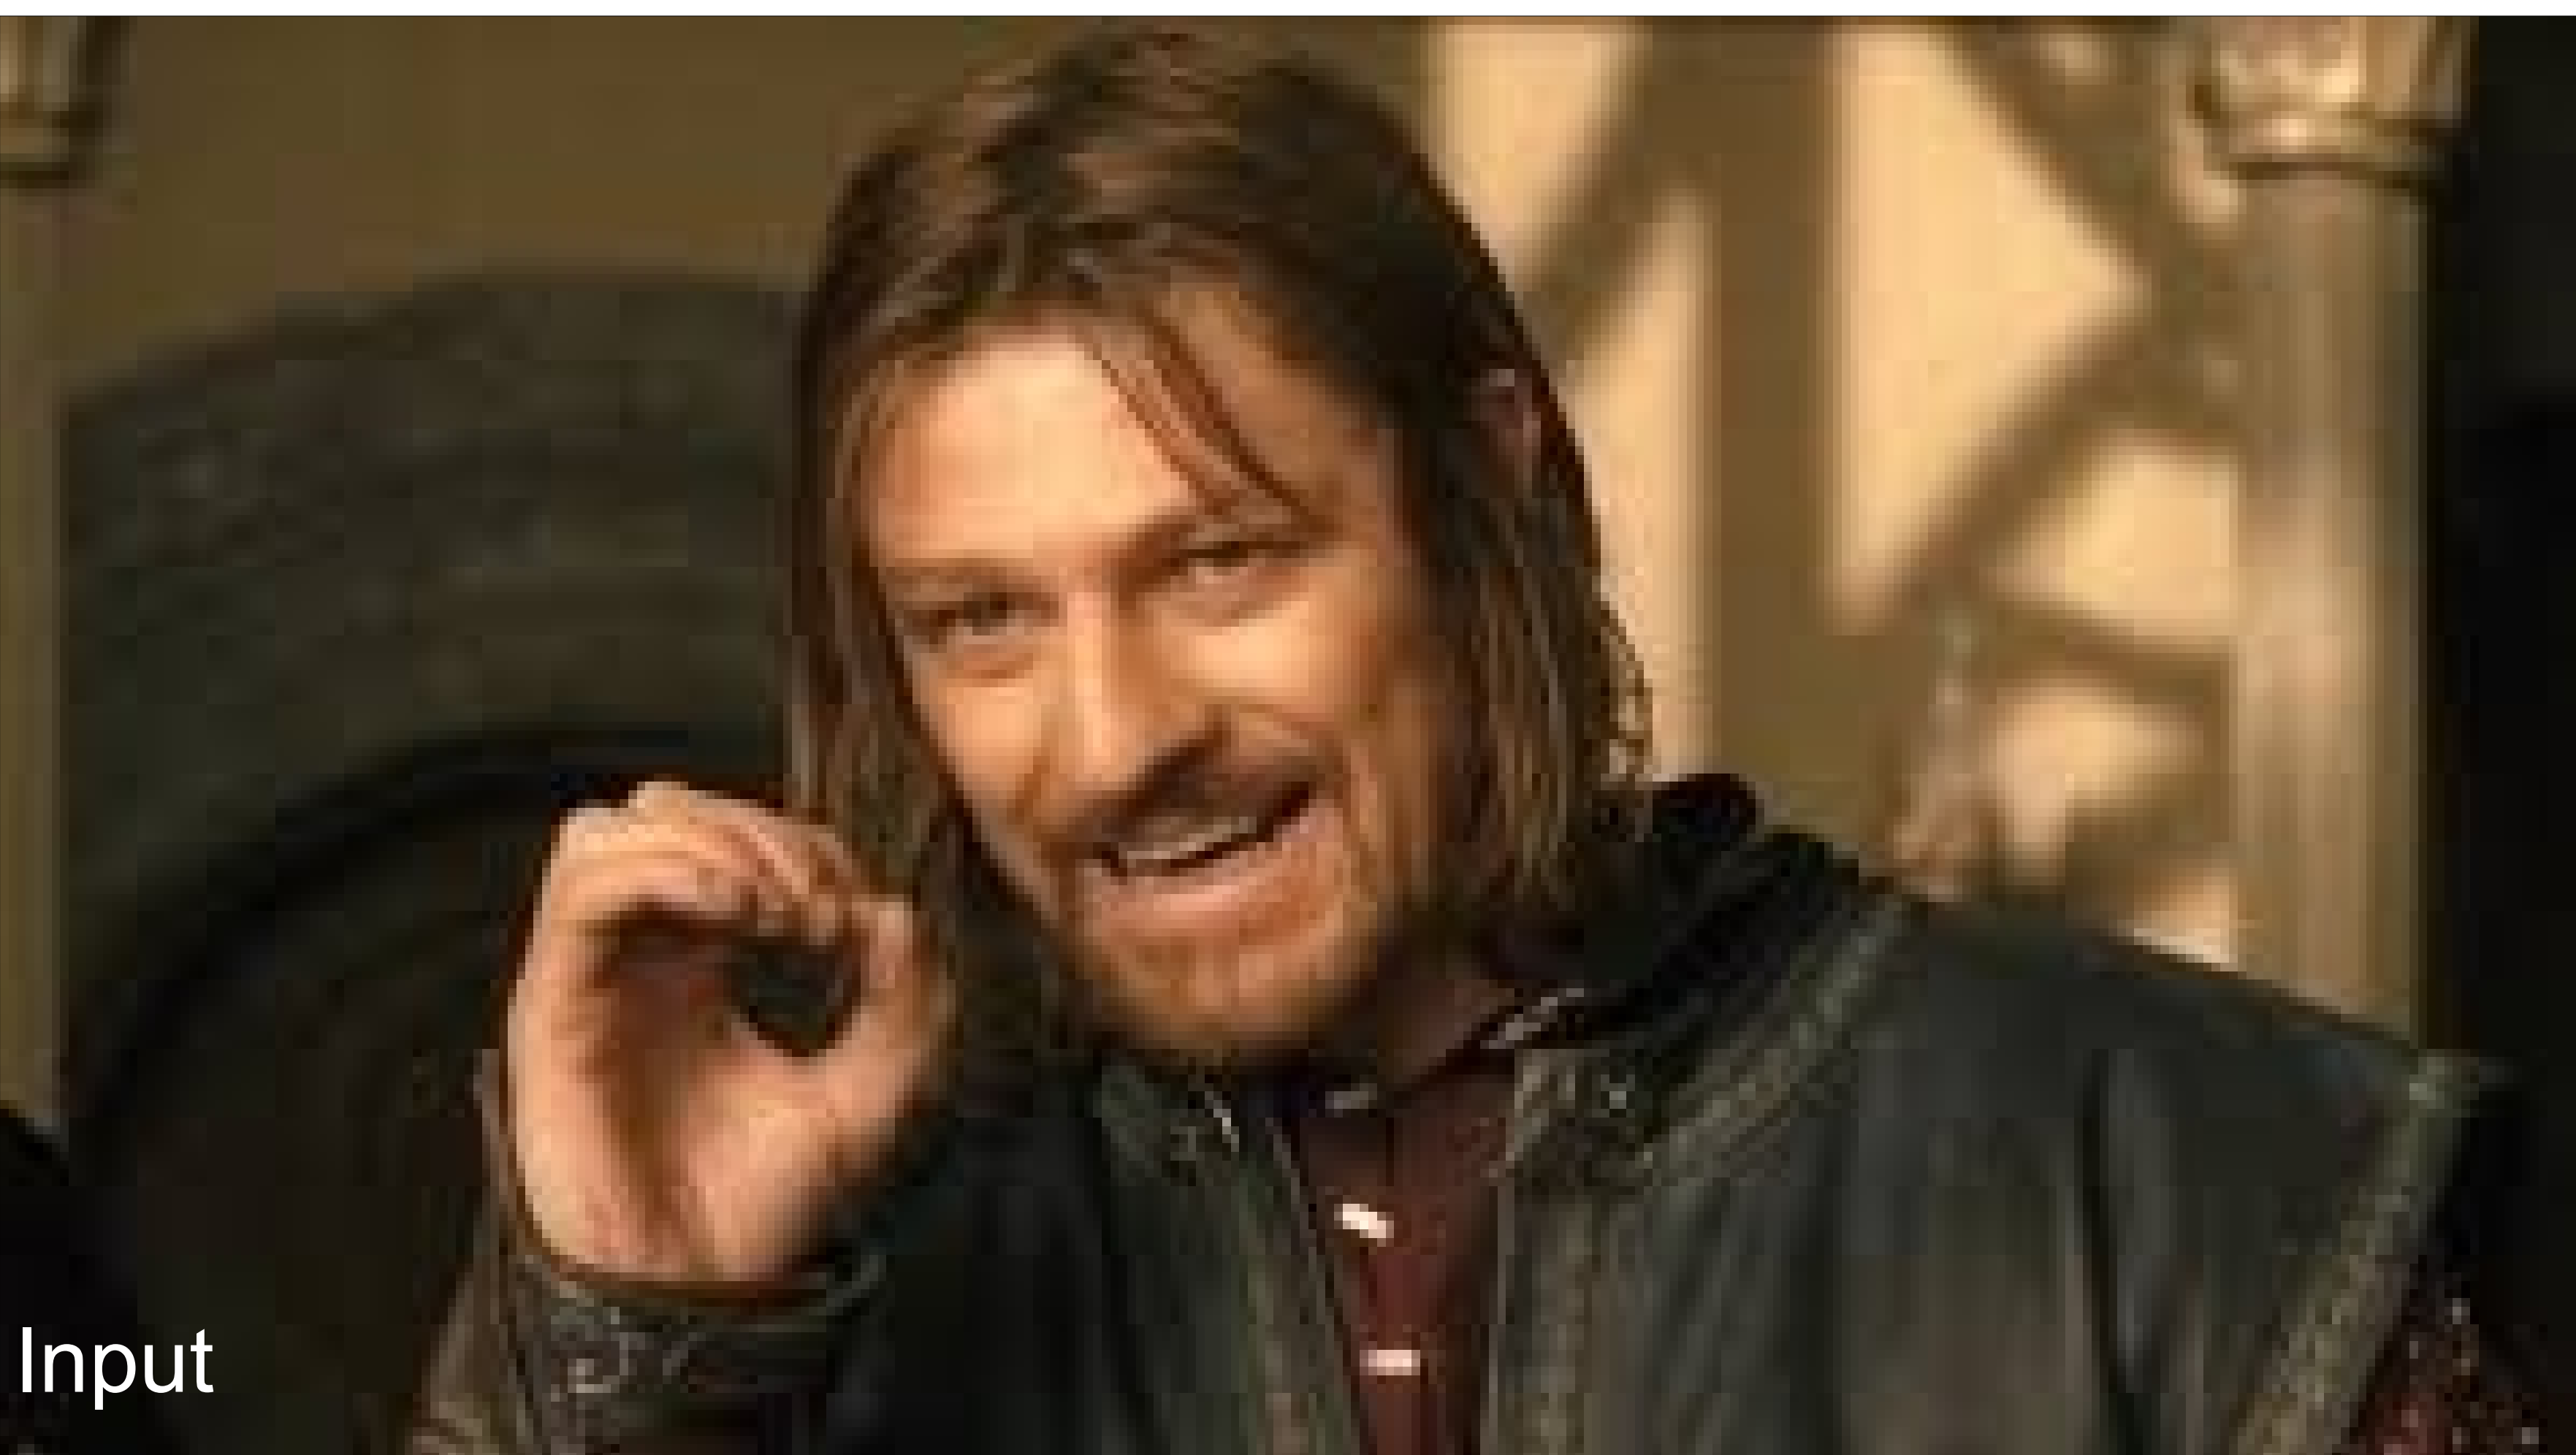

Input

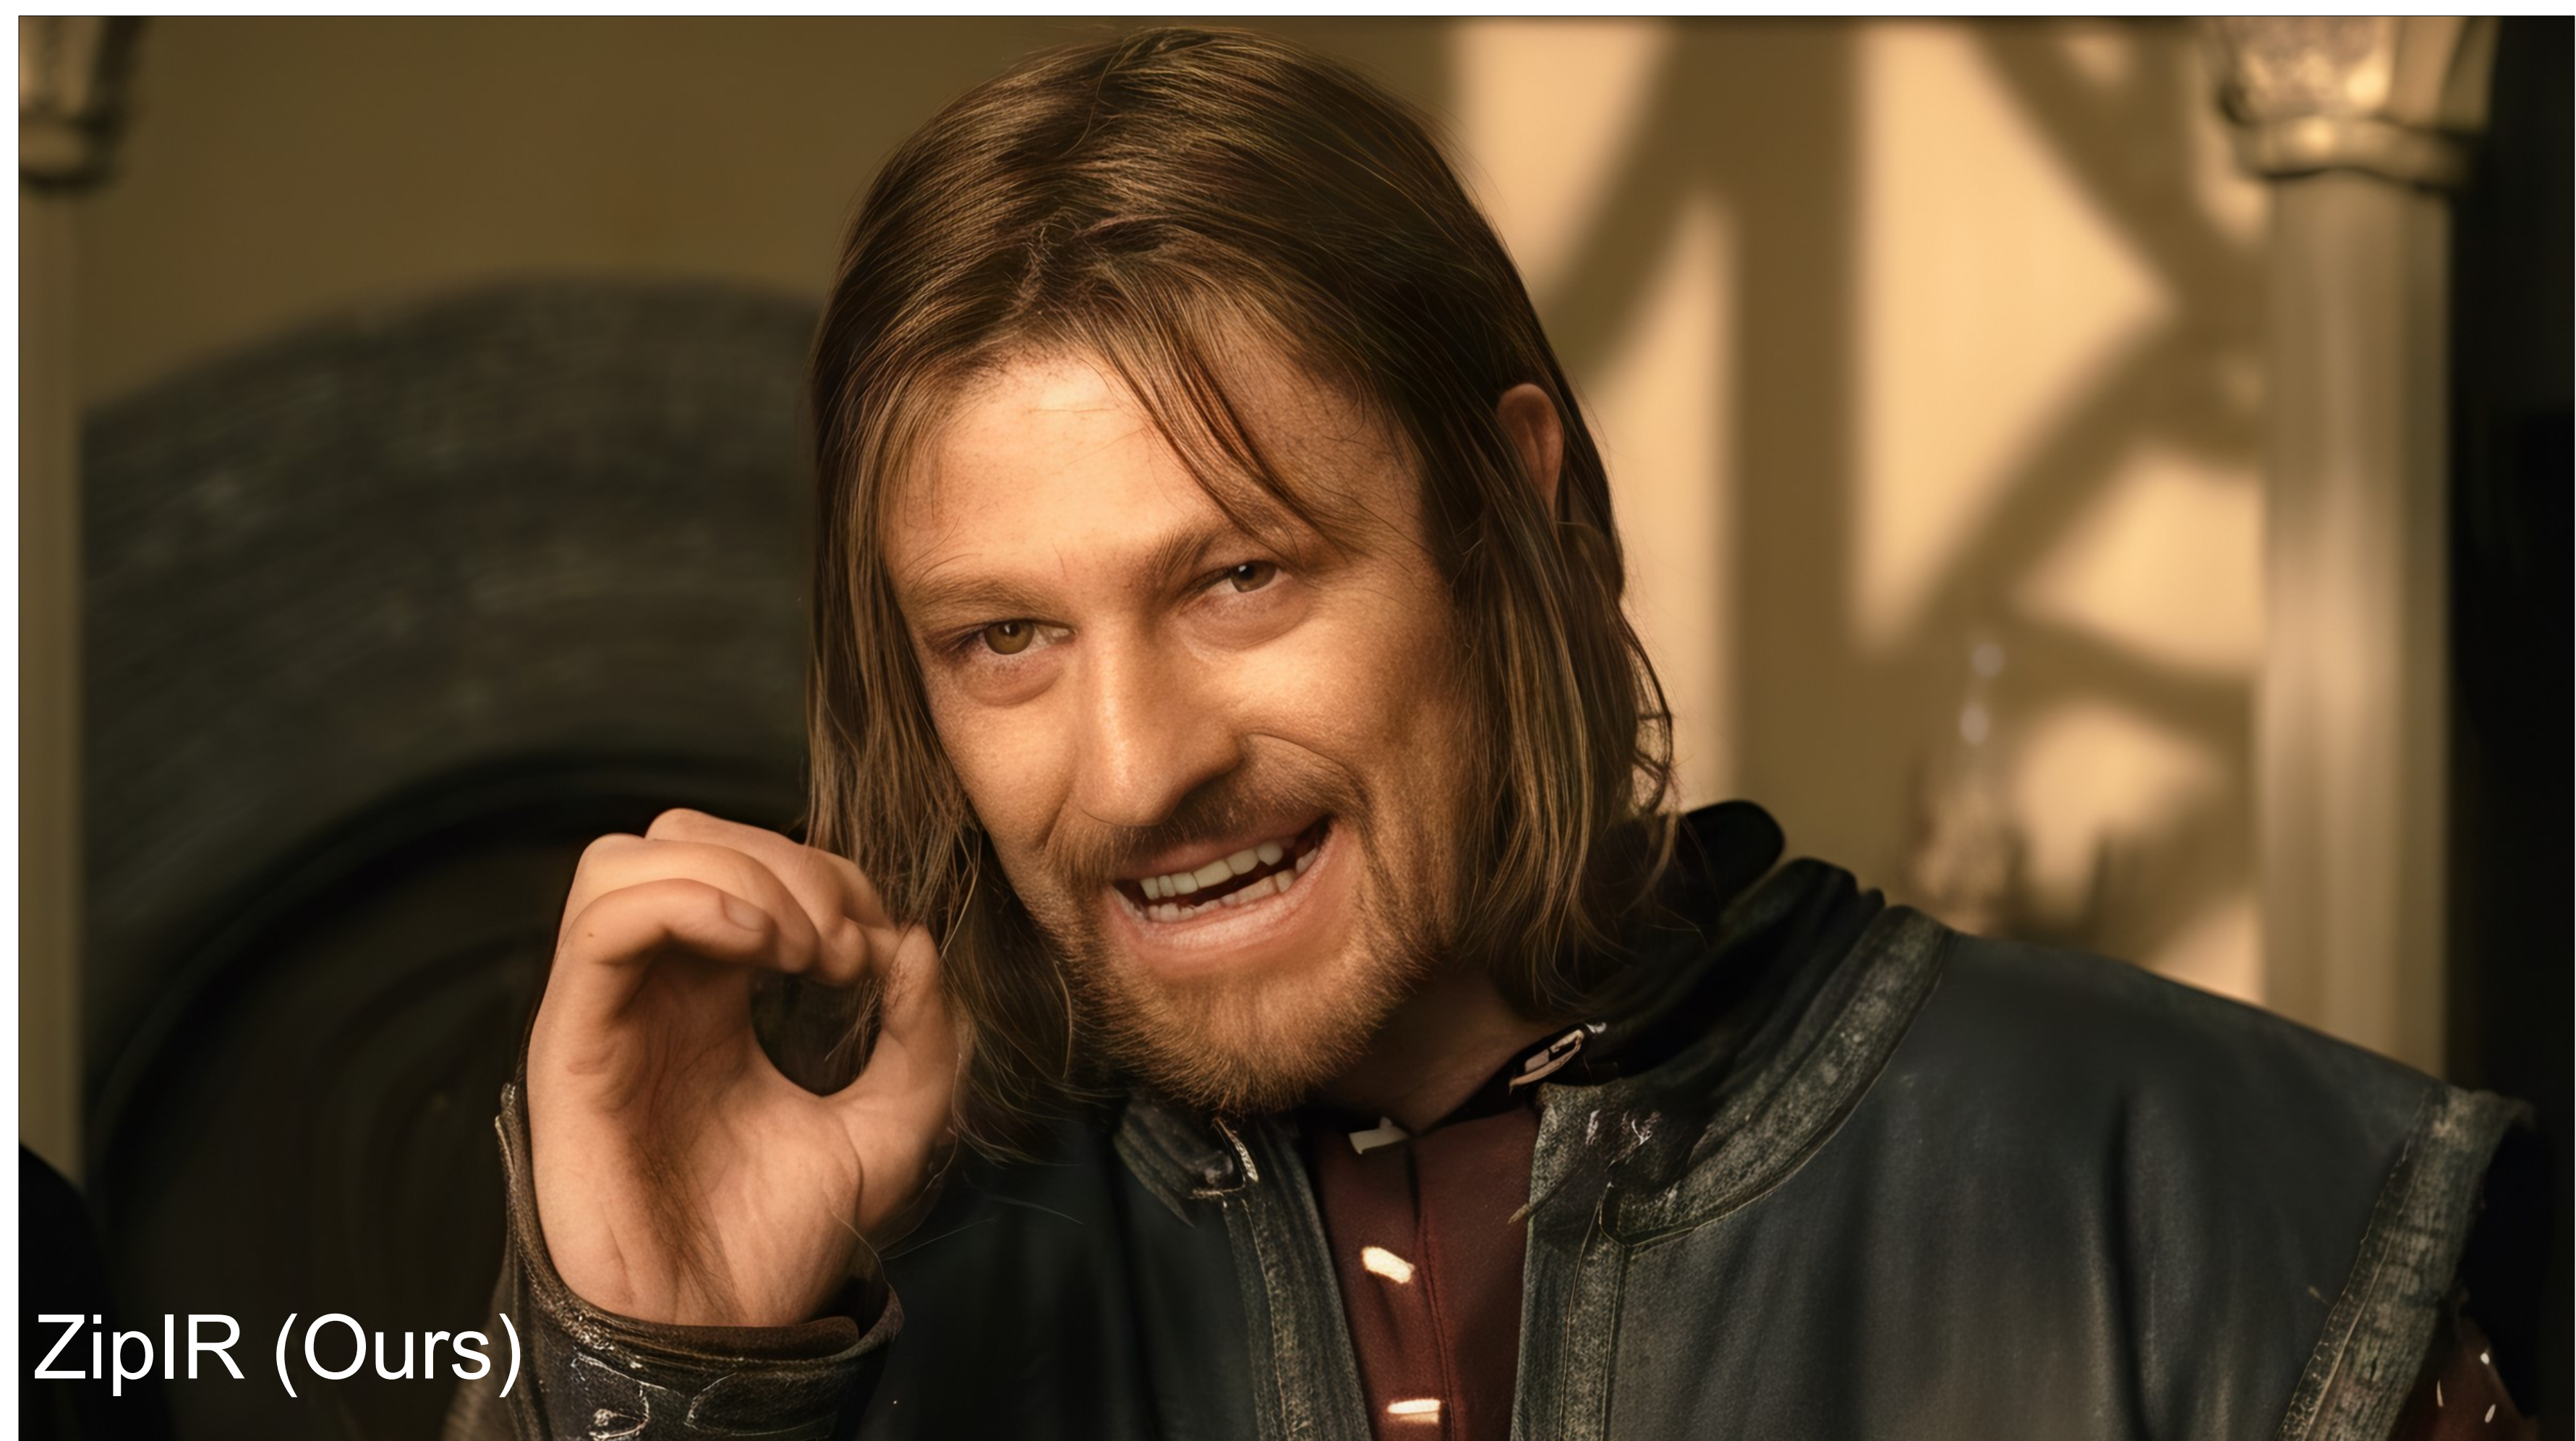

ZipIR (Ours)

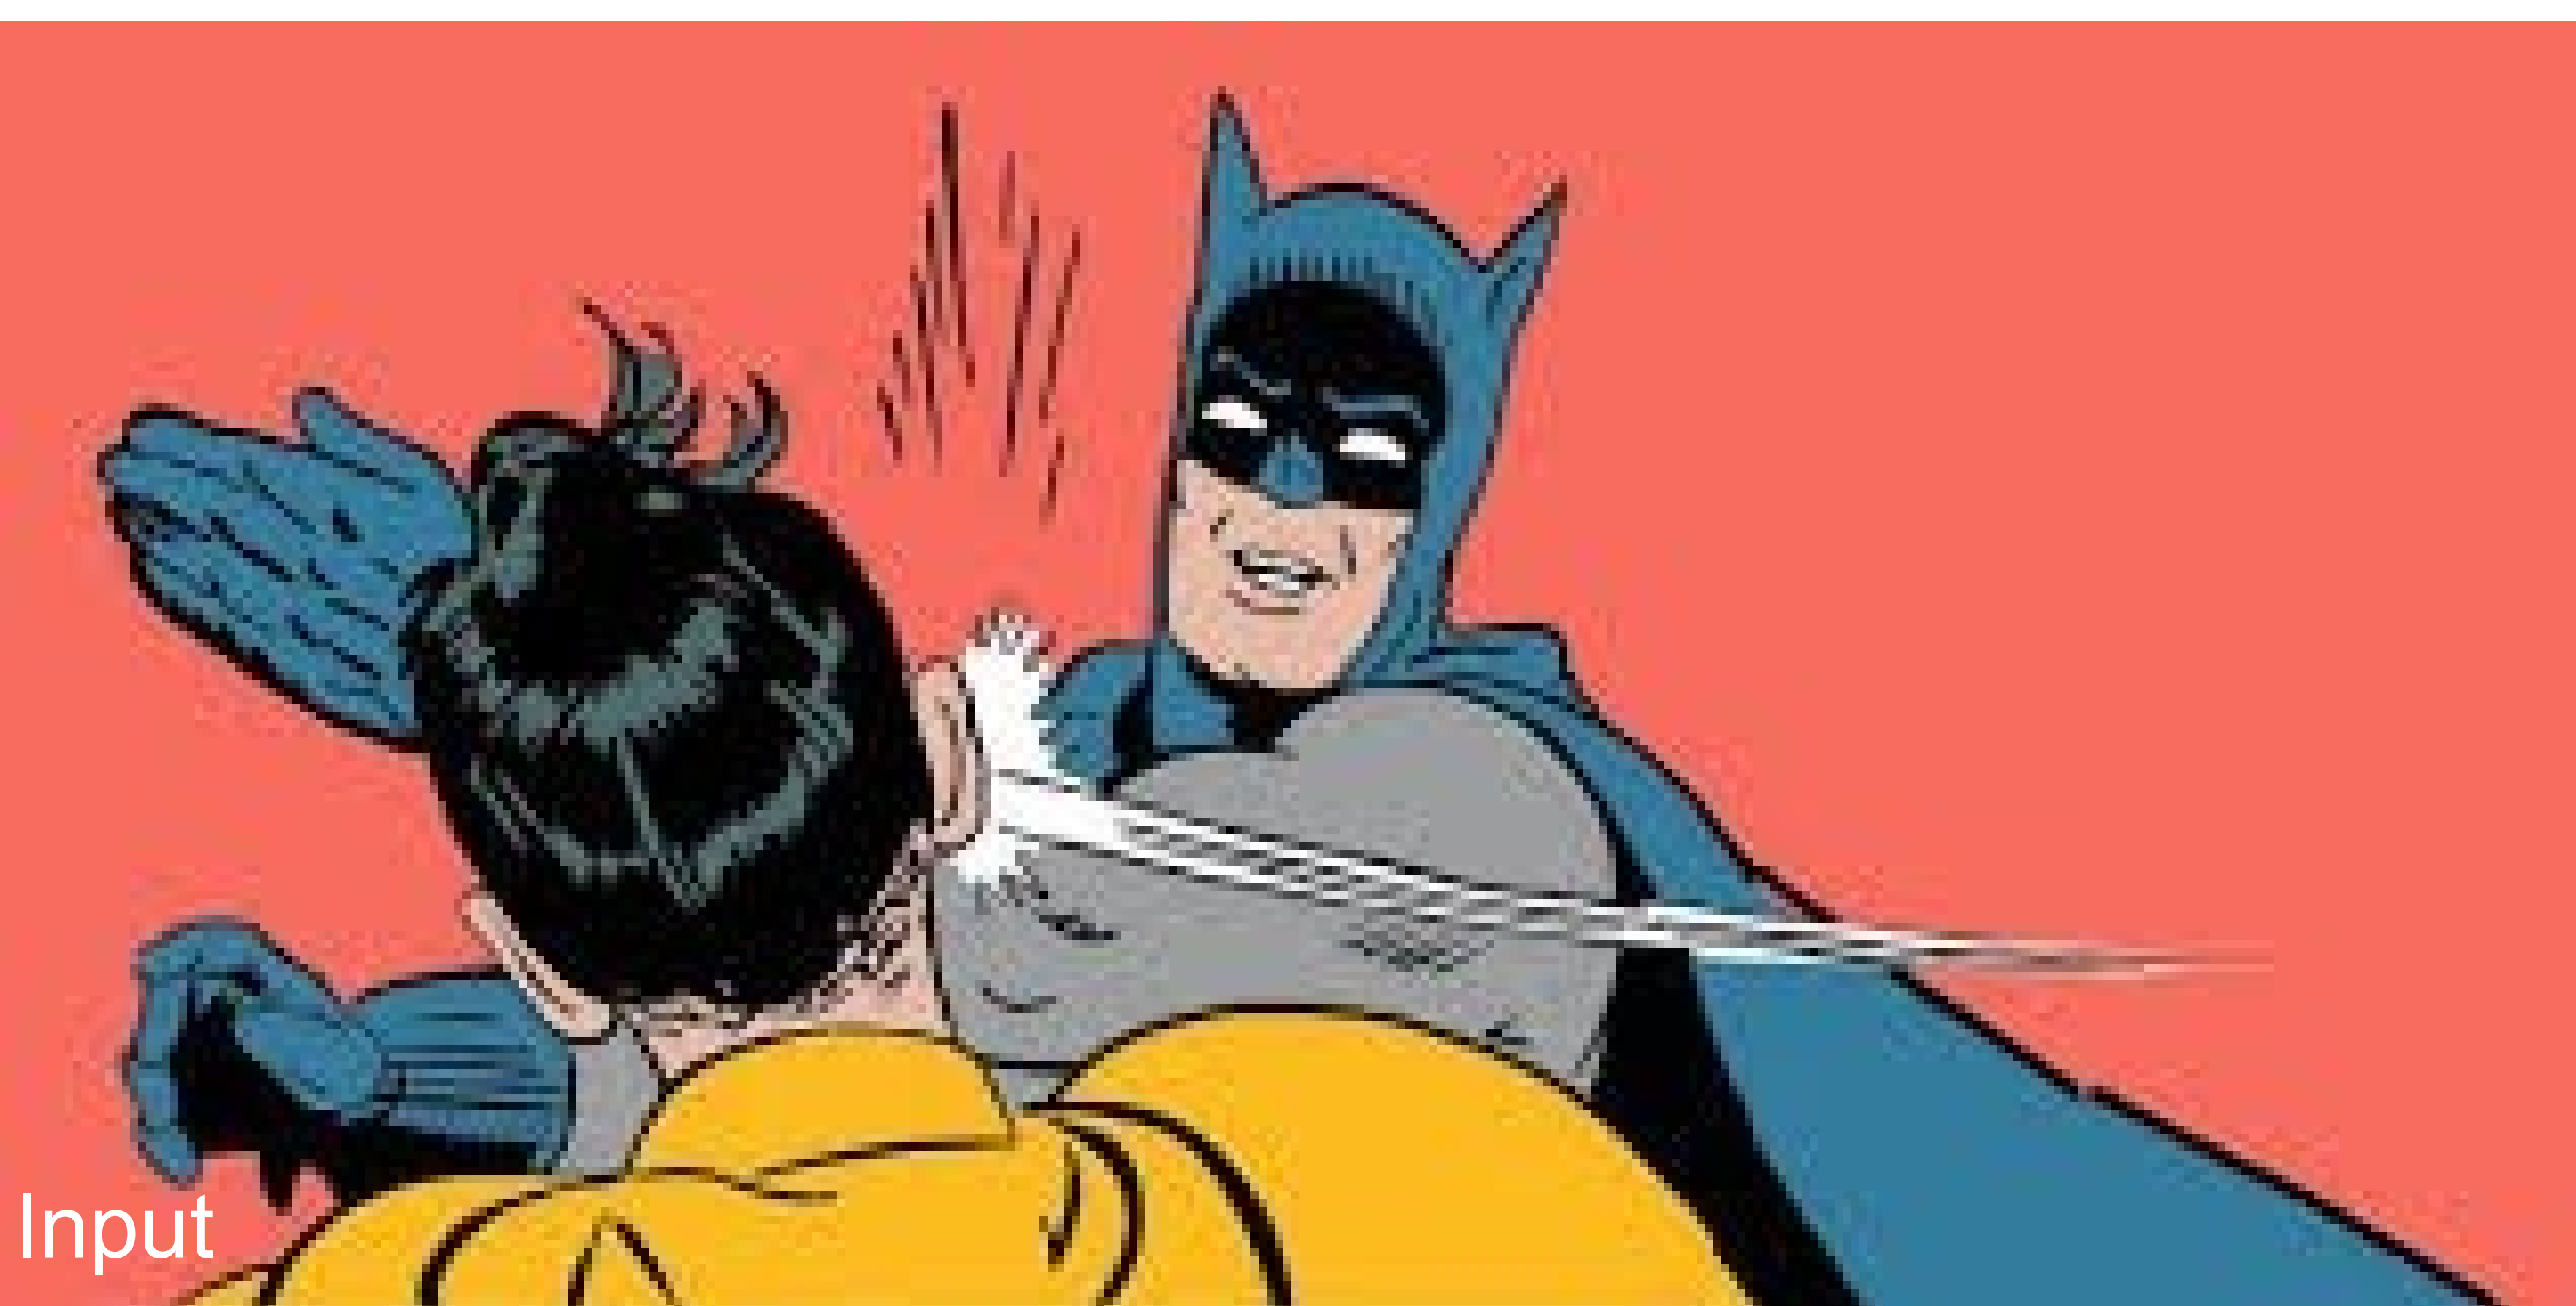

Input

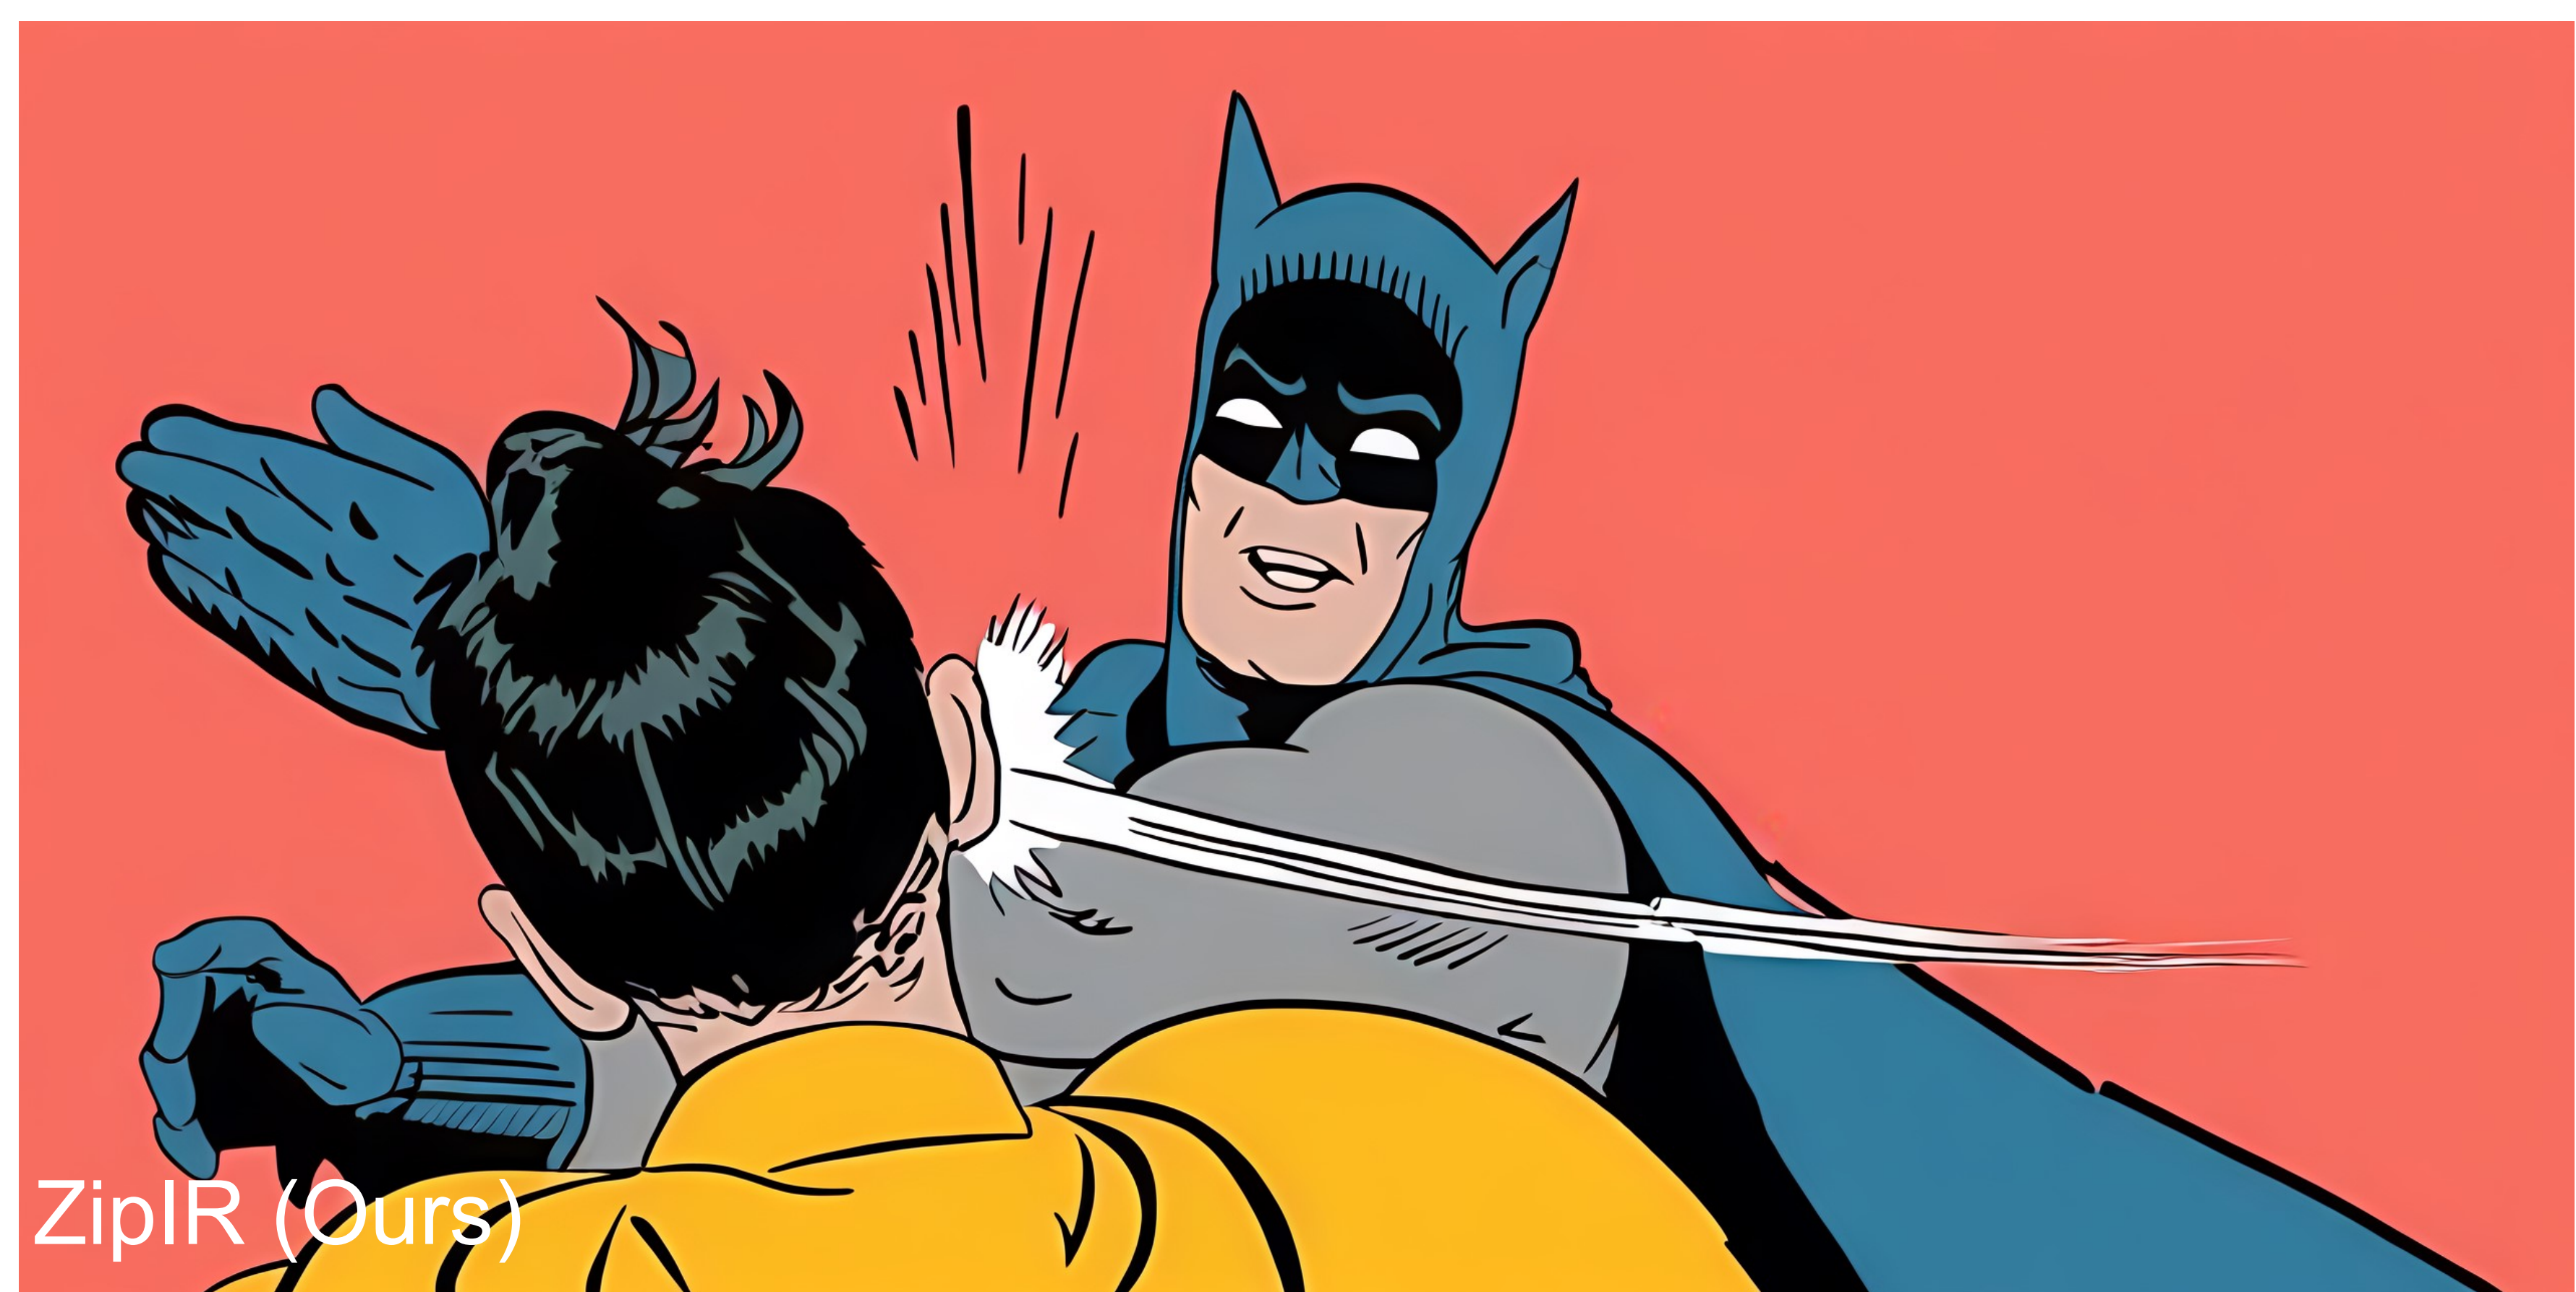

ZipIR (Ours)

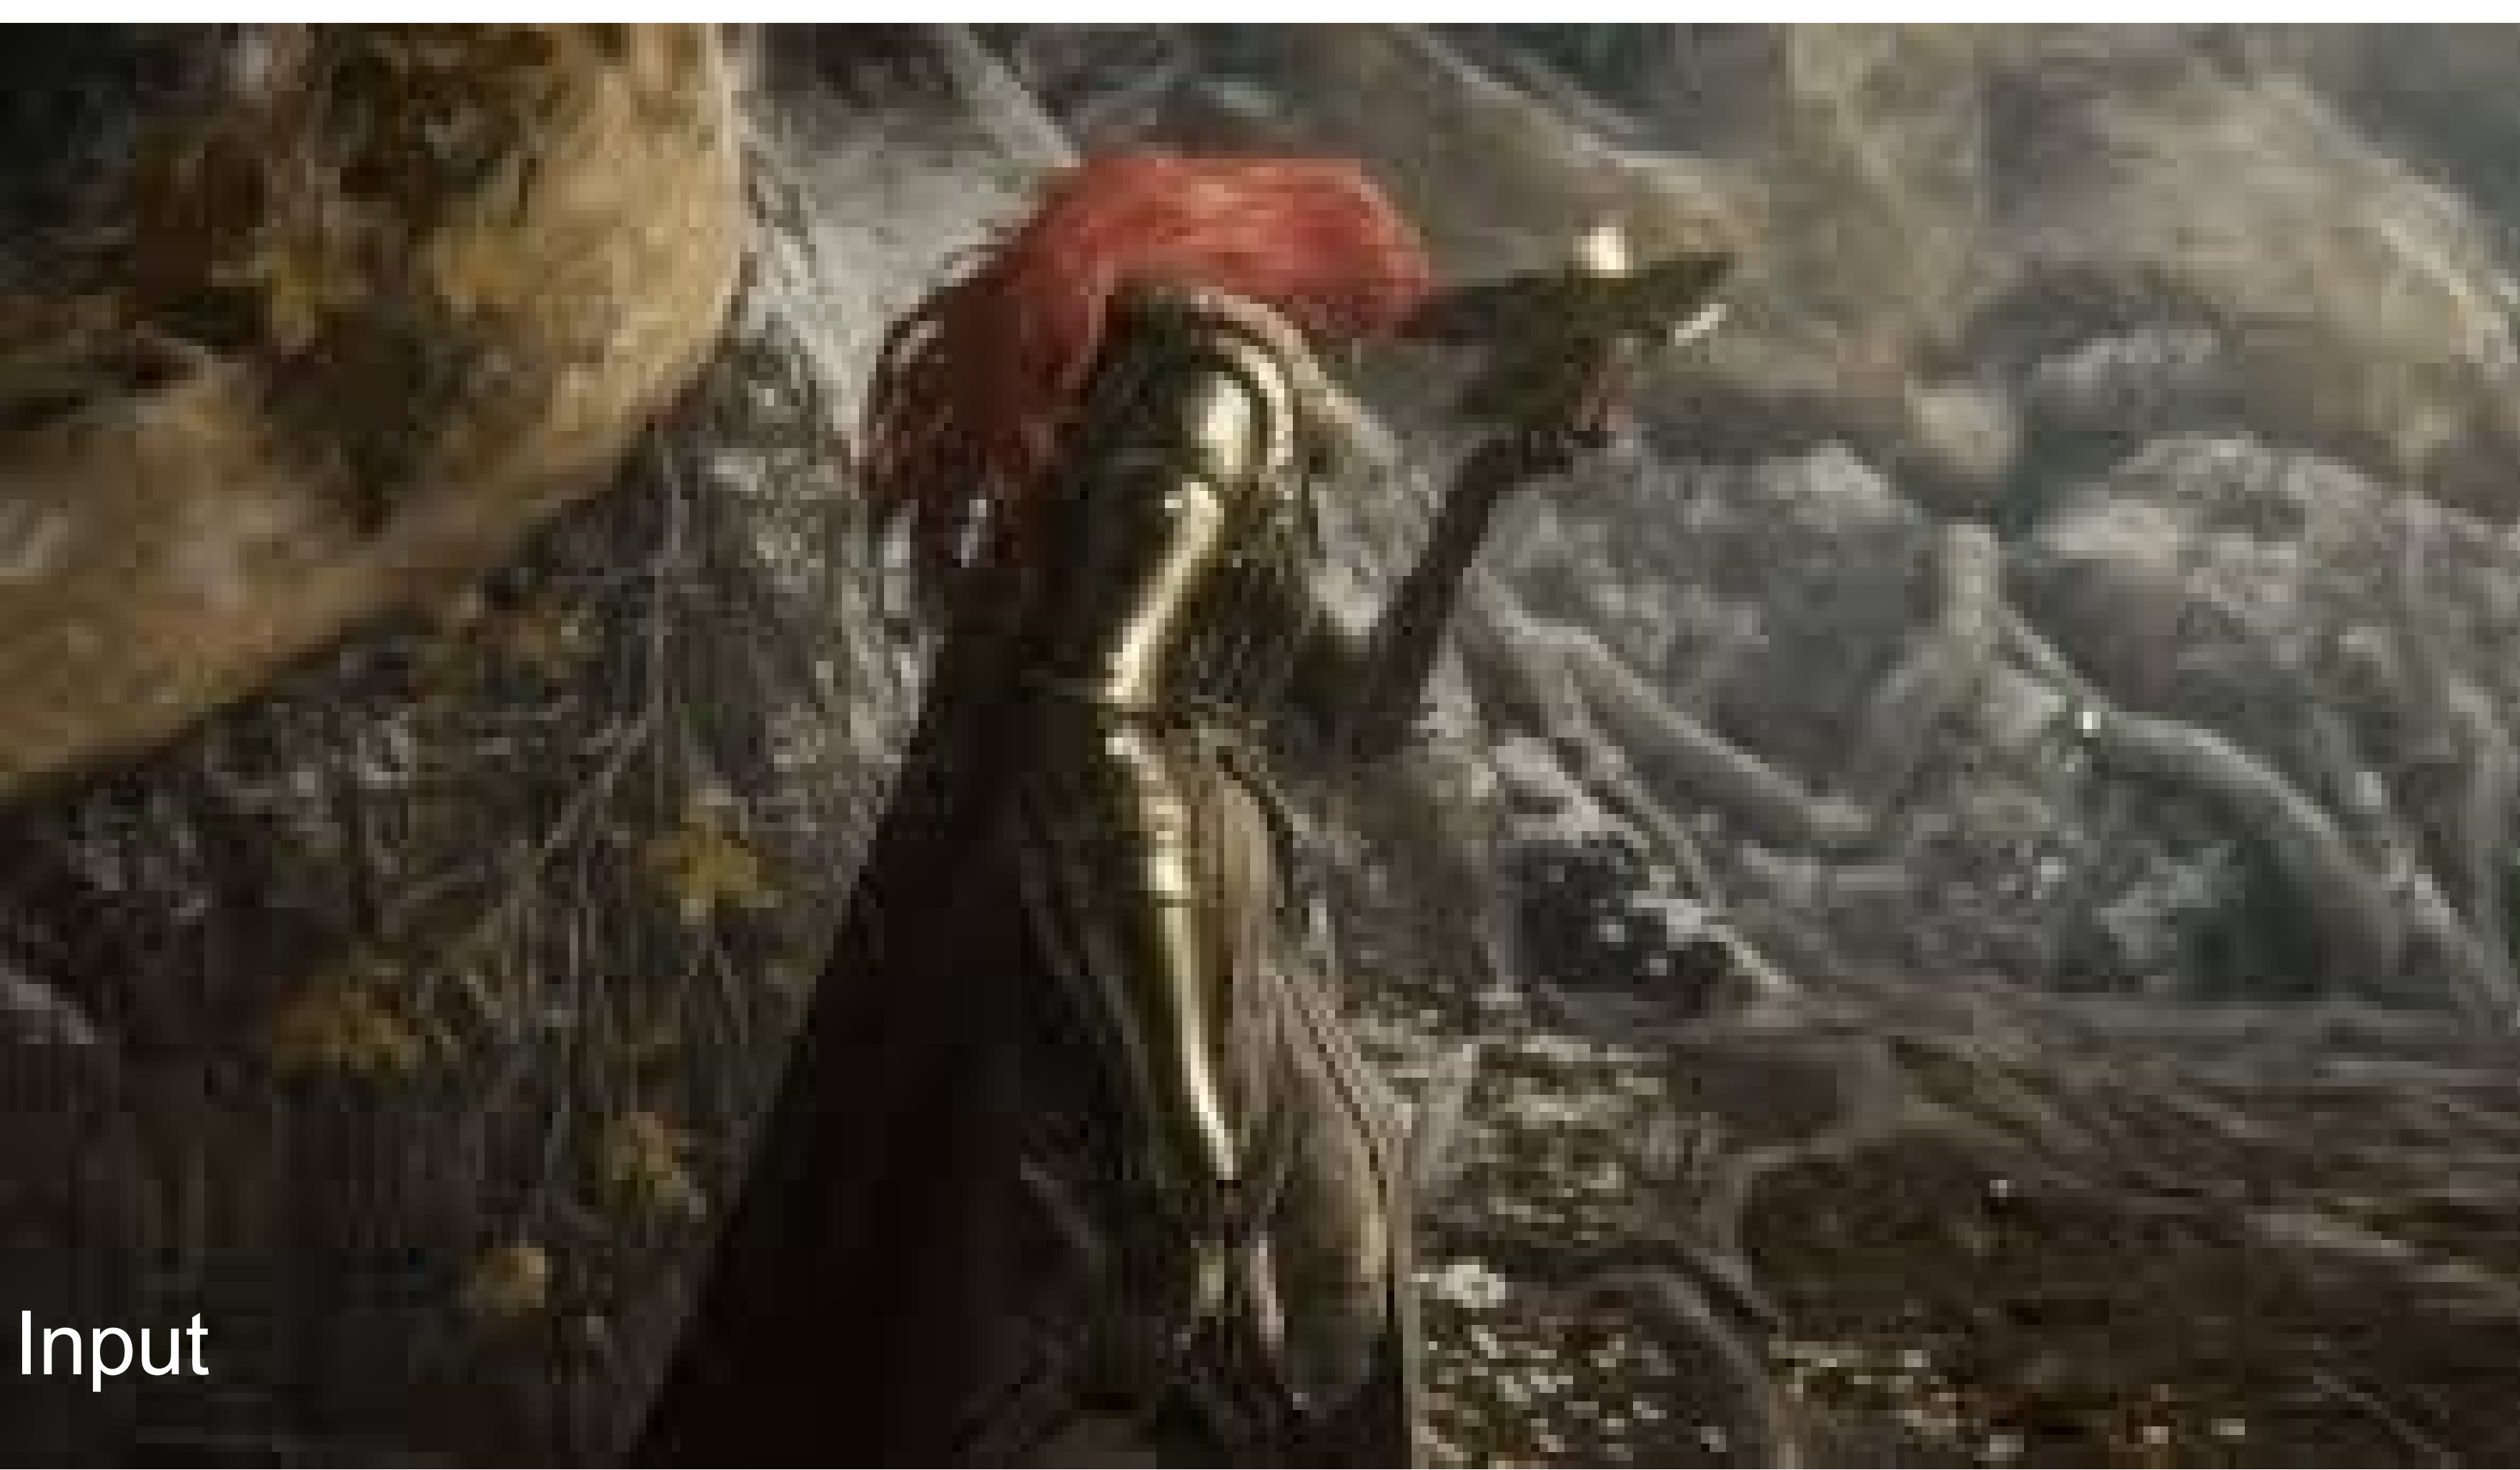

Input

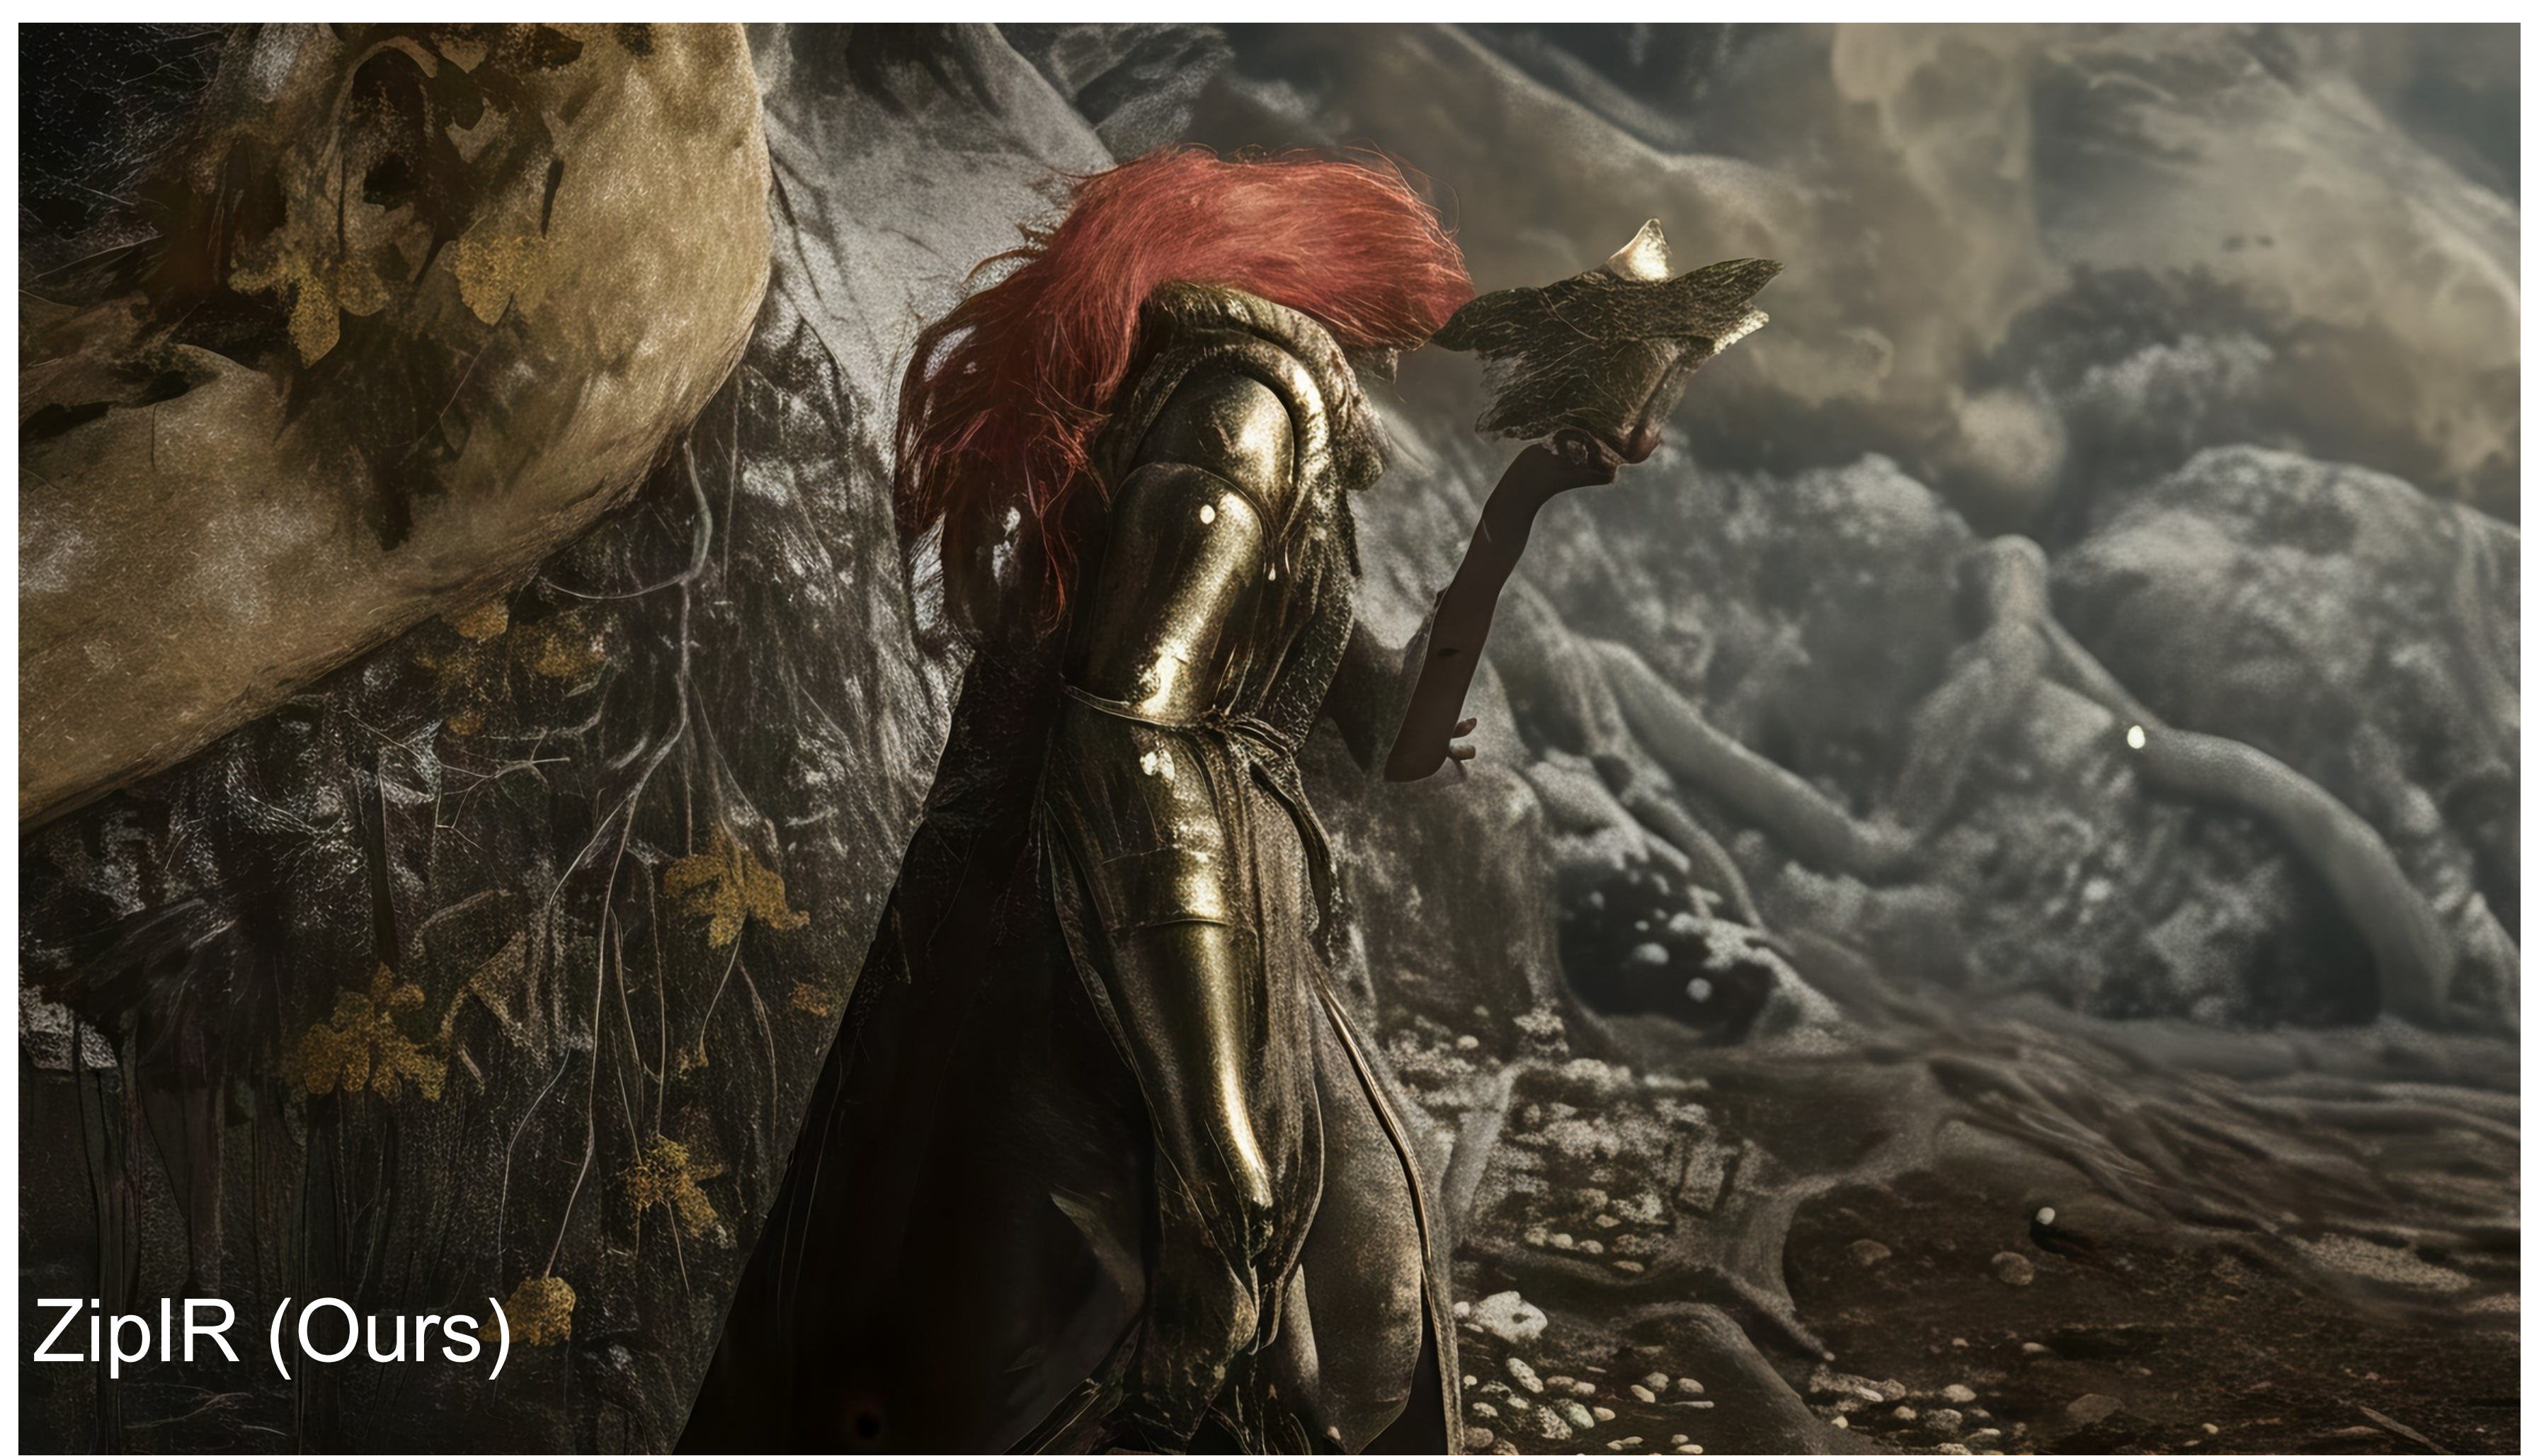

ZipIR (Ours)



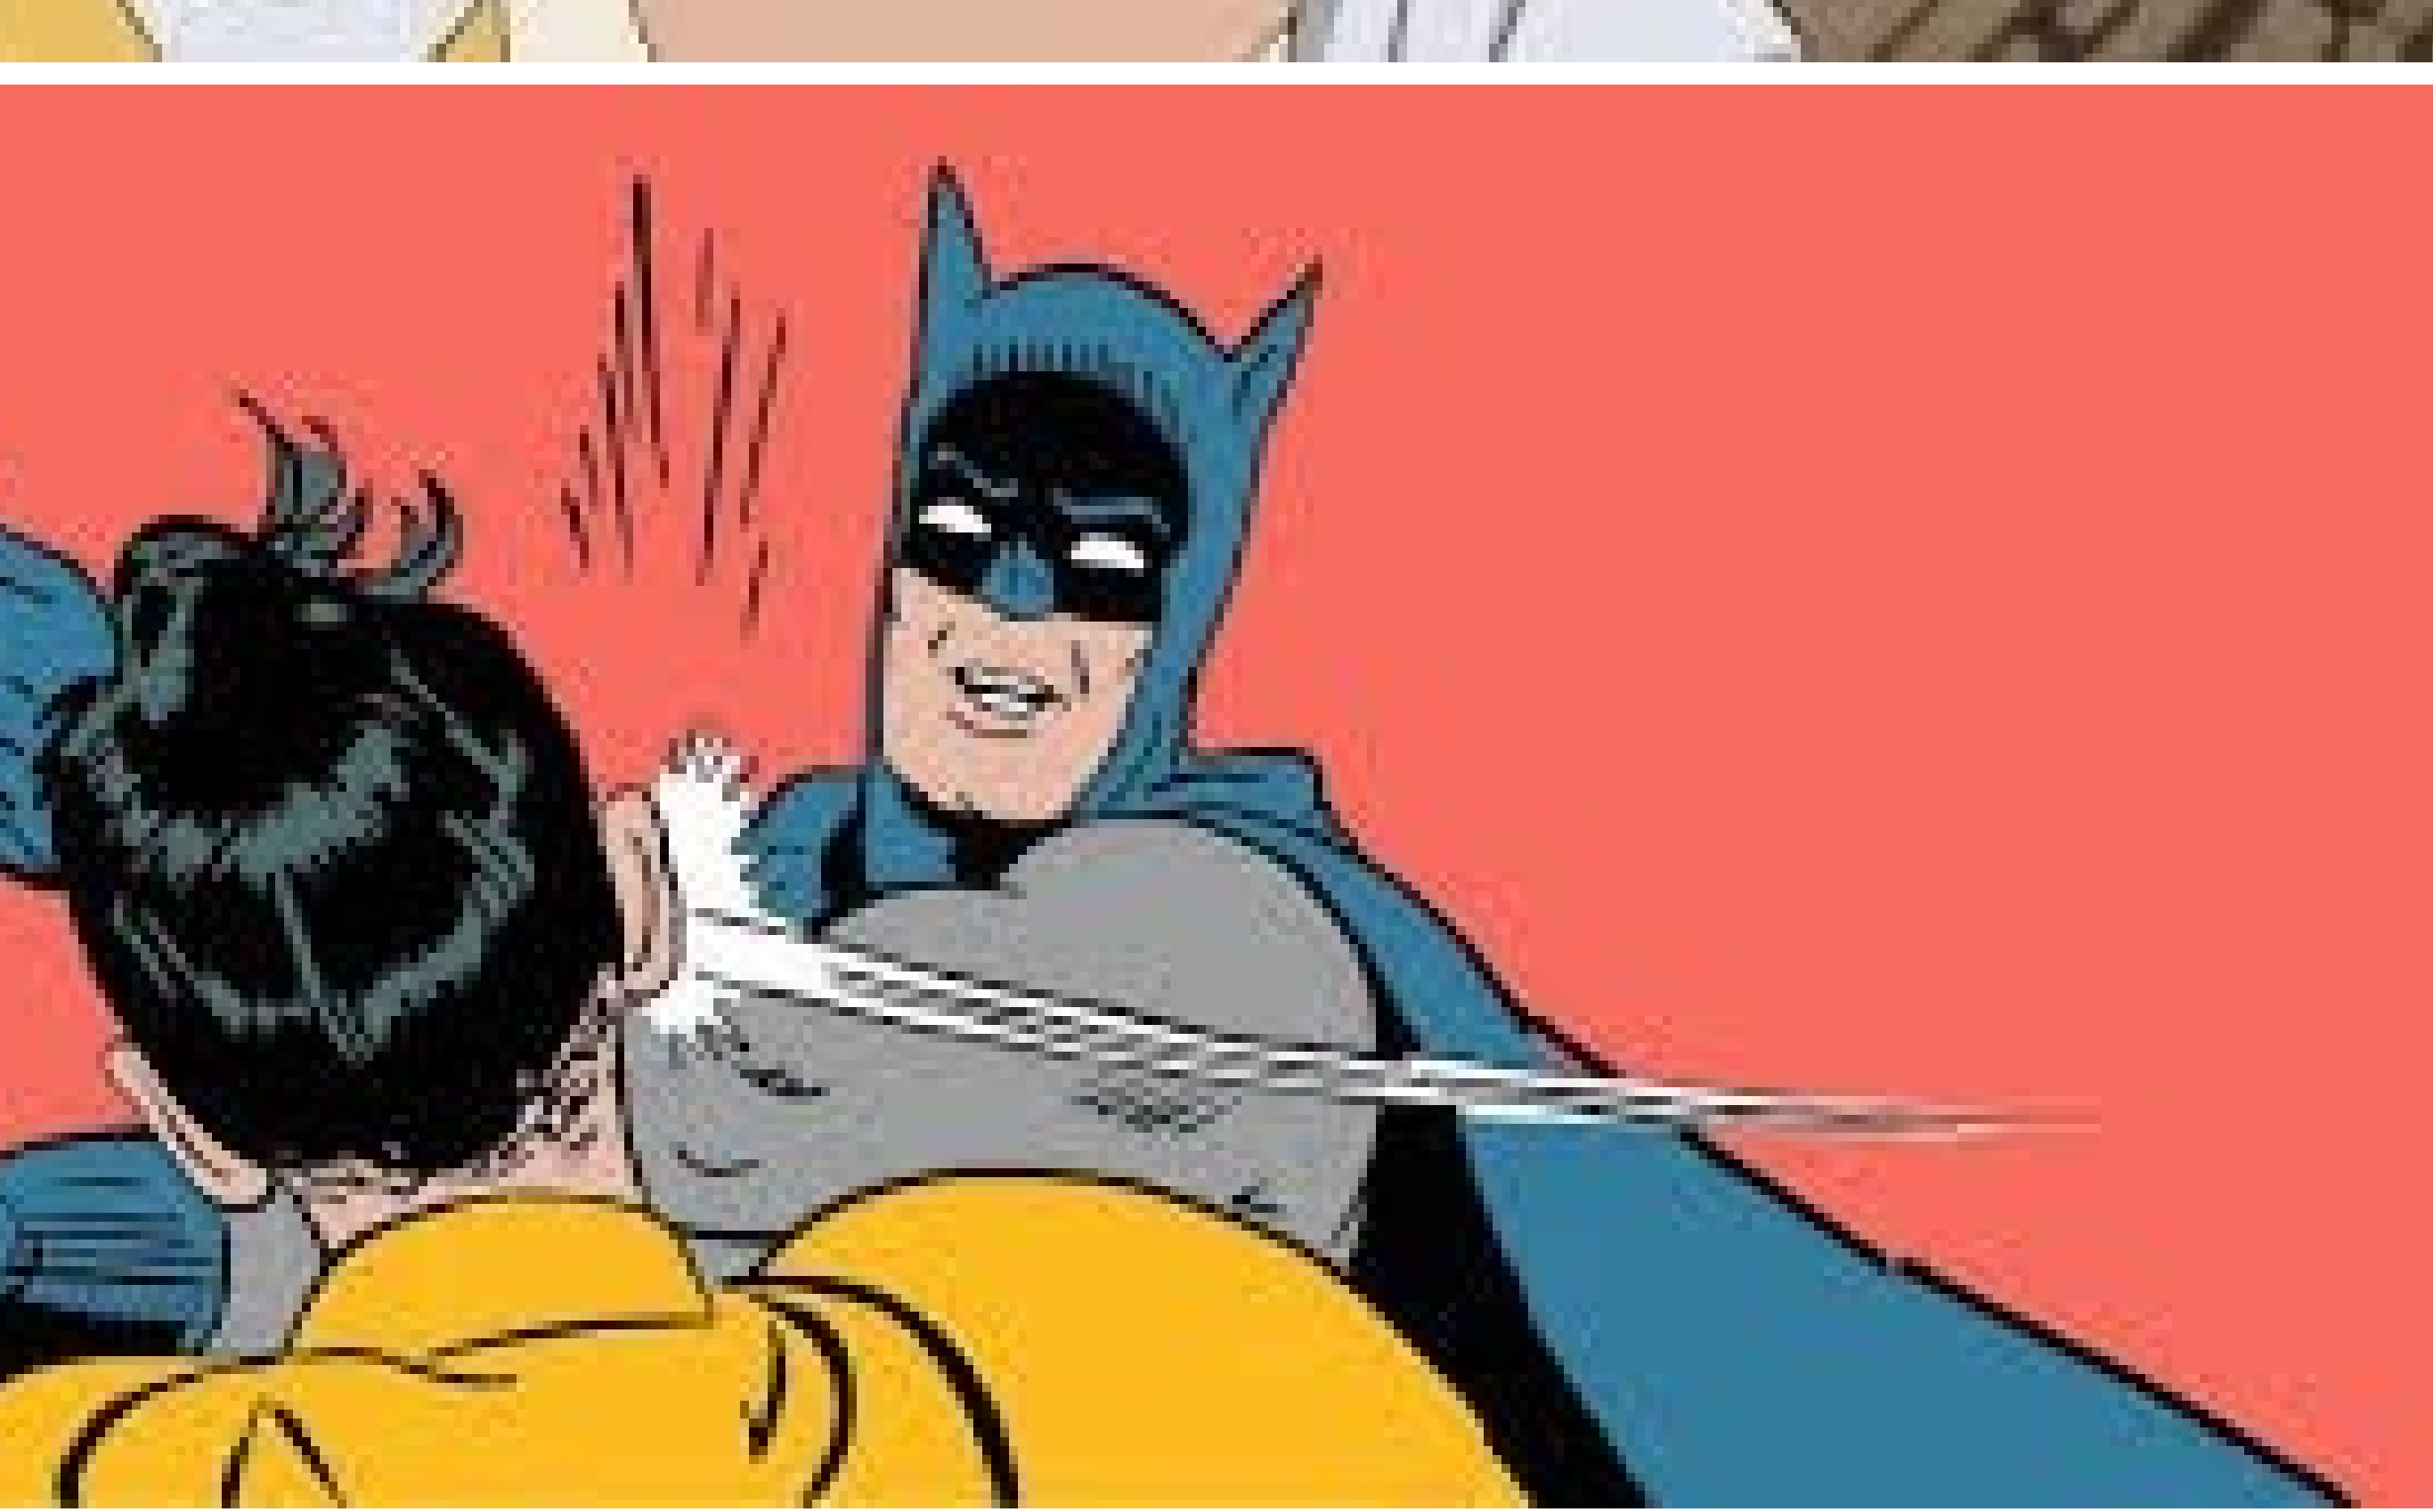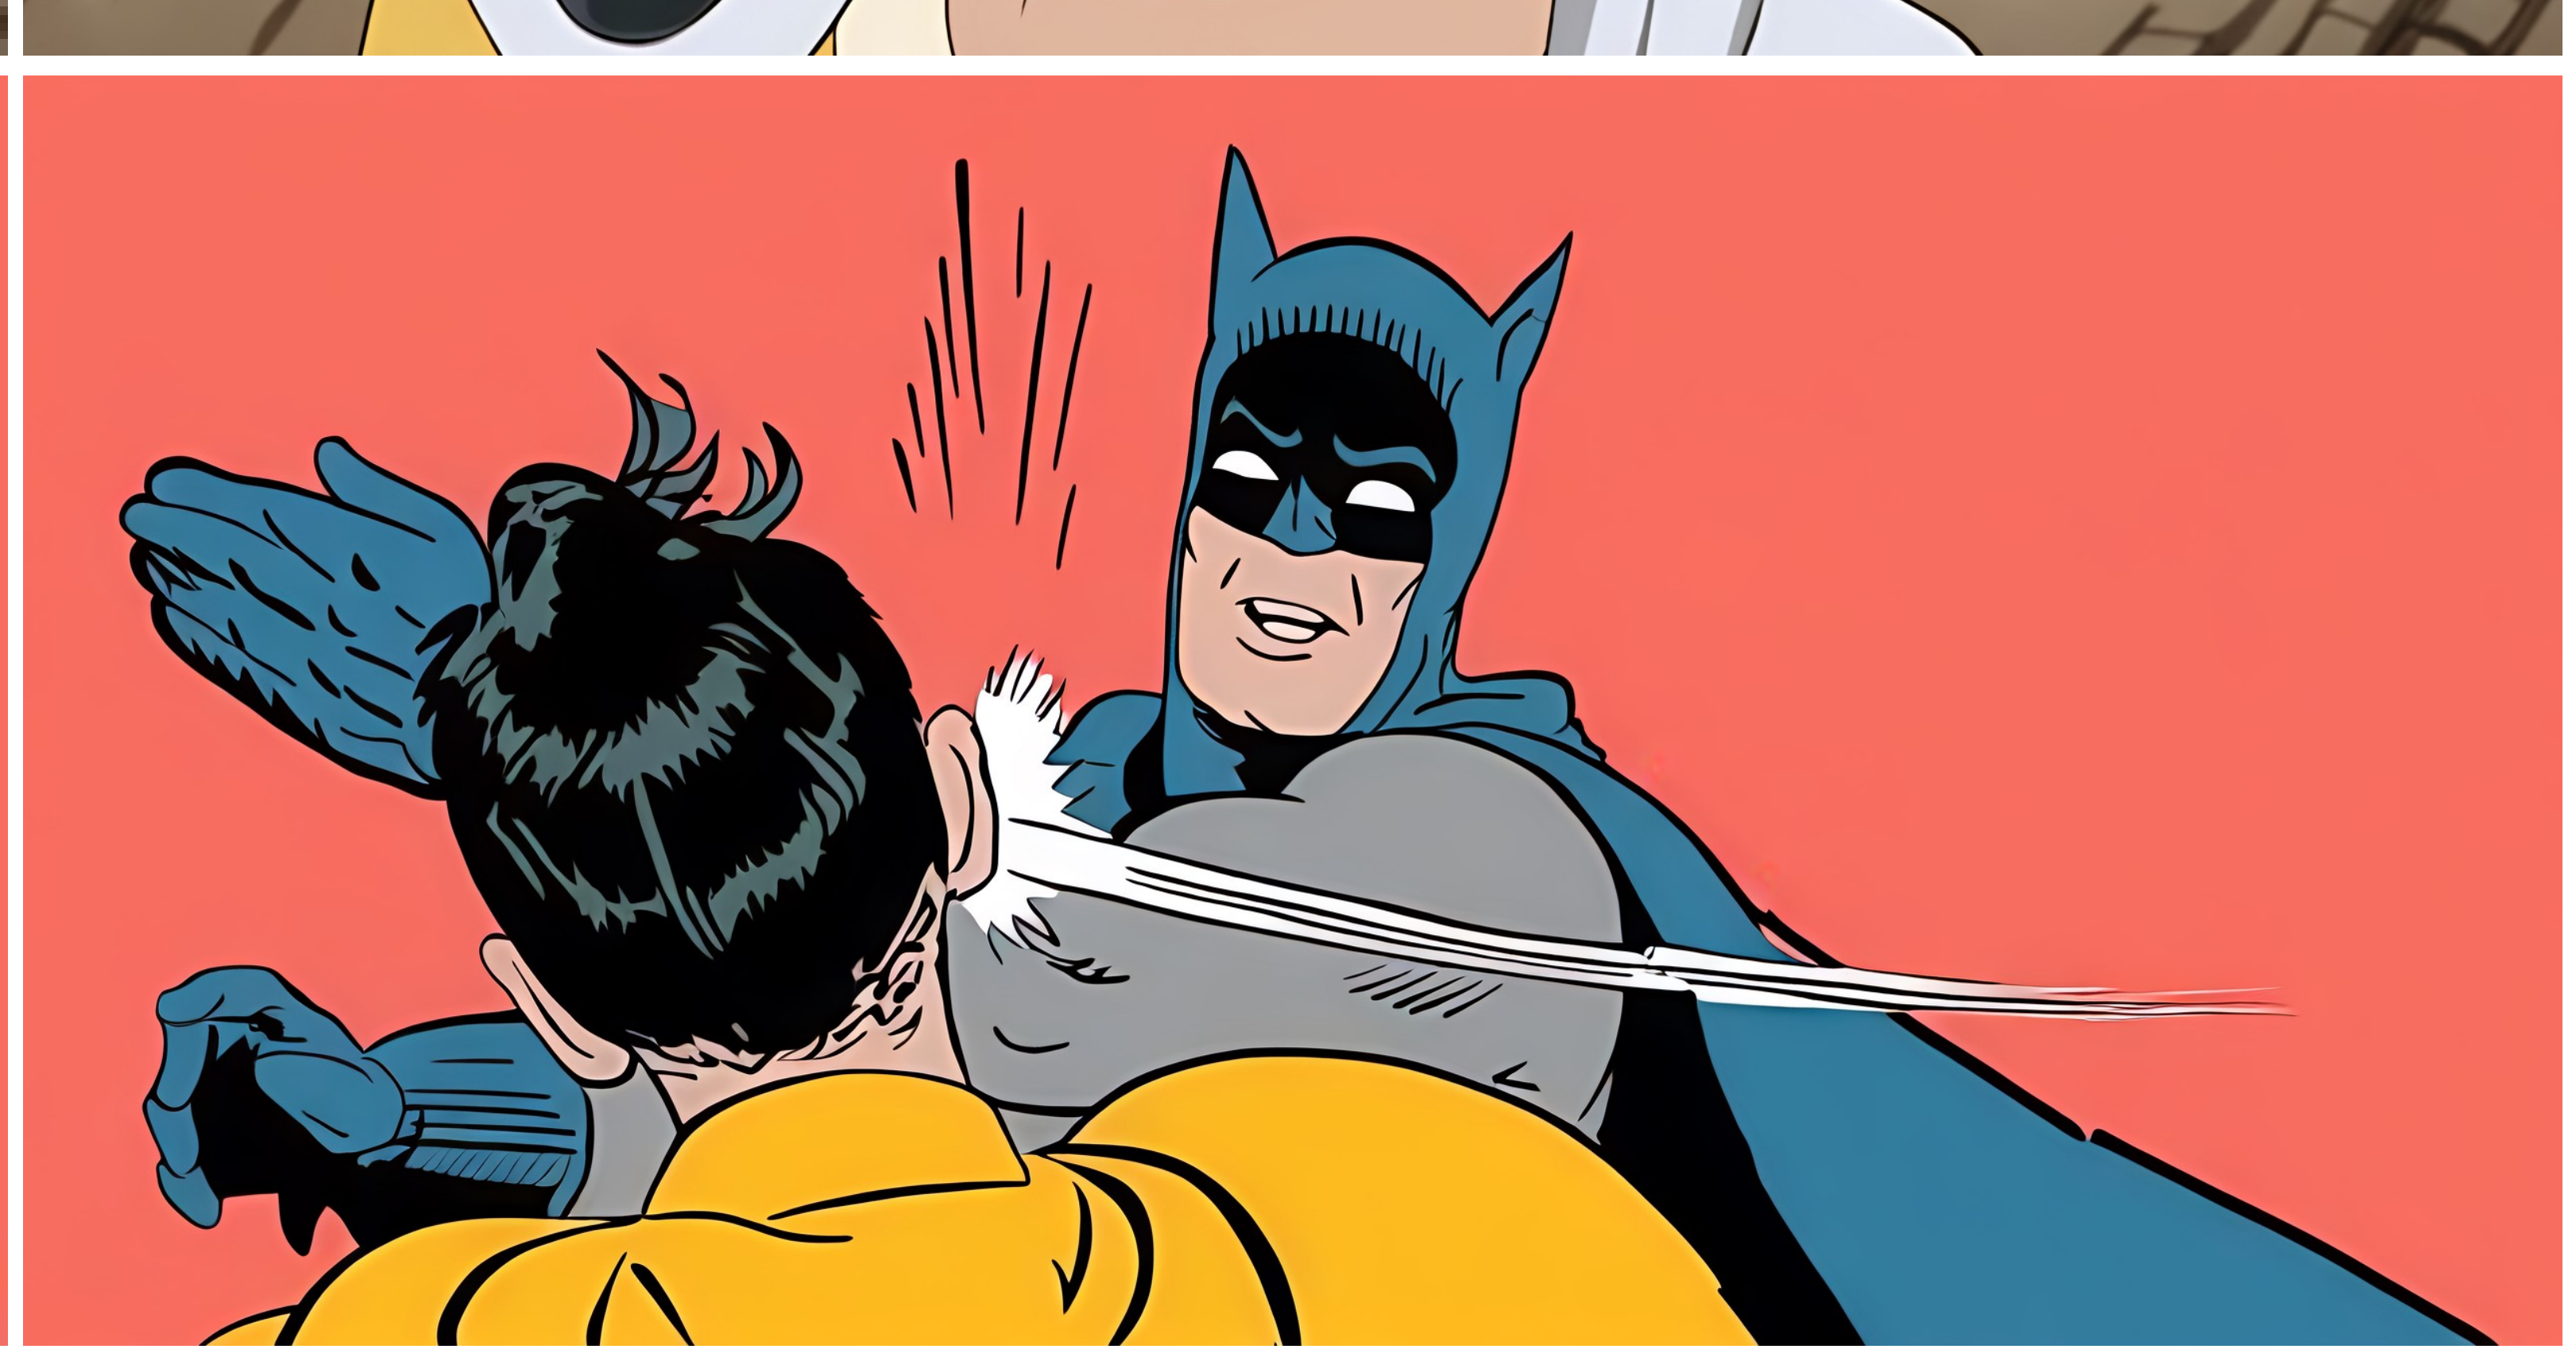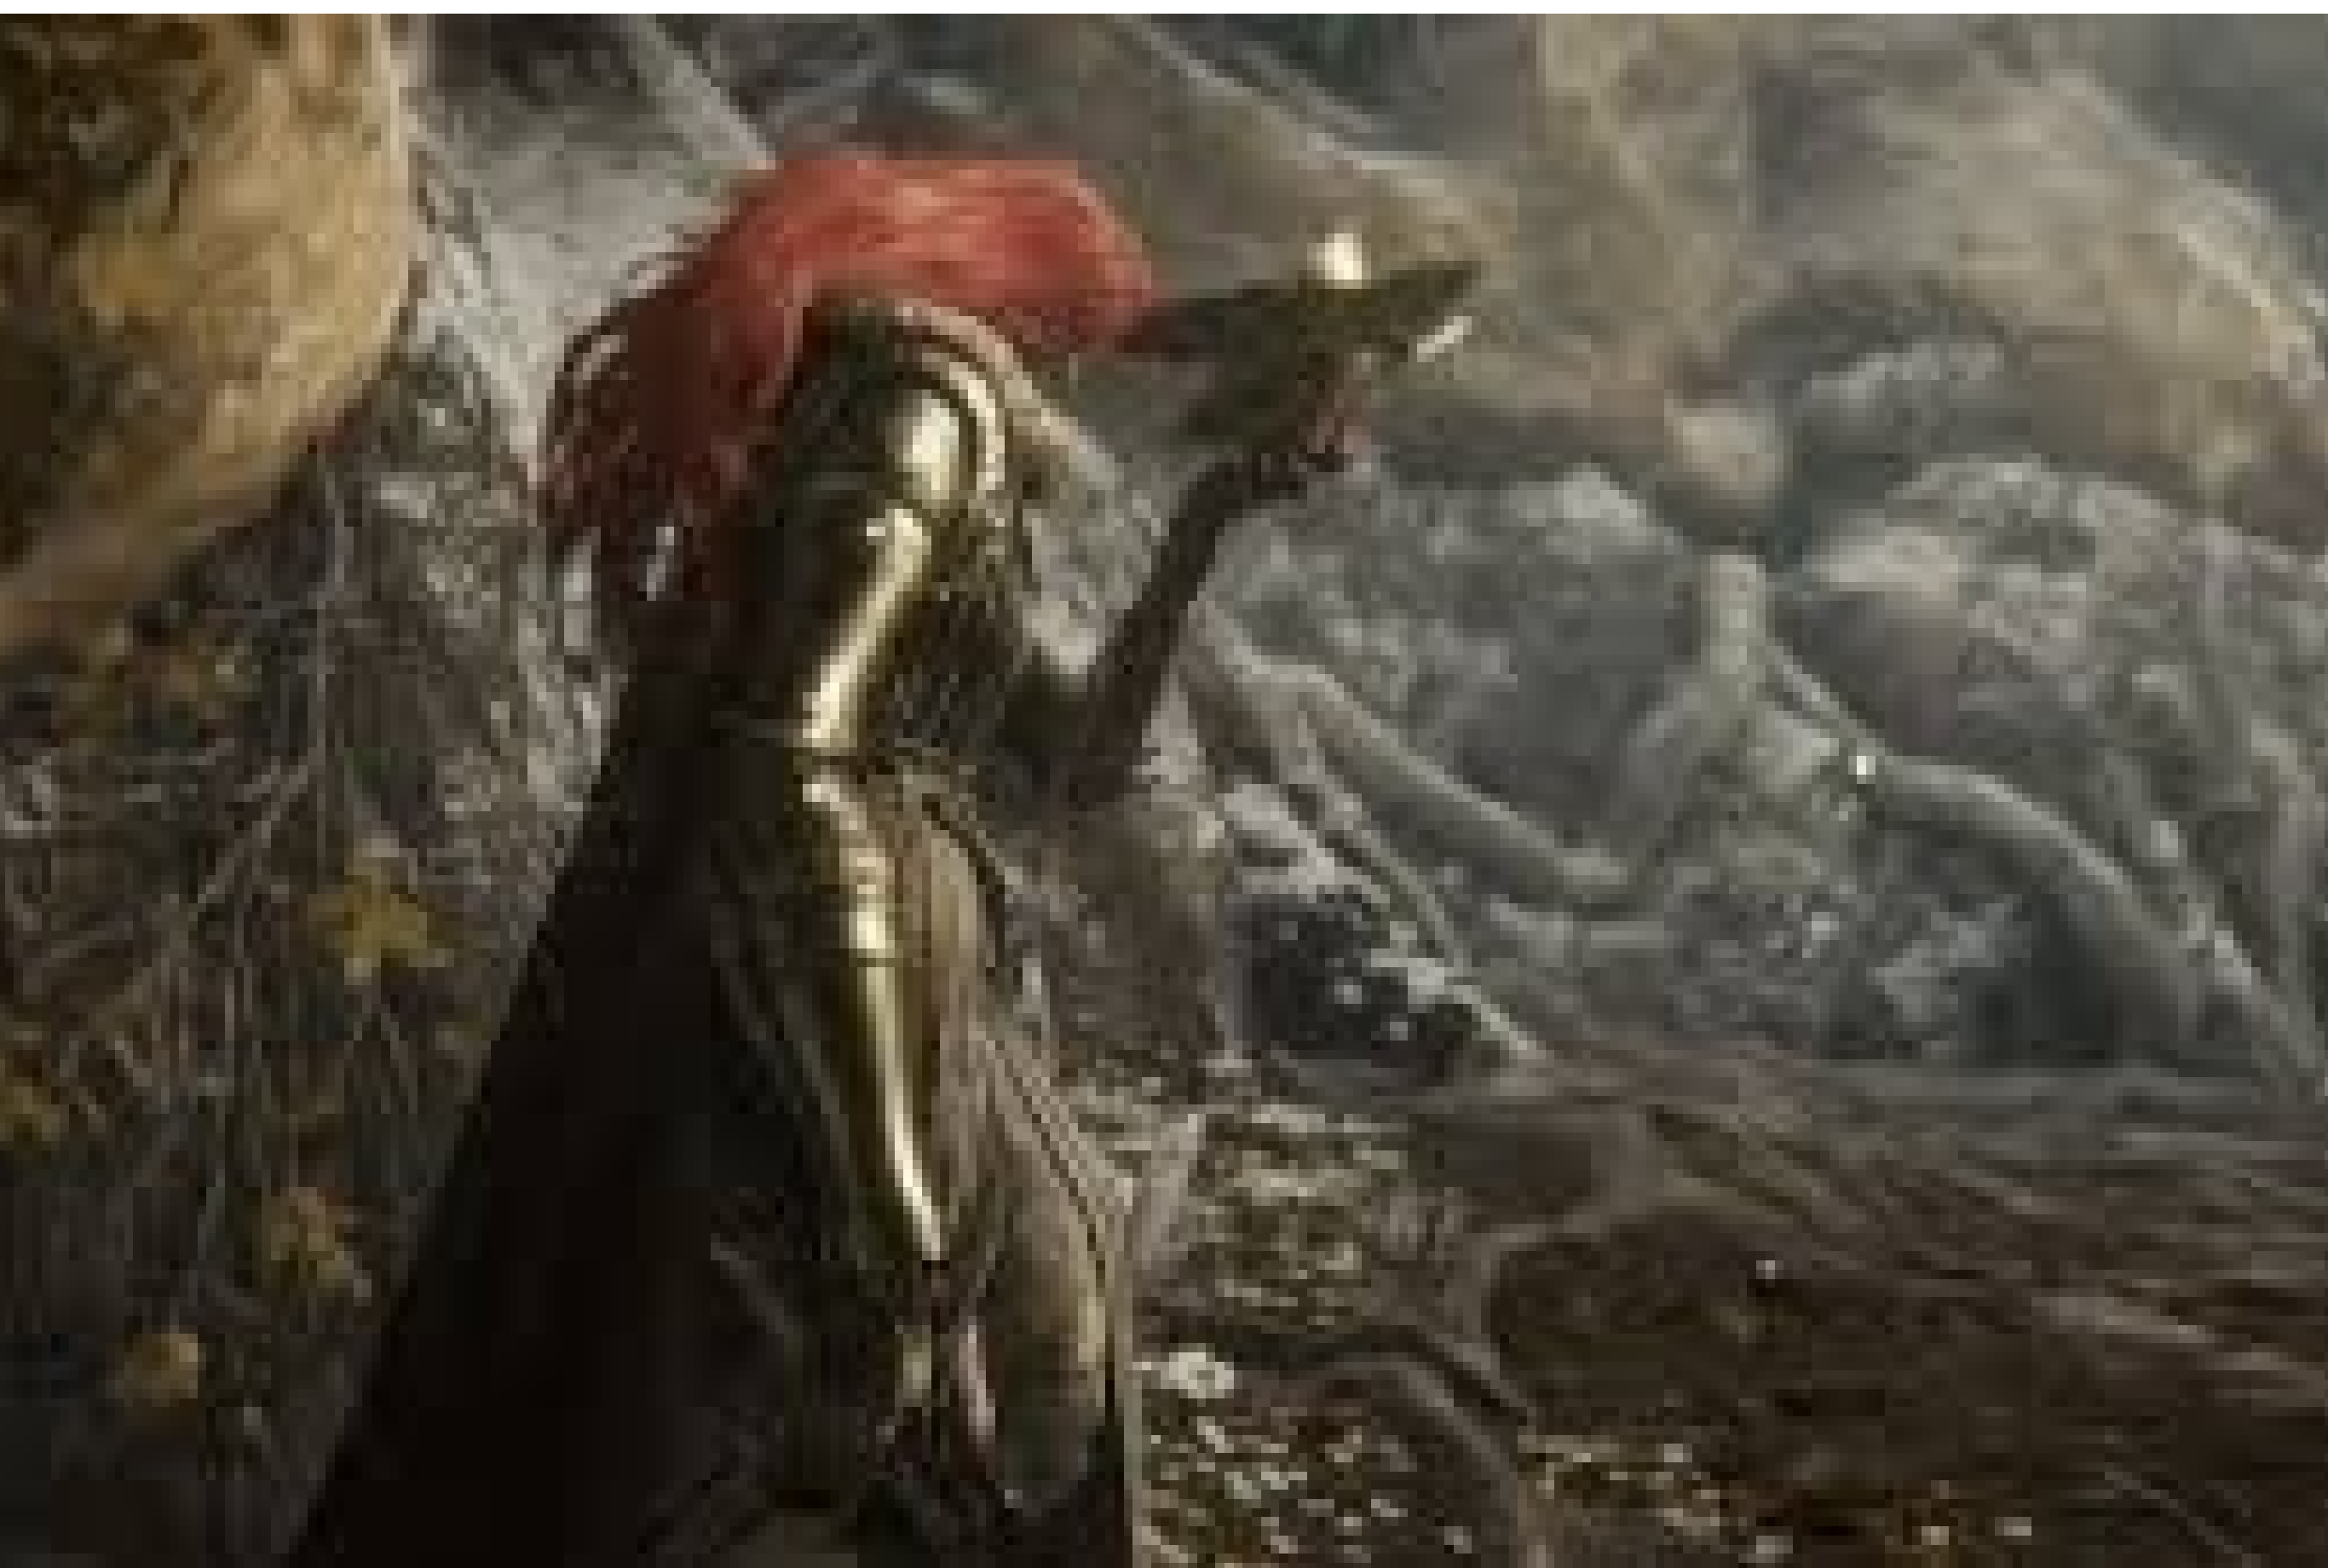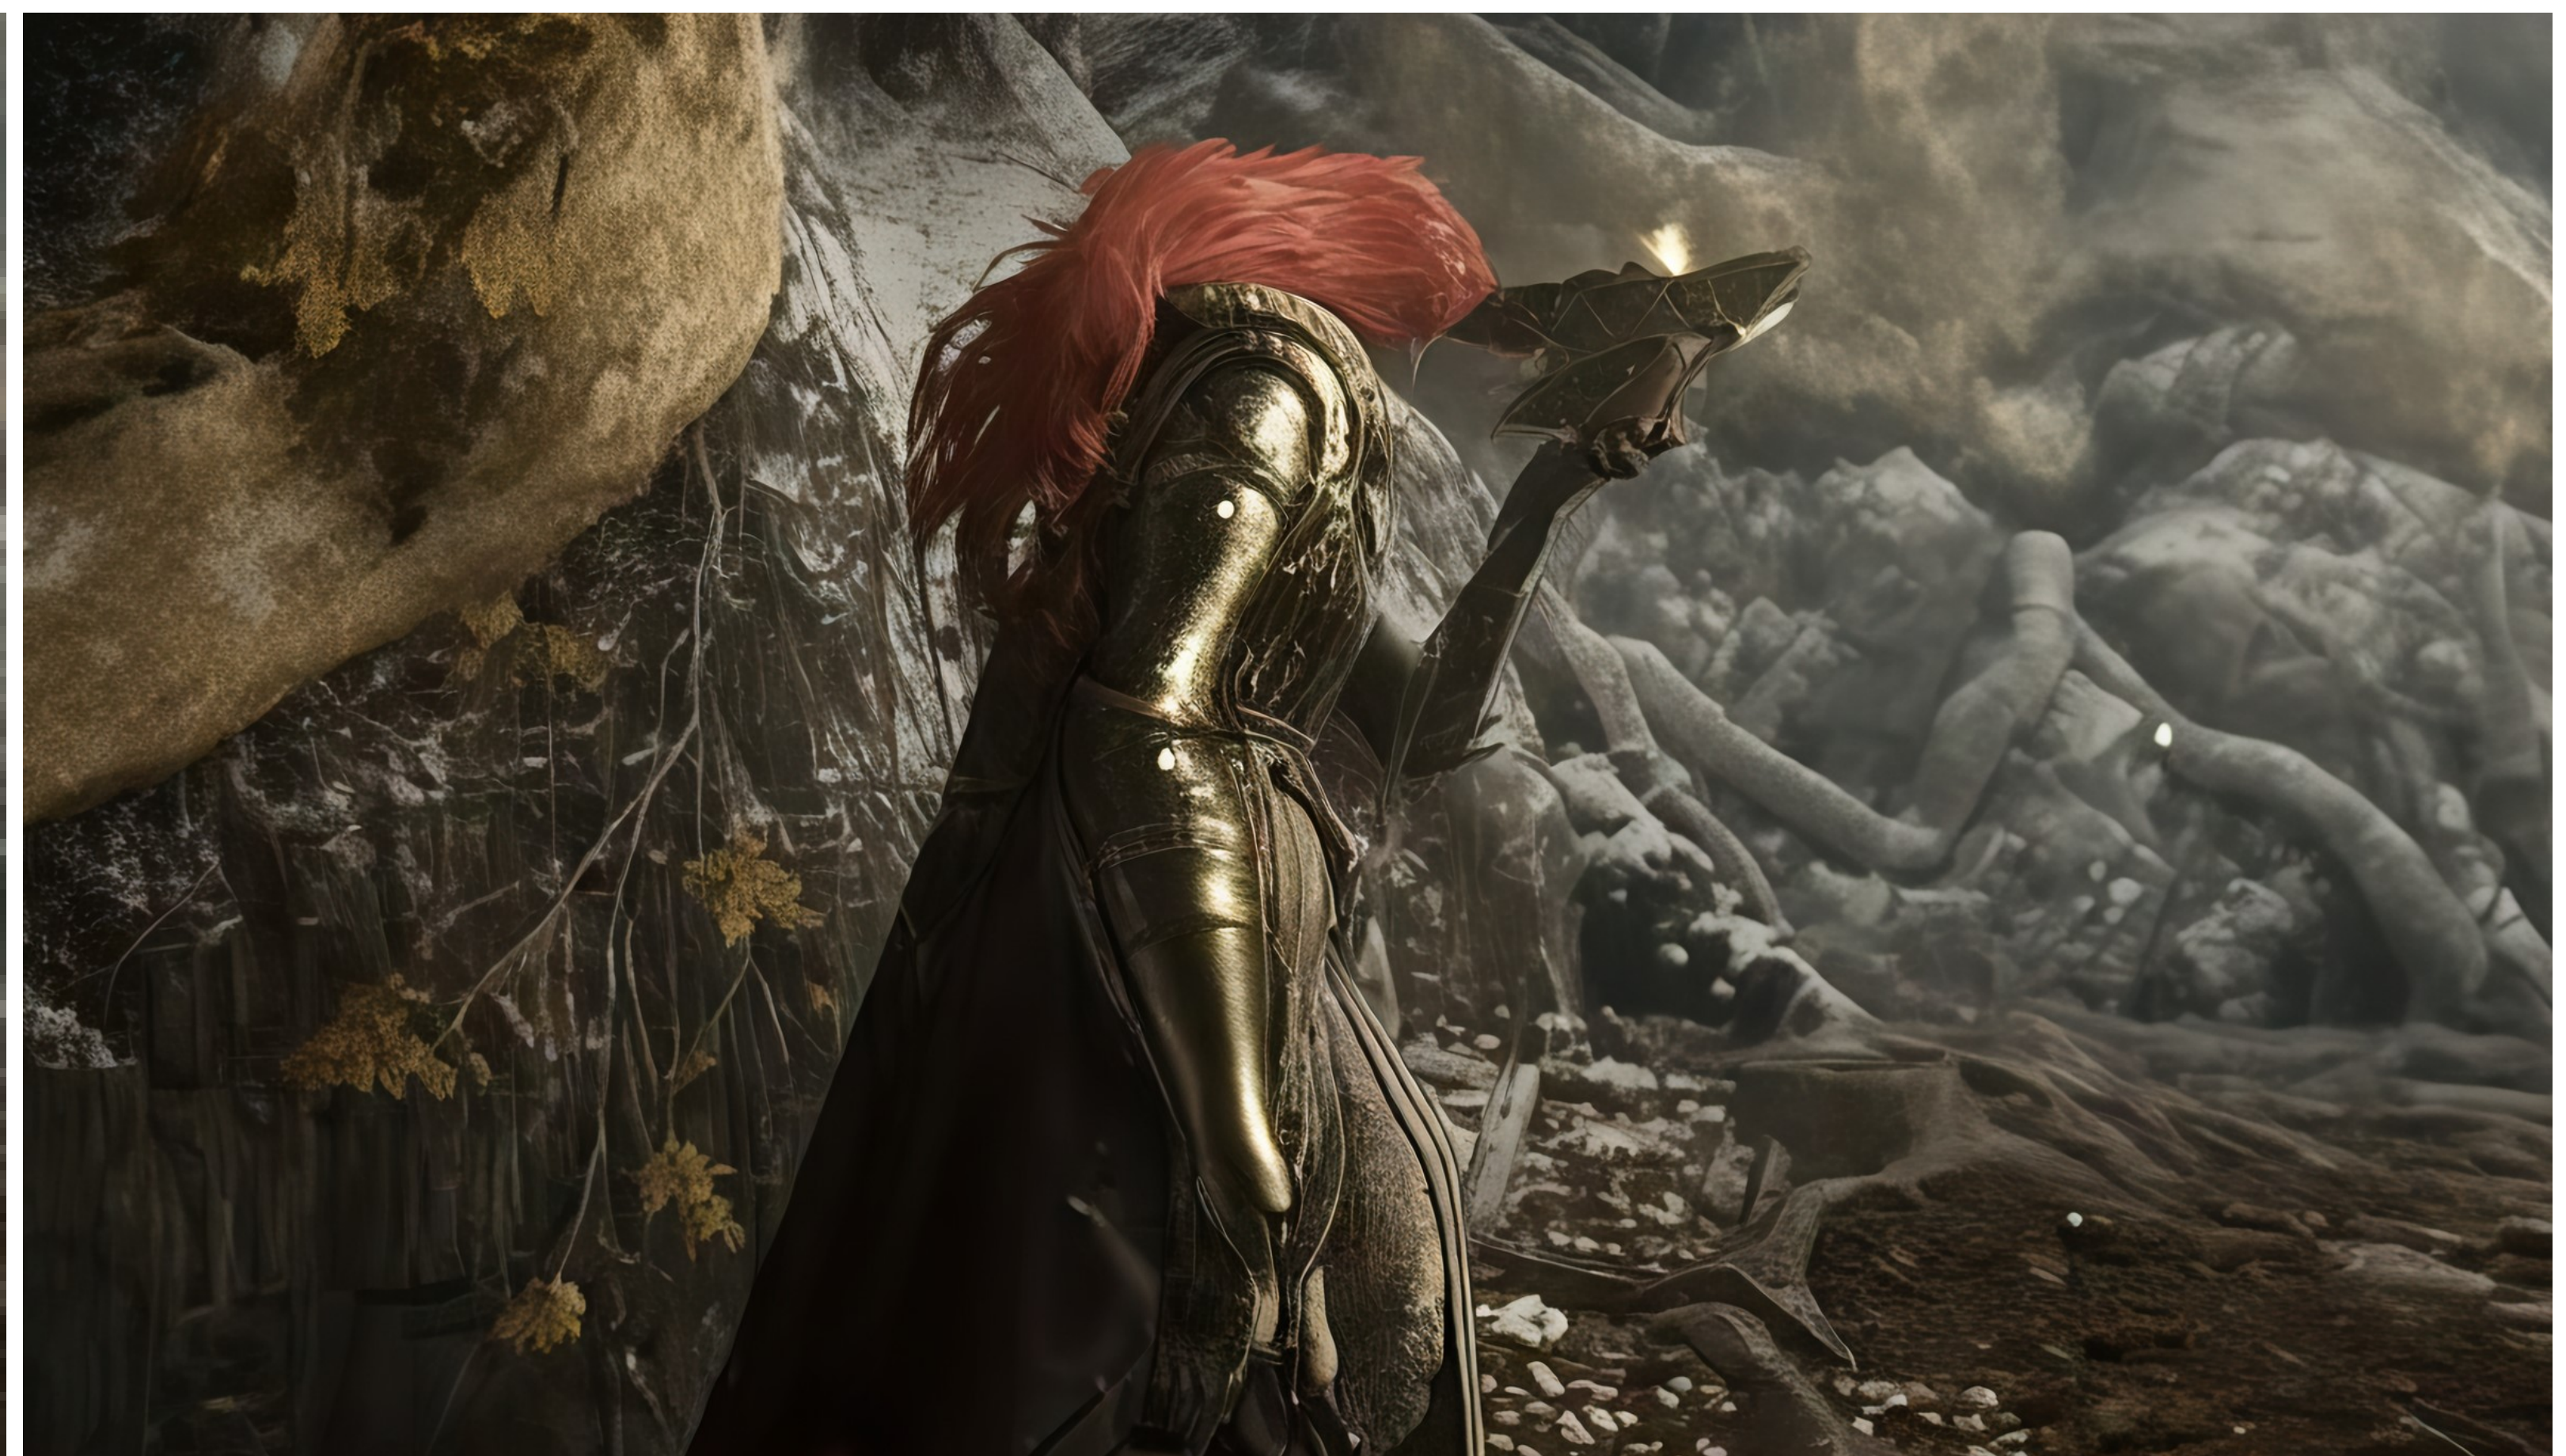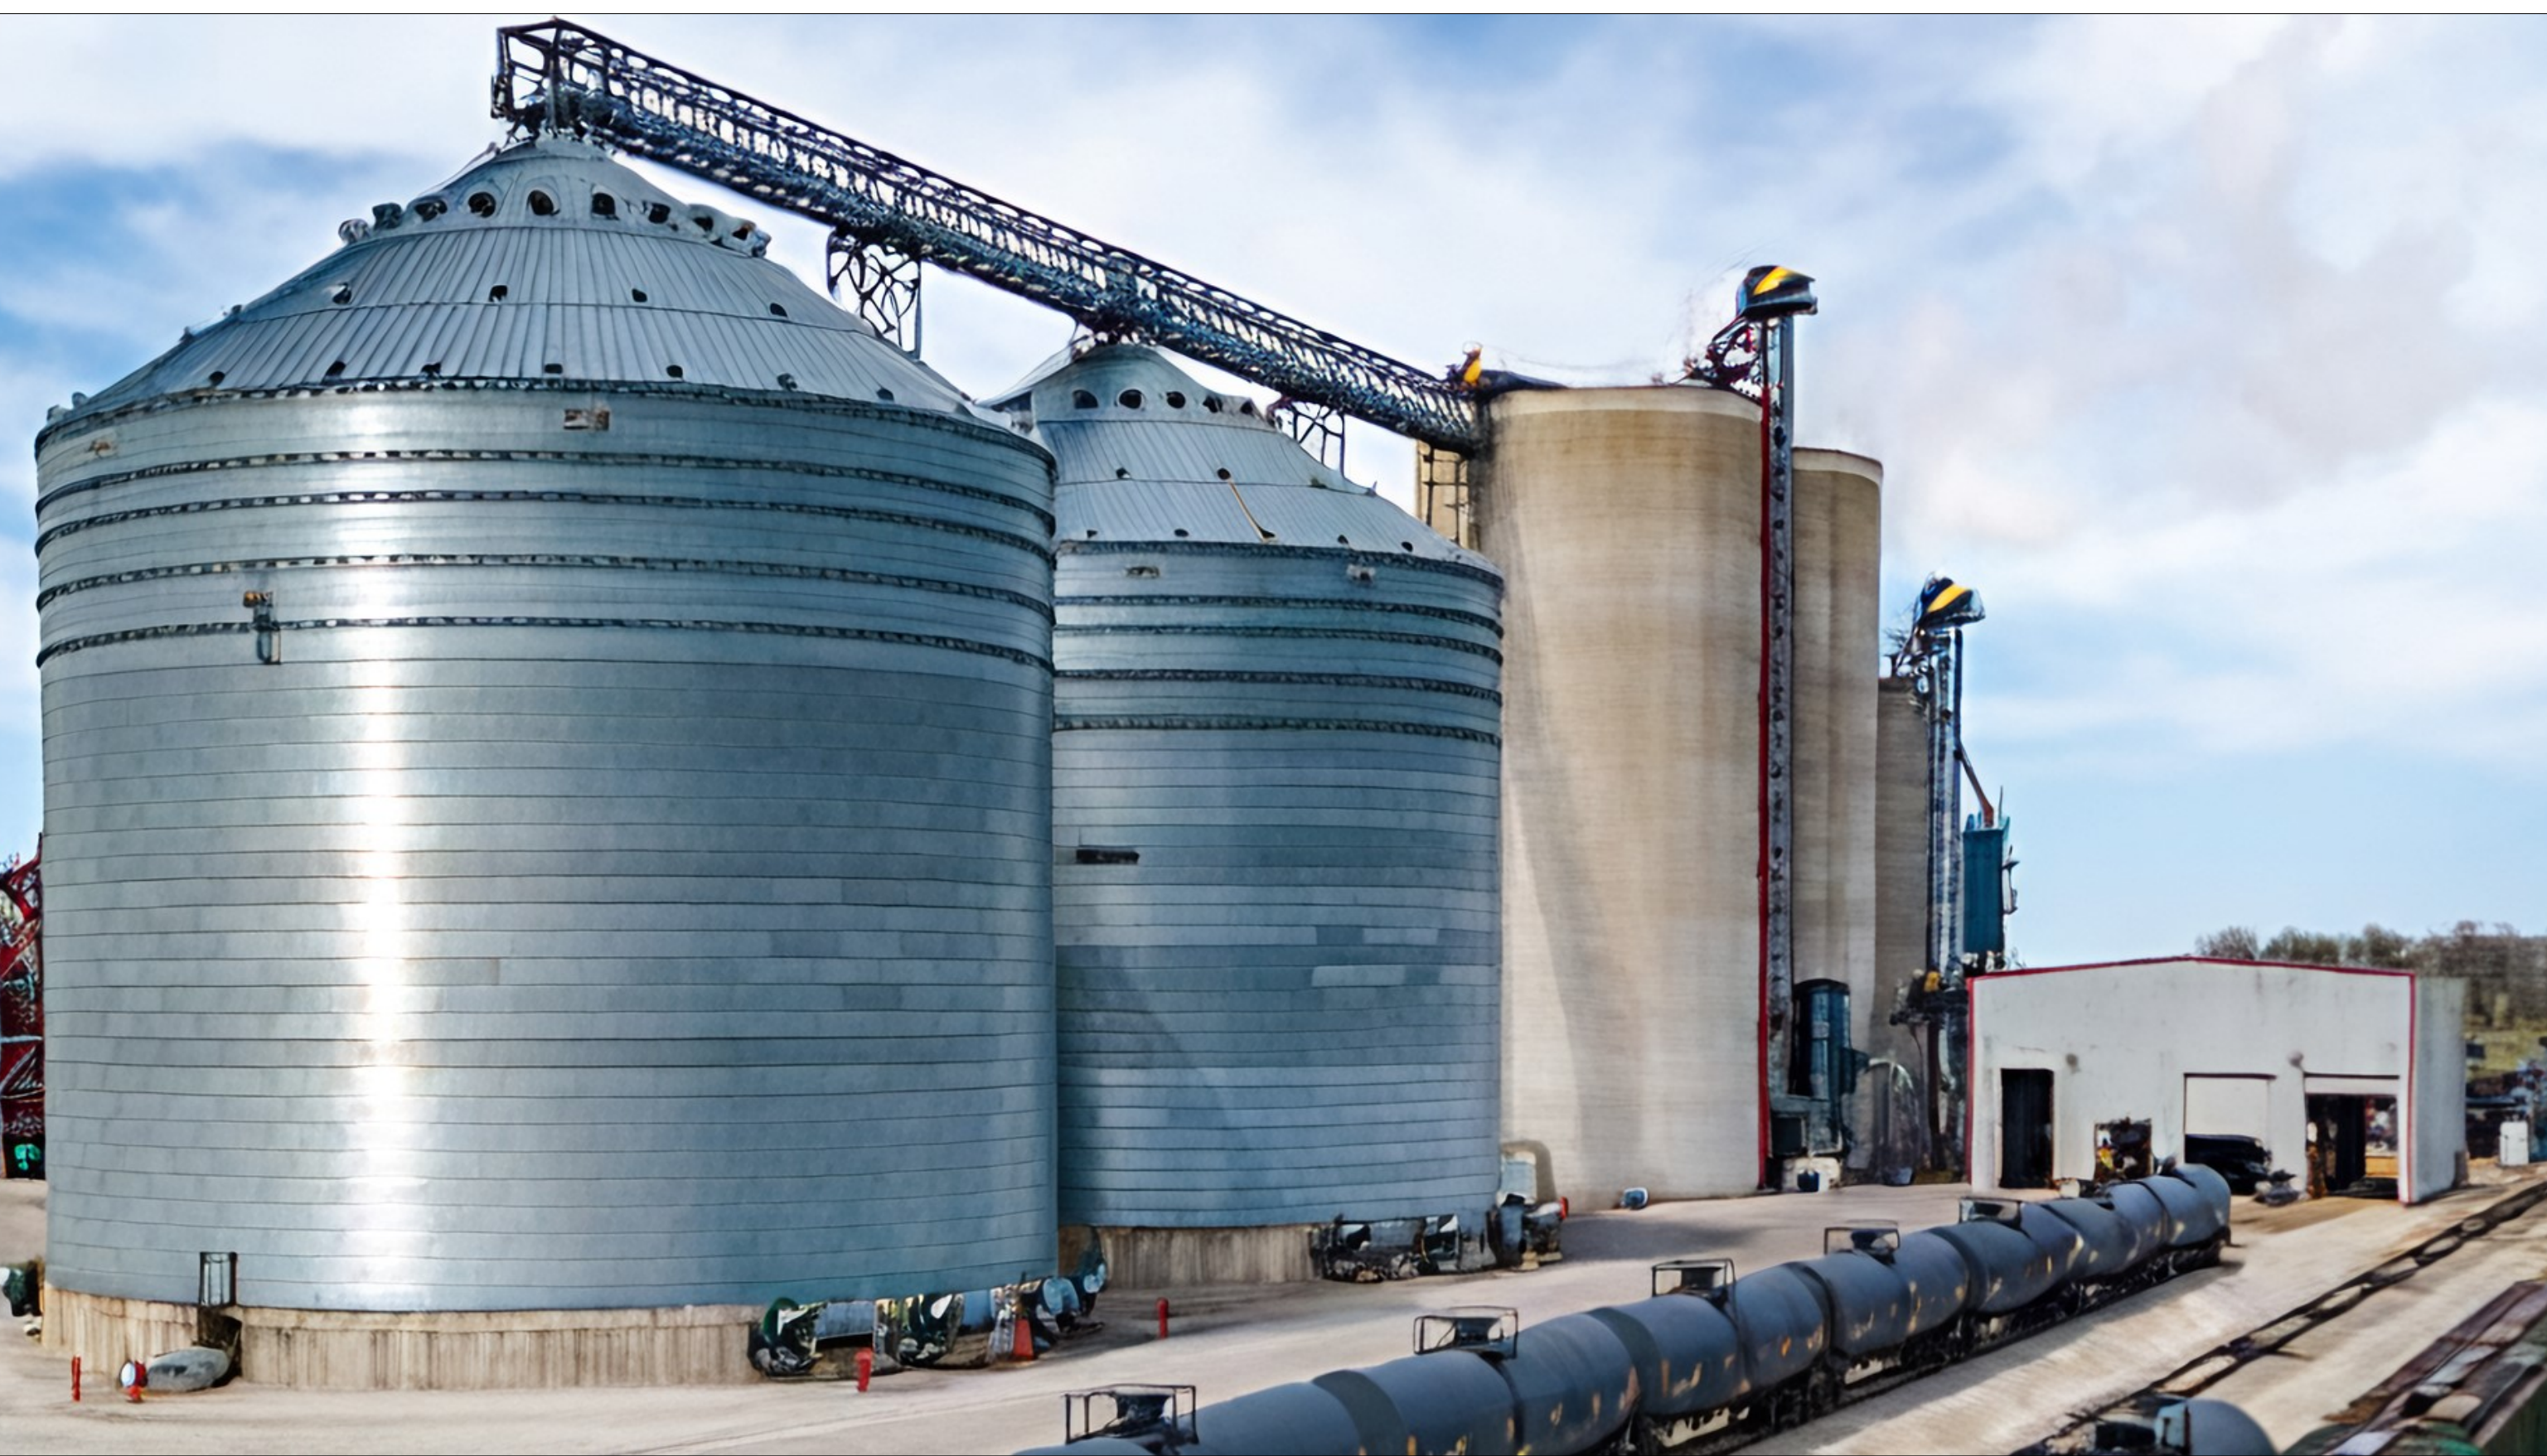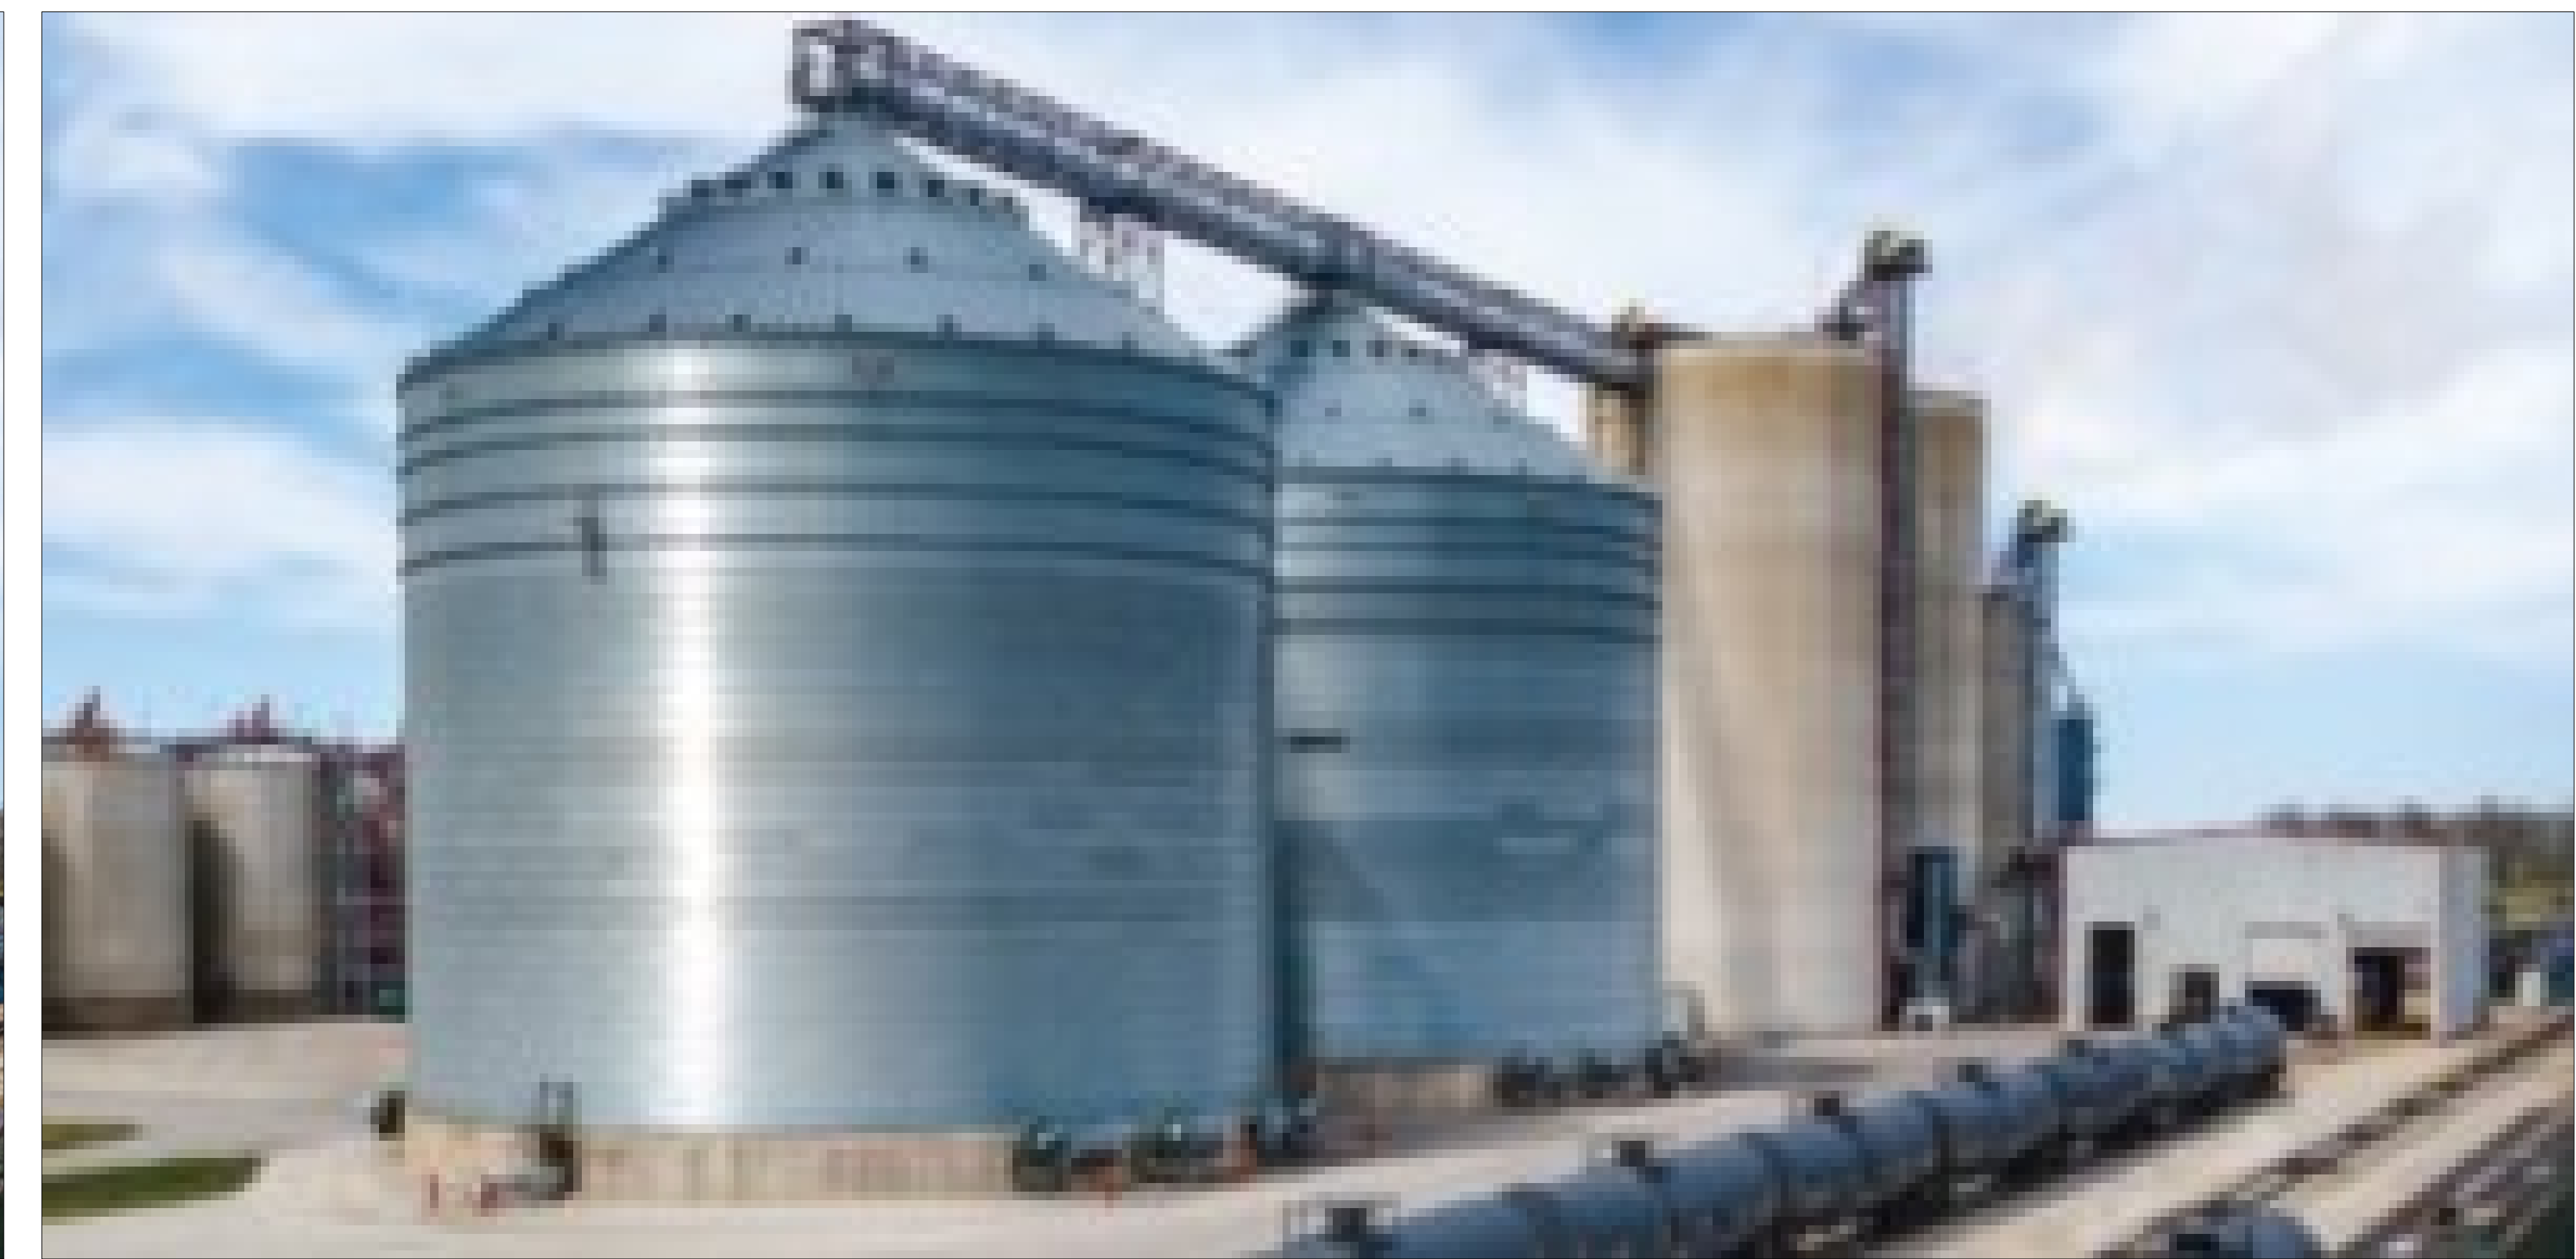

ALL DAY ME AT 3AM

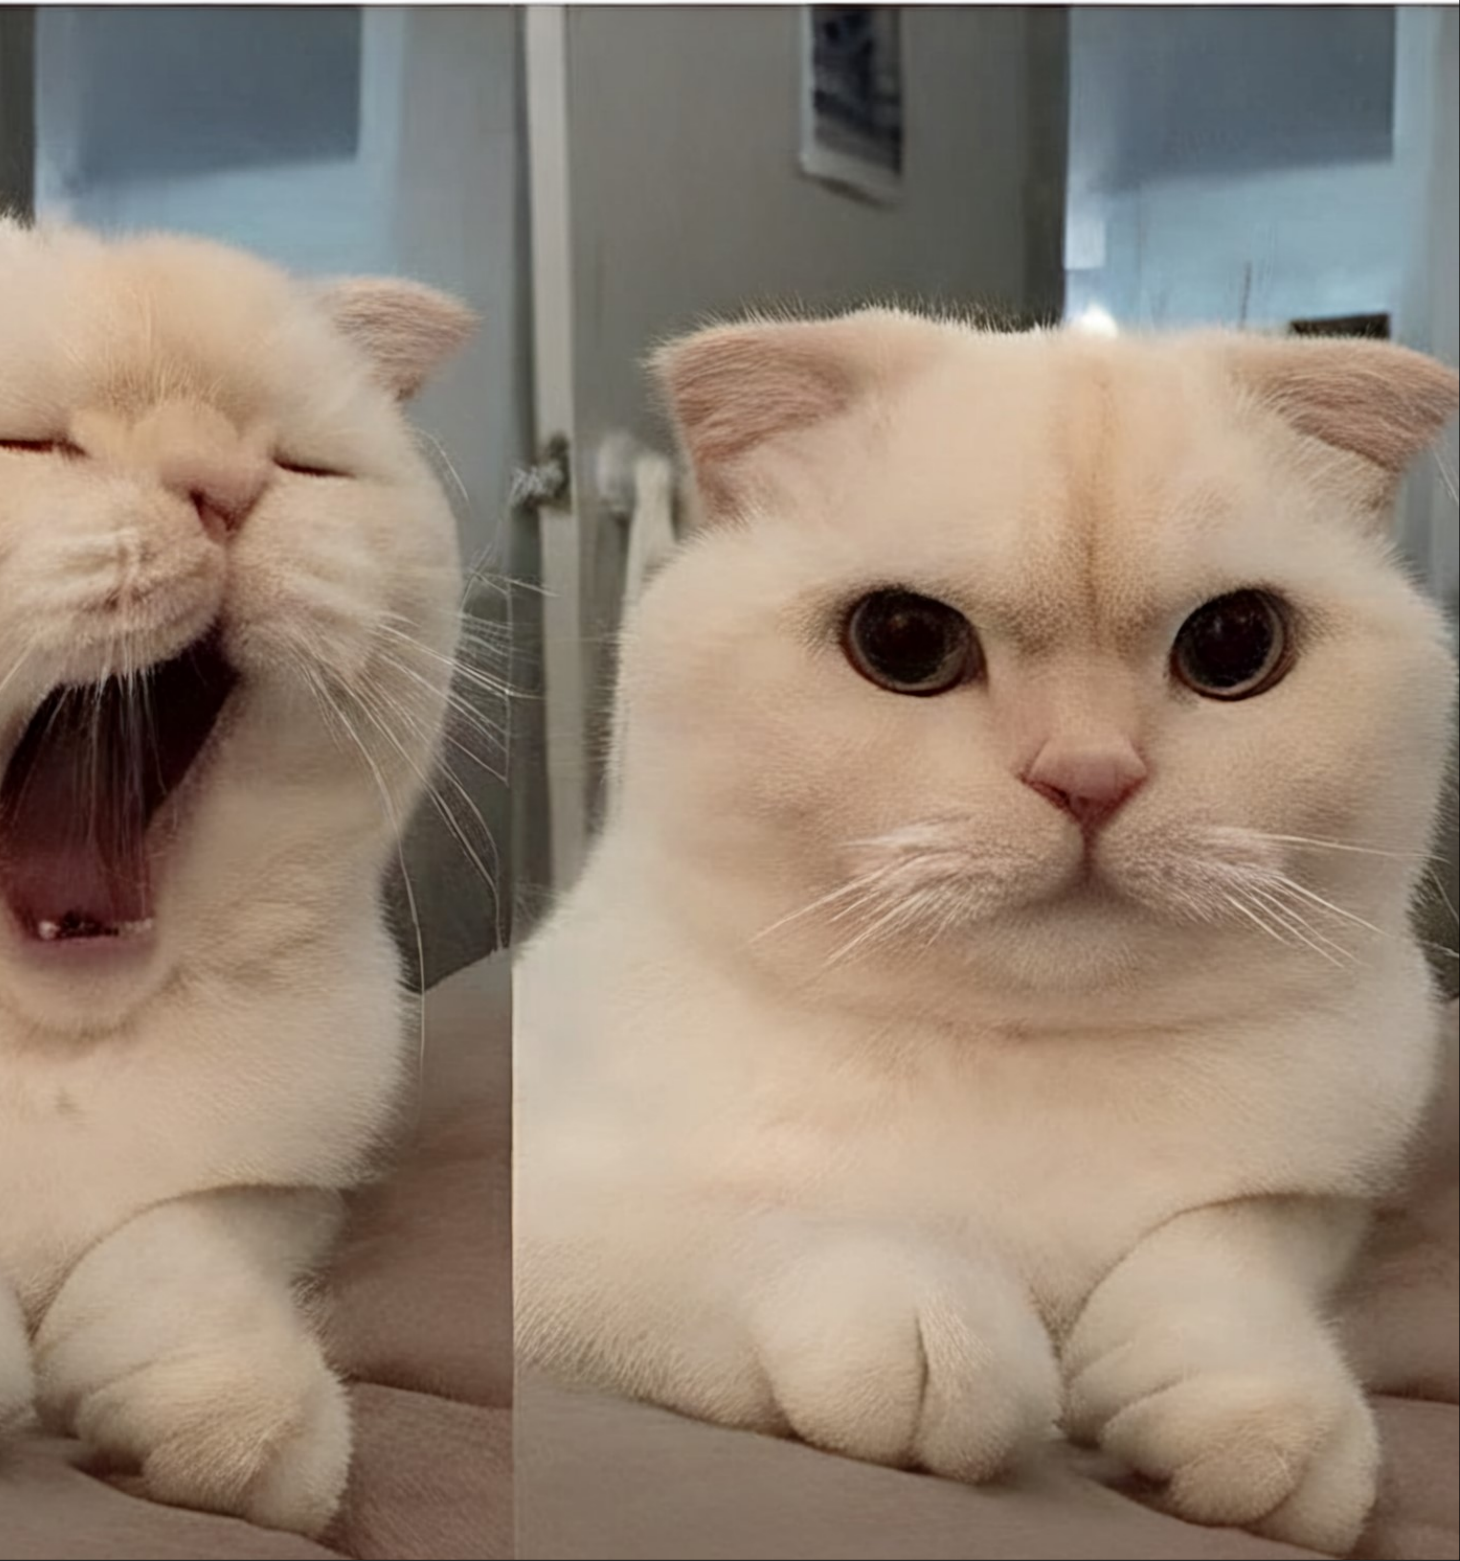

ME ALL DAY ME AT 3AM

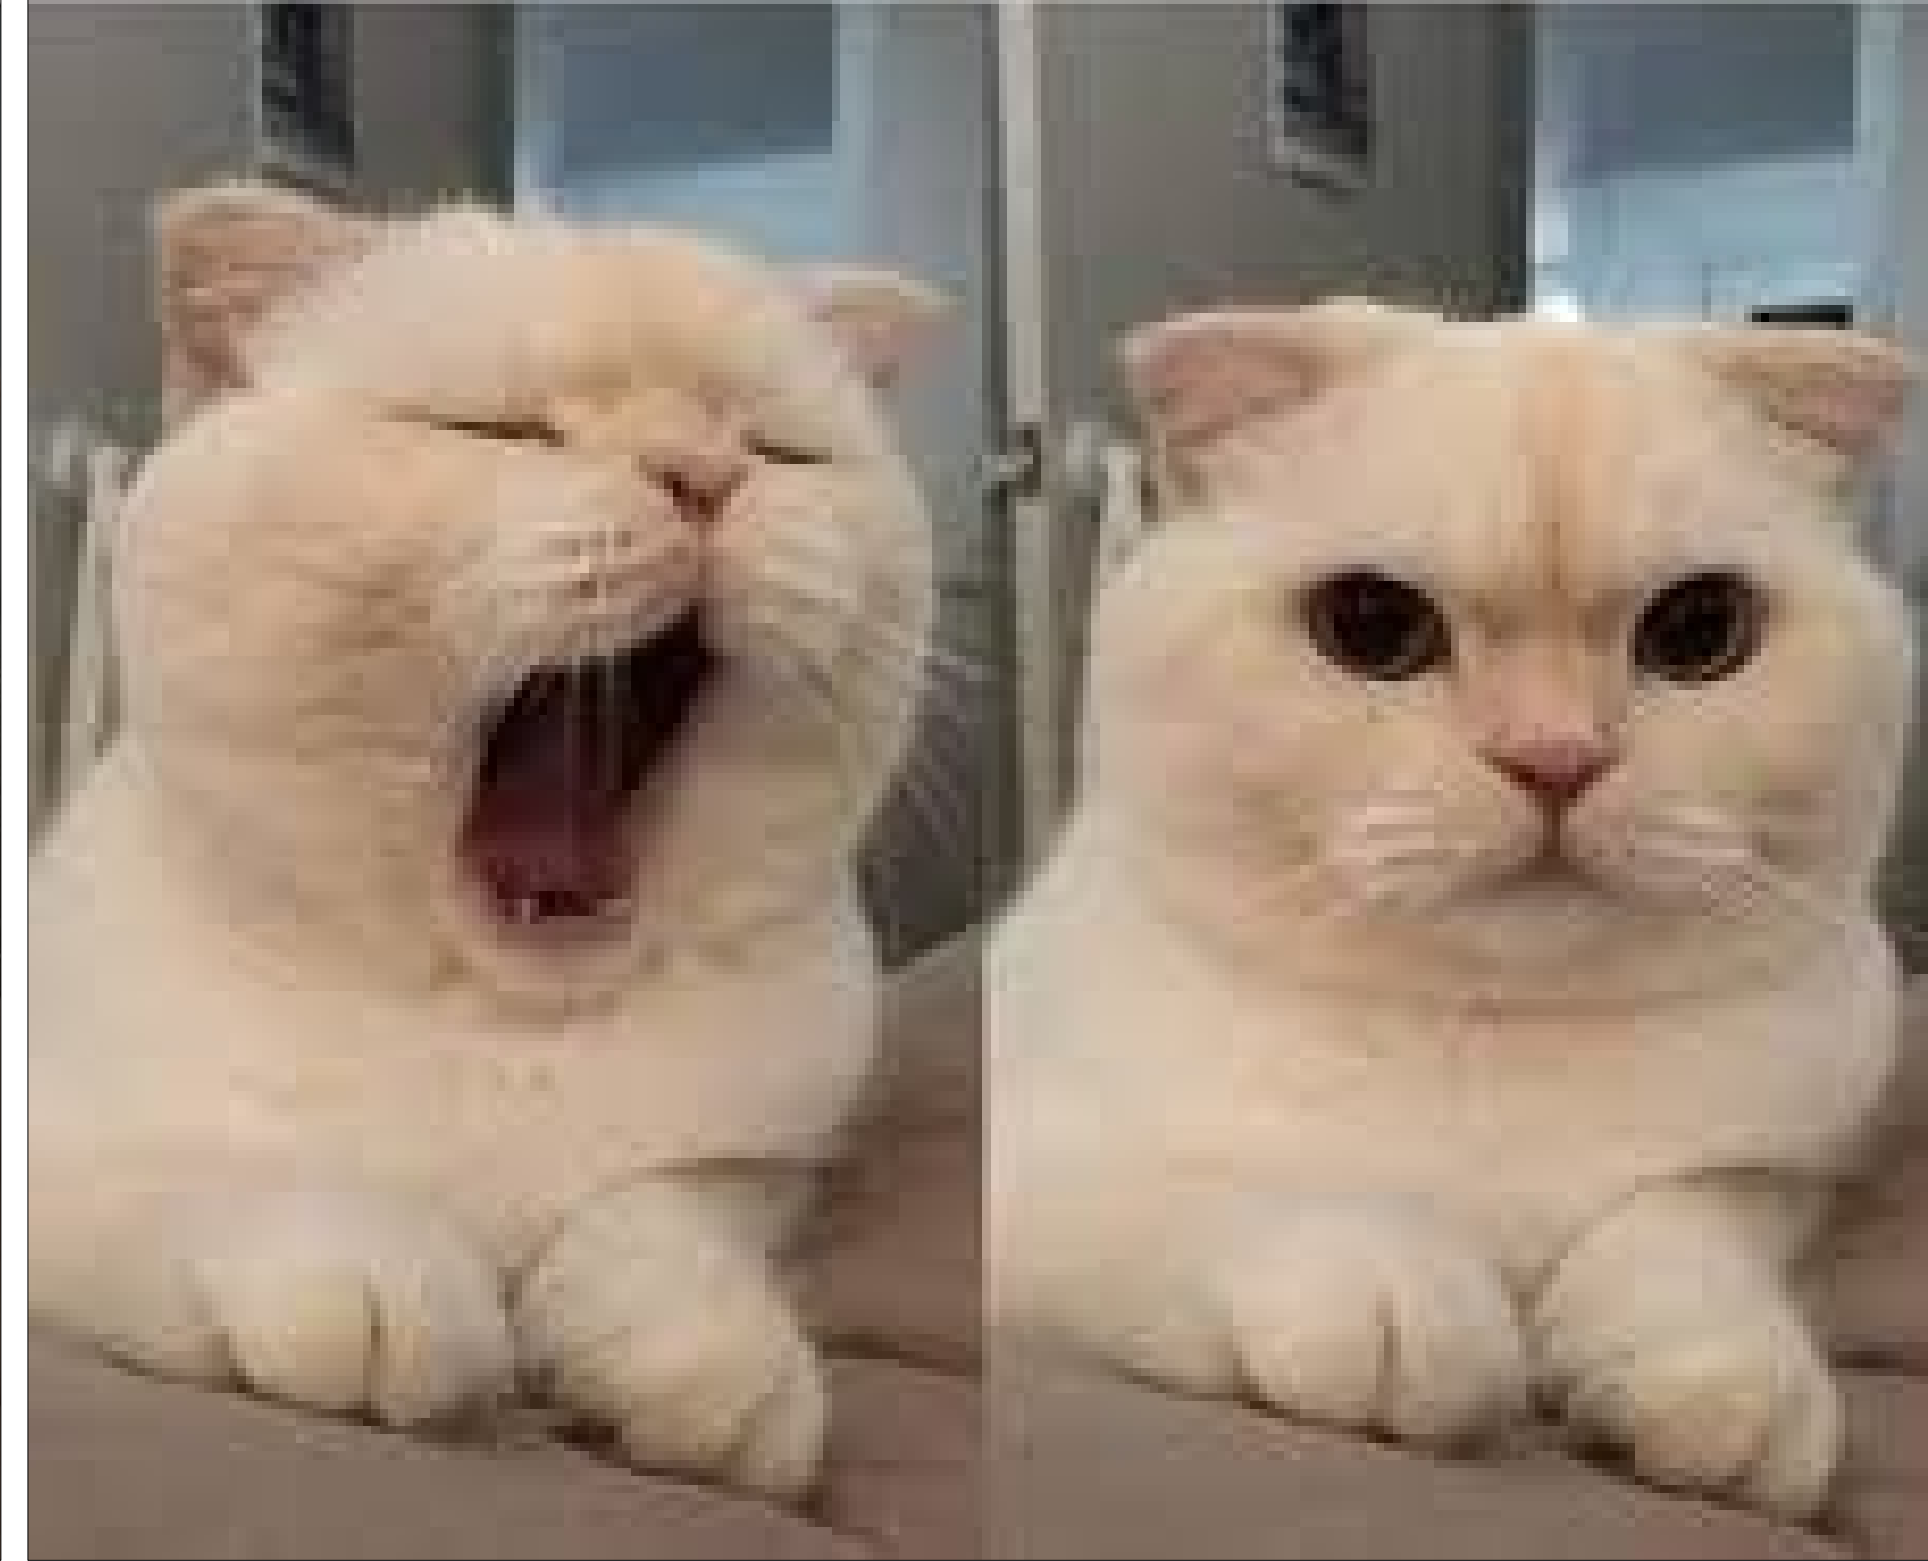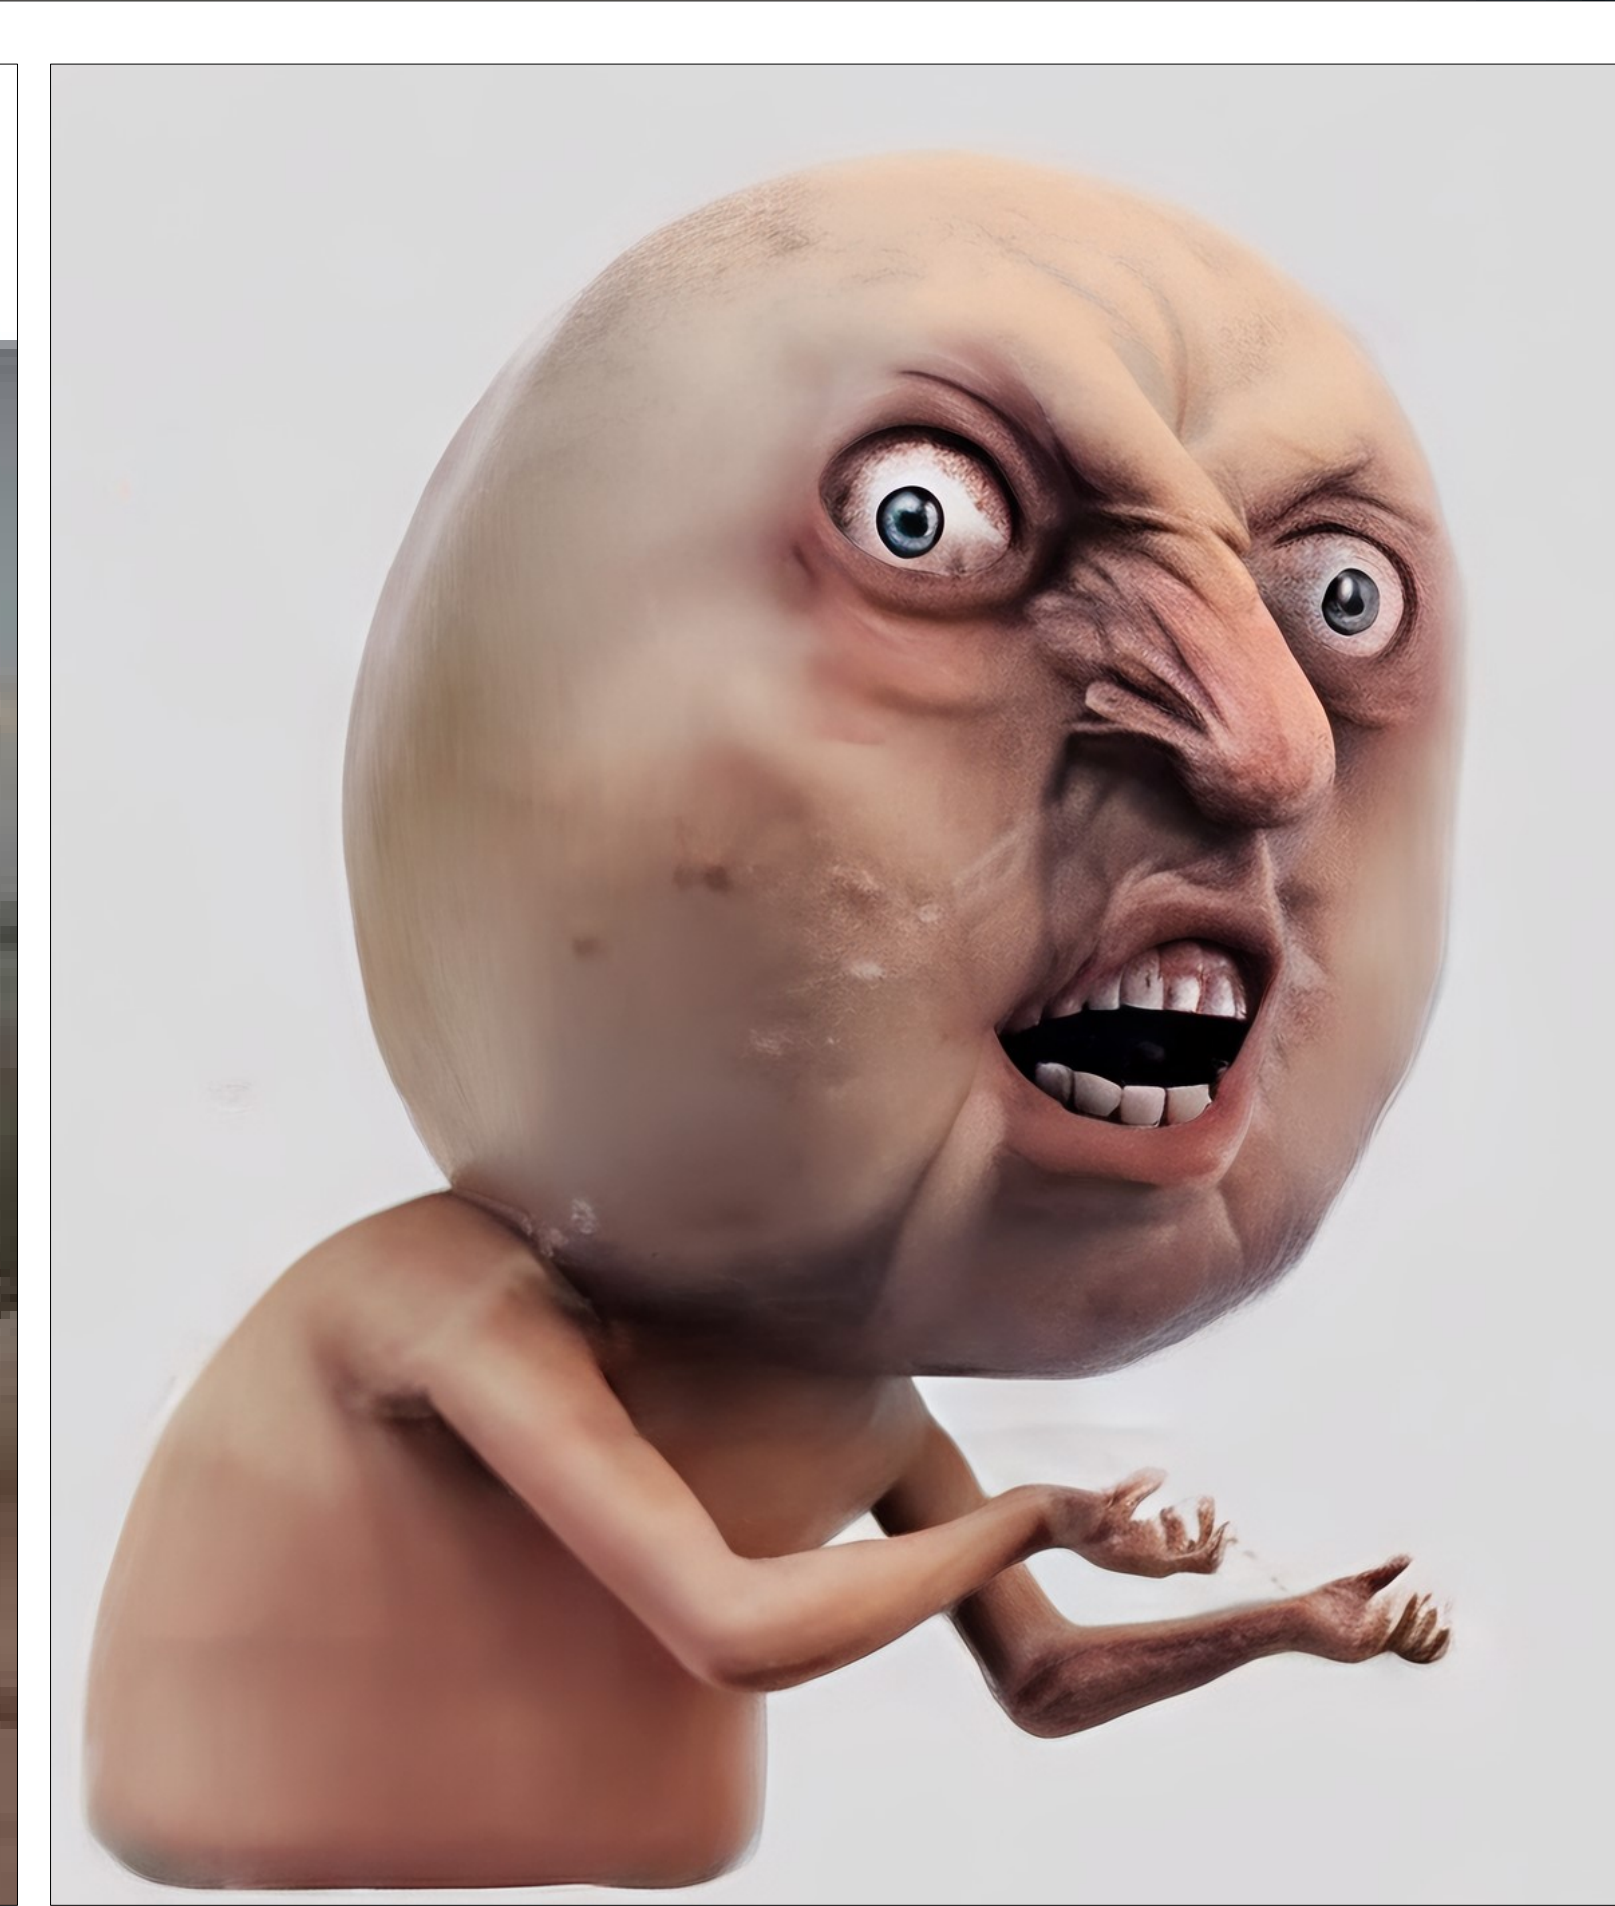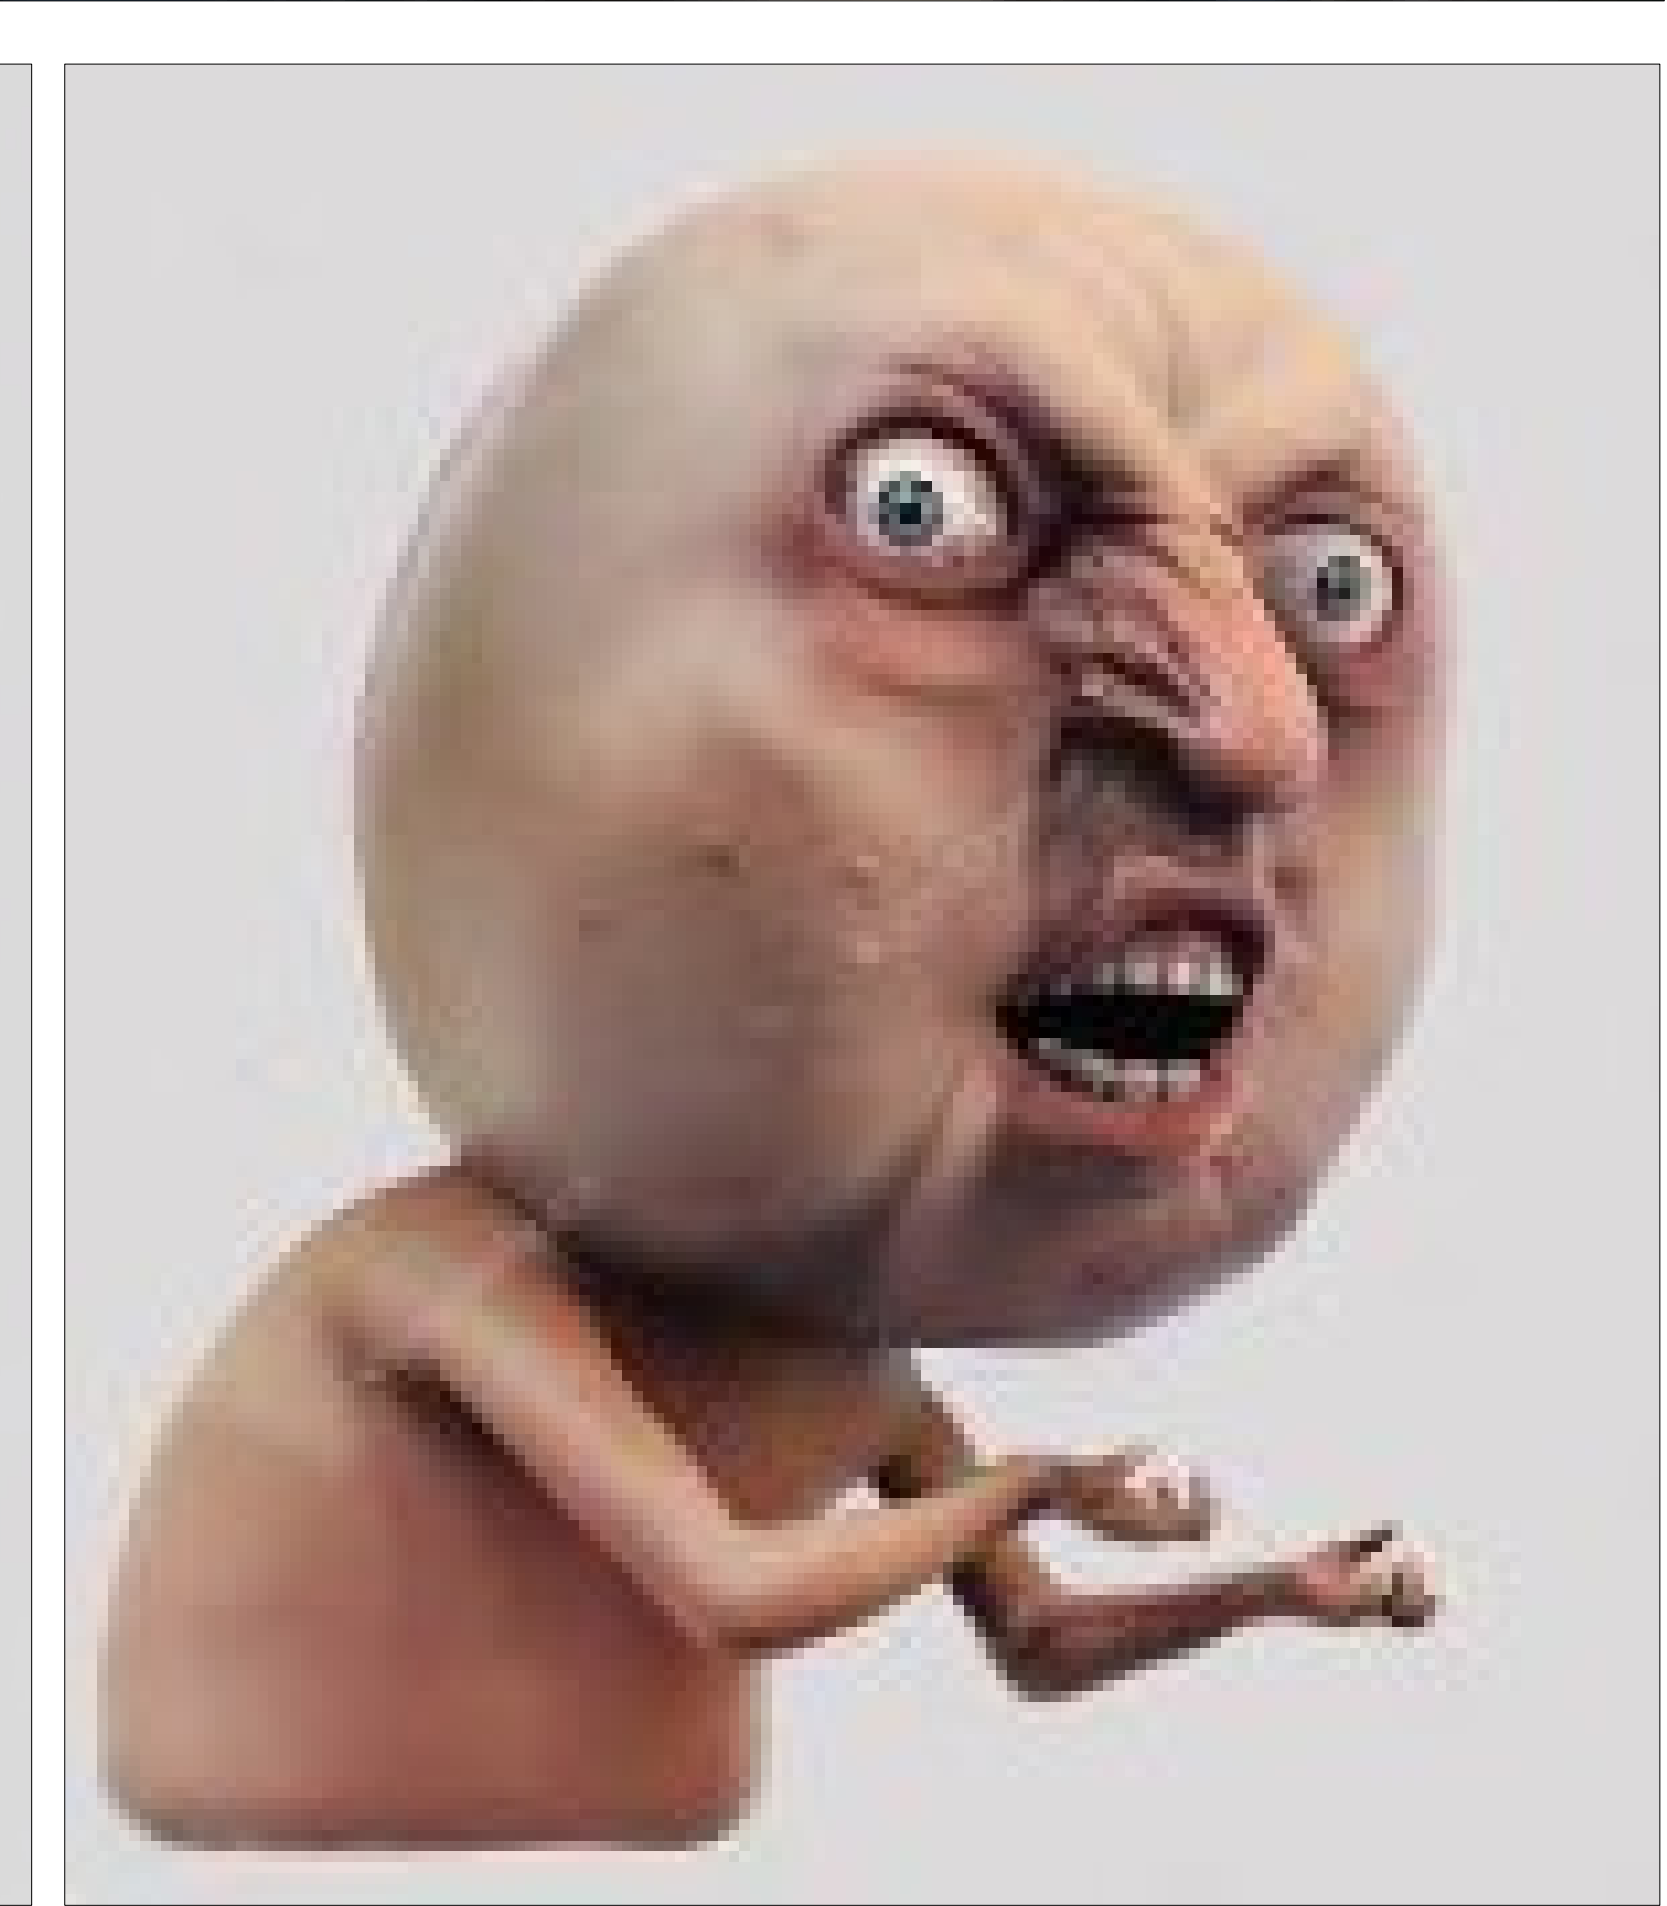

Supplement: Supplementary file 1 [file RealWorldCases-crop.pdf]
