# Supplementary material for: ZipIR: Latent Pyramid Diffusion Transformer for High-Resolution Image Restoration
Source: arXiv:2504.08591 source file (2025-04-11)
Supplement: Supplementary file 2 [file comparison_vae_recon-crop.pdf]

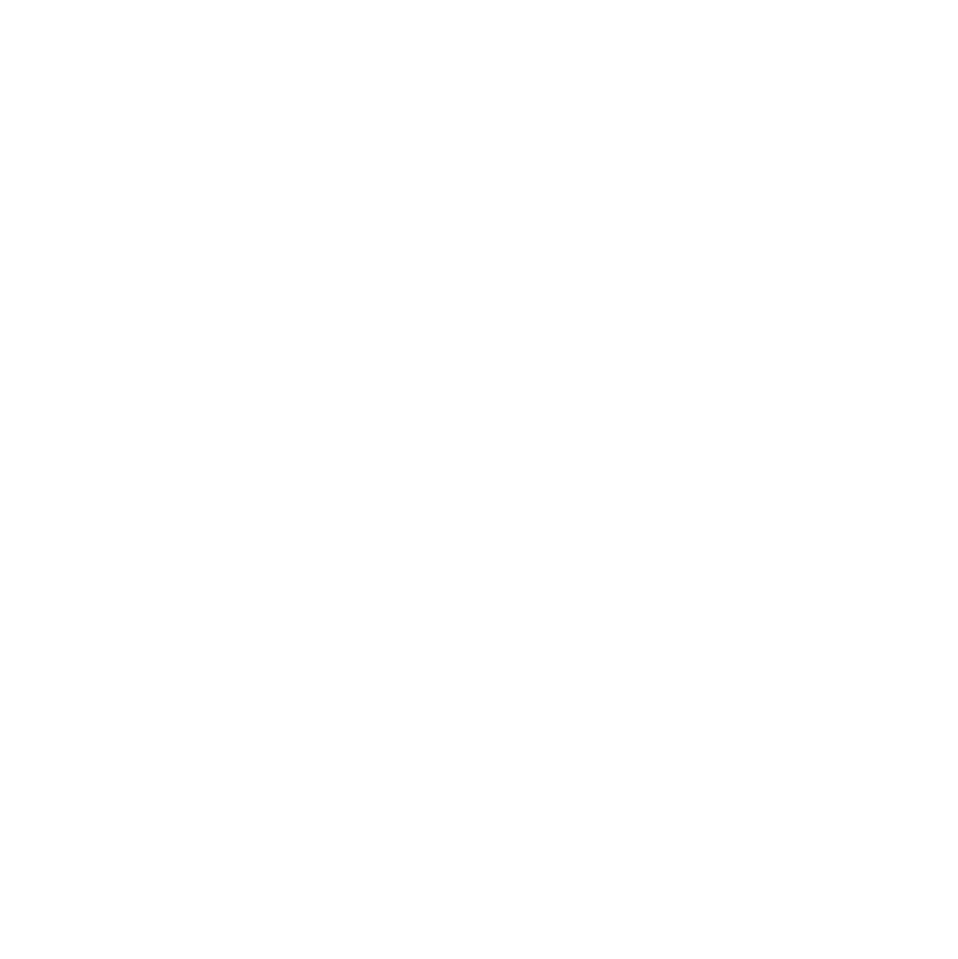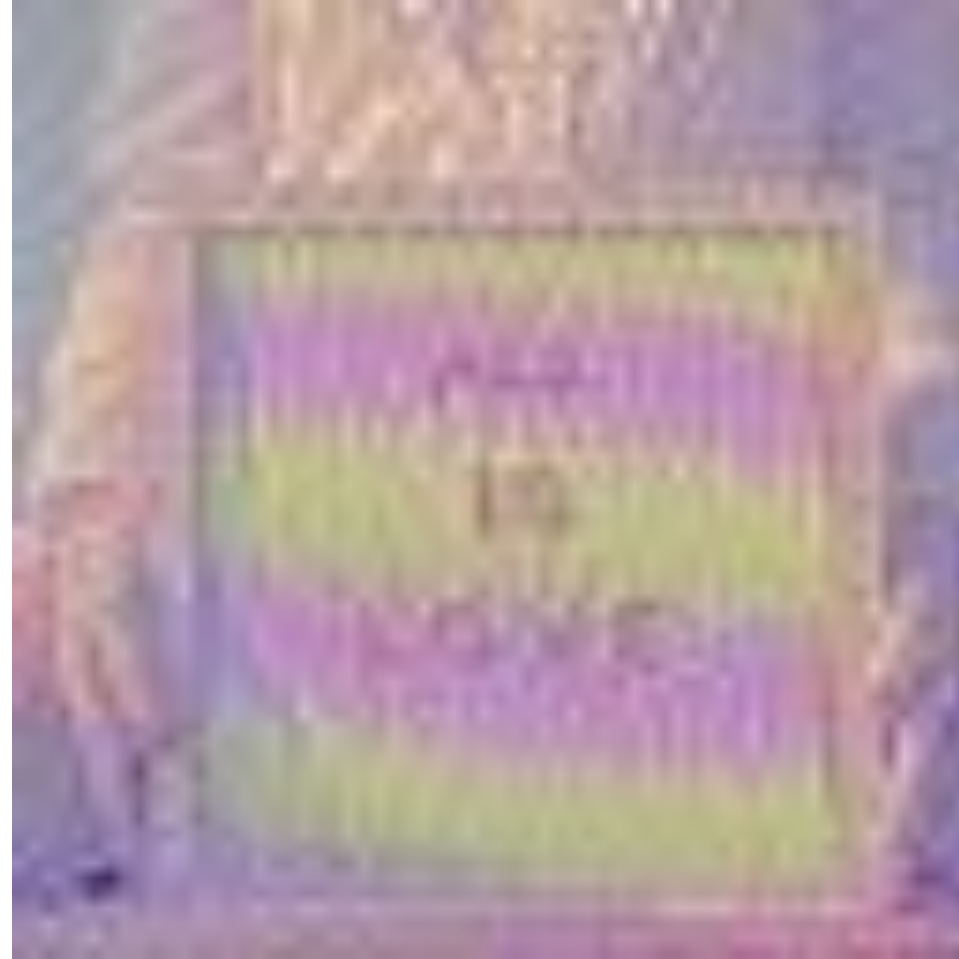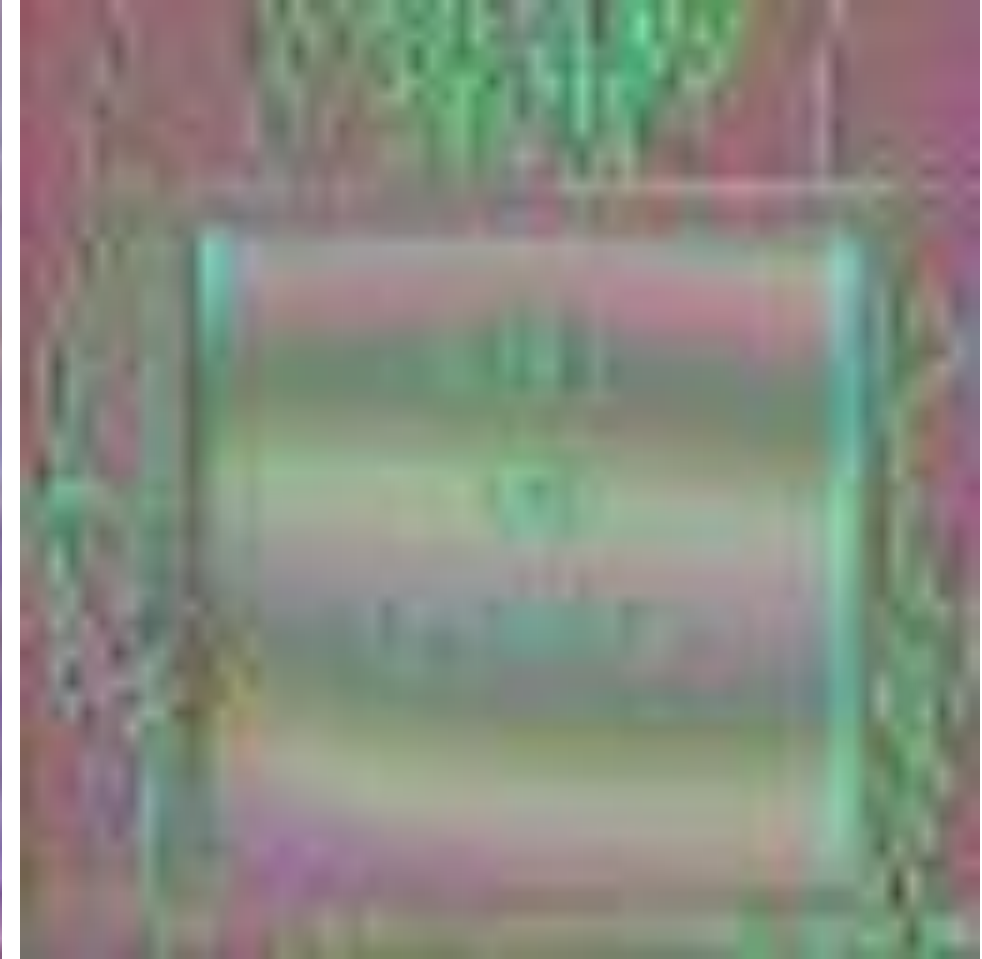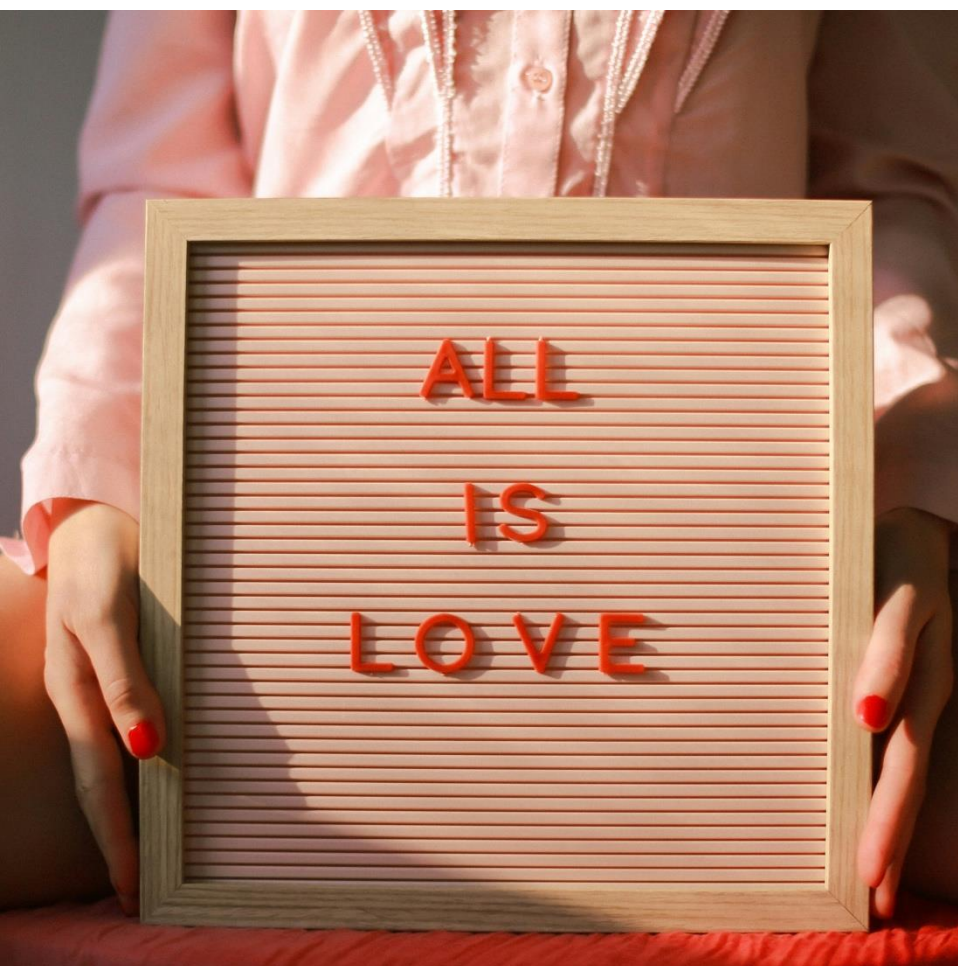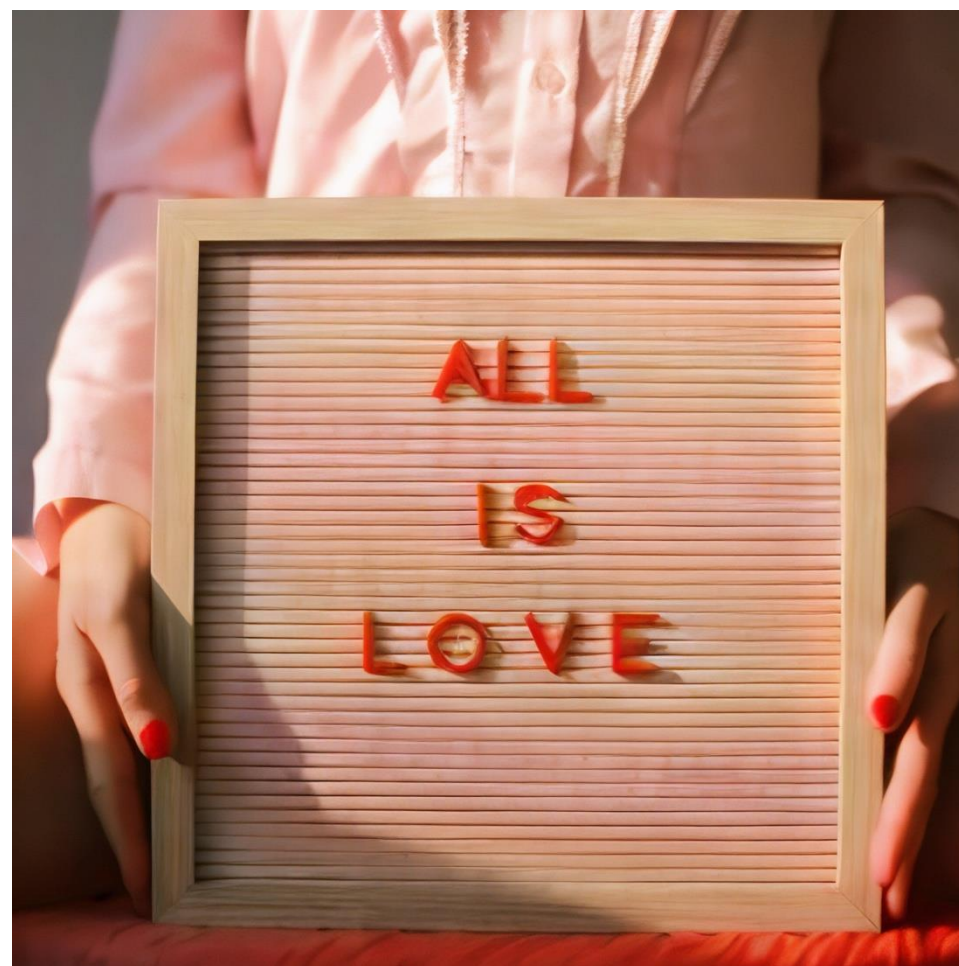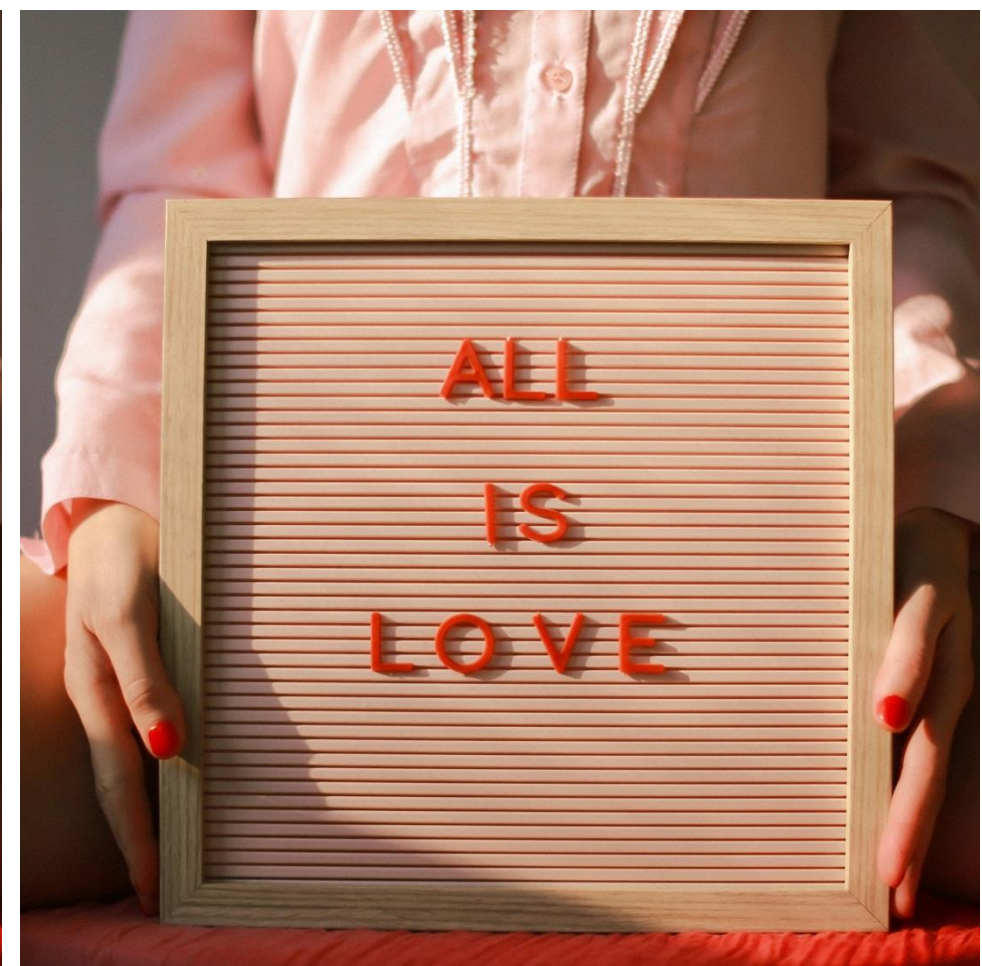

Ground Truth

SD-VAE f32c64 Results

LP-VAE Results



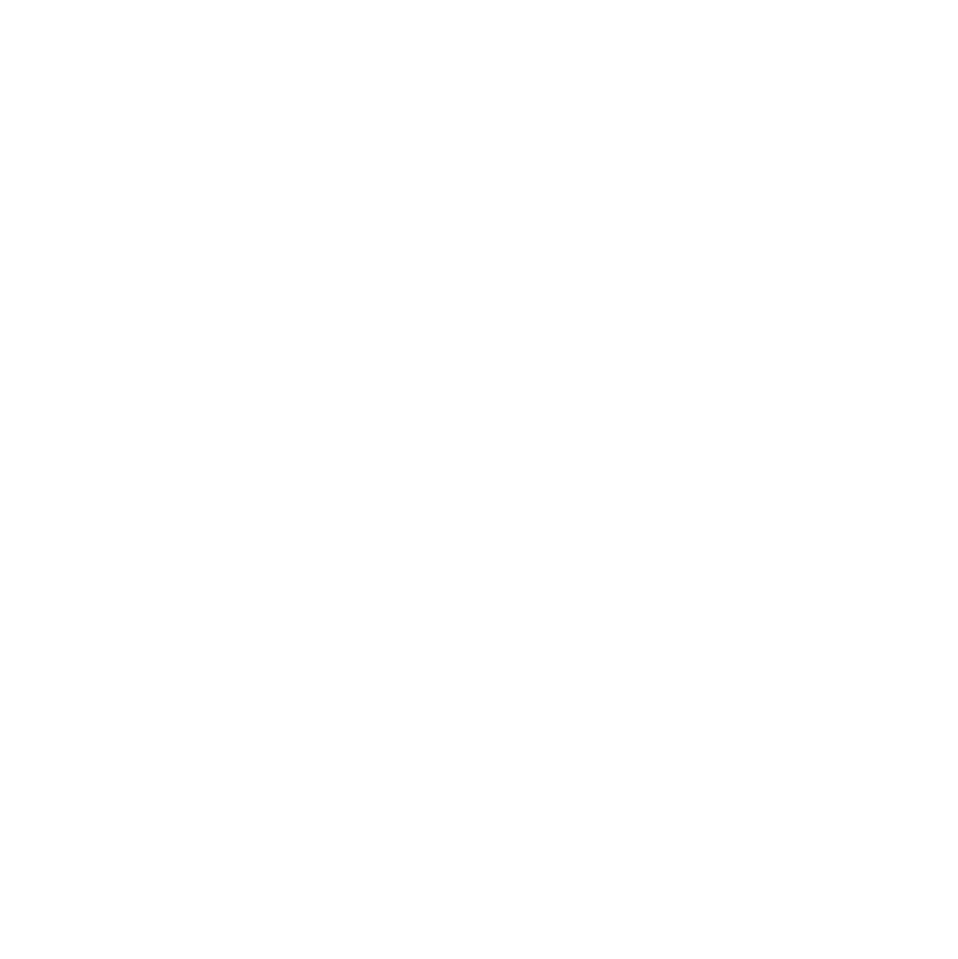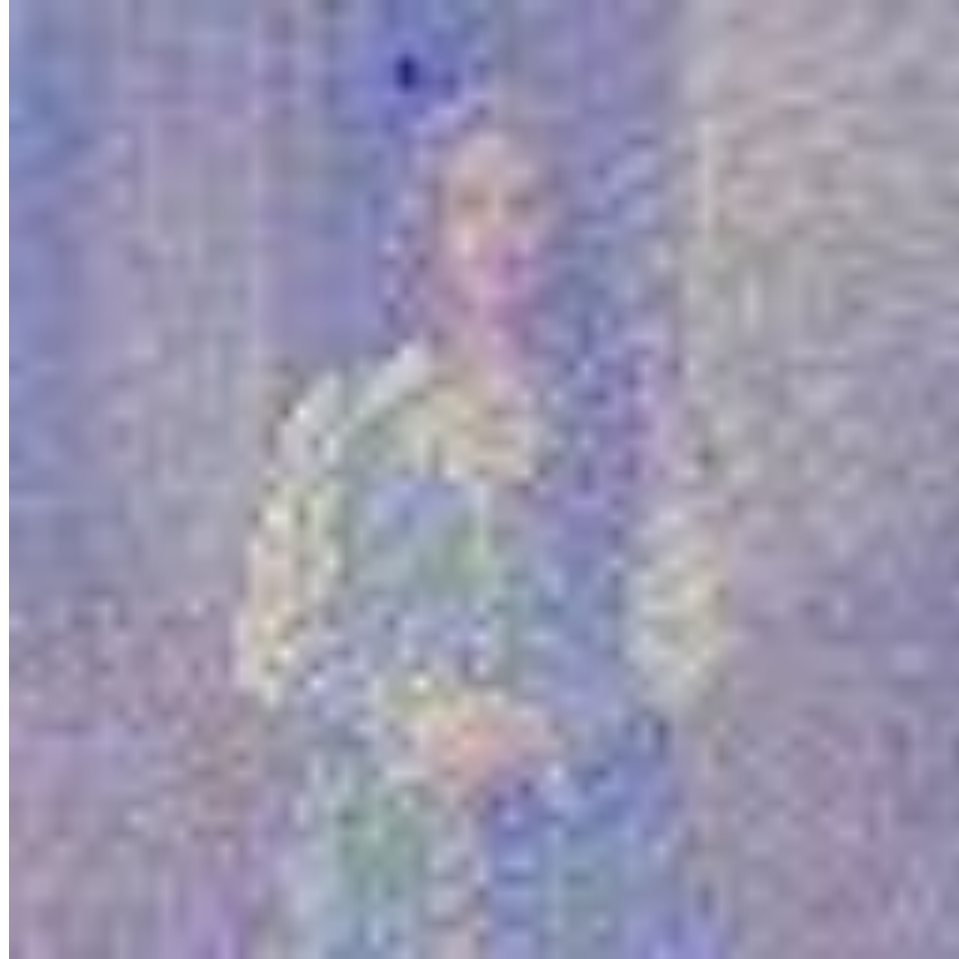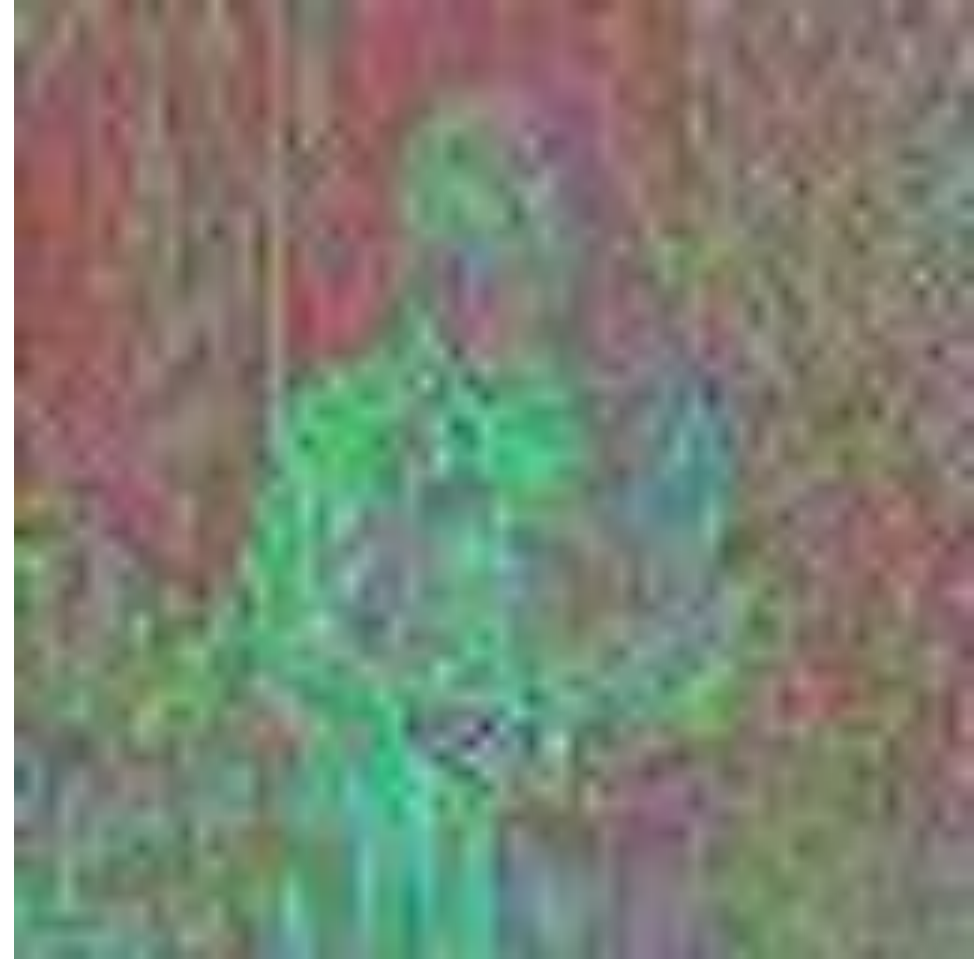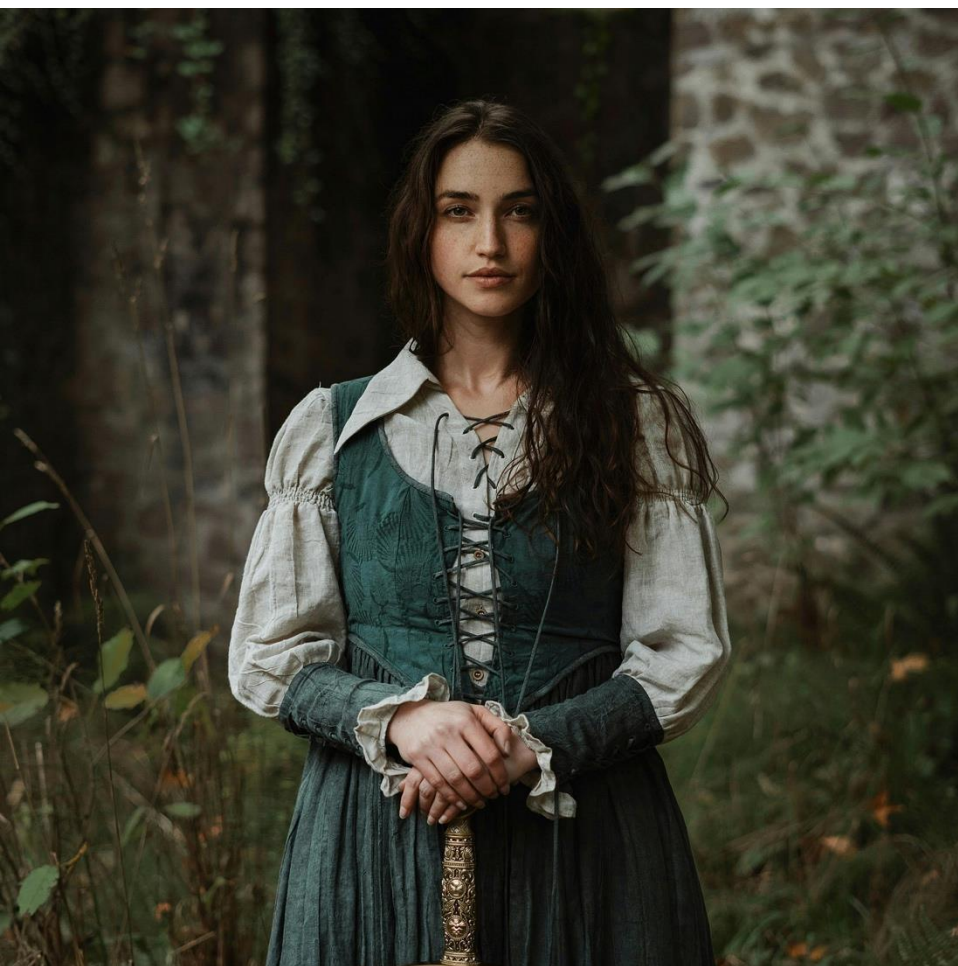

Ground Truth

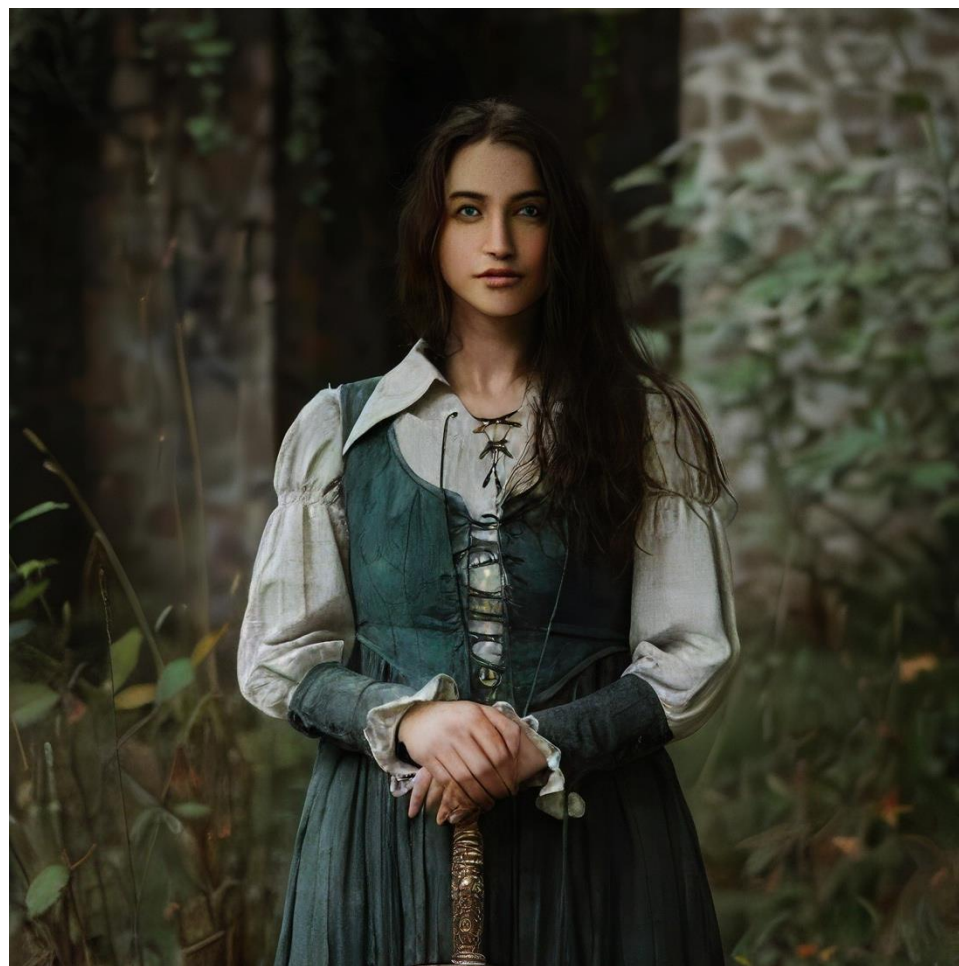

SD-VAE f32c64 Results

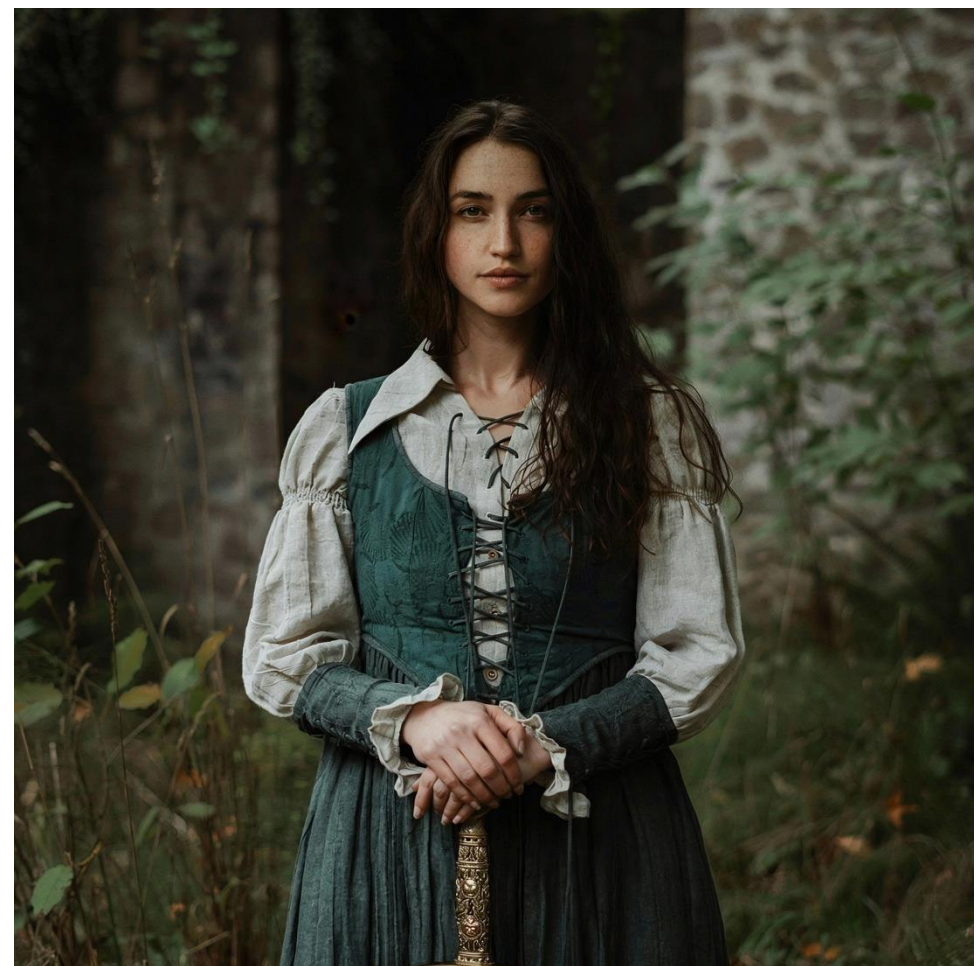

LP-VAE Results
