# Supplementary material for: ZipIR: Latent Pyramid Diffusion Transformer for High-Resolution Image Restoration
Source: arXiv:2504.08591 source file (2025-04-11)
Supplement: Supplementary file 3 [file supp_qualitative_comparison-crop.pdf]



Ours (6.9s)

16× SR, 2048px, 4Mpix

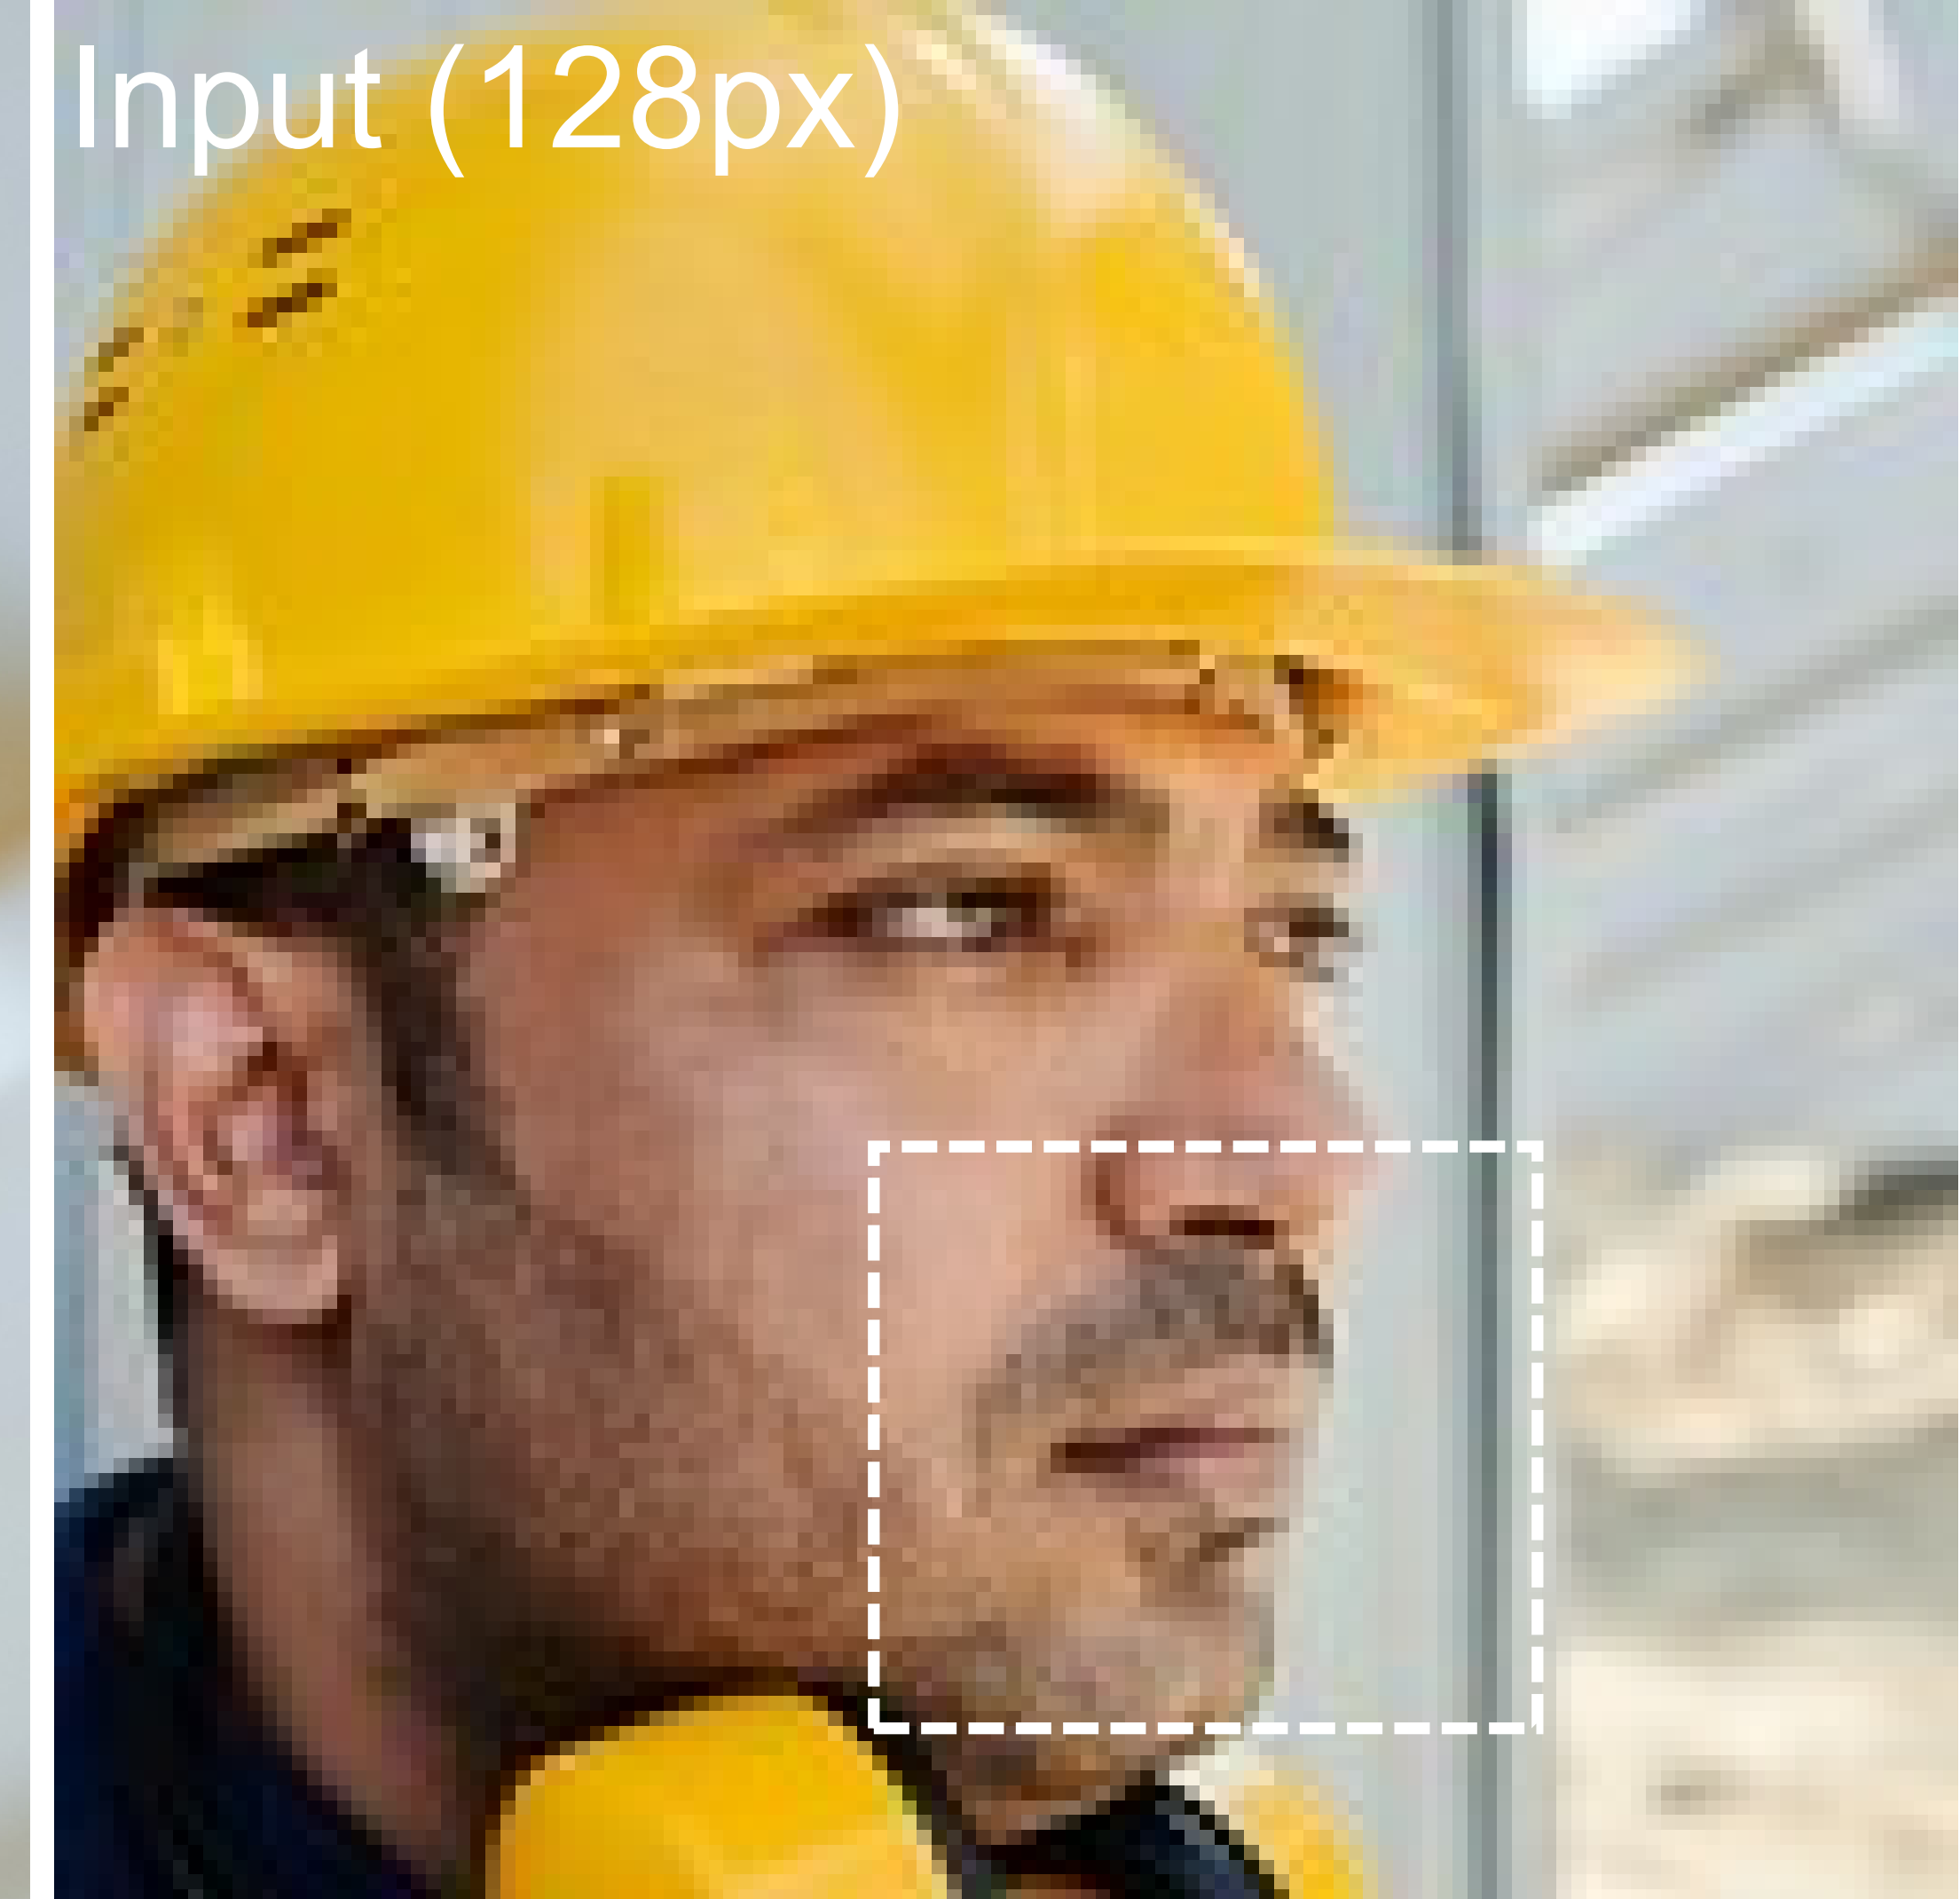

Input (128px)

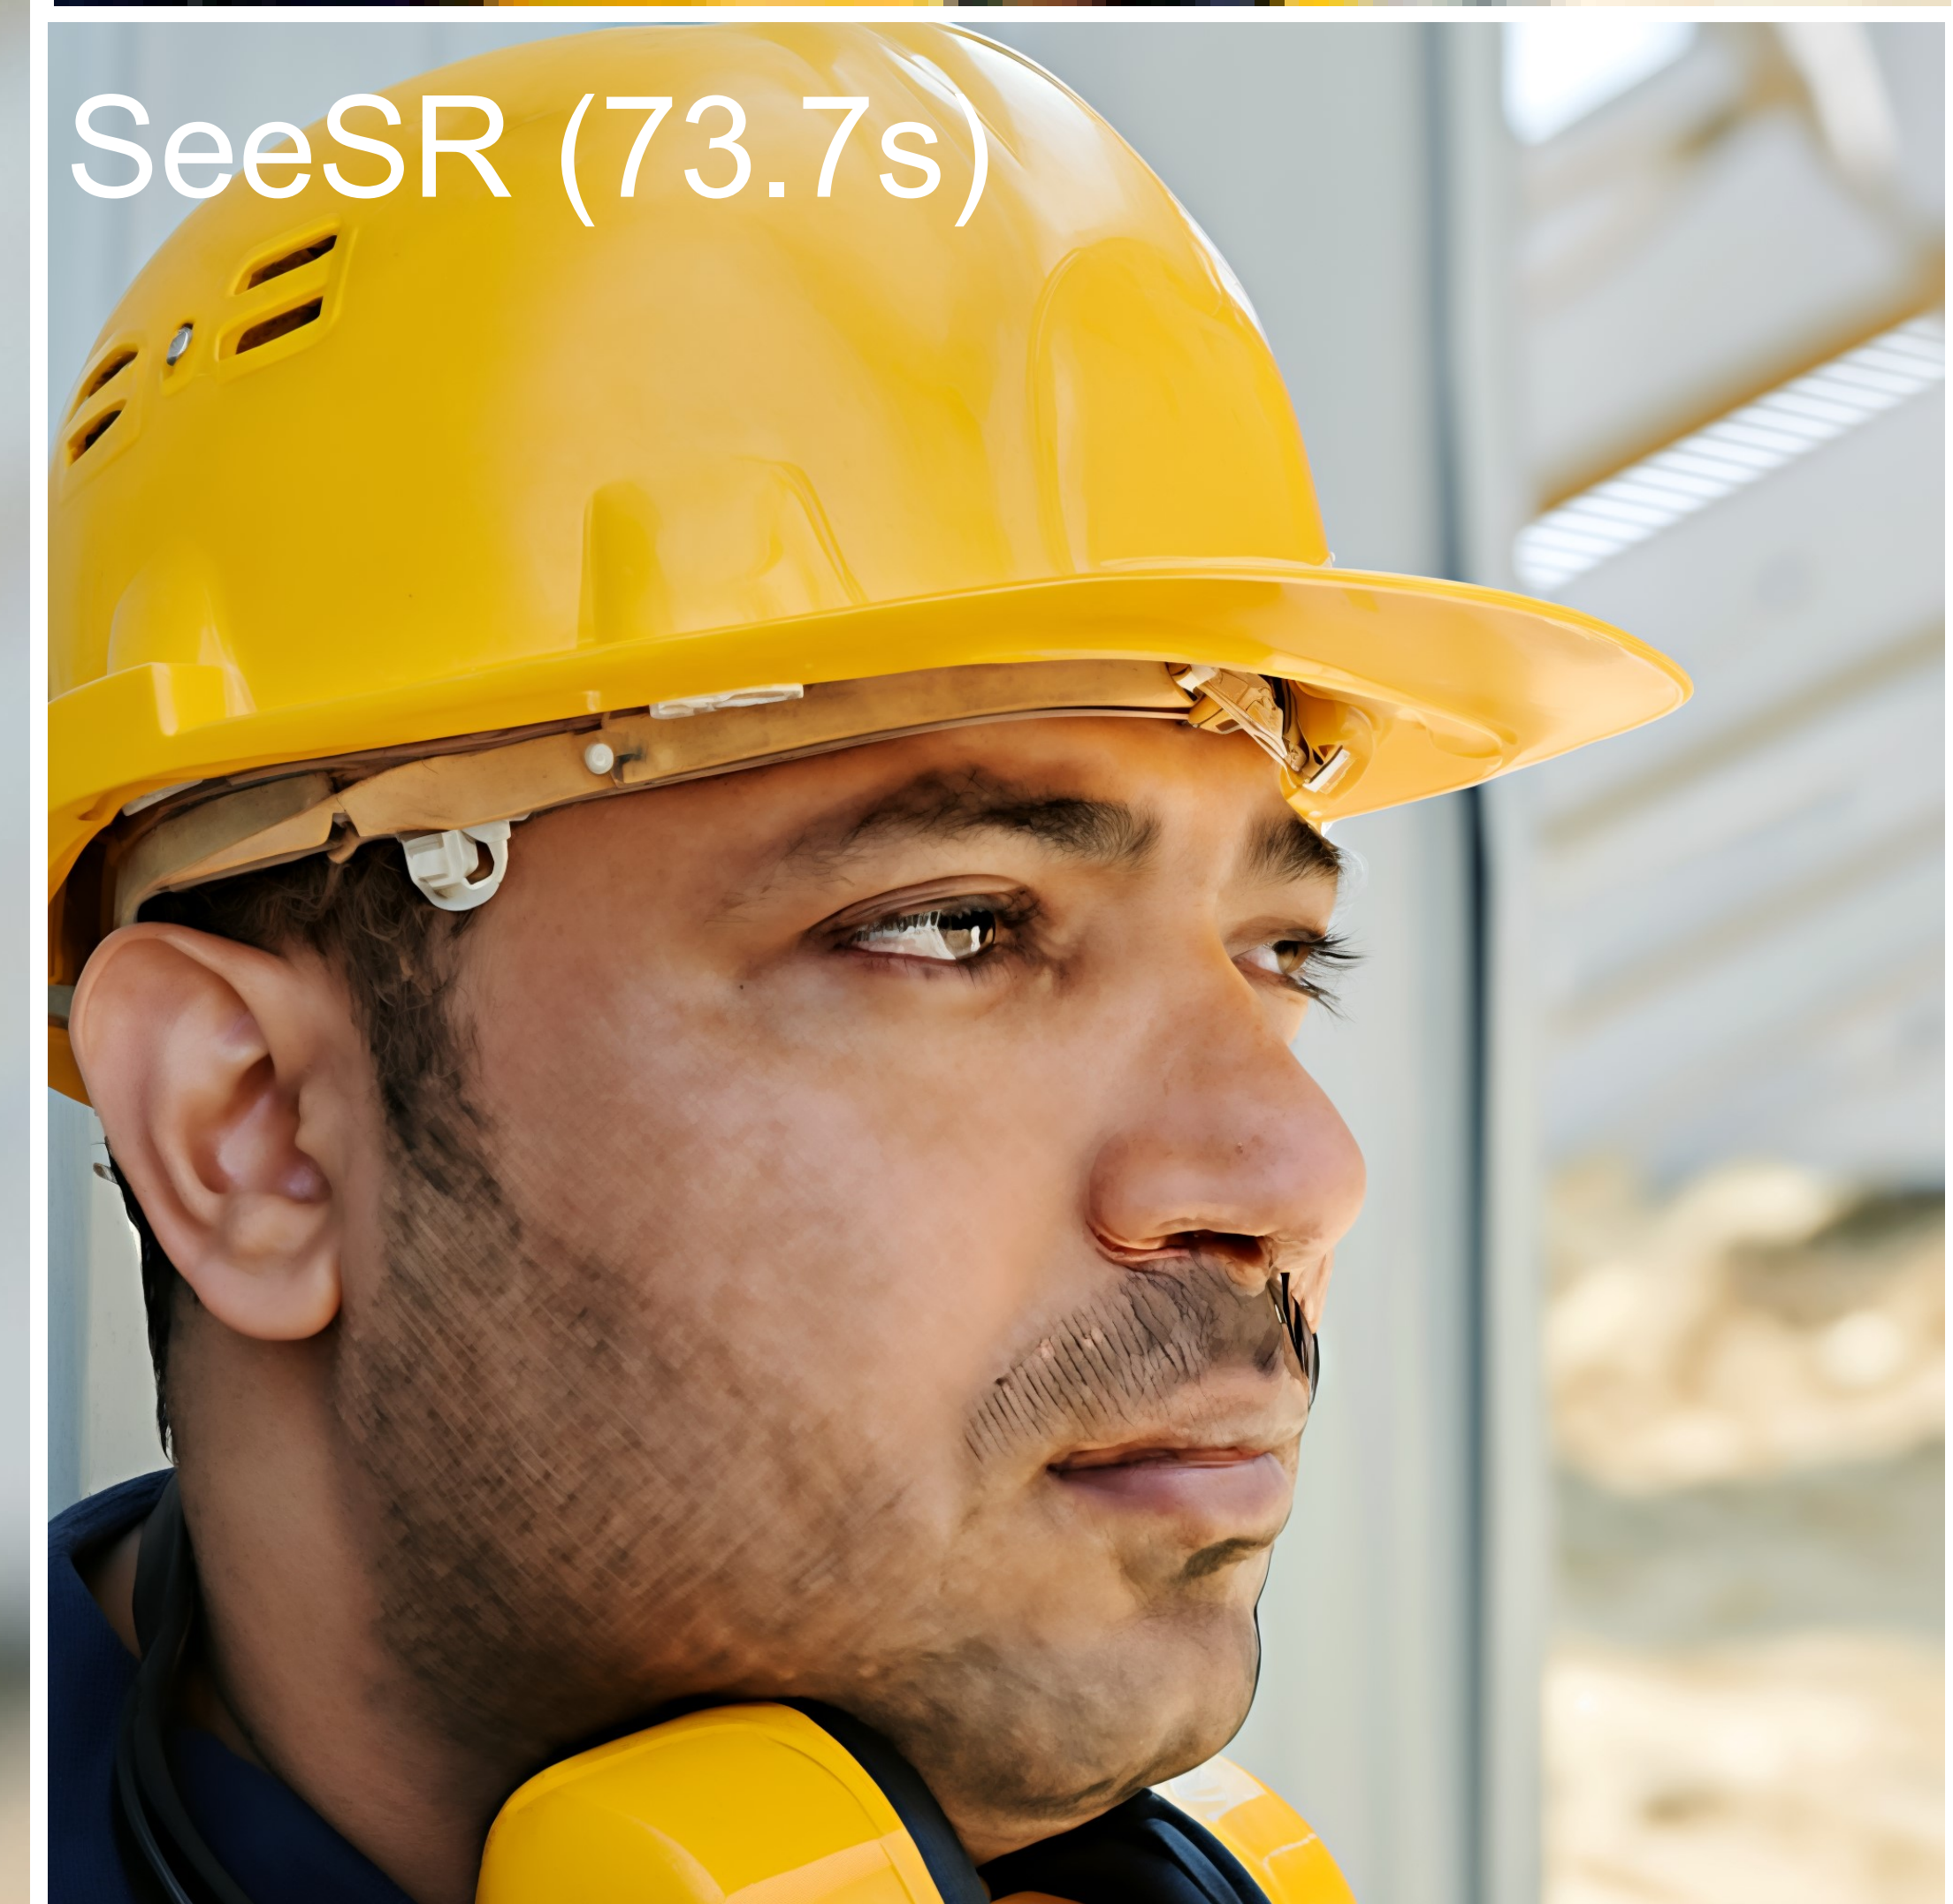

SeeSR (73.7s)

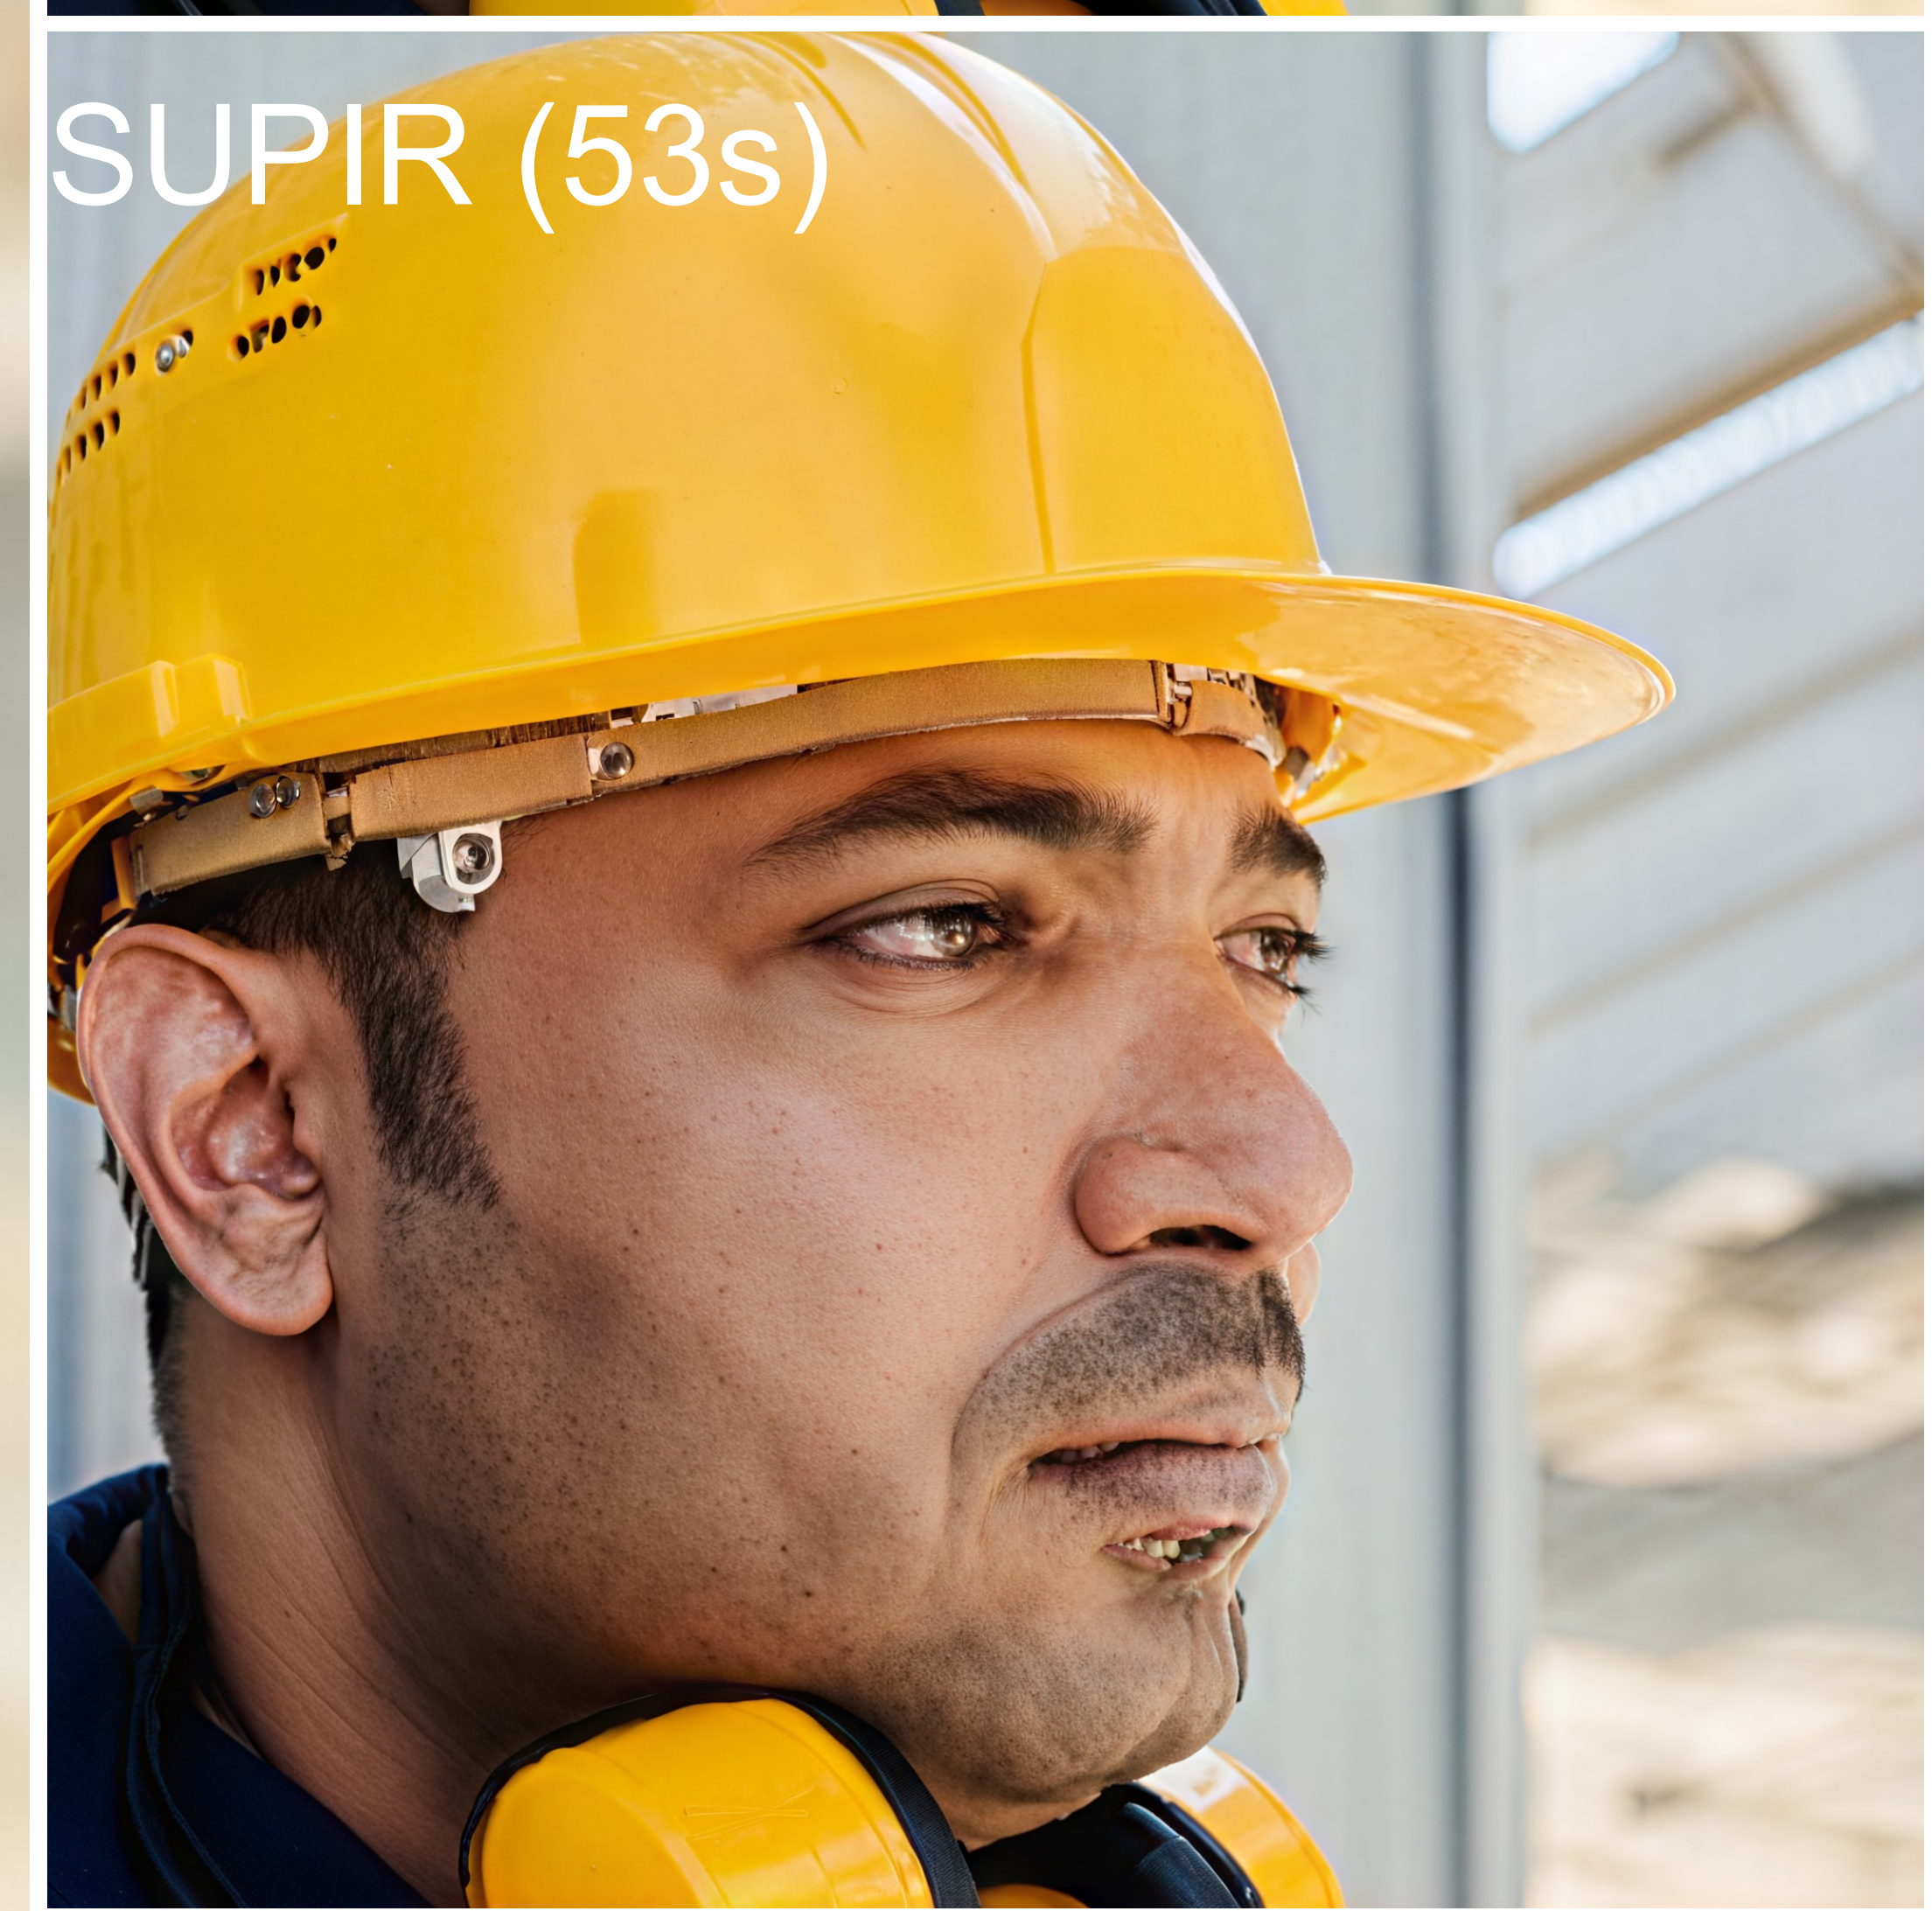

SUPIR (53s)

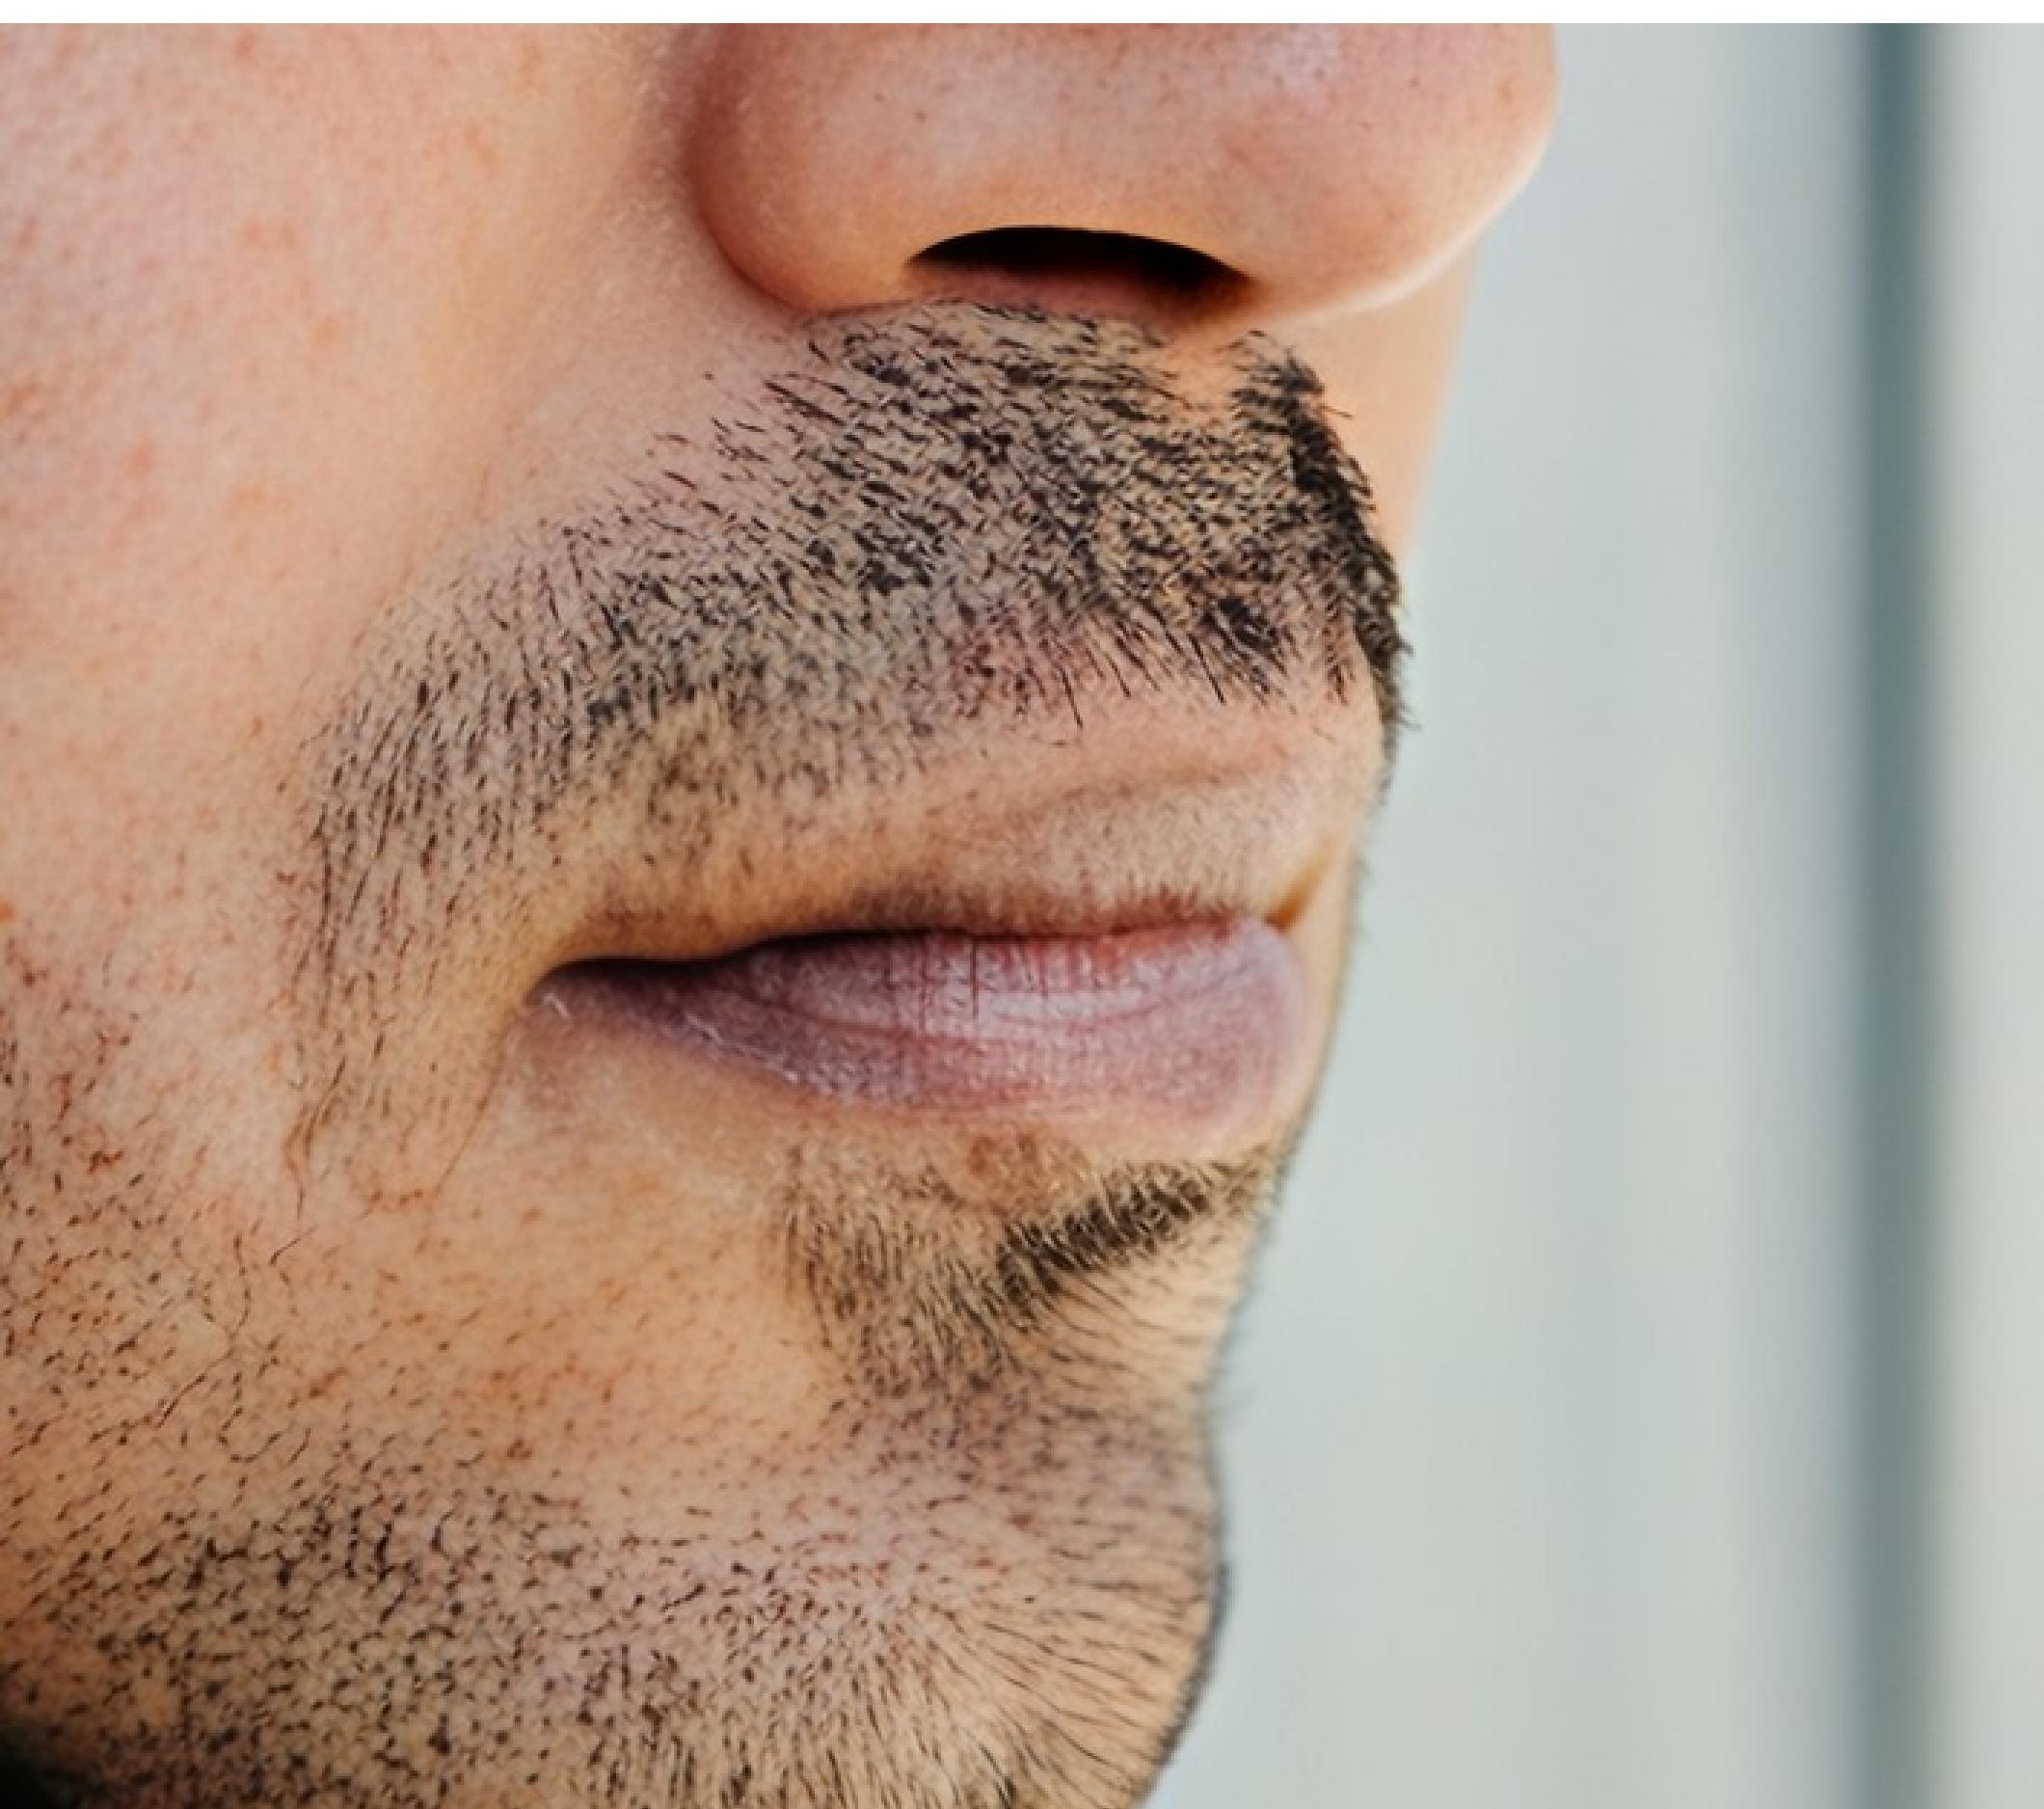

Ours

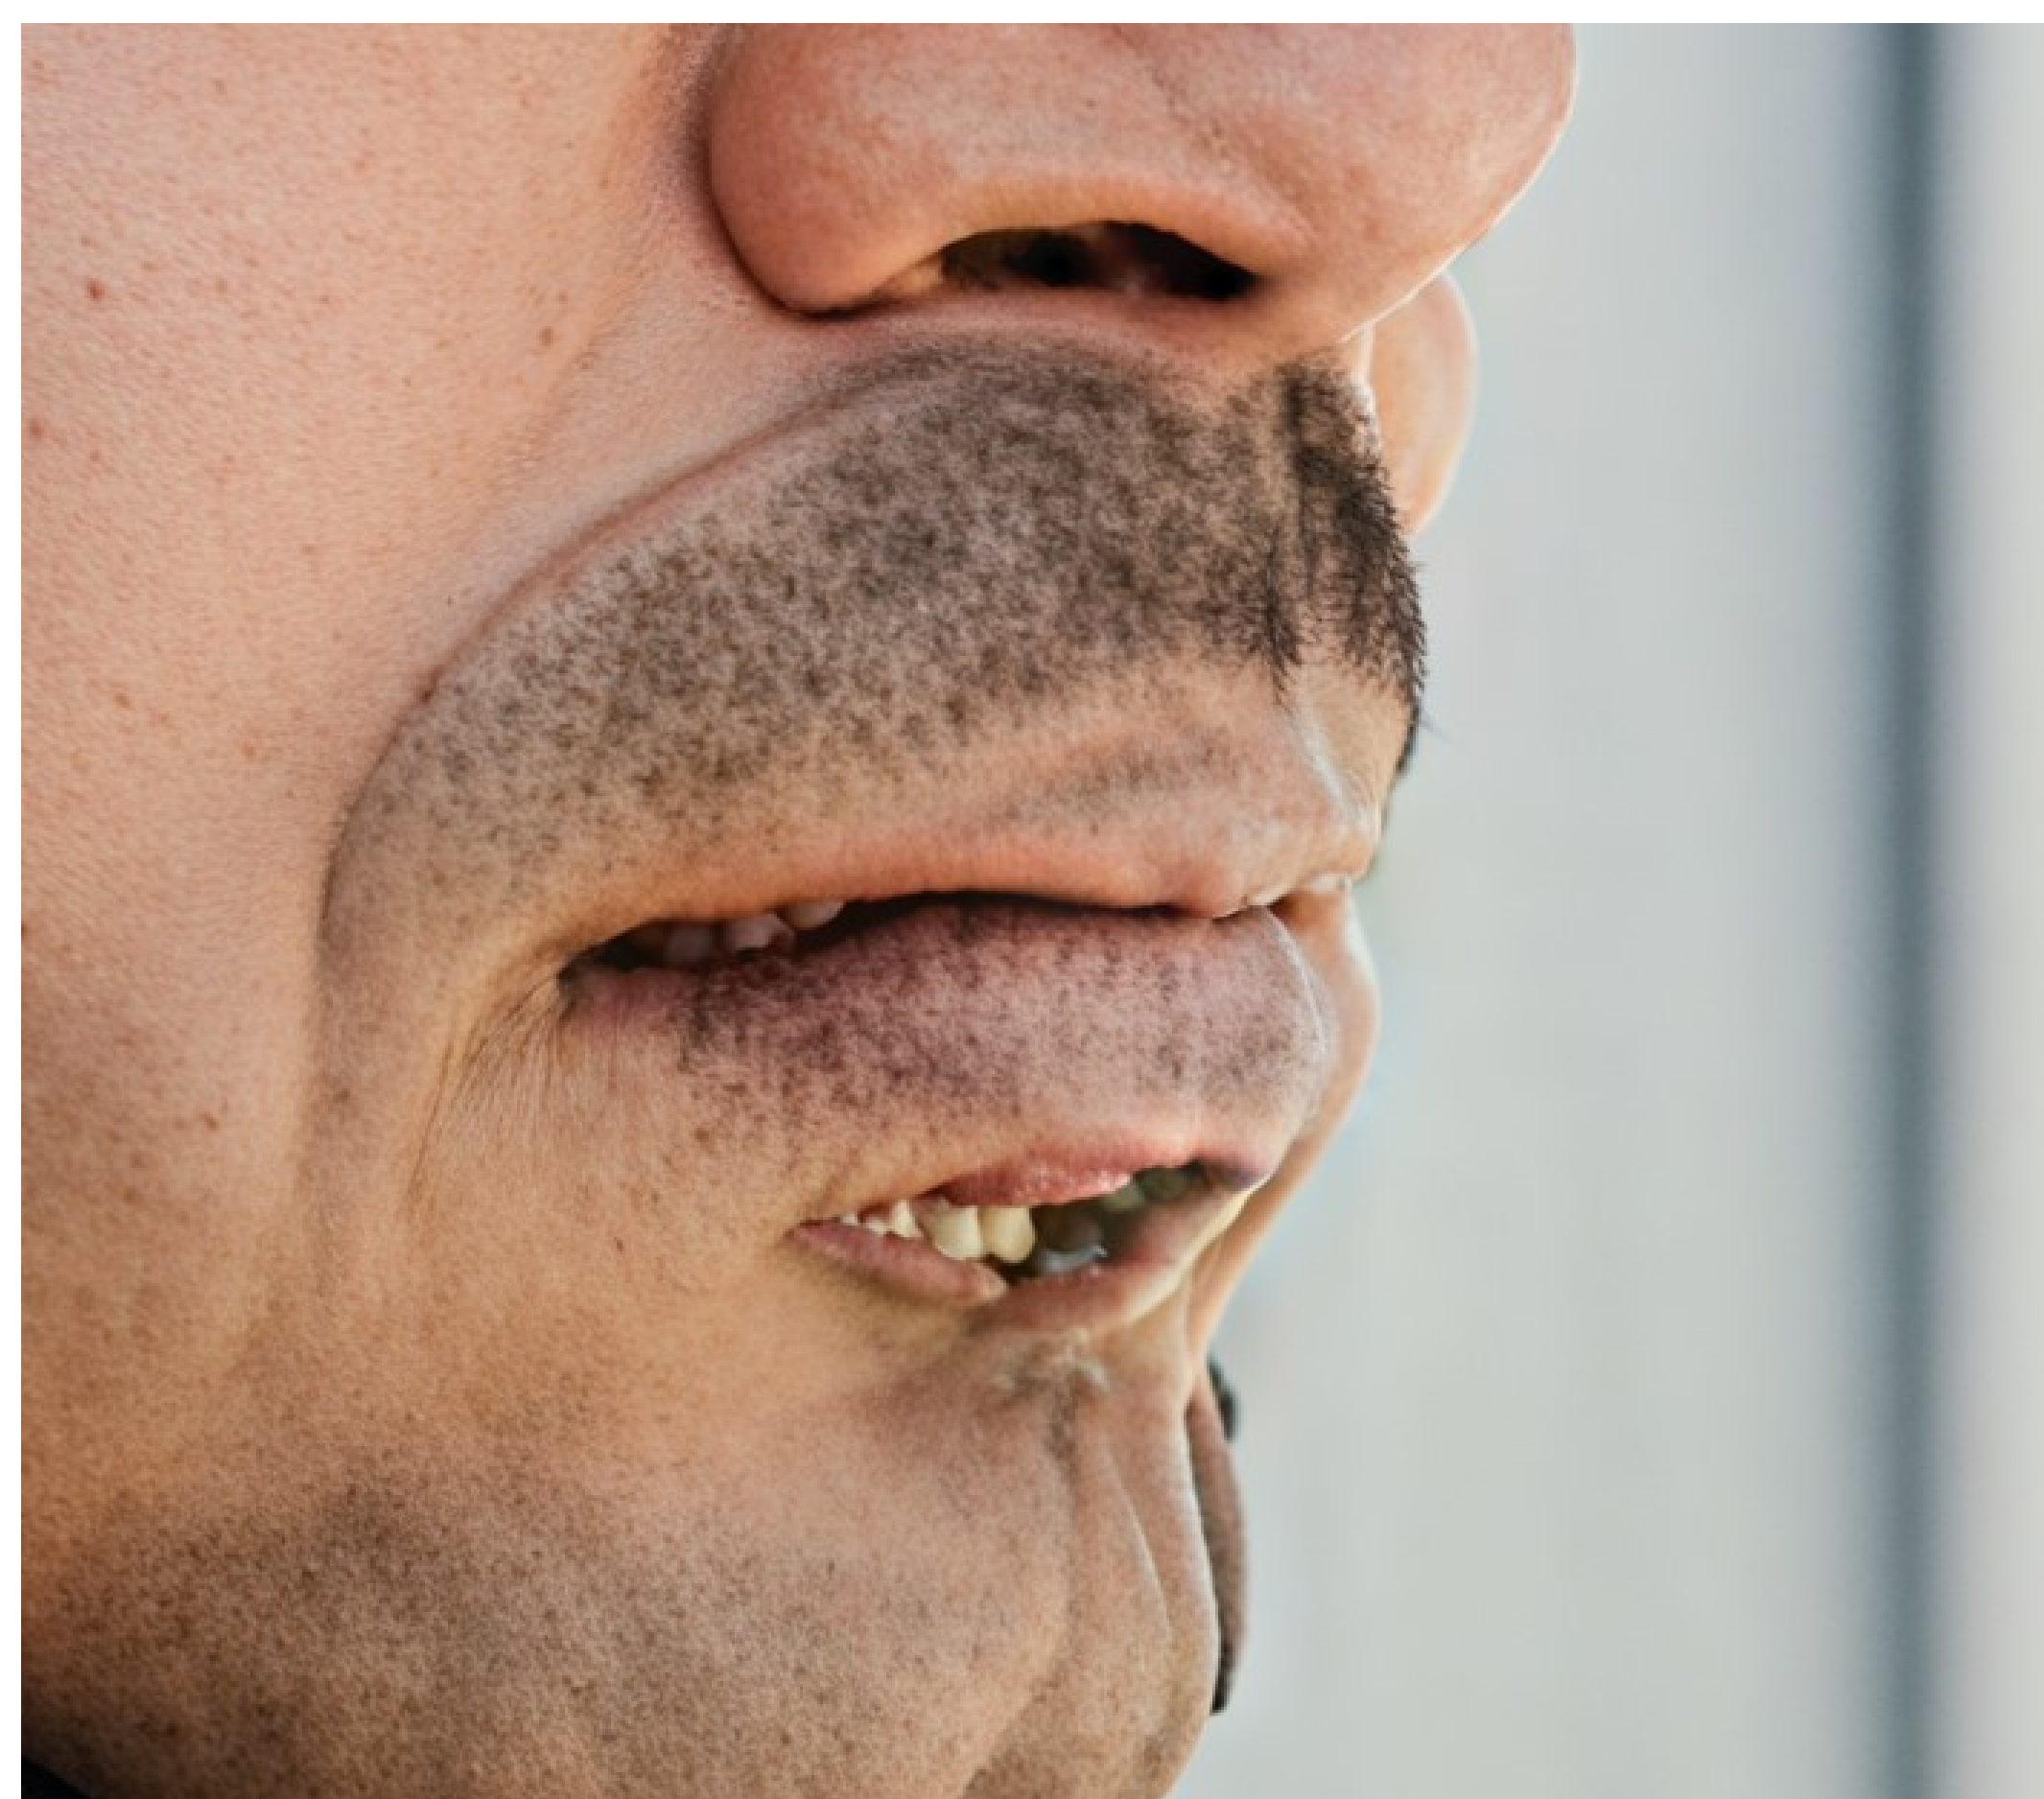

SUPIR

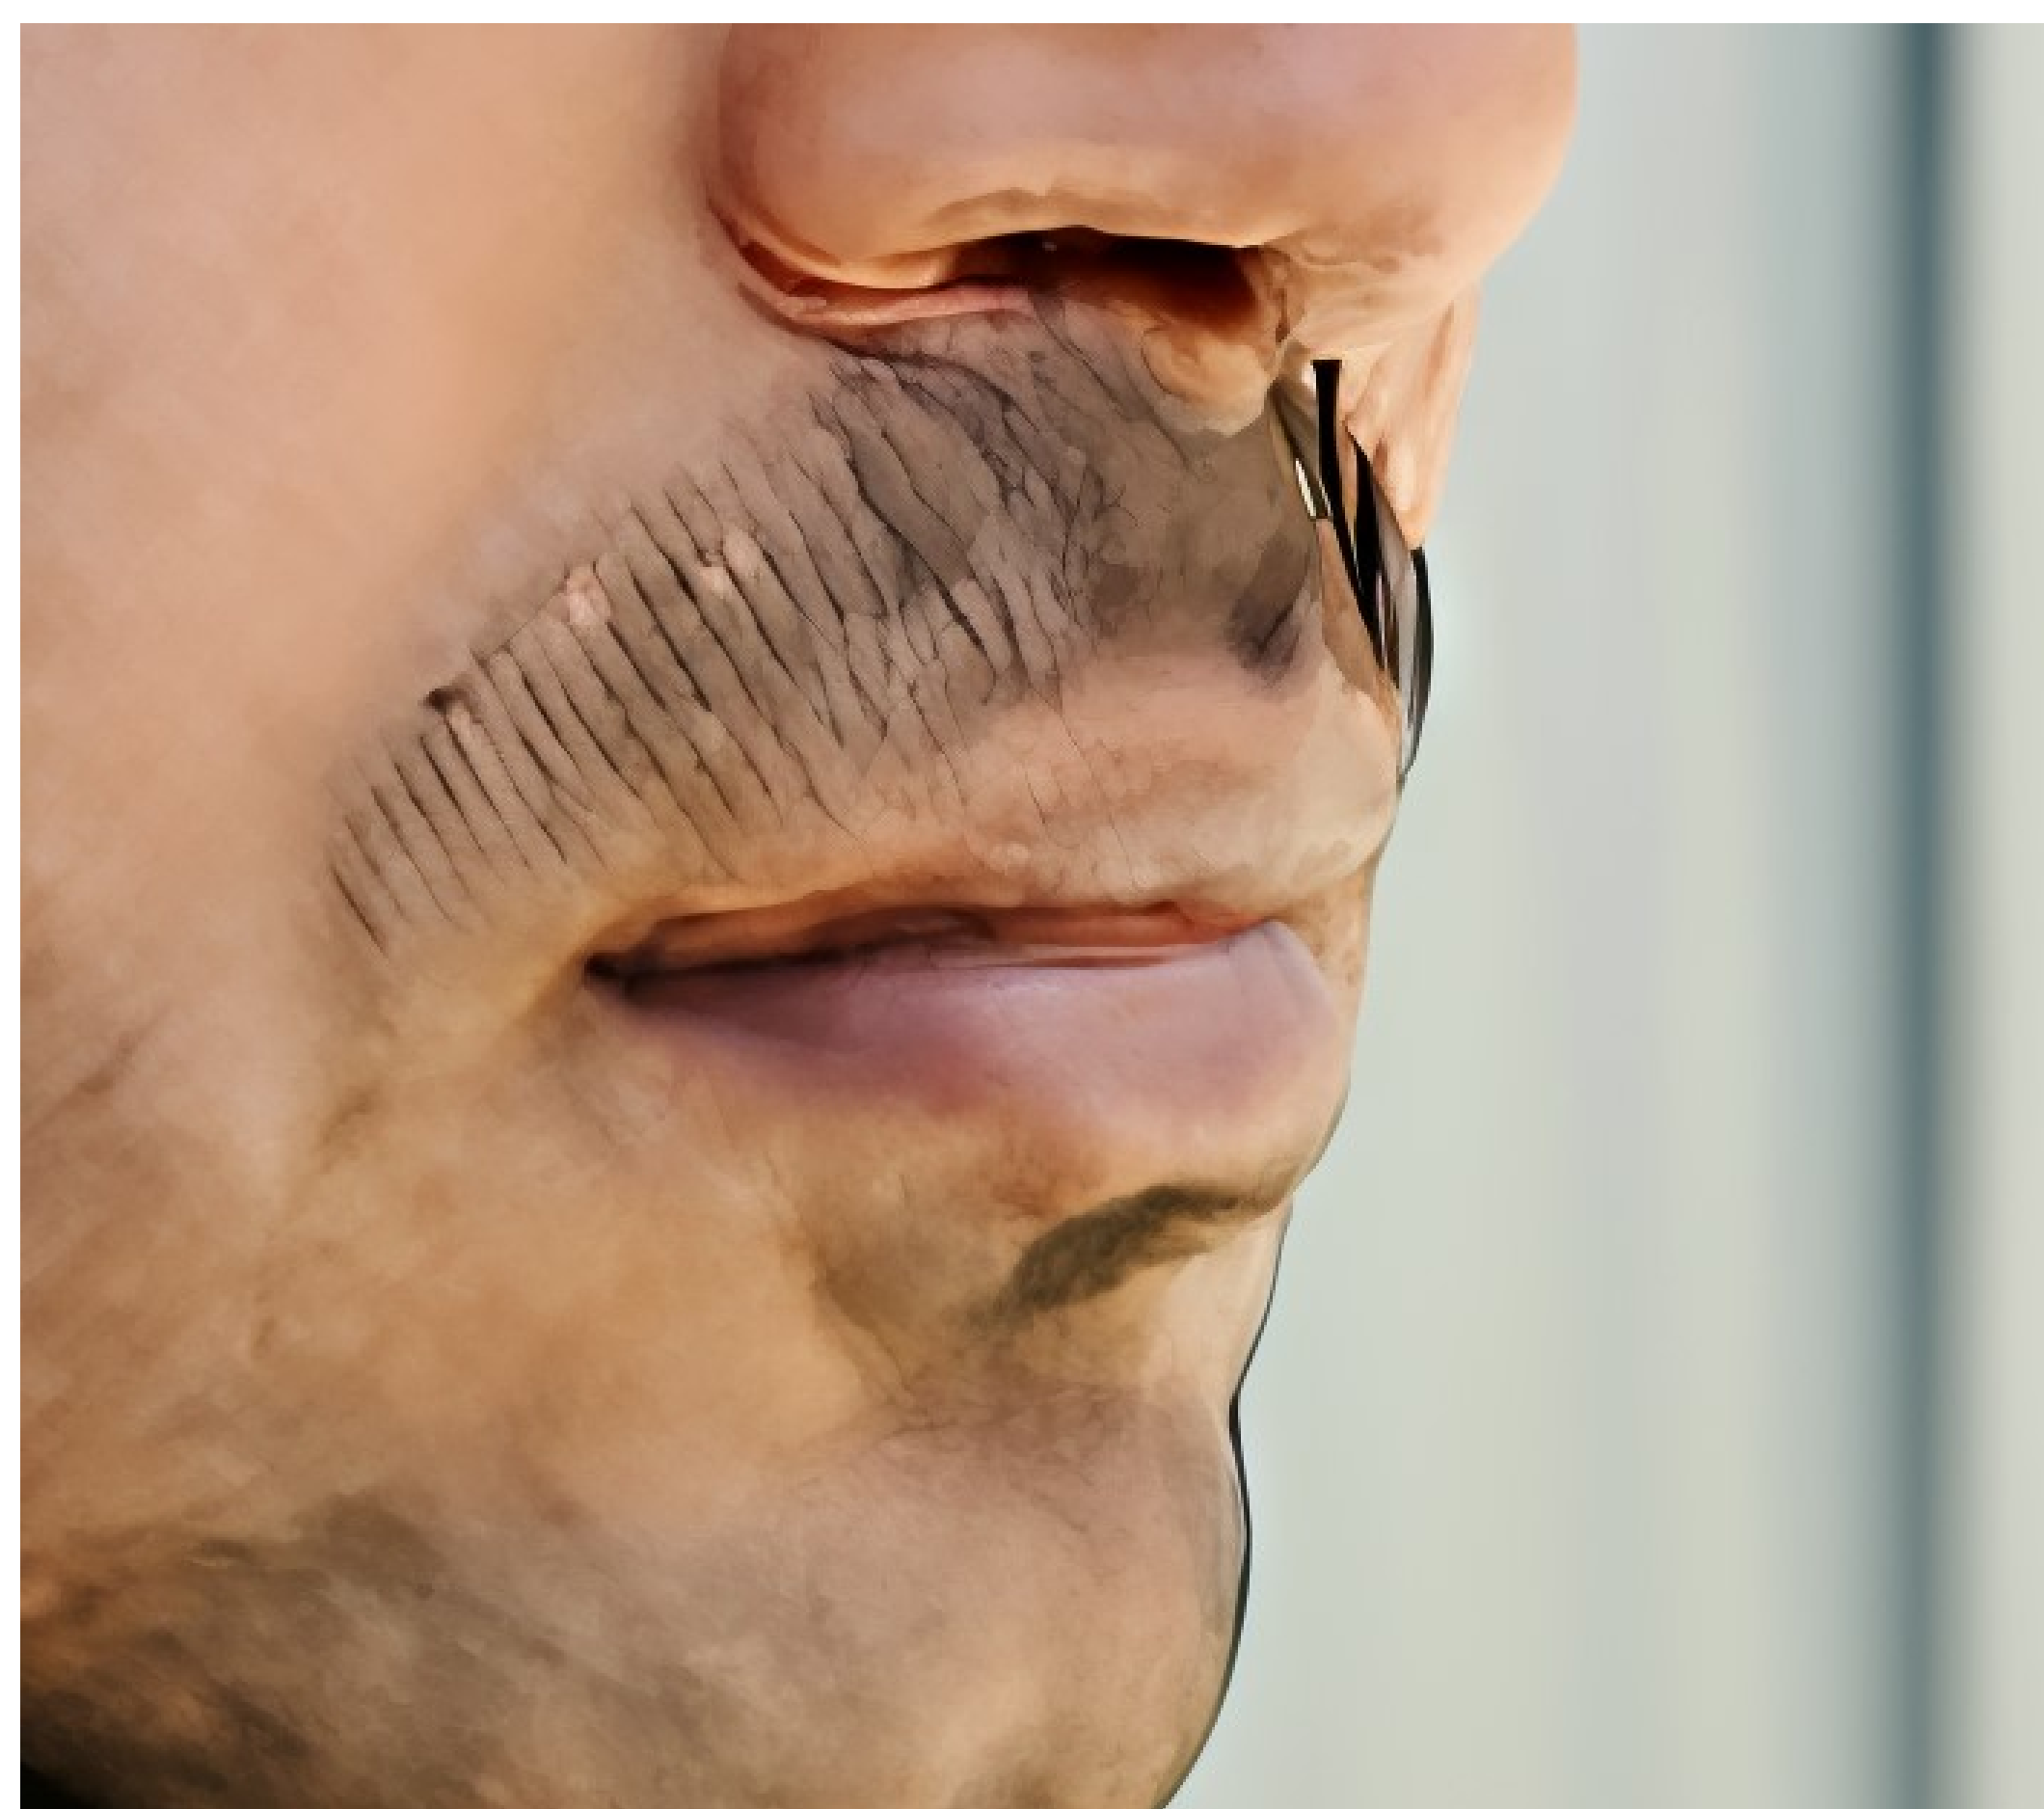

SeeSR

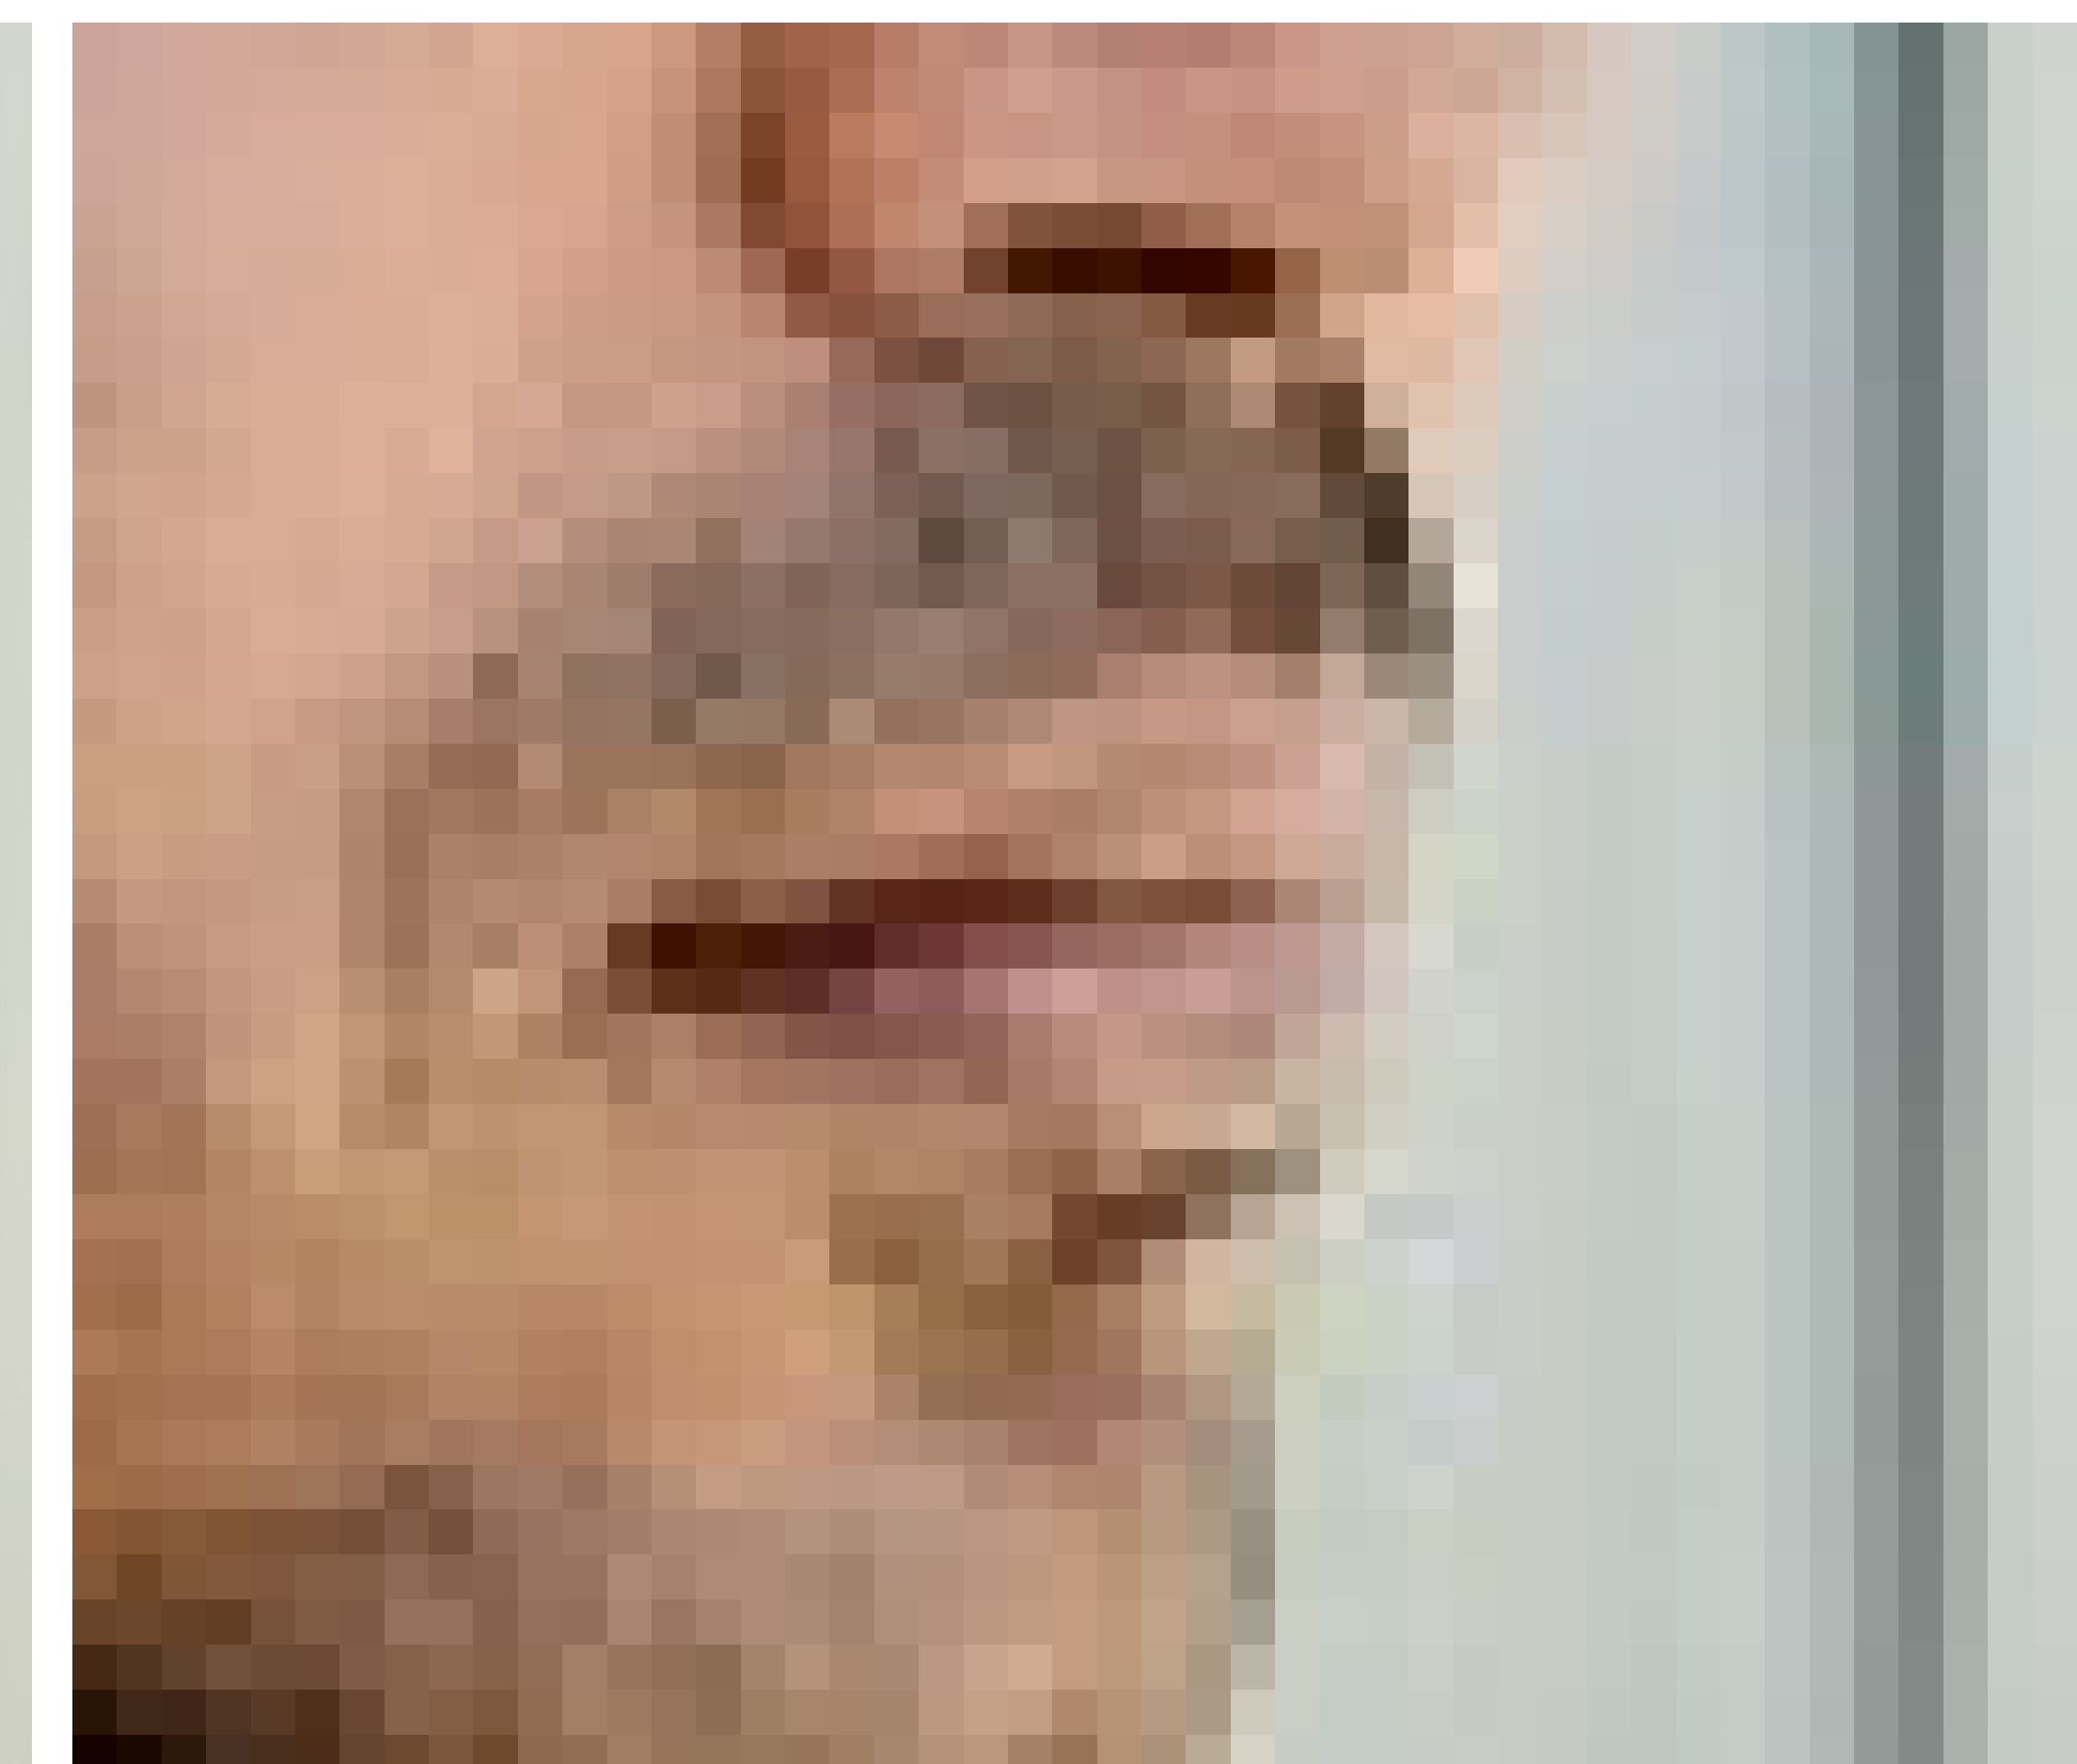

Input



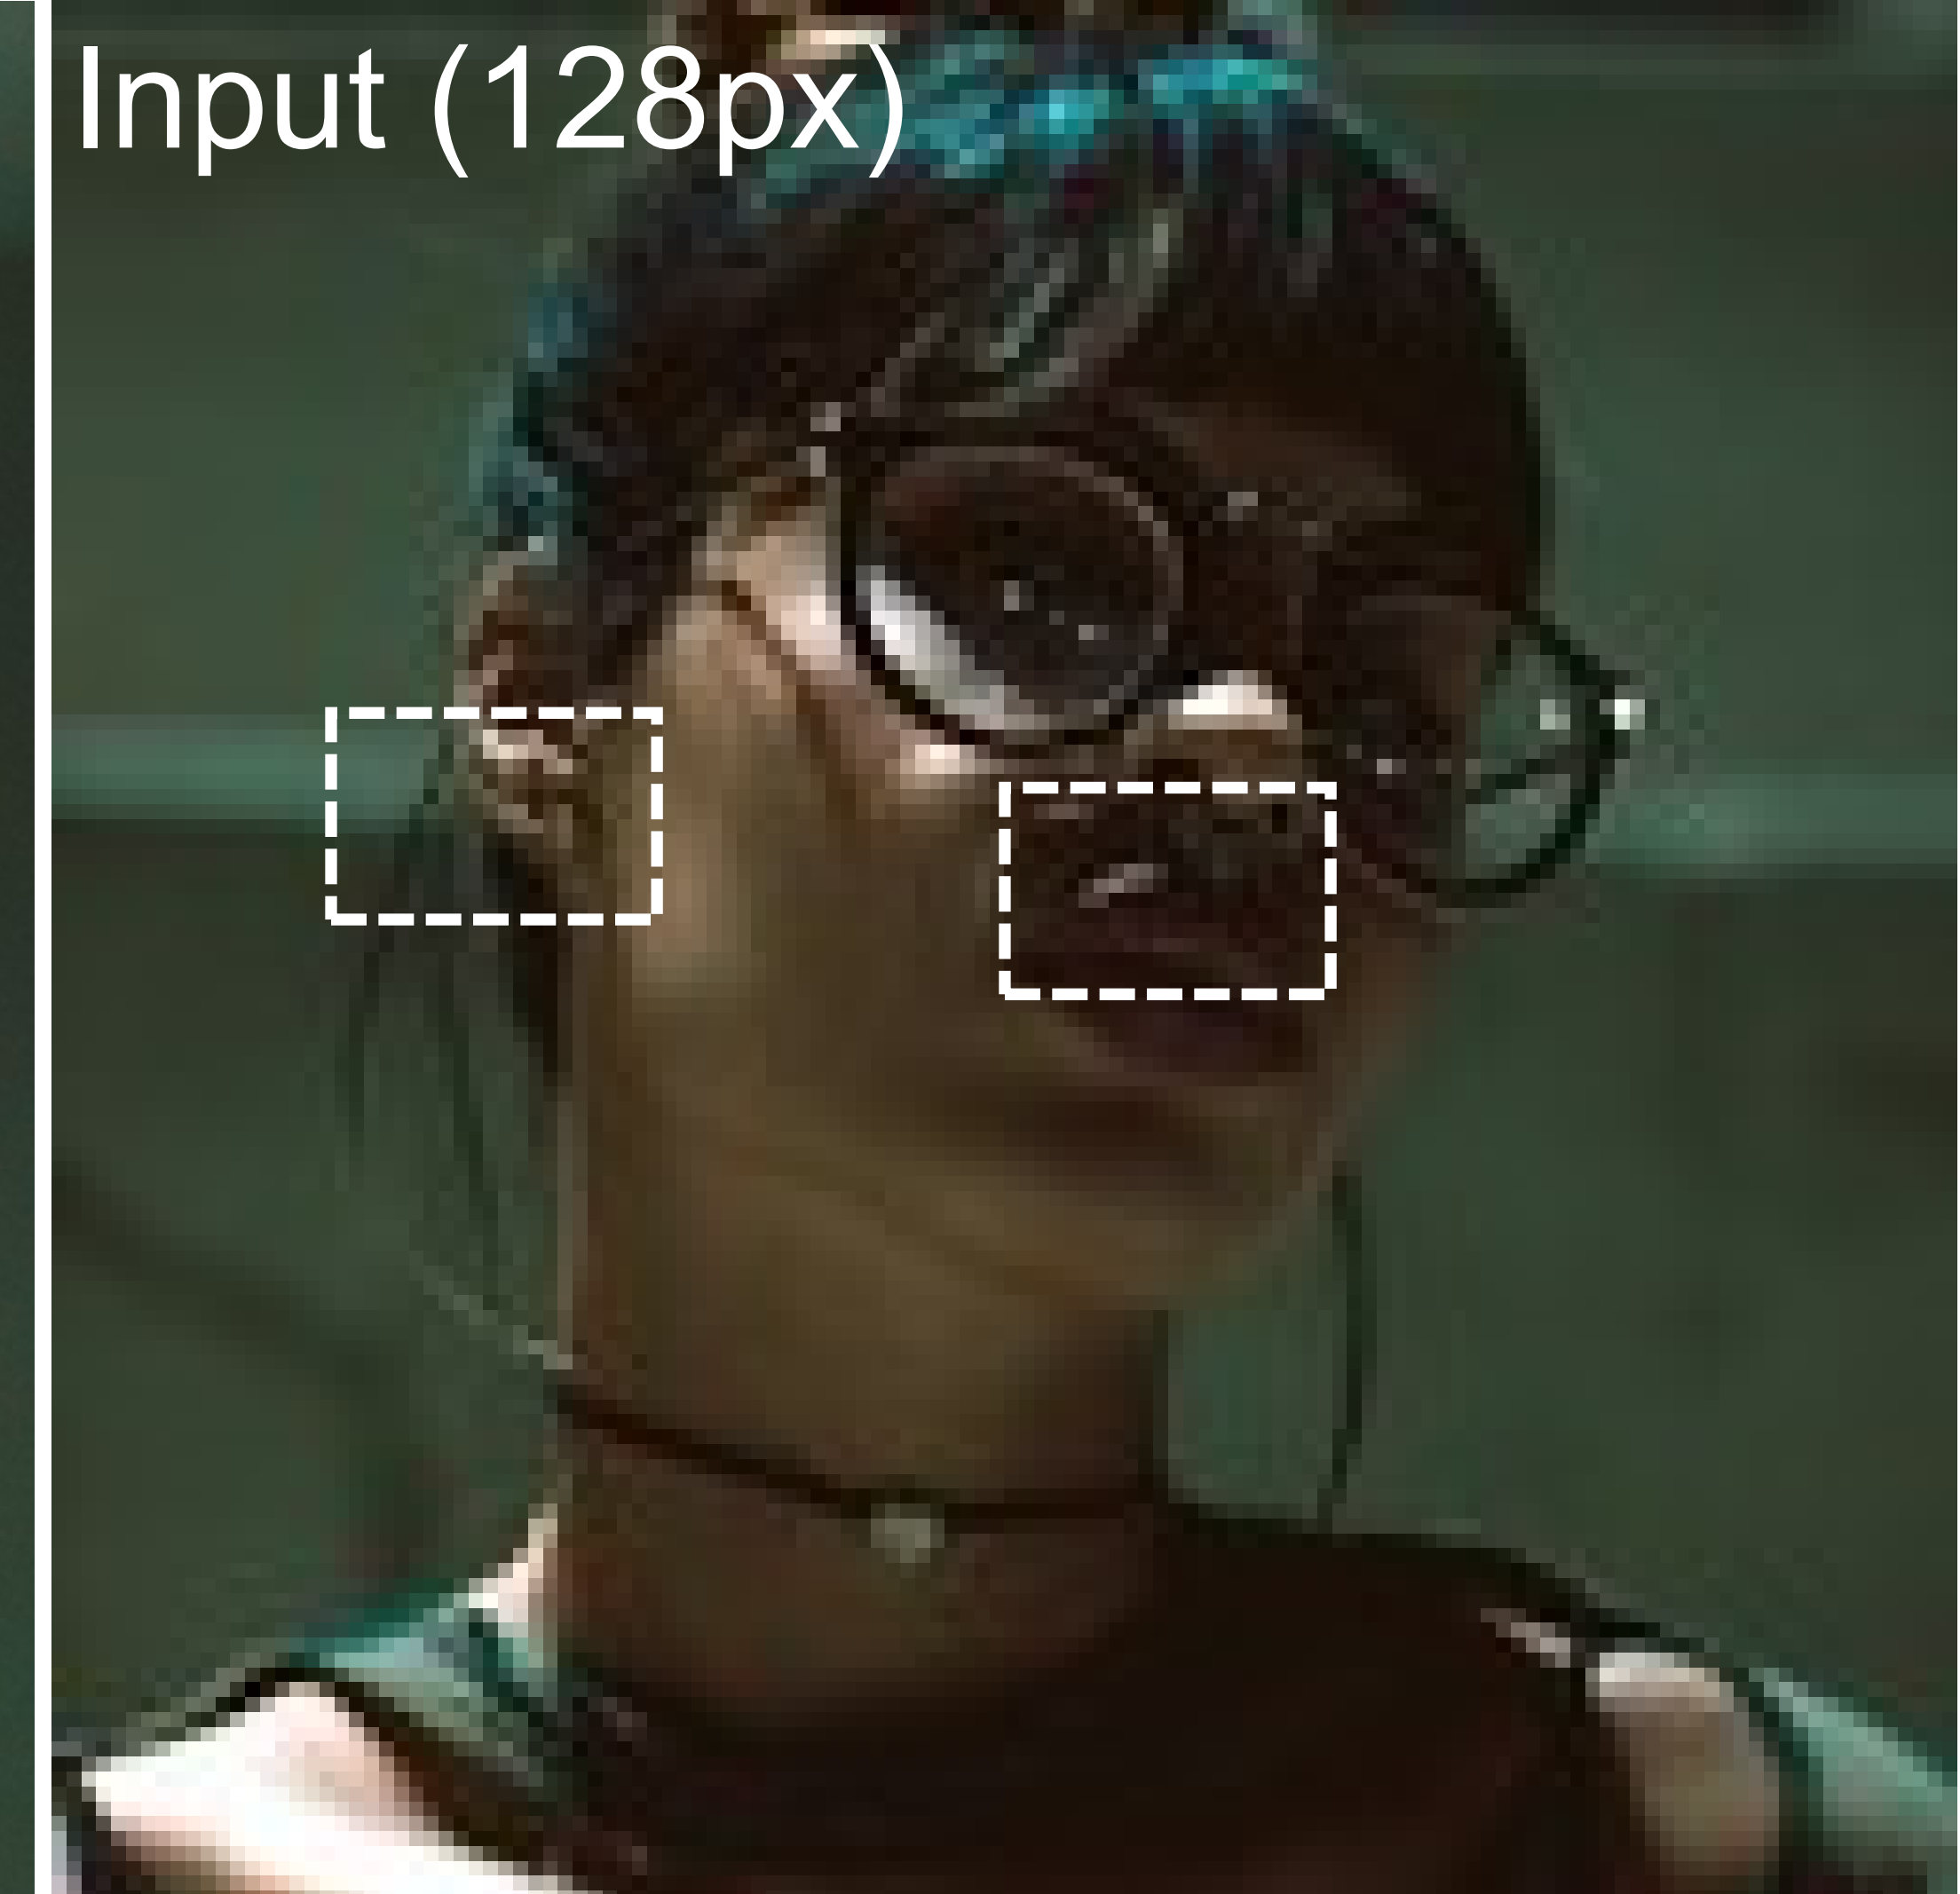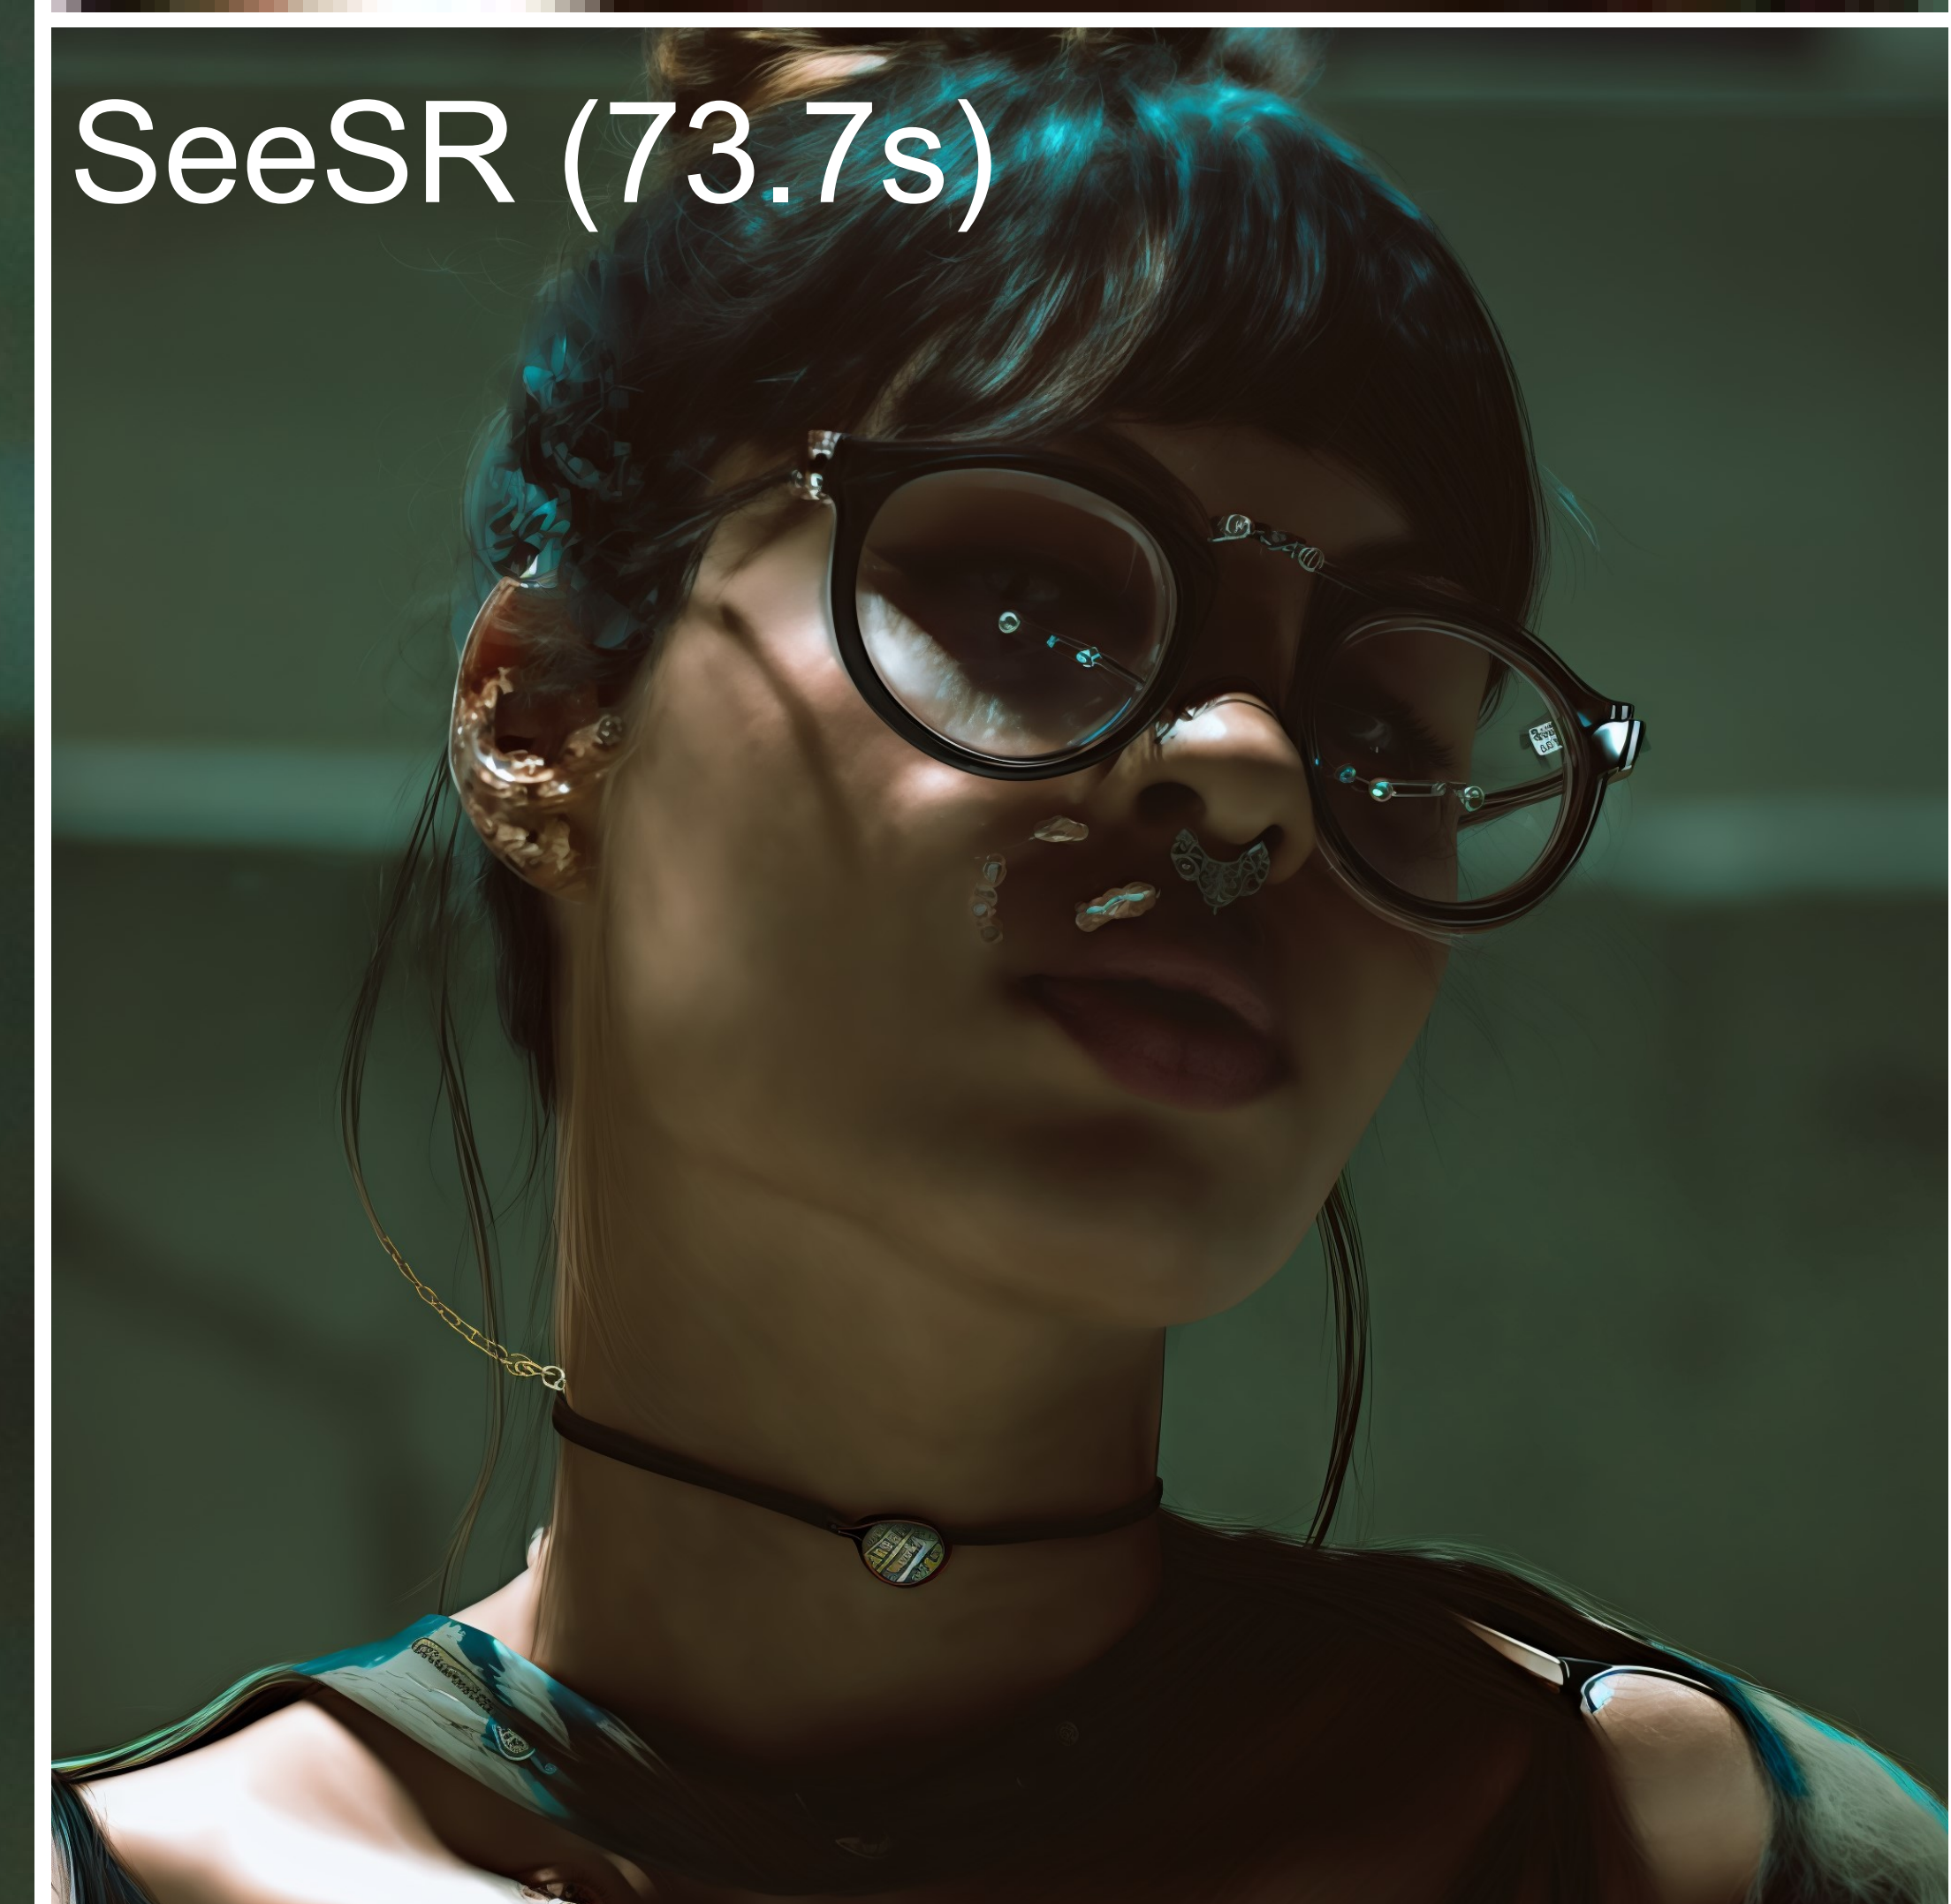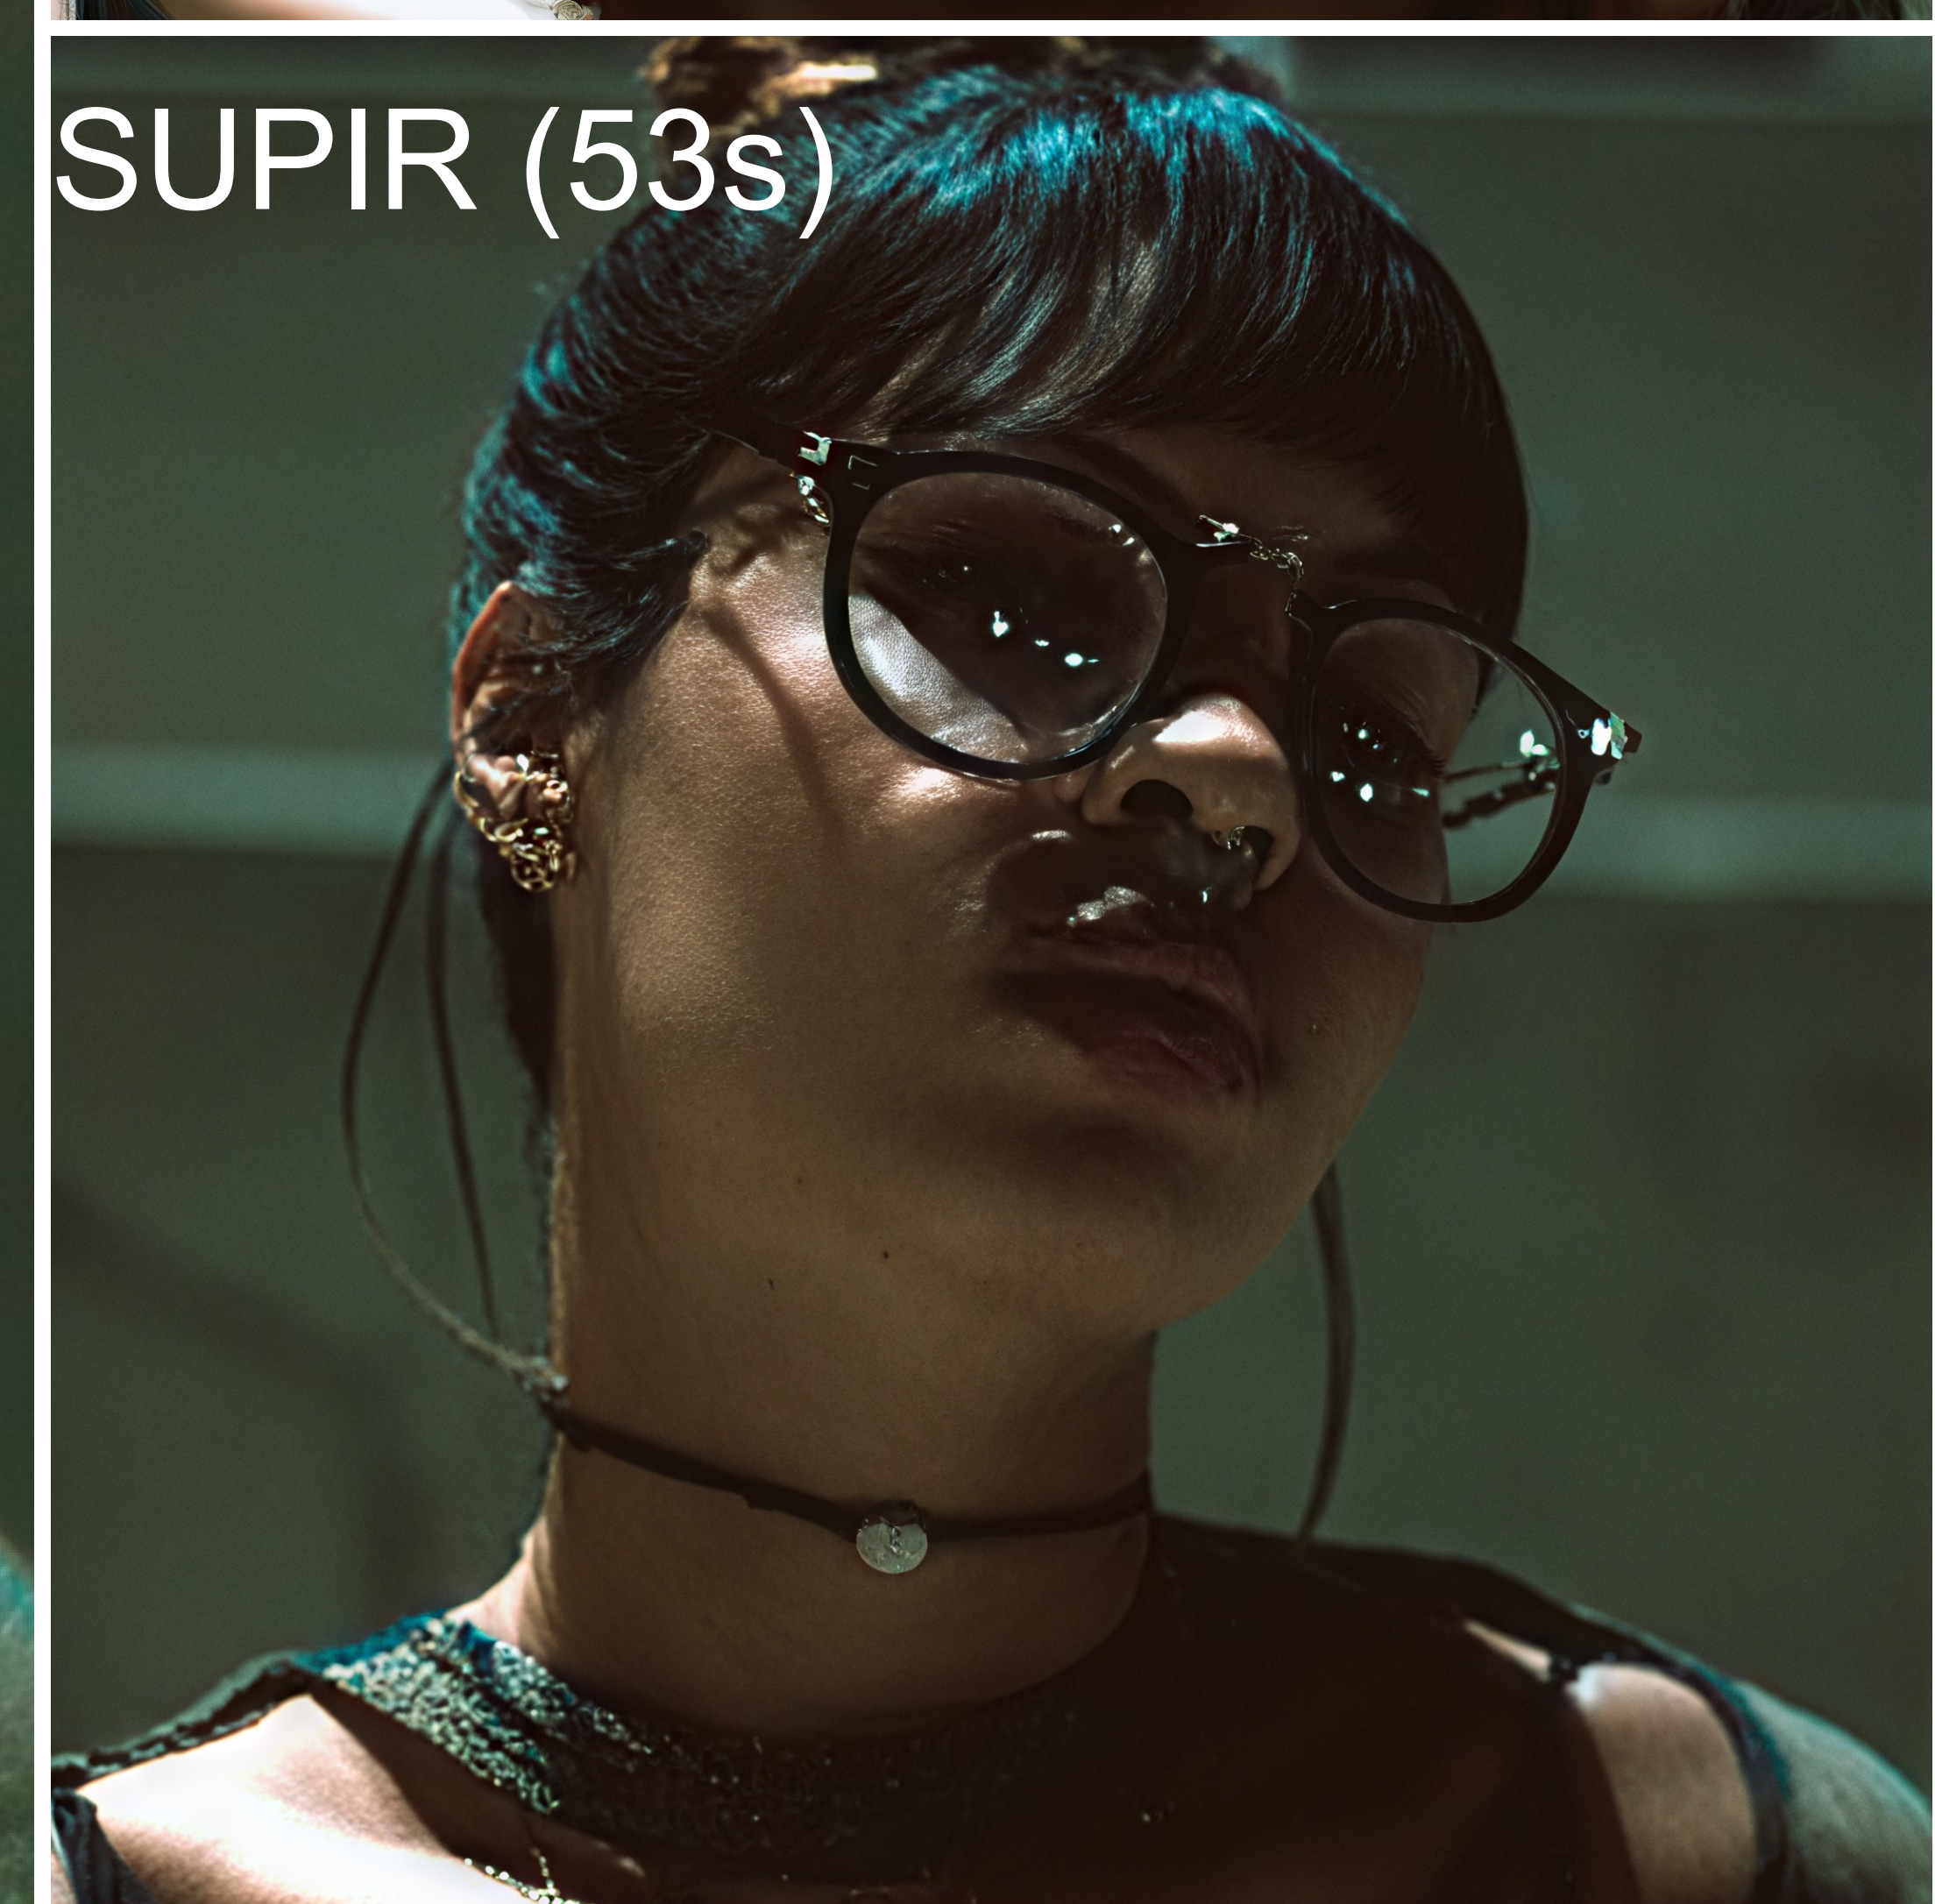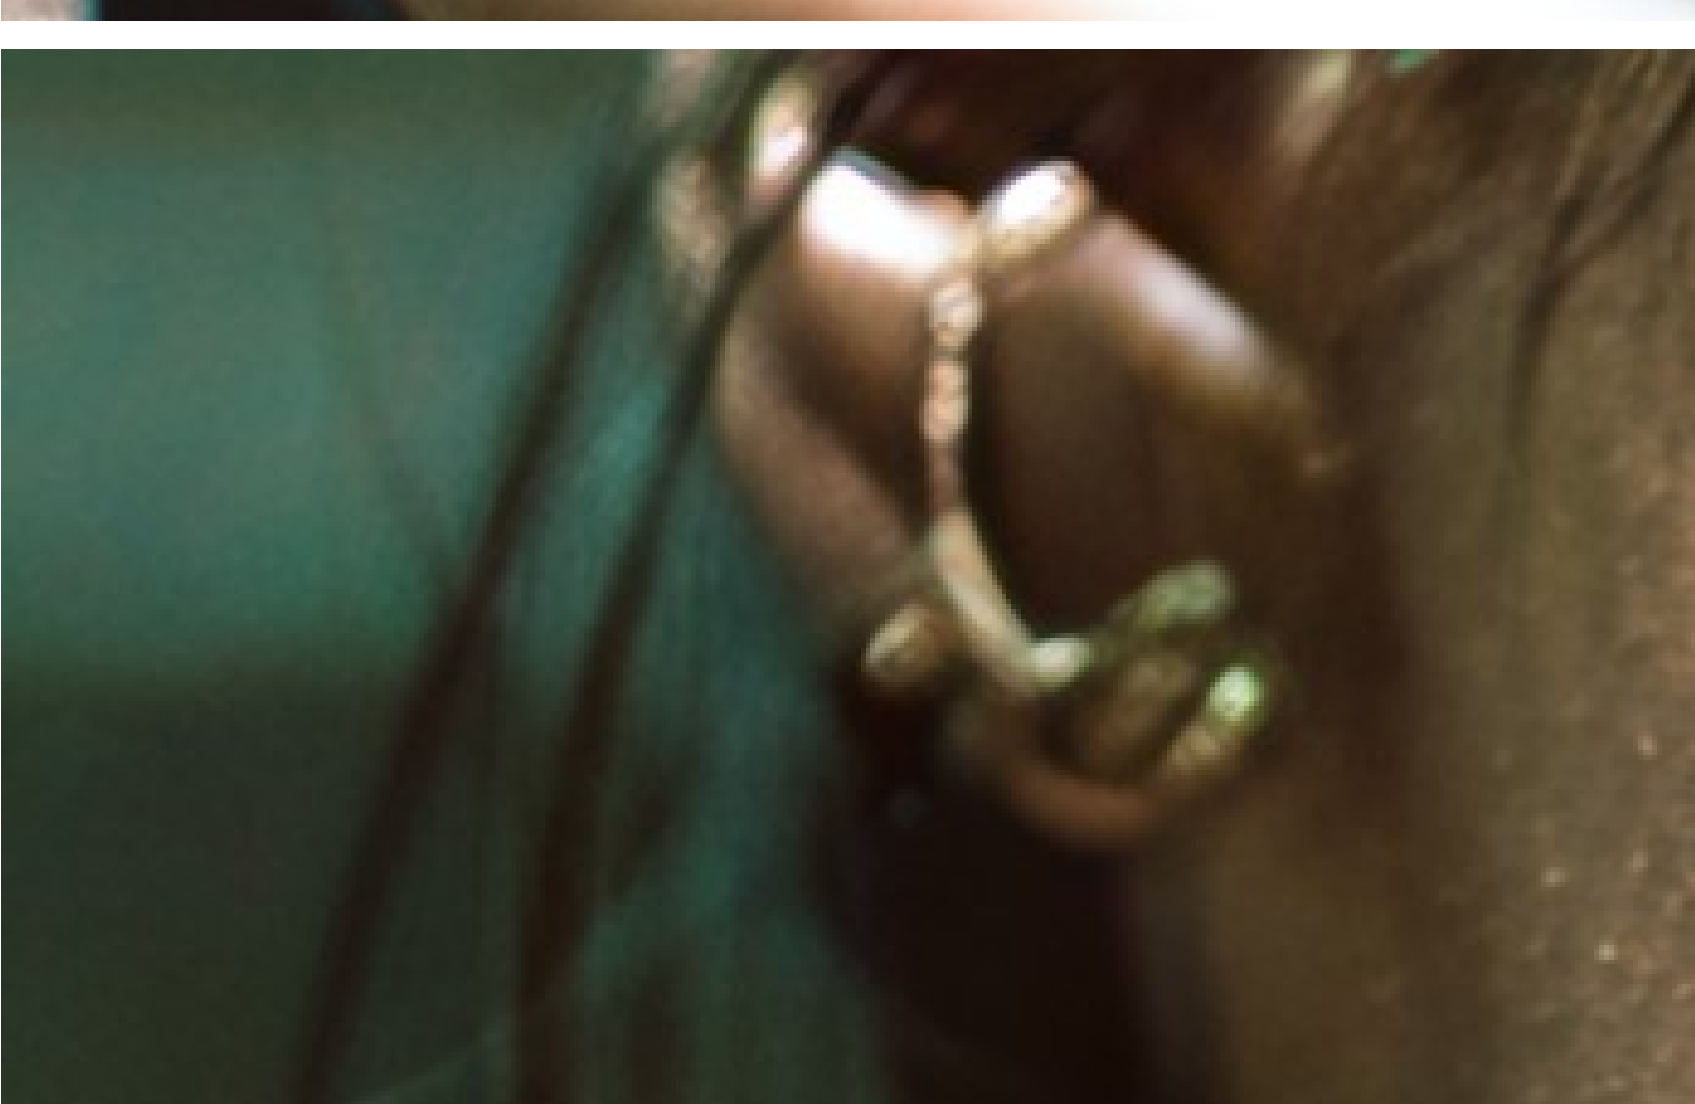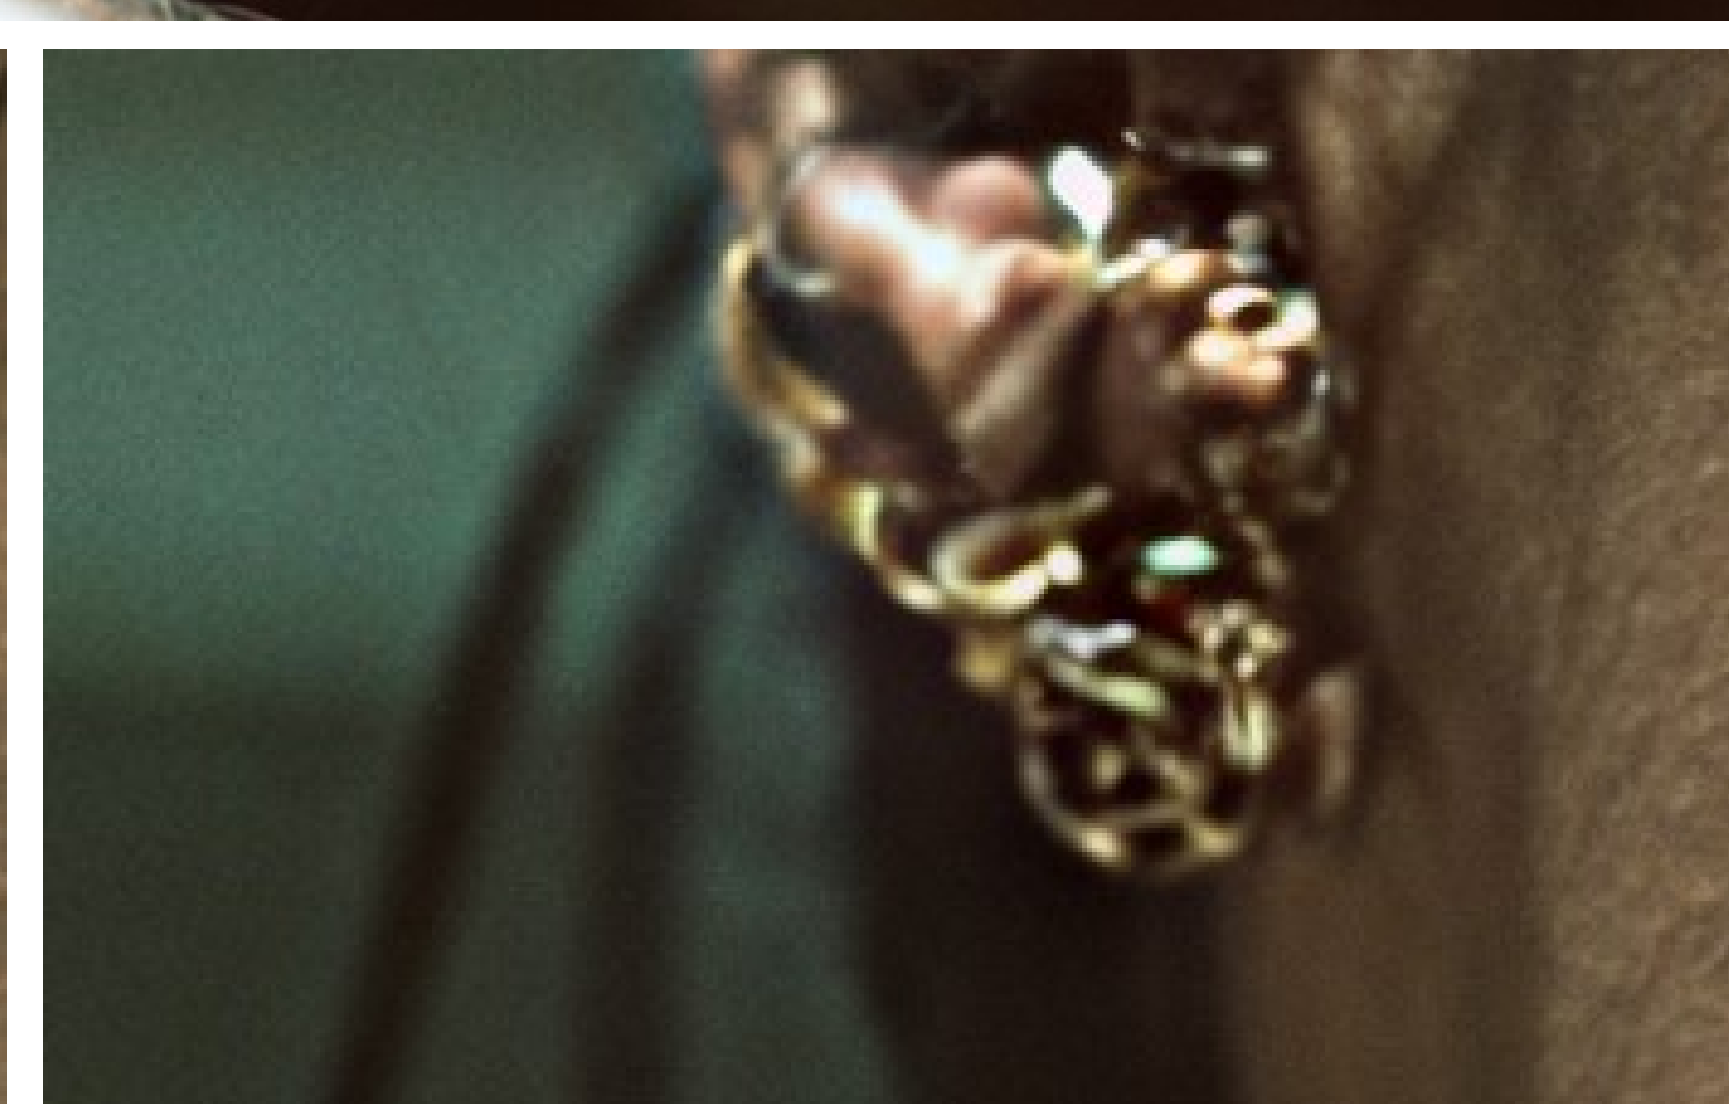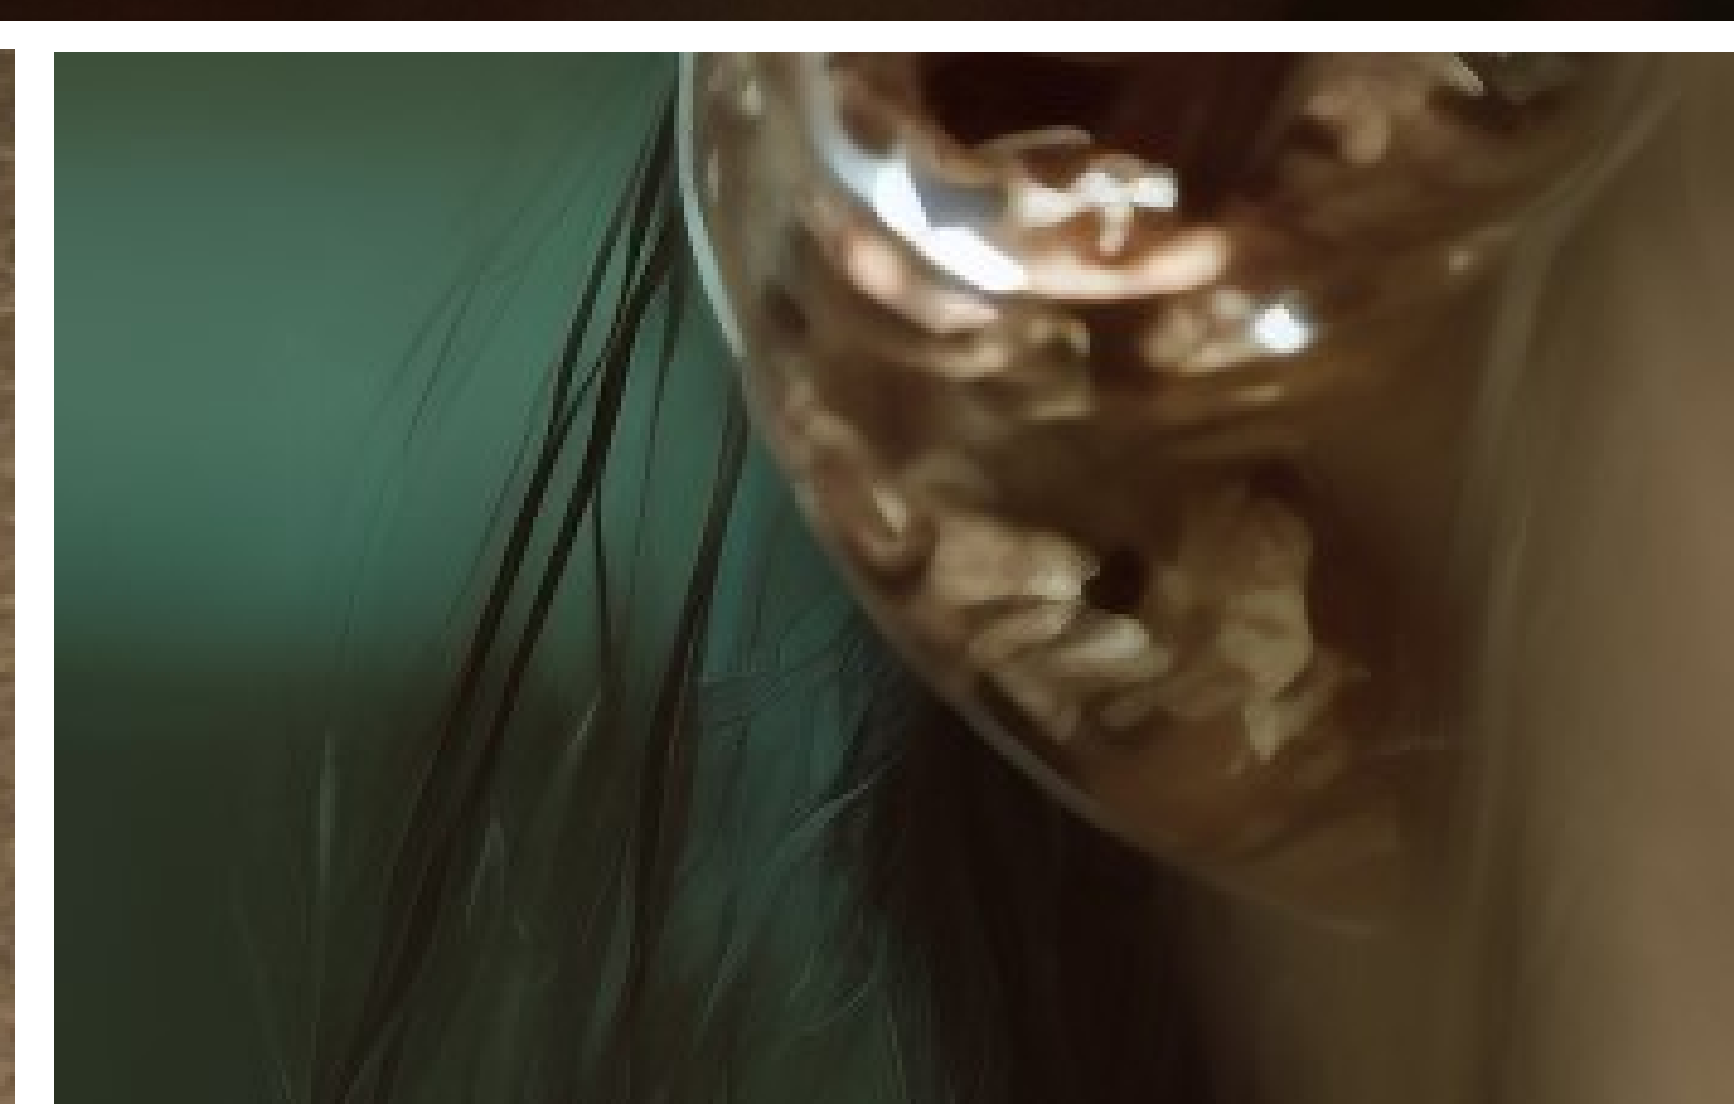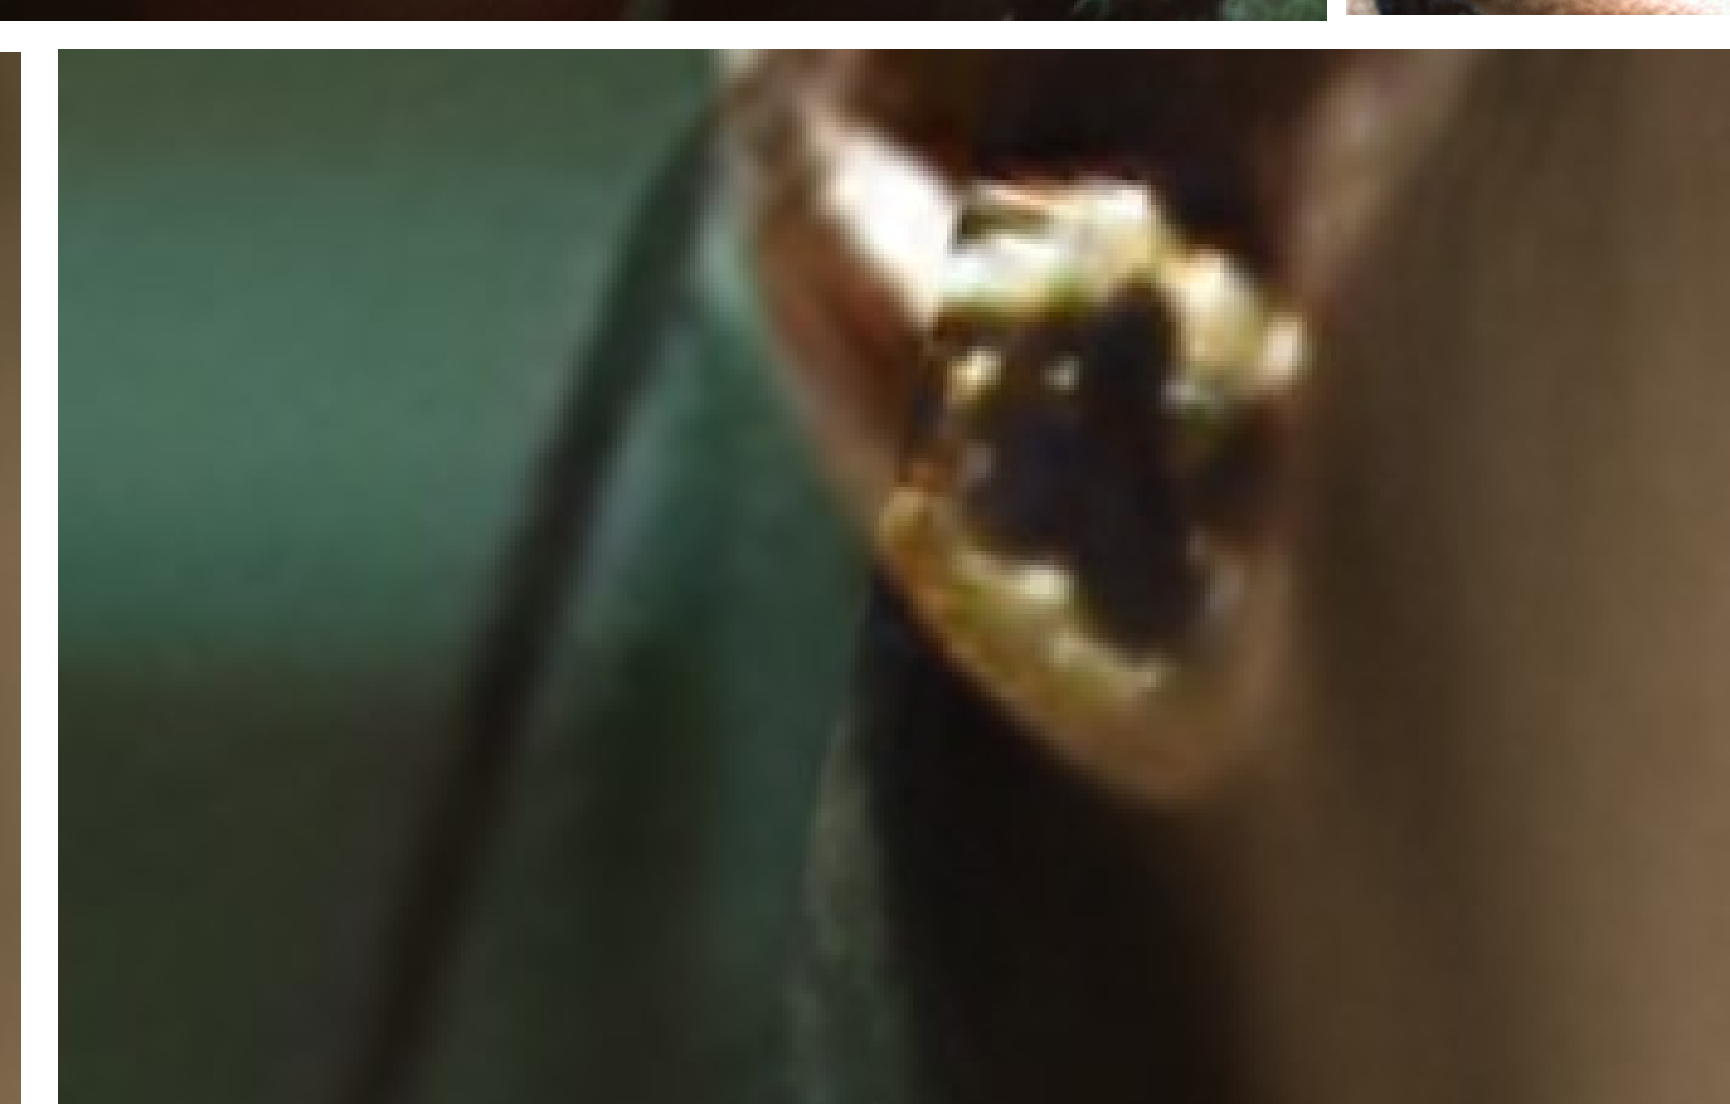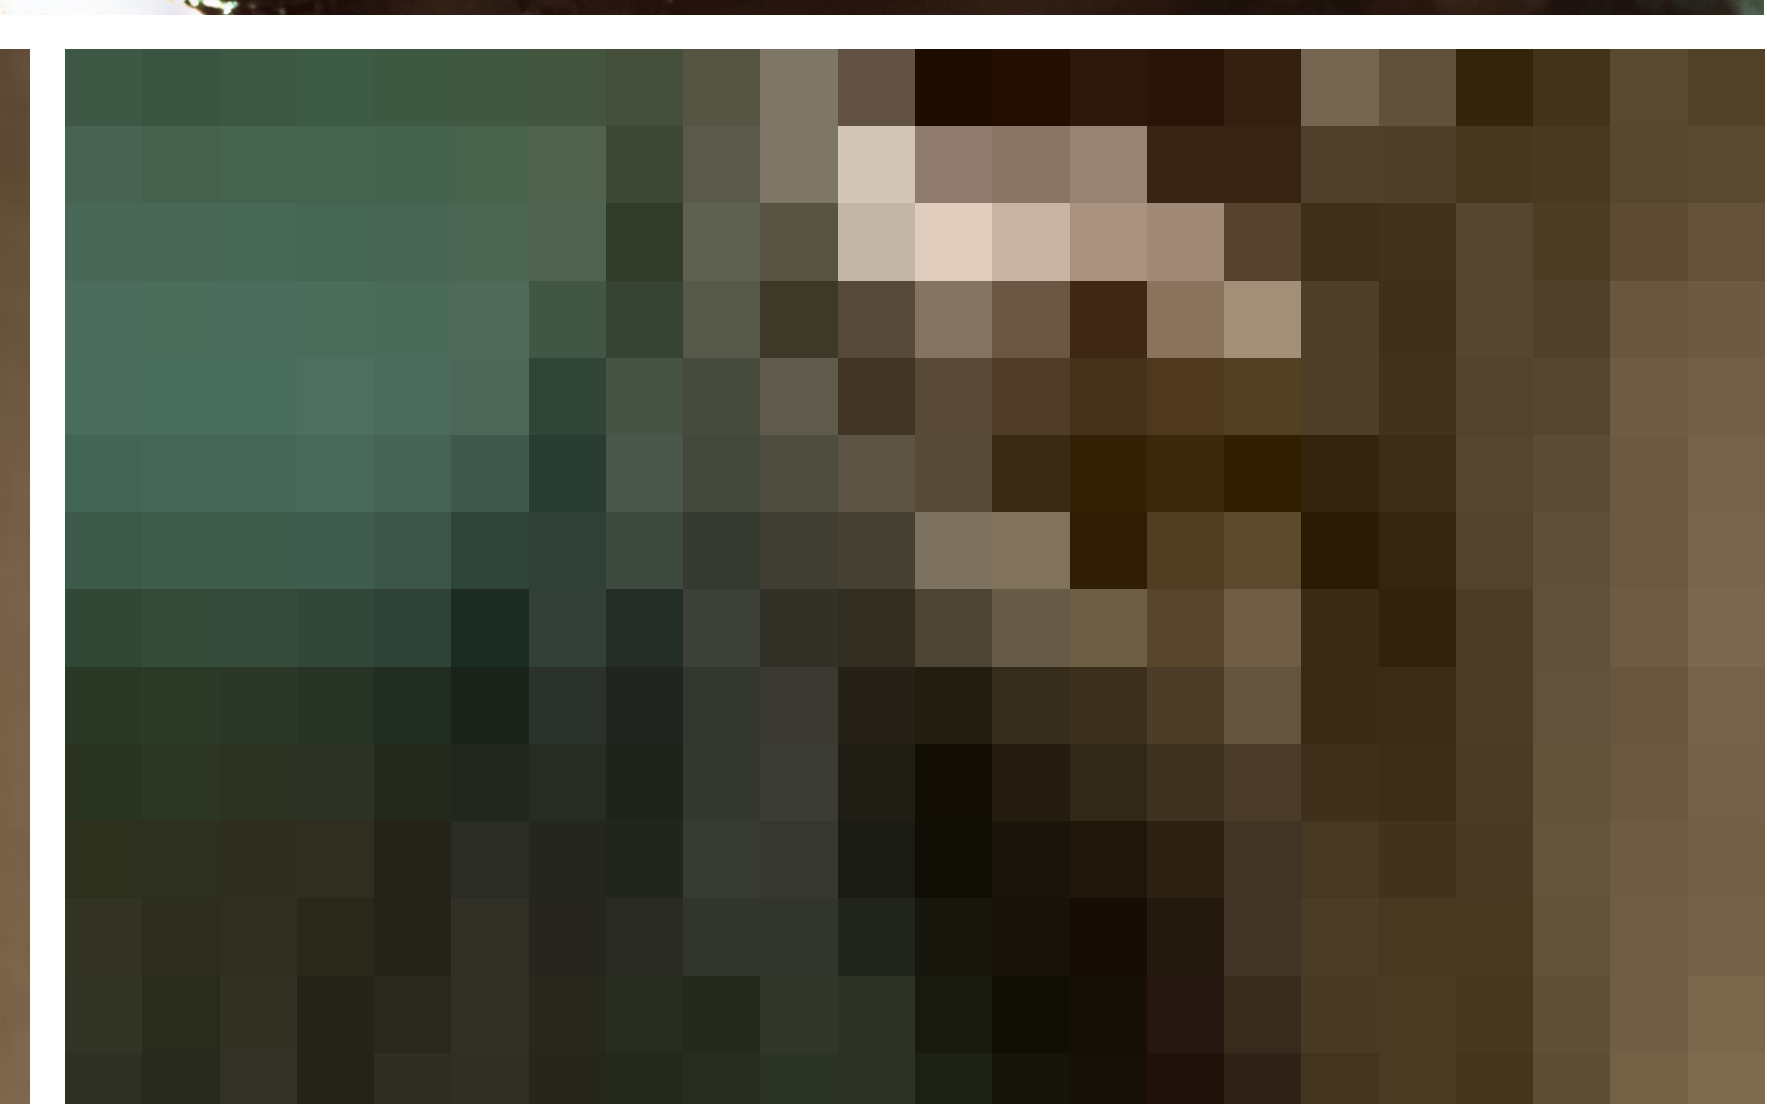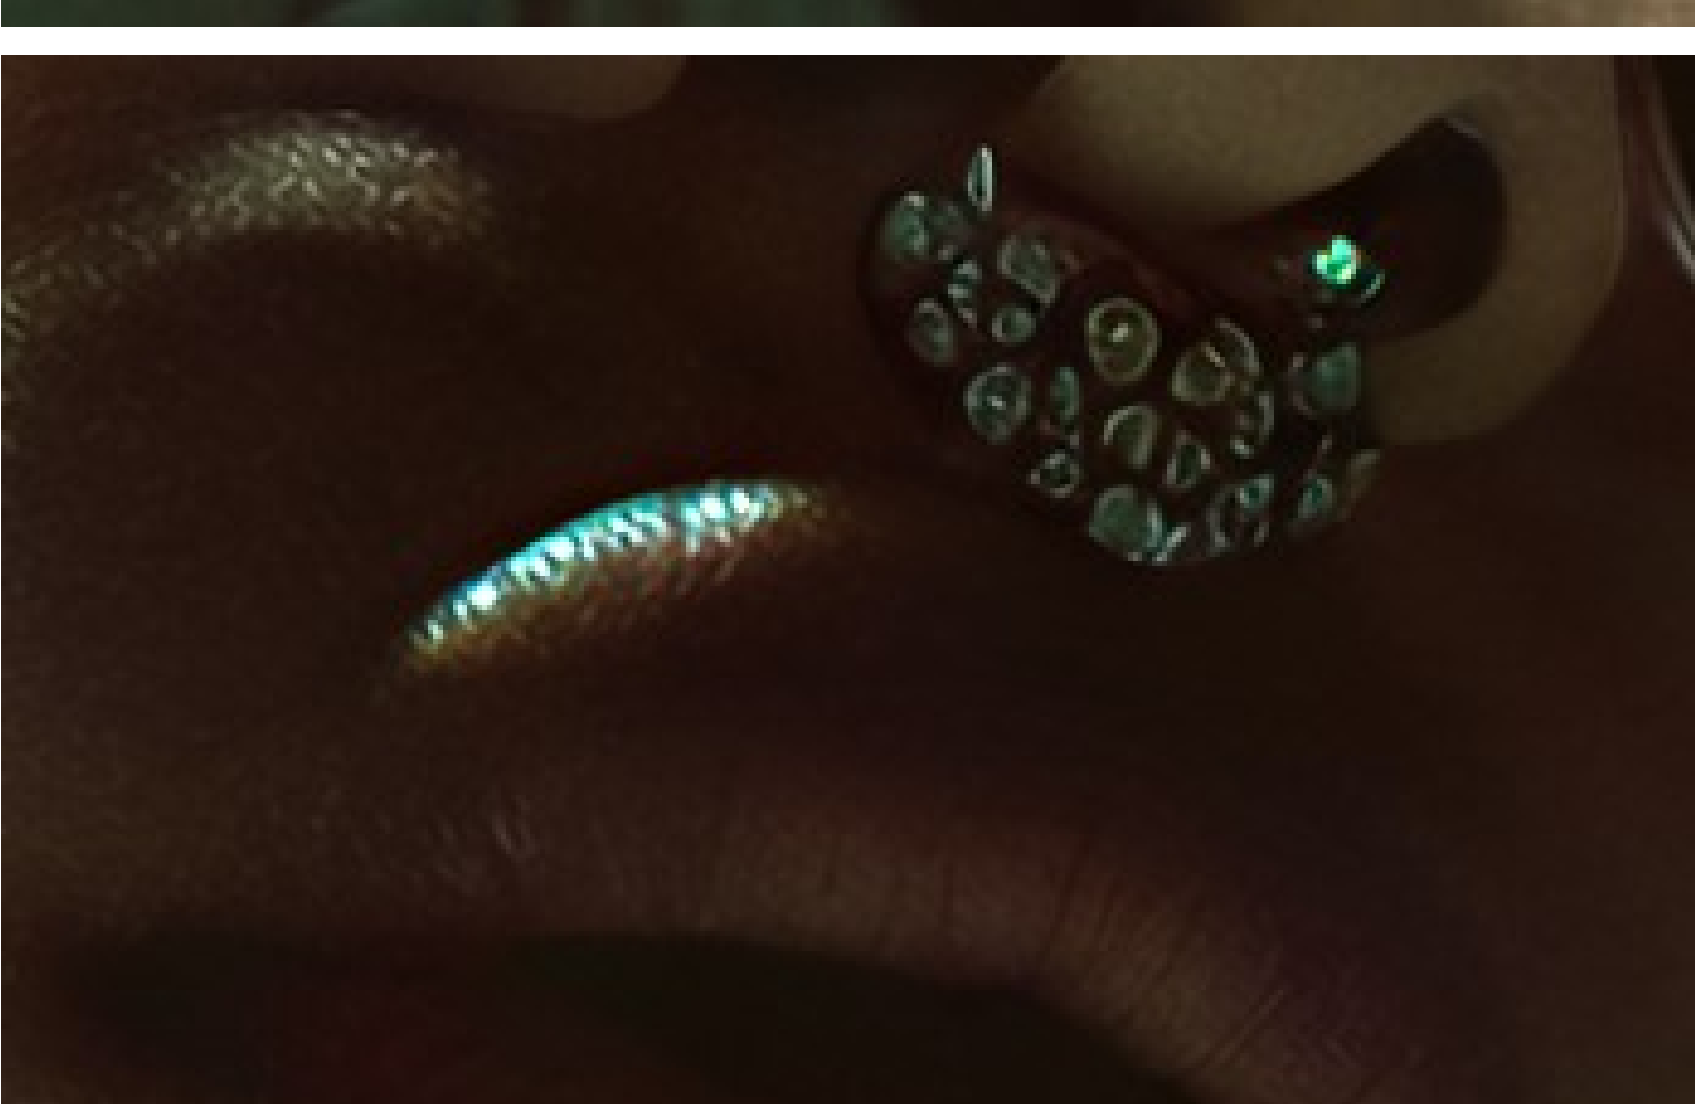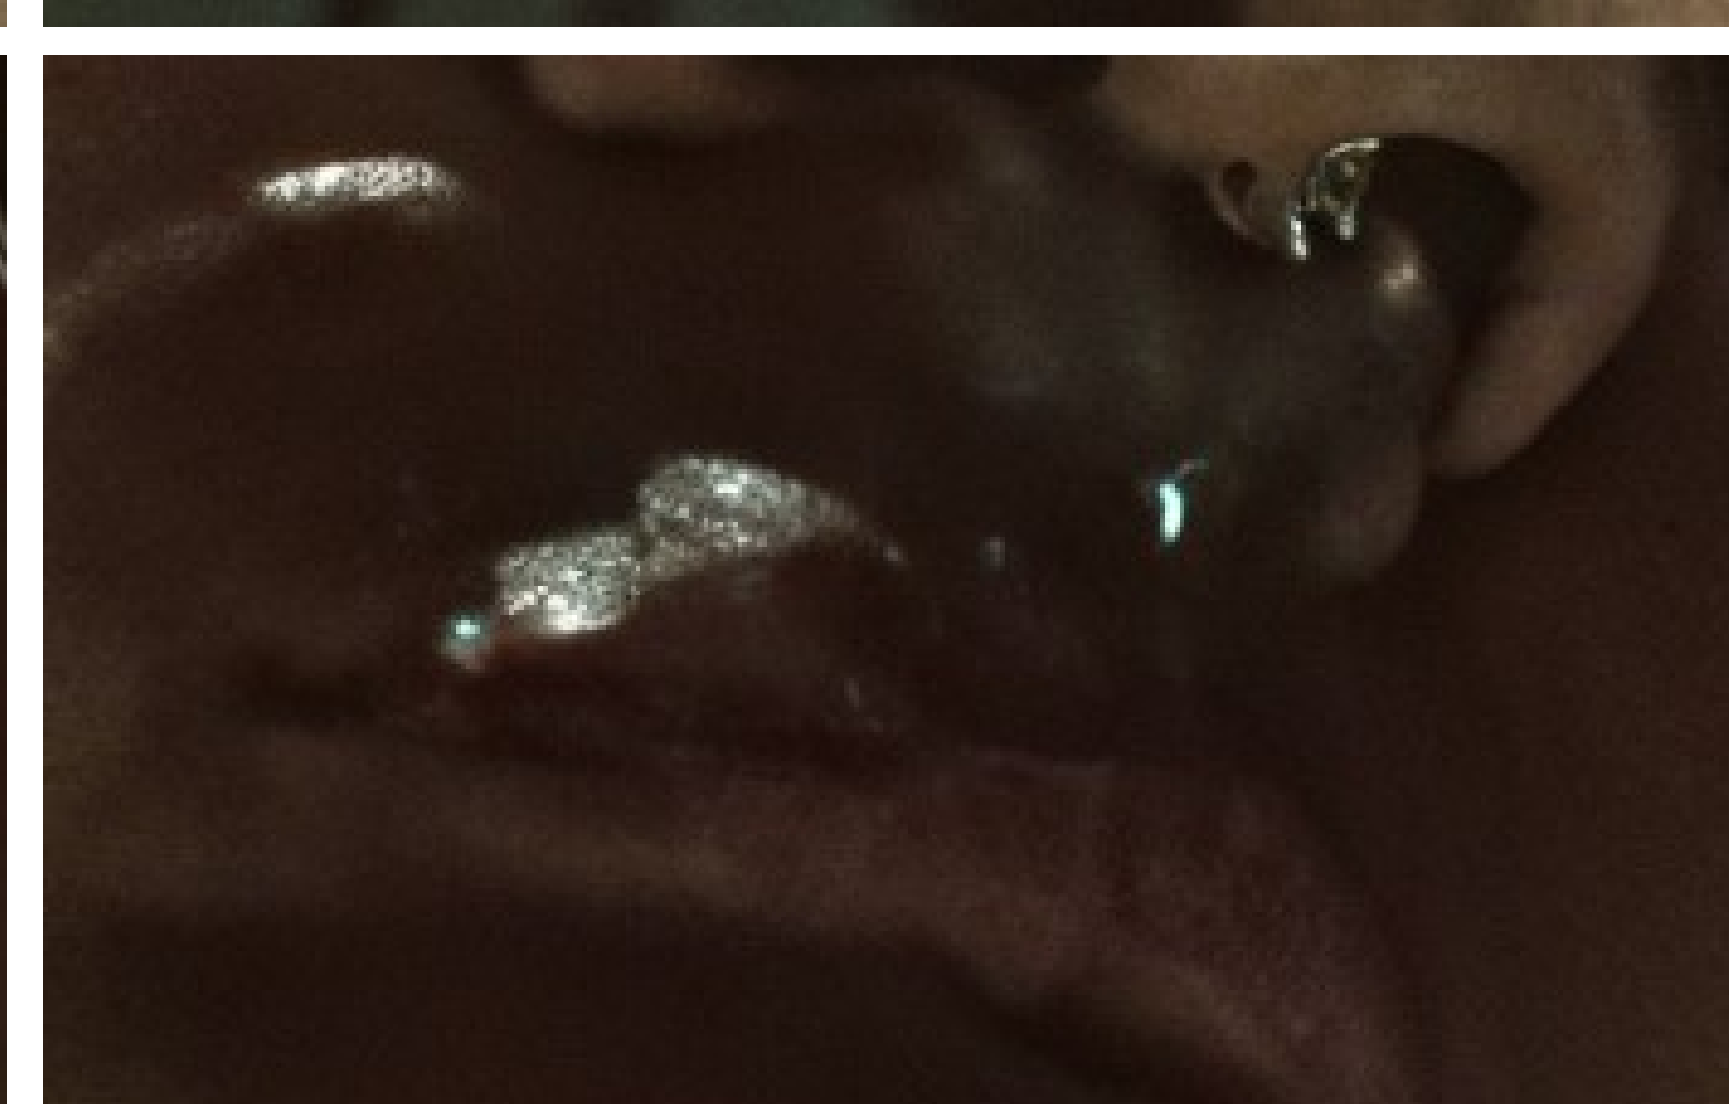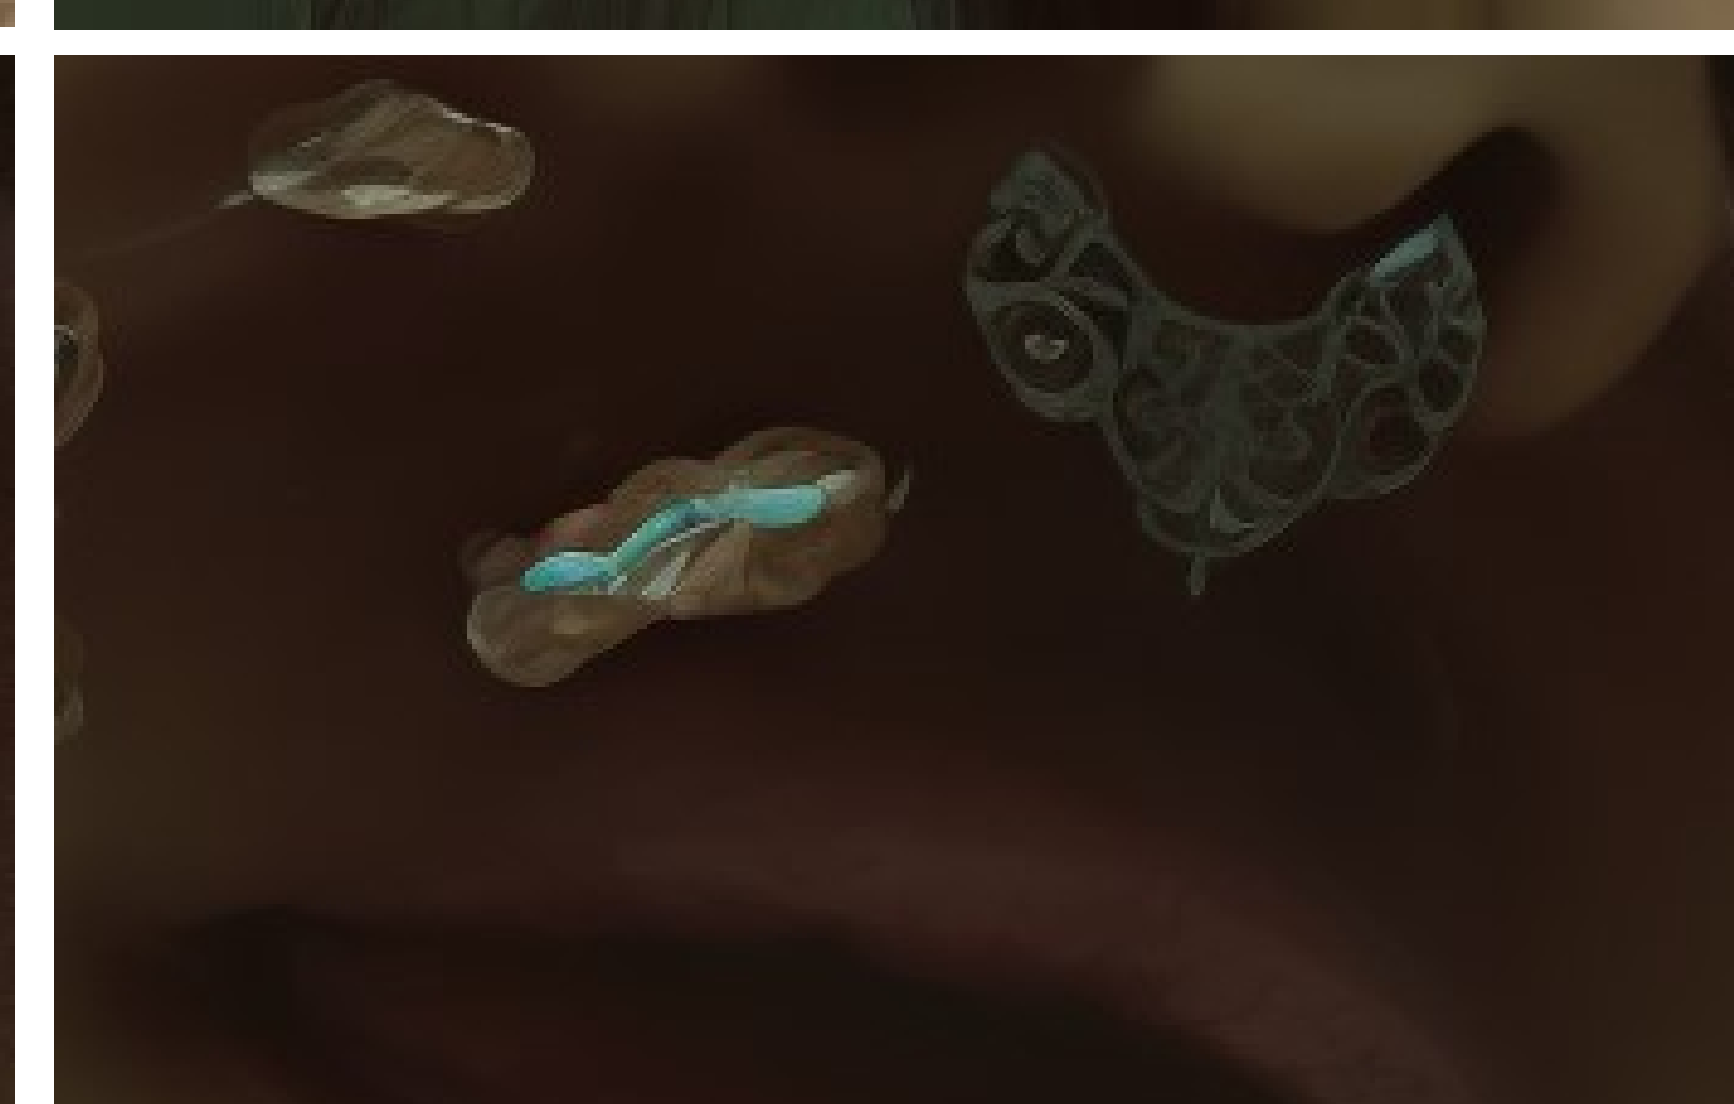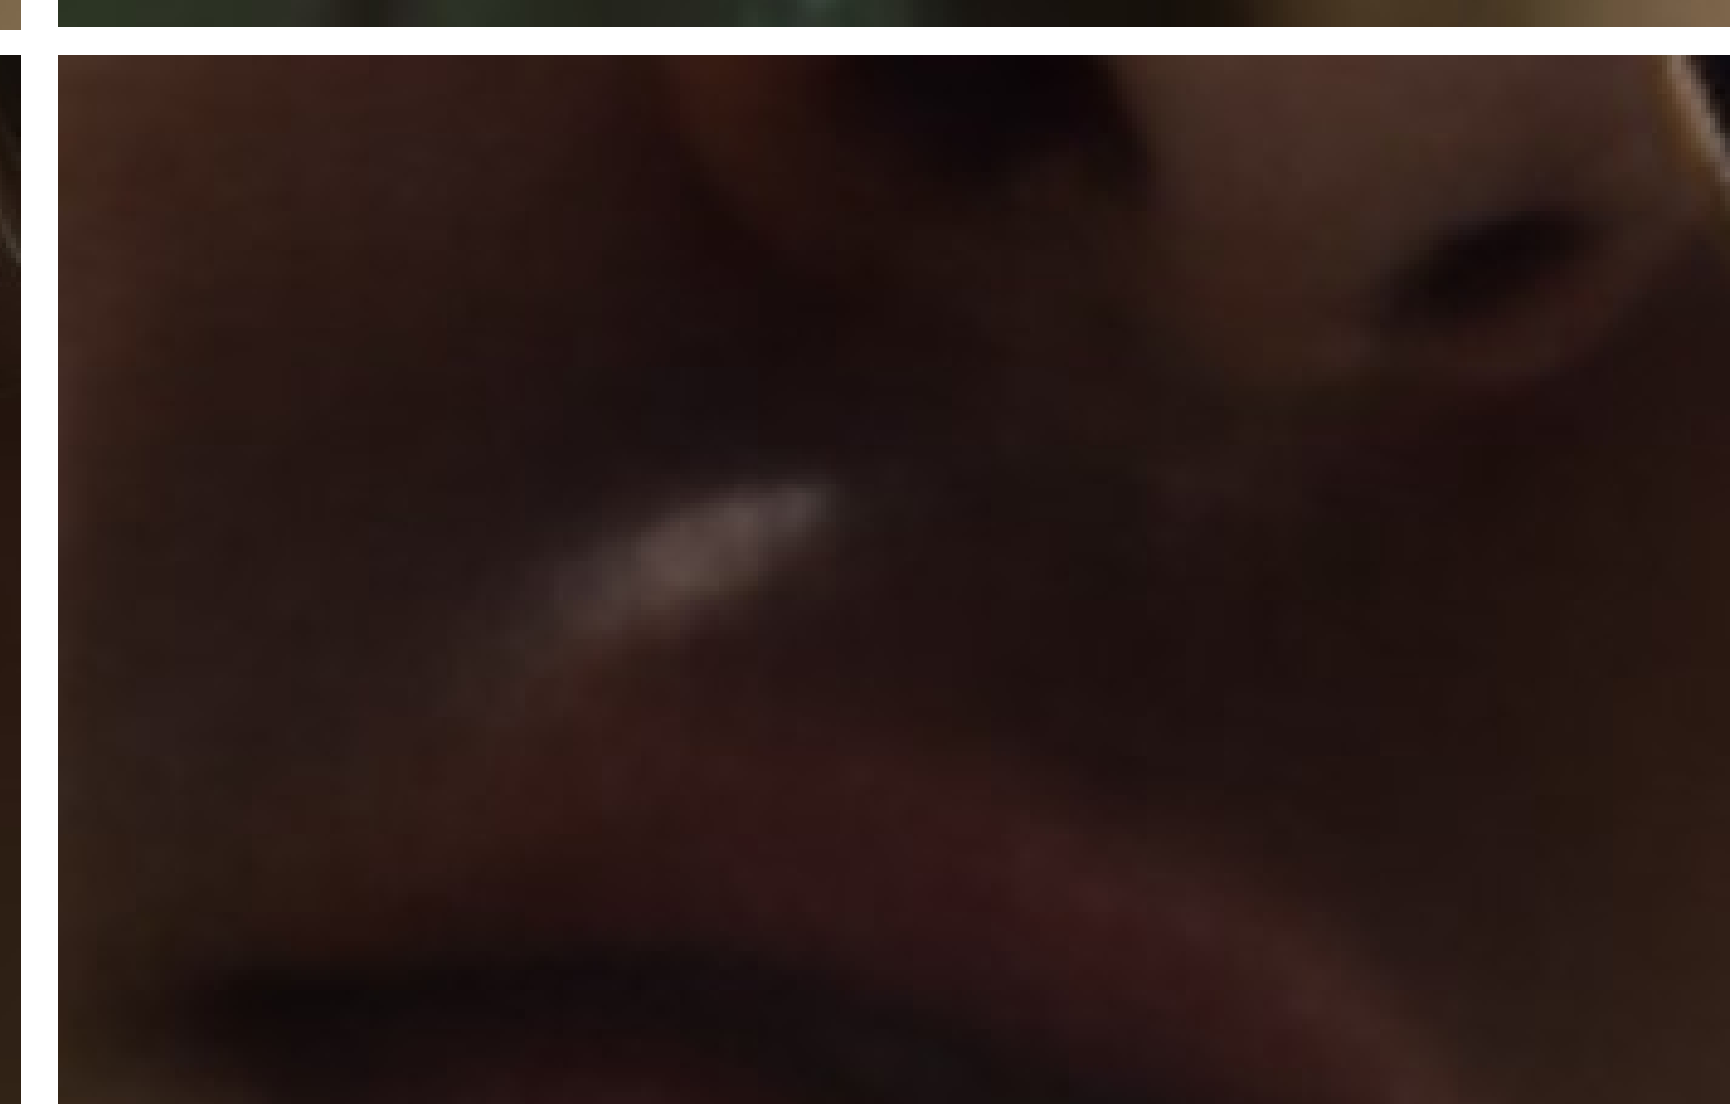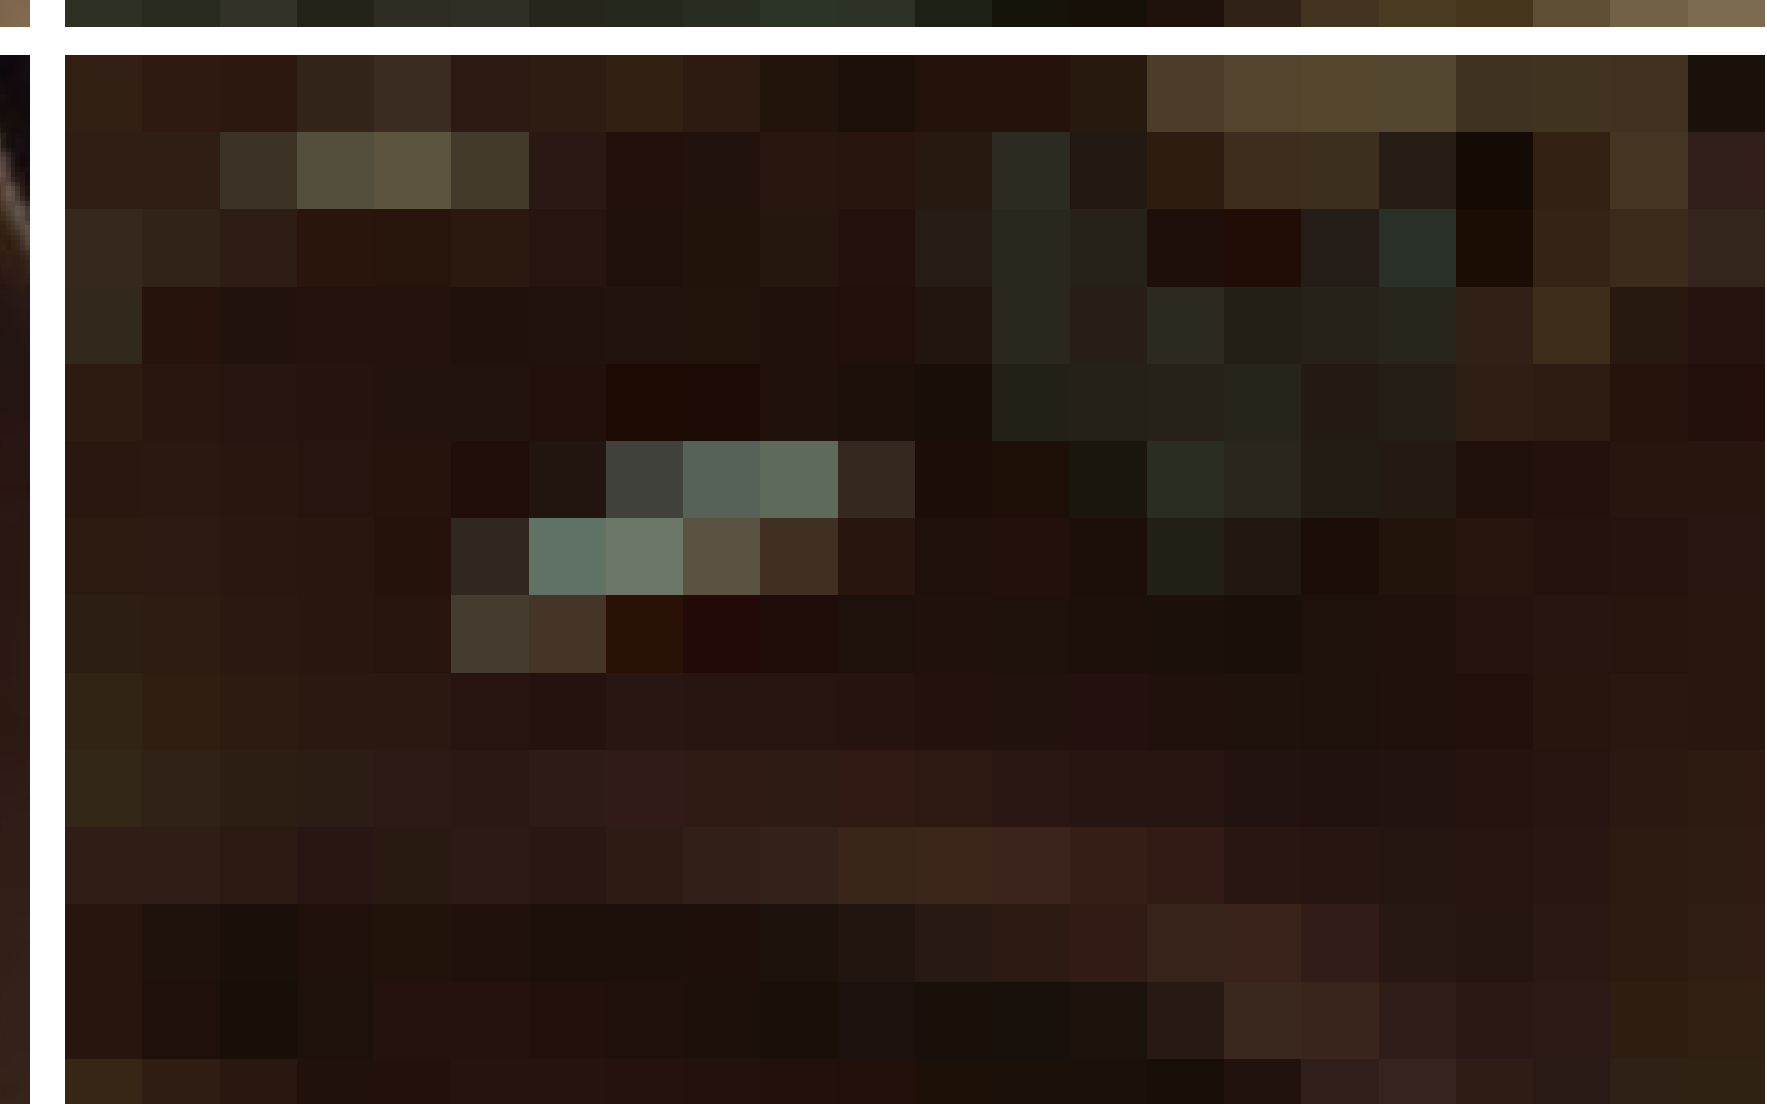

Ours

SUPIR

SeeSR

Real-ESRGAN

Input





Ours (6.9s)

16× SR, 2048px, 4Mpix

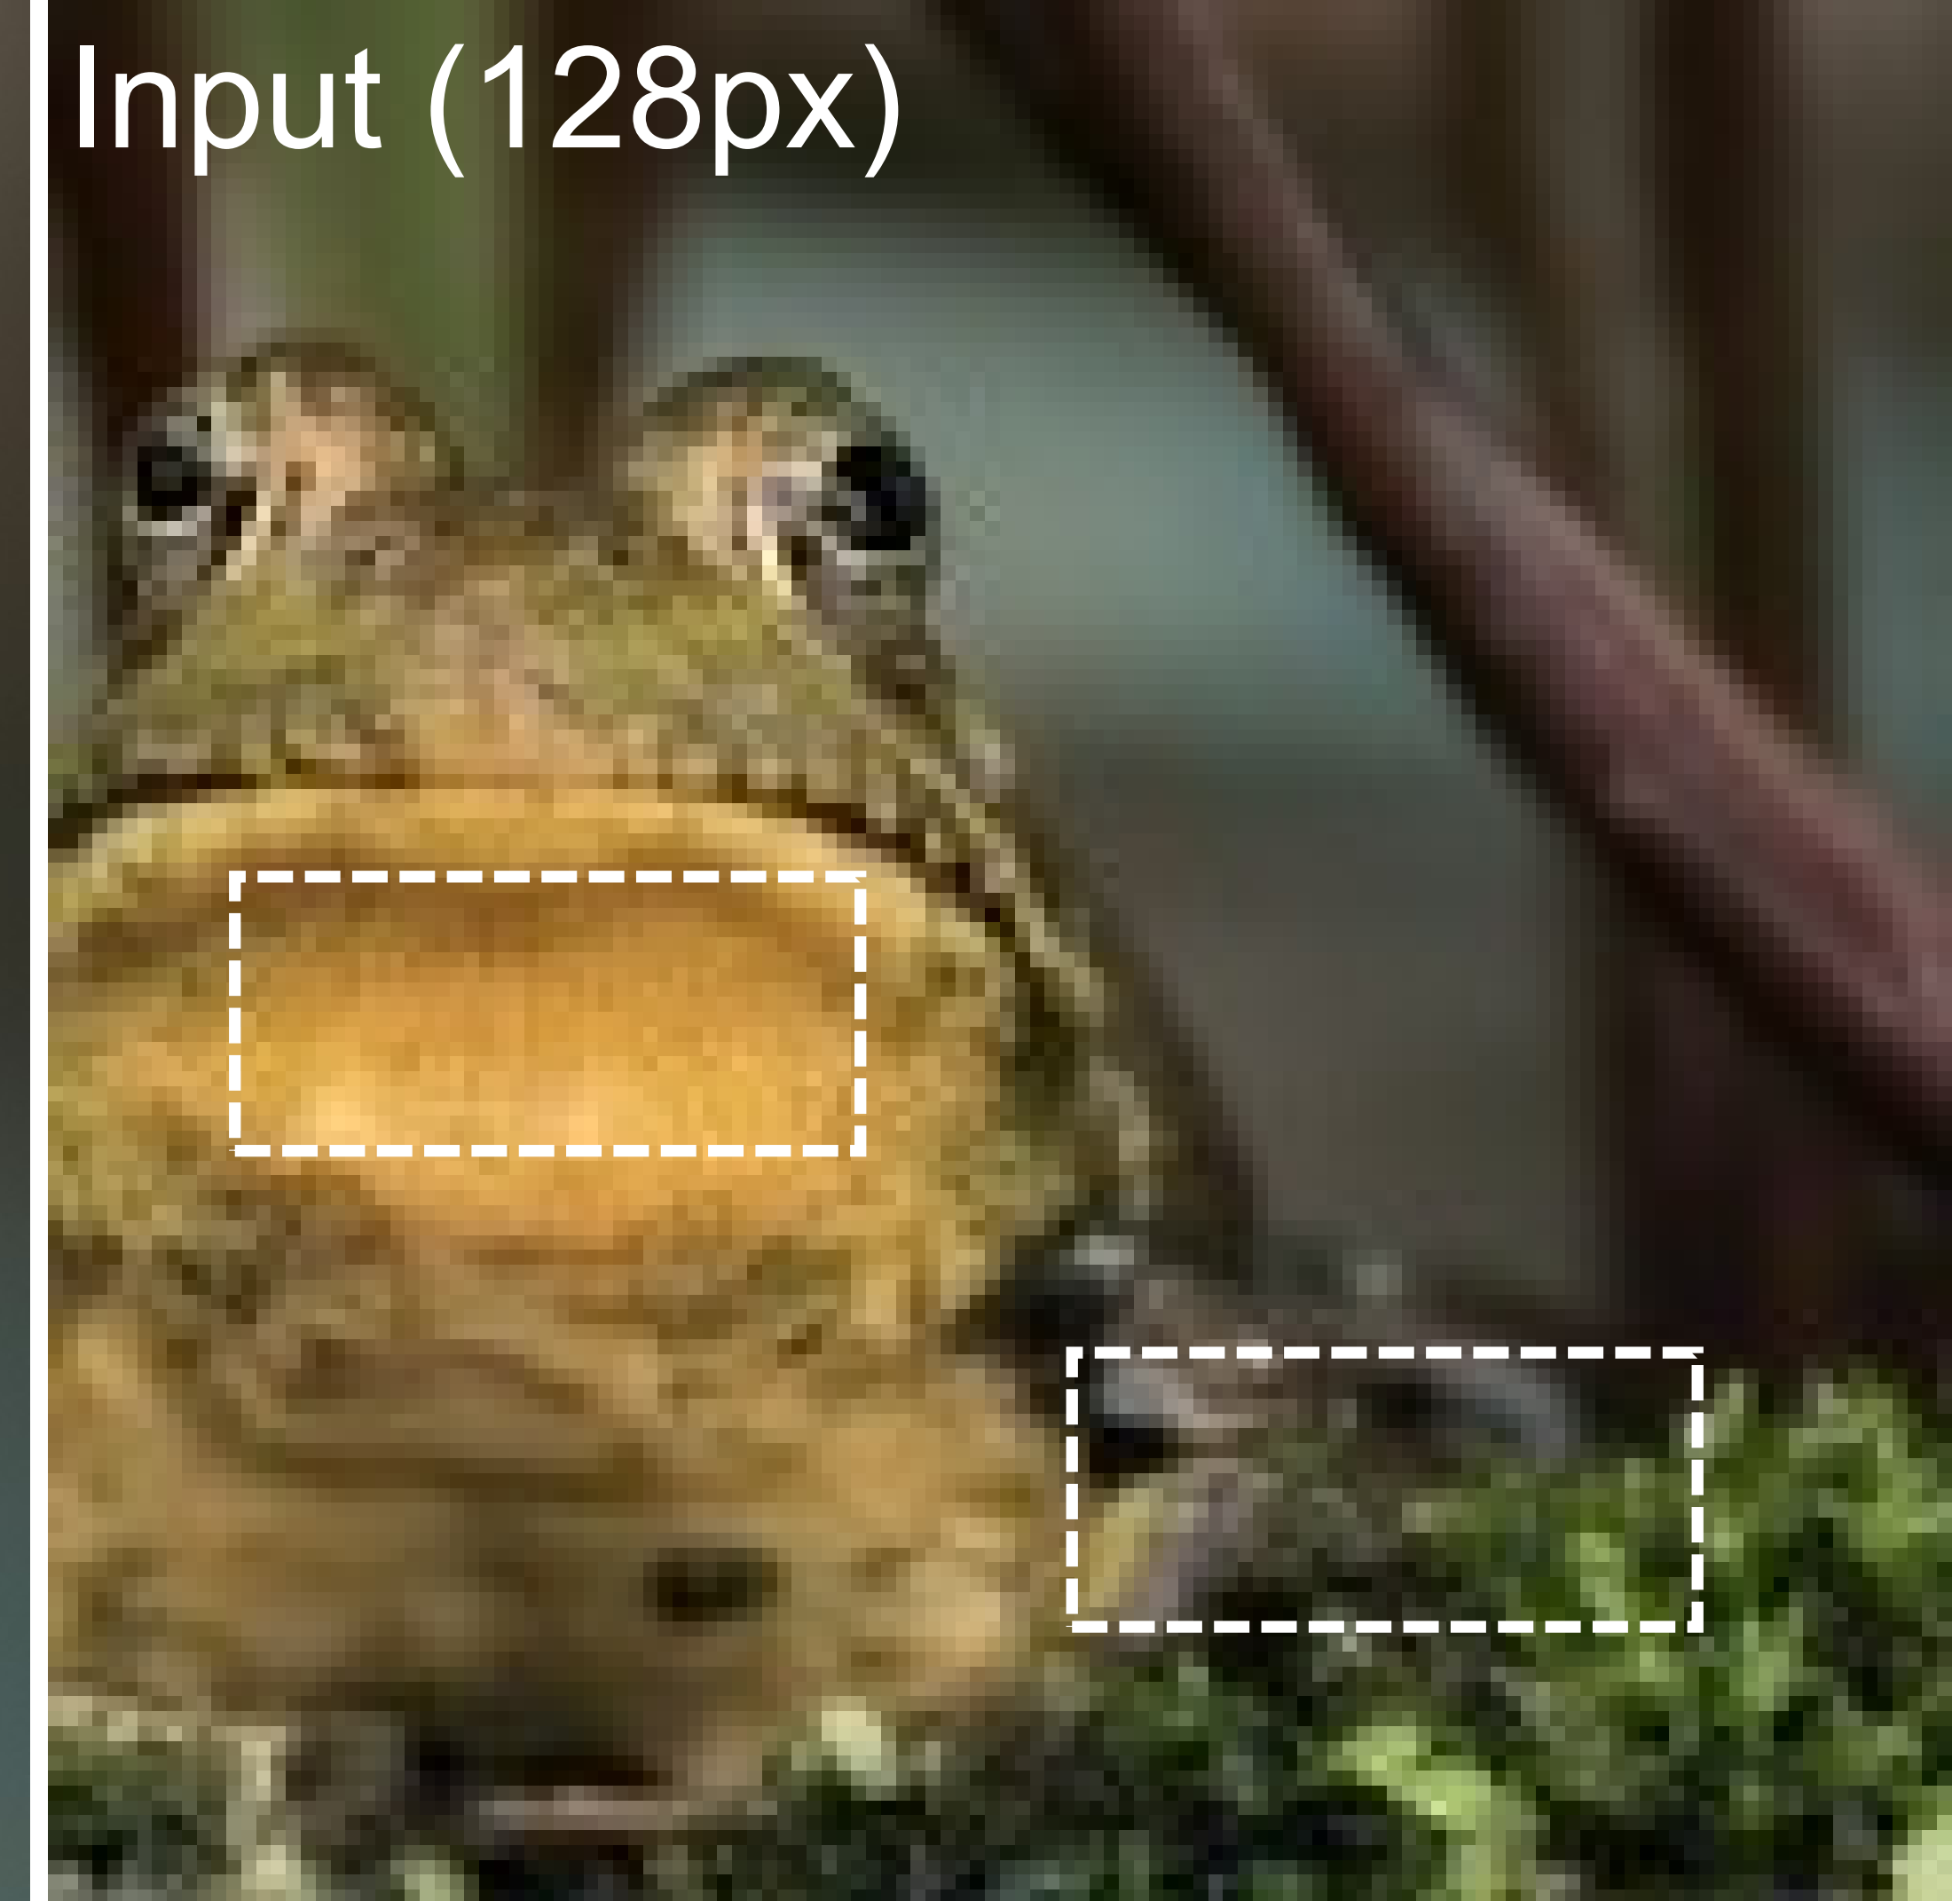

Input (128px)

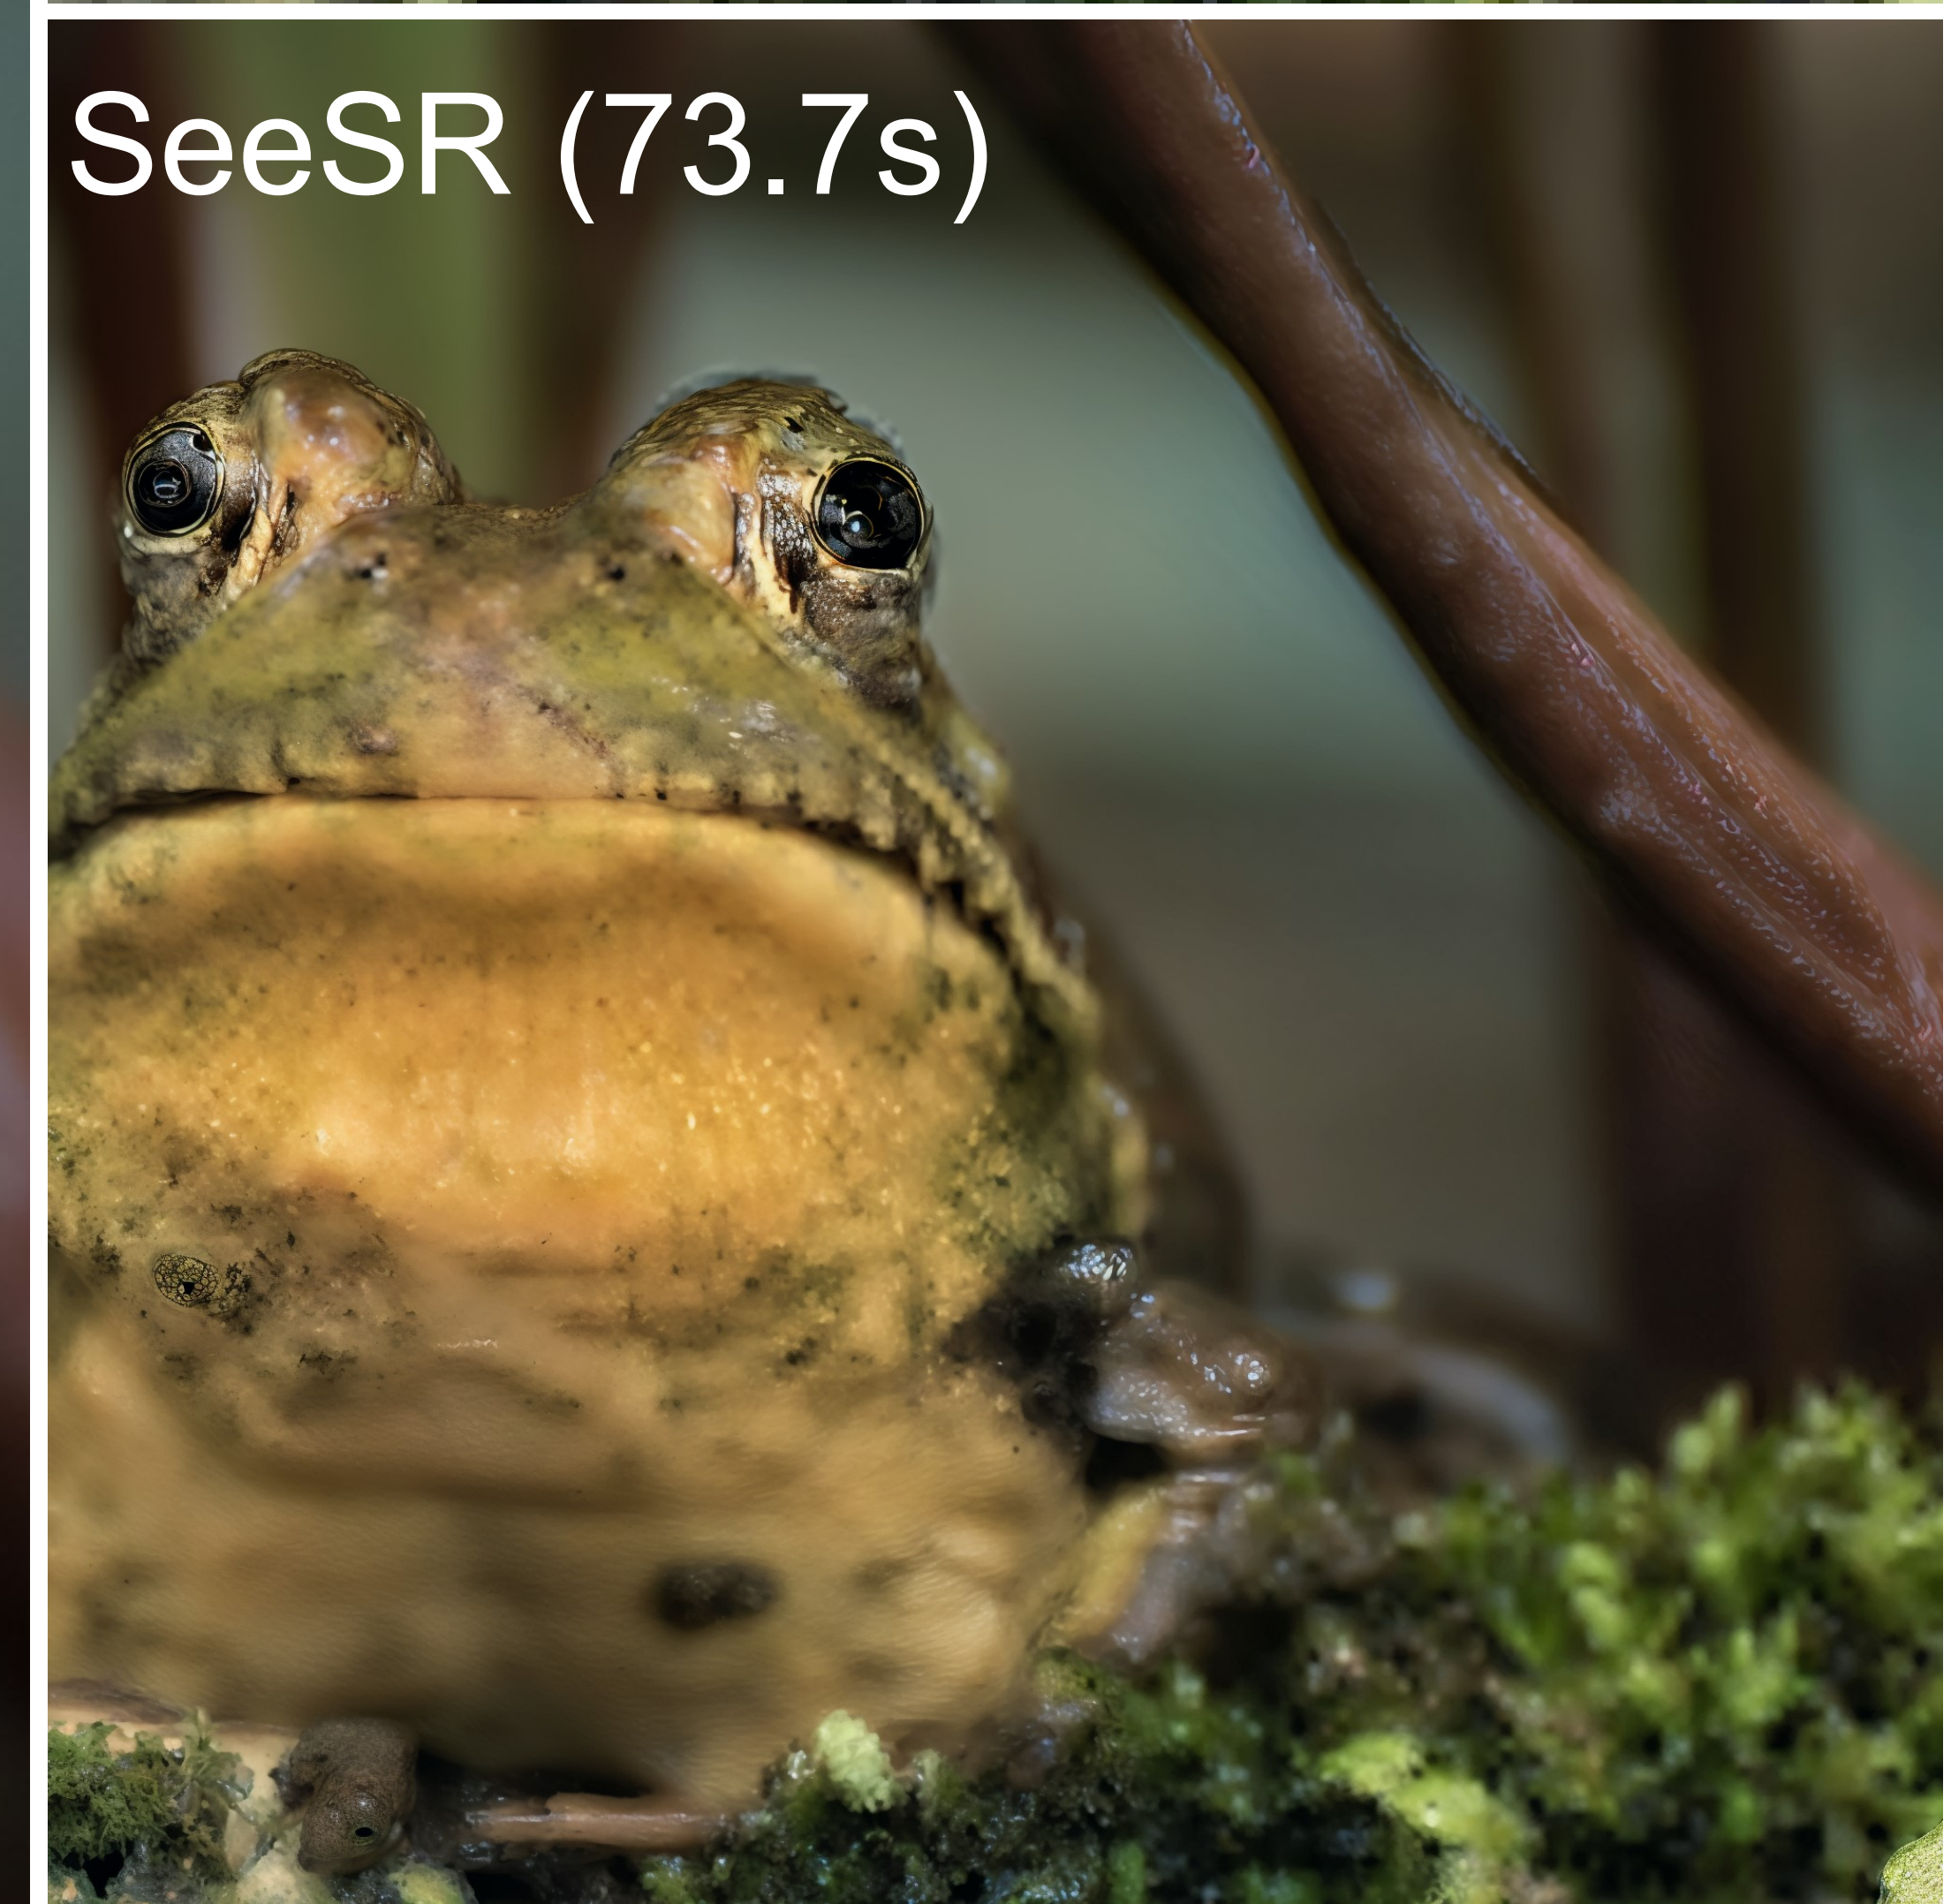

SeeSR (73.7s)

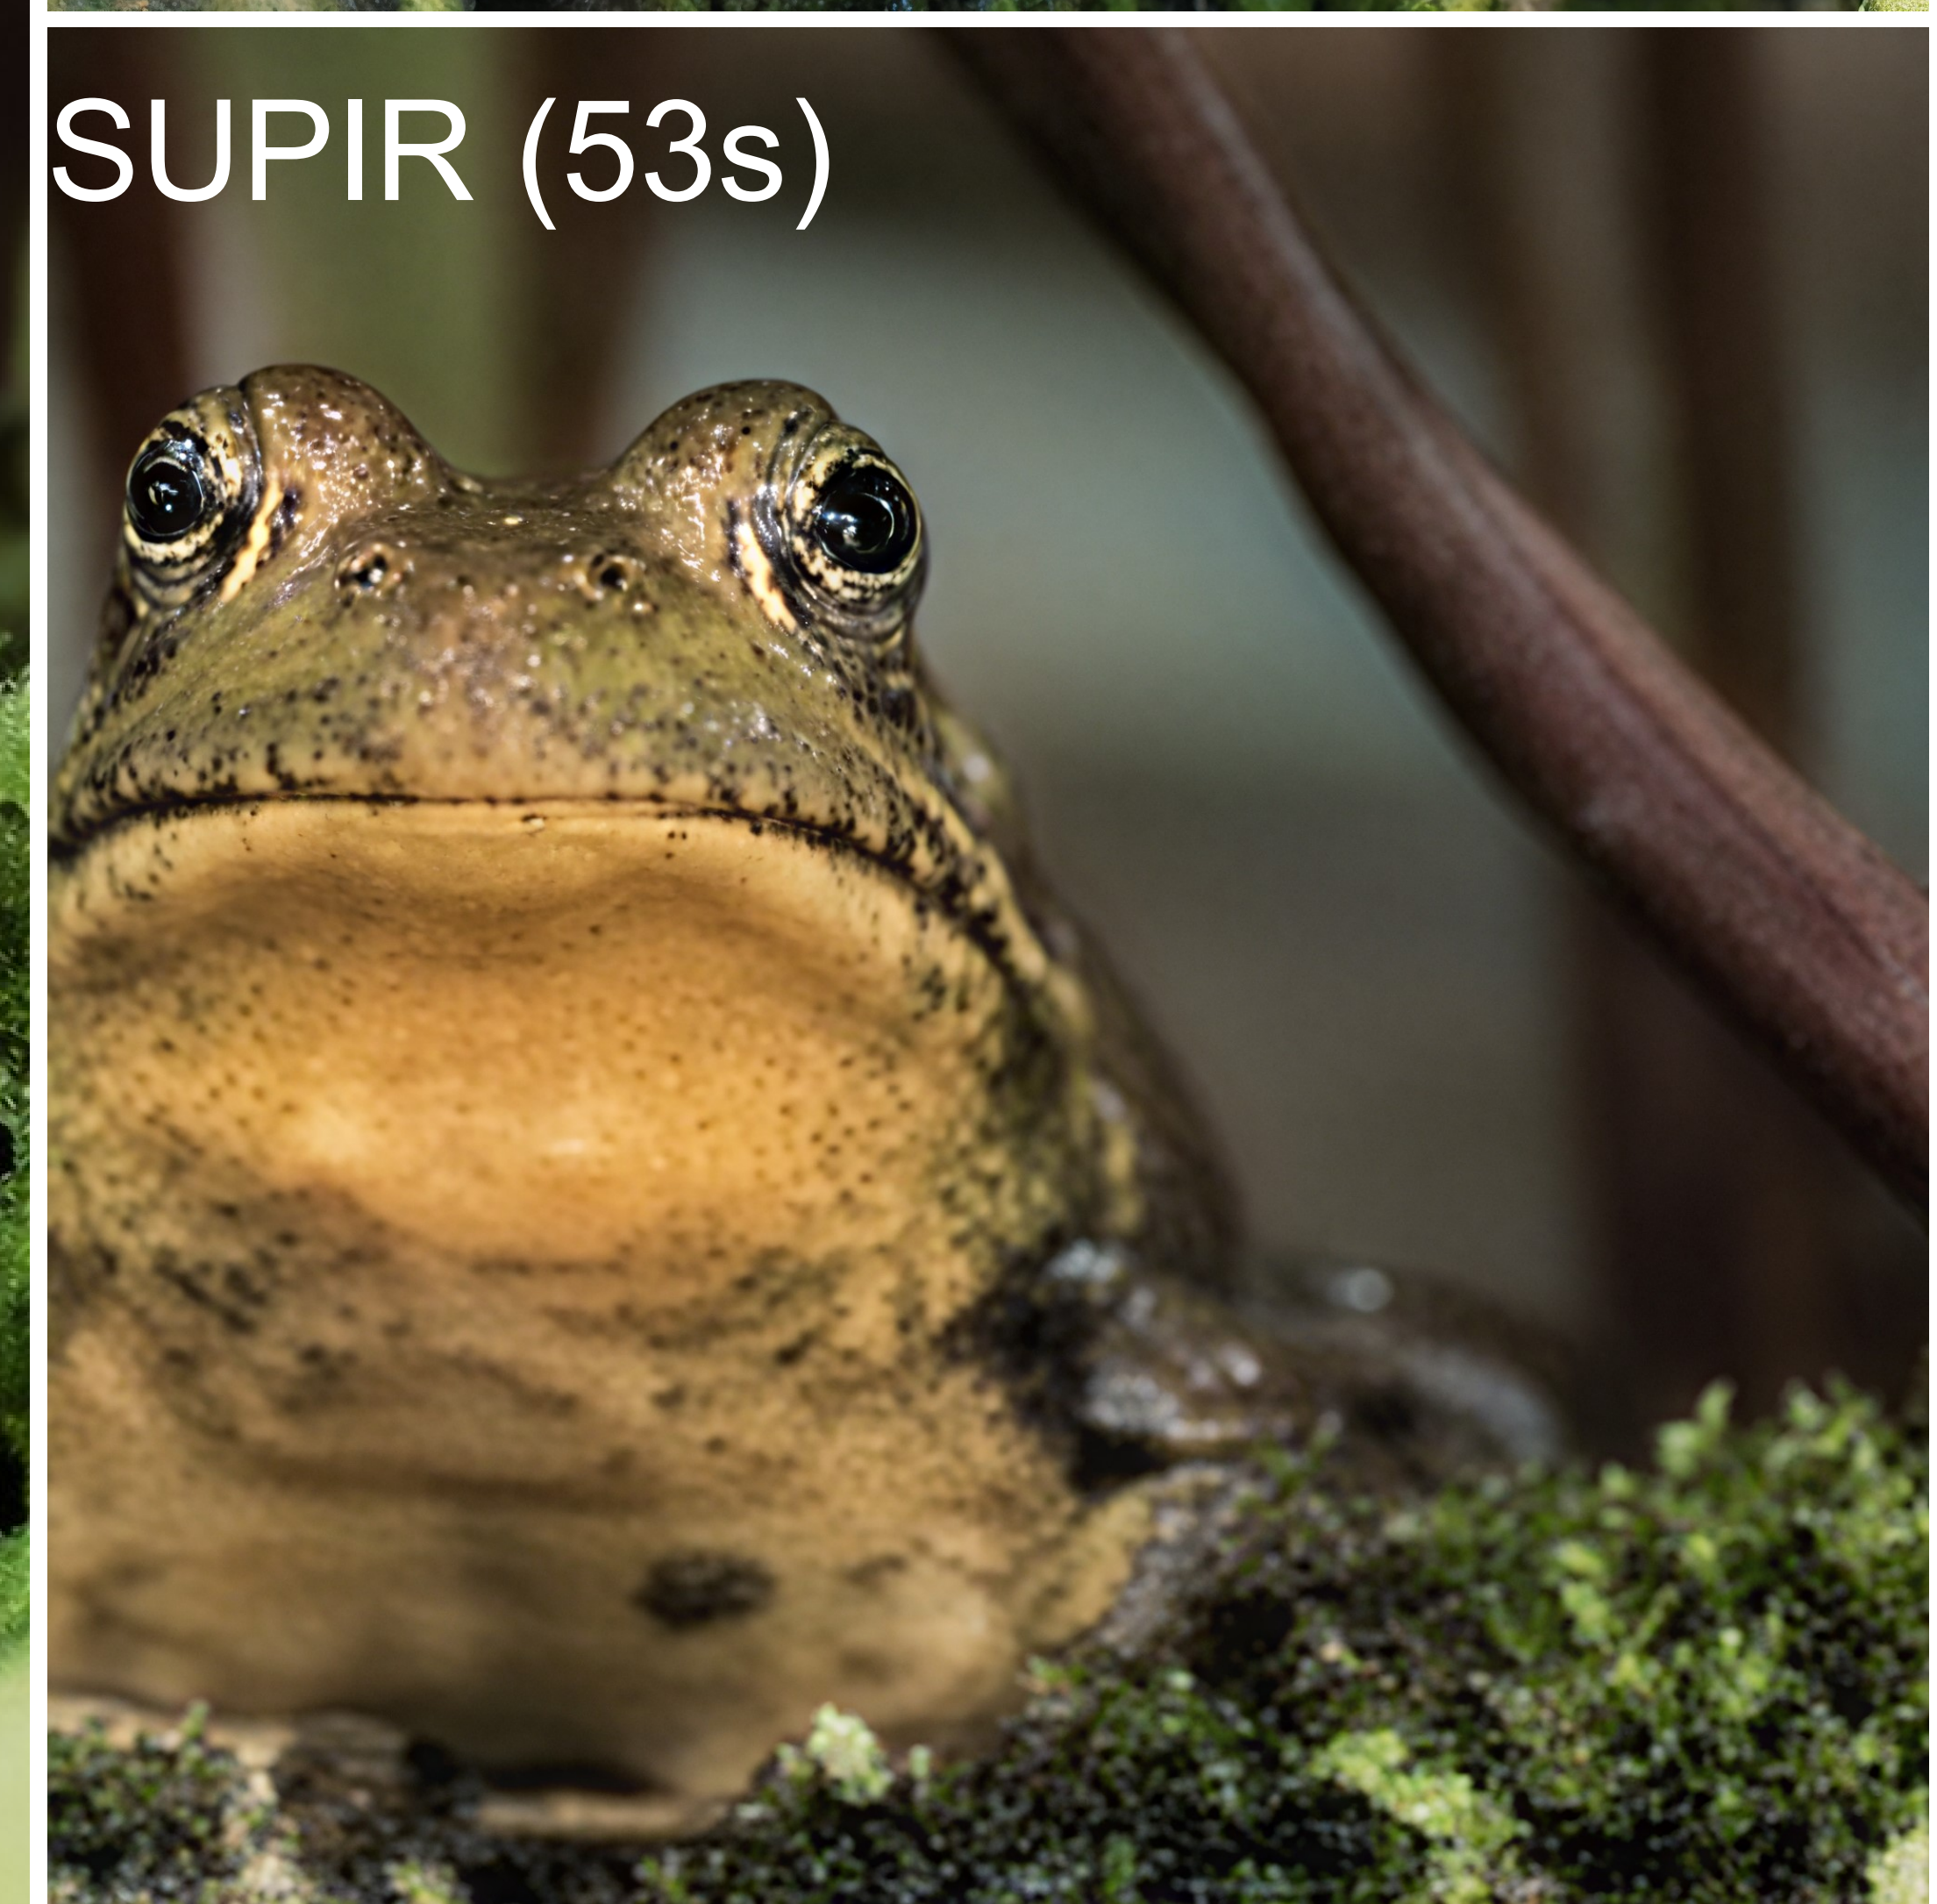

SUPIR (53s)

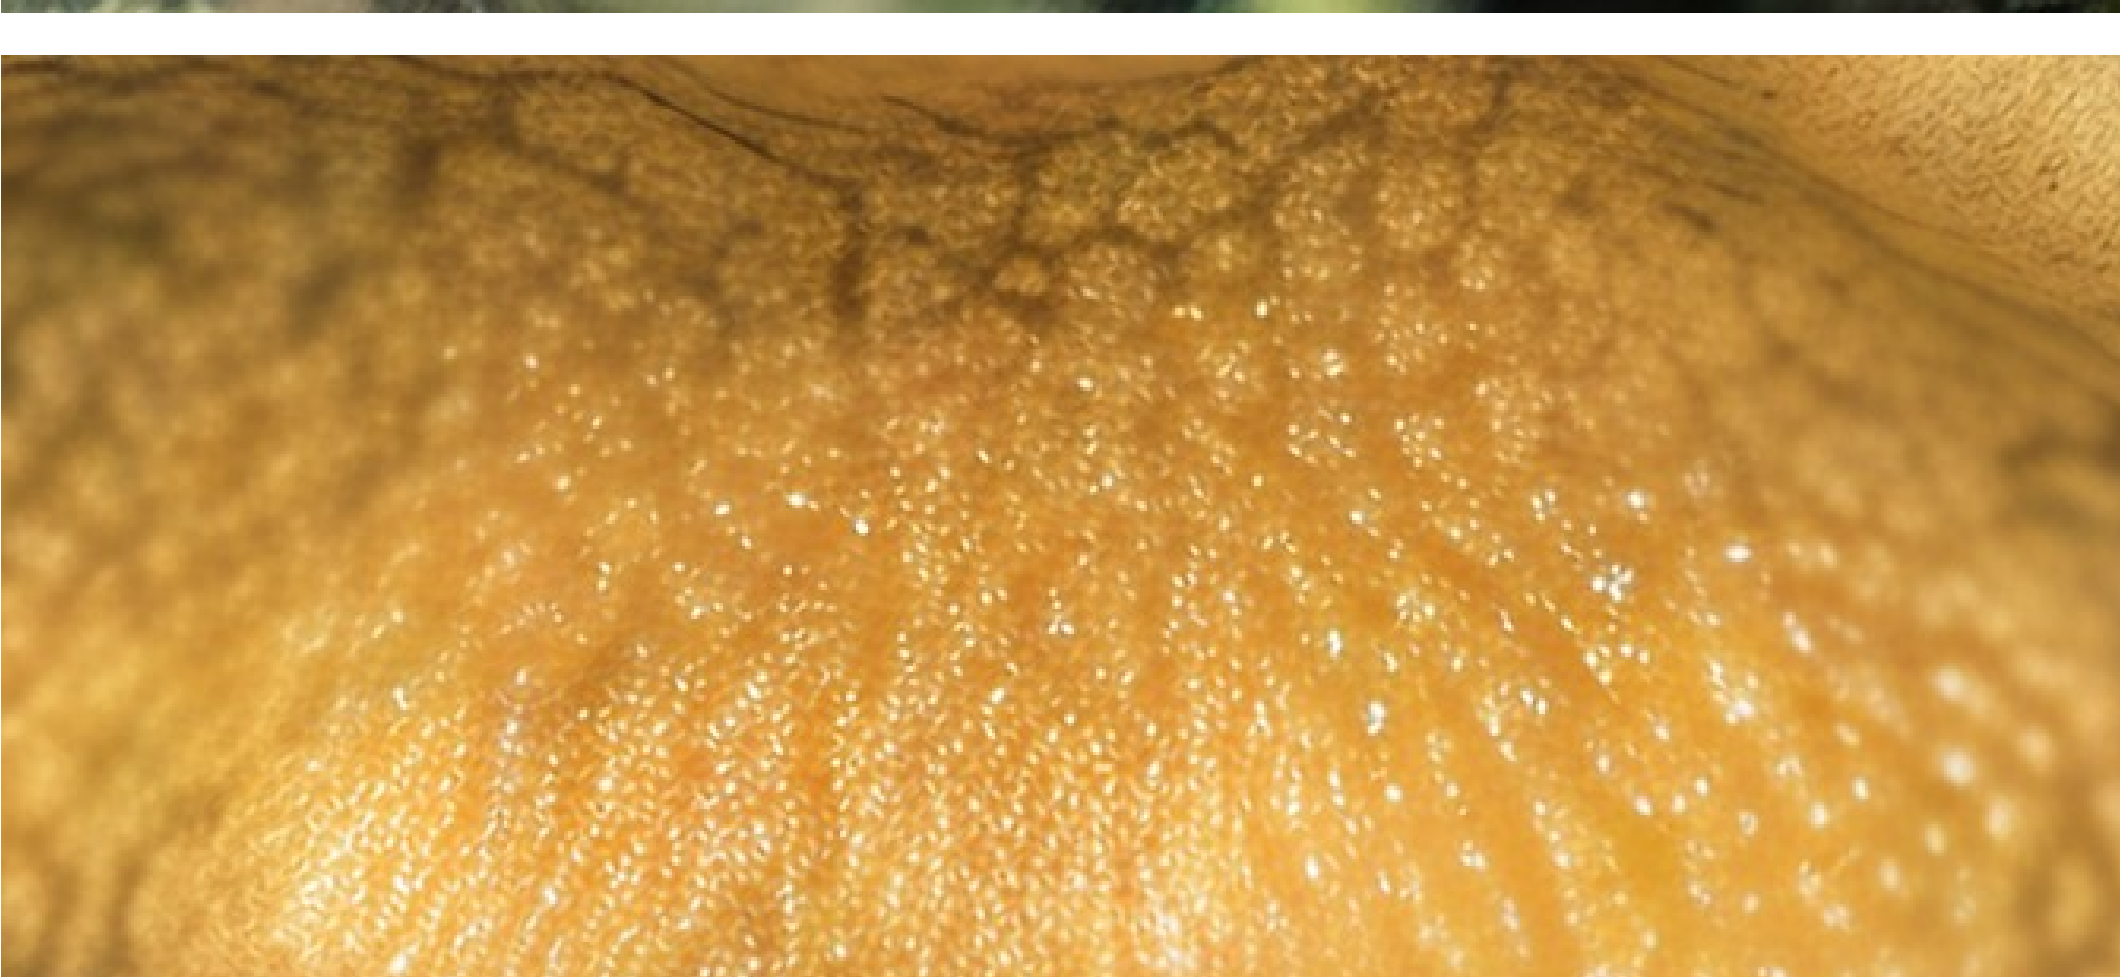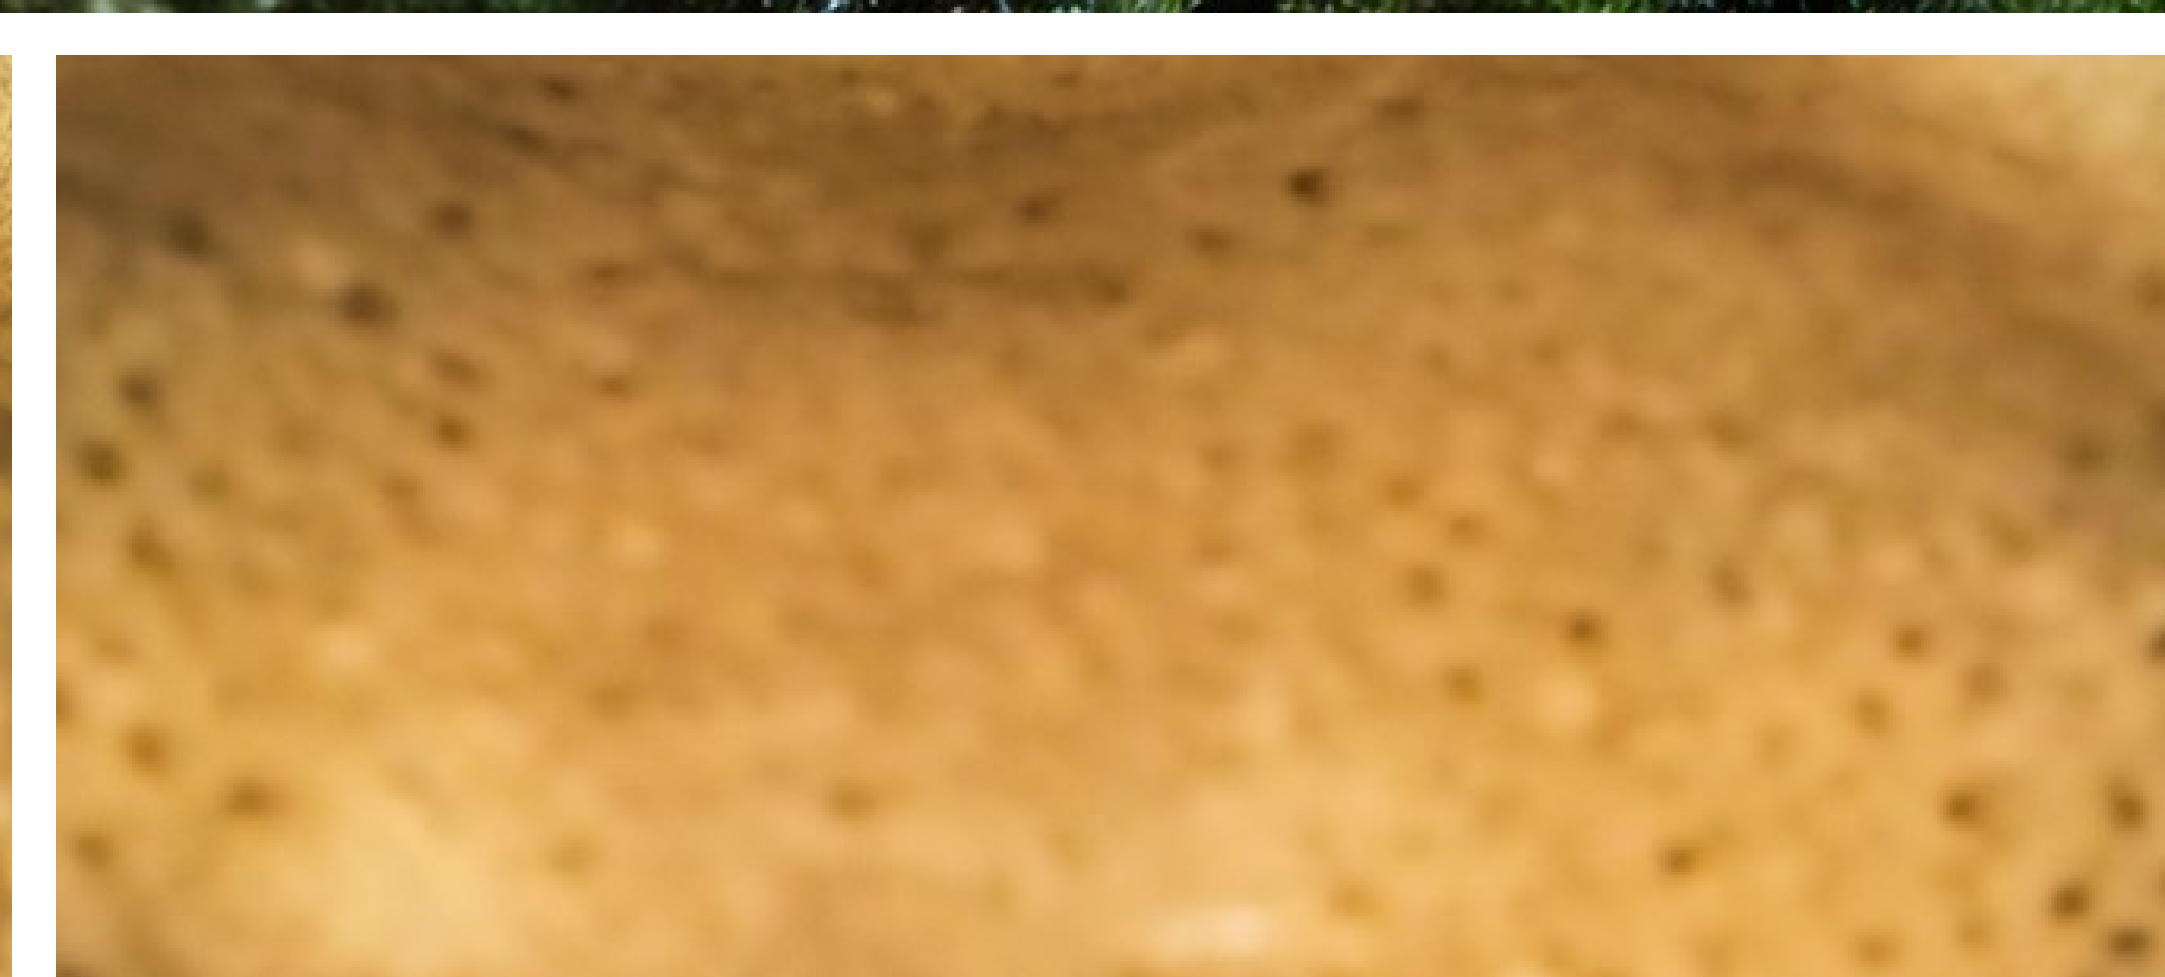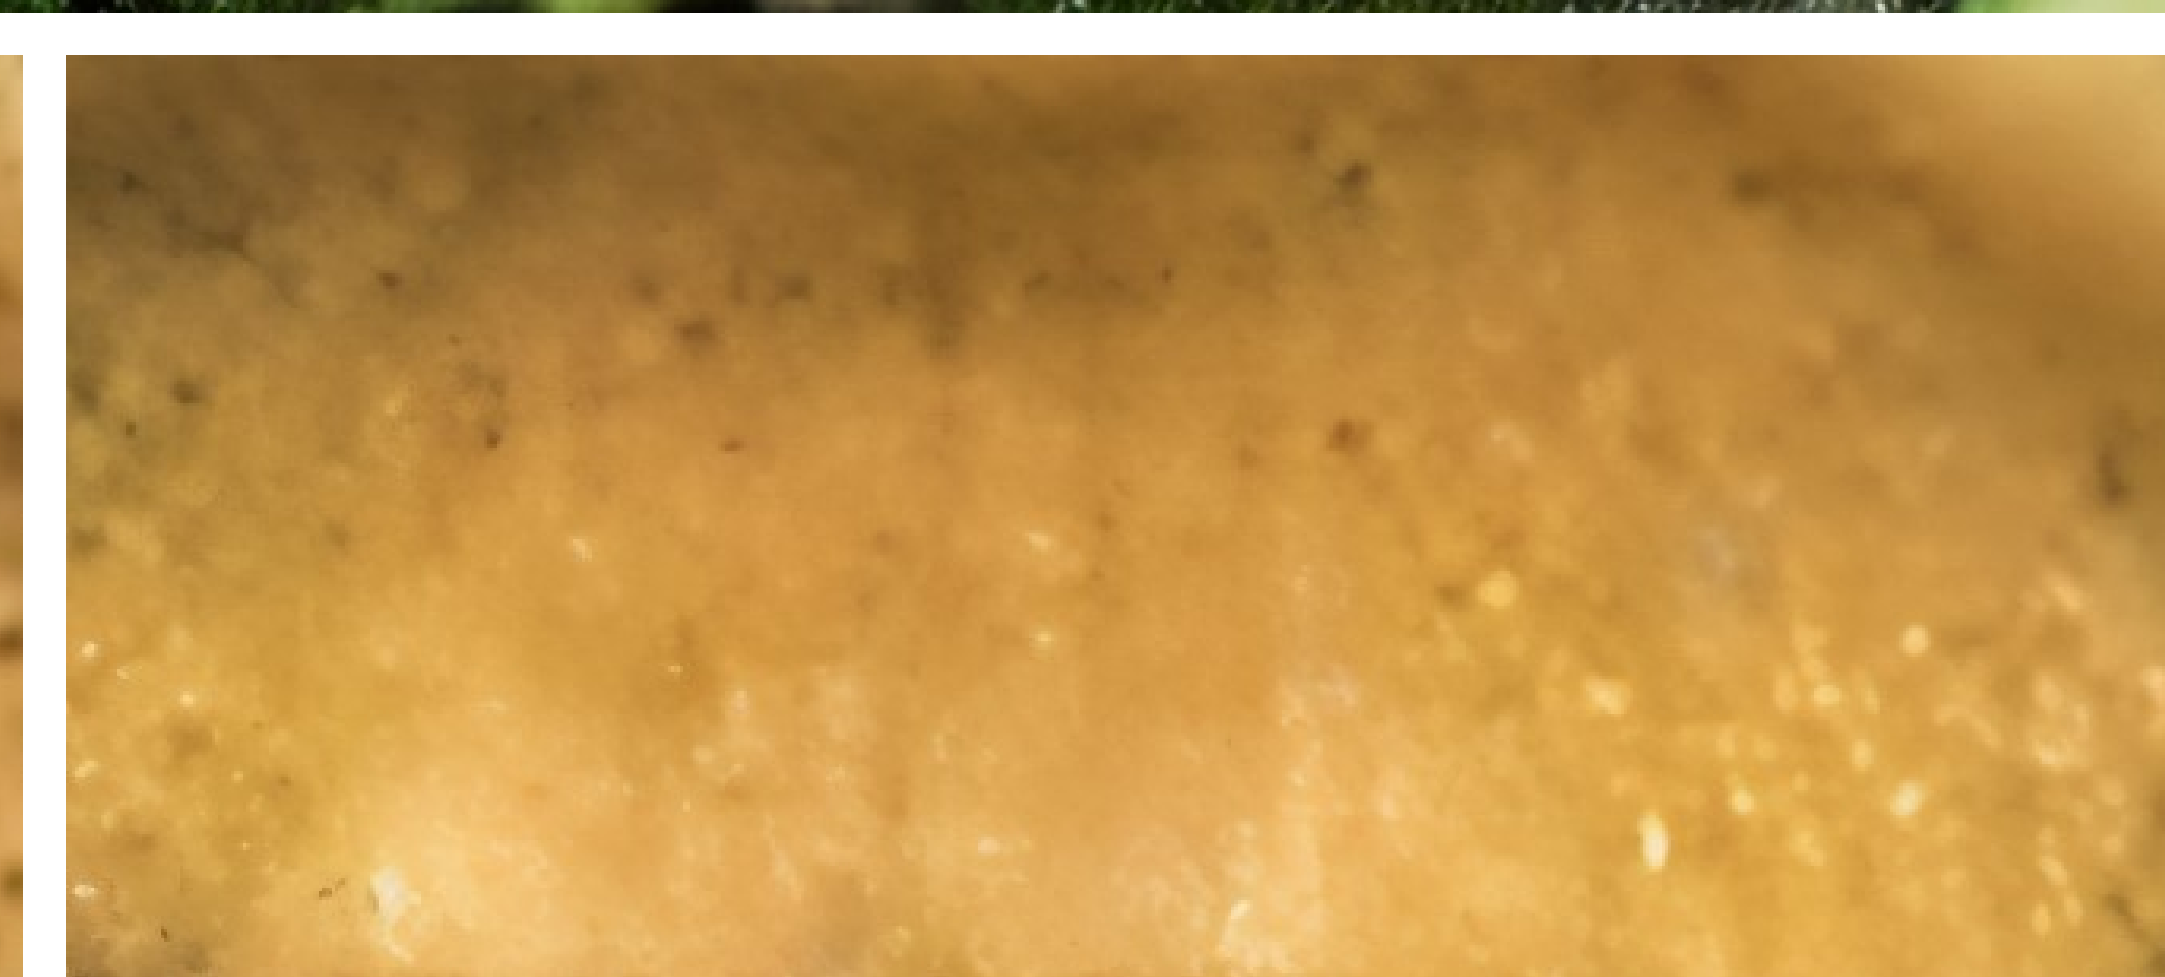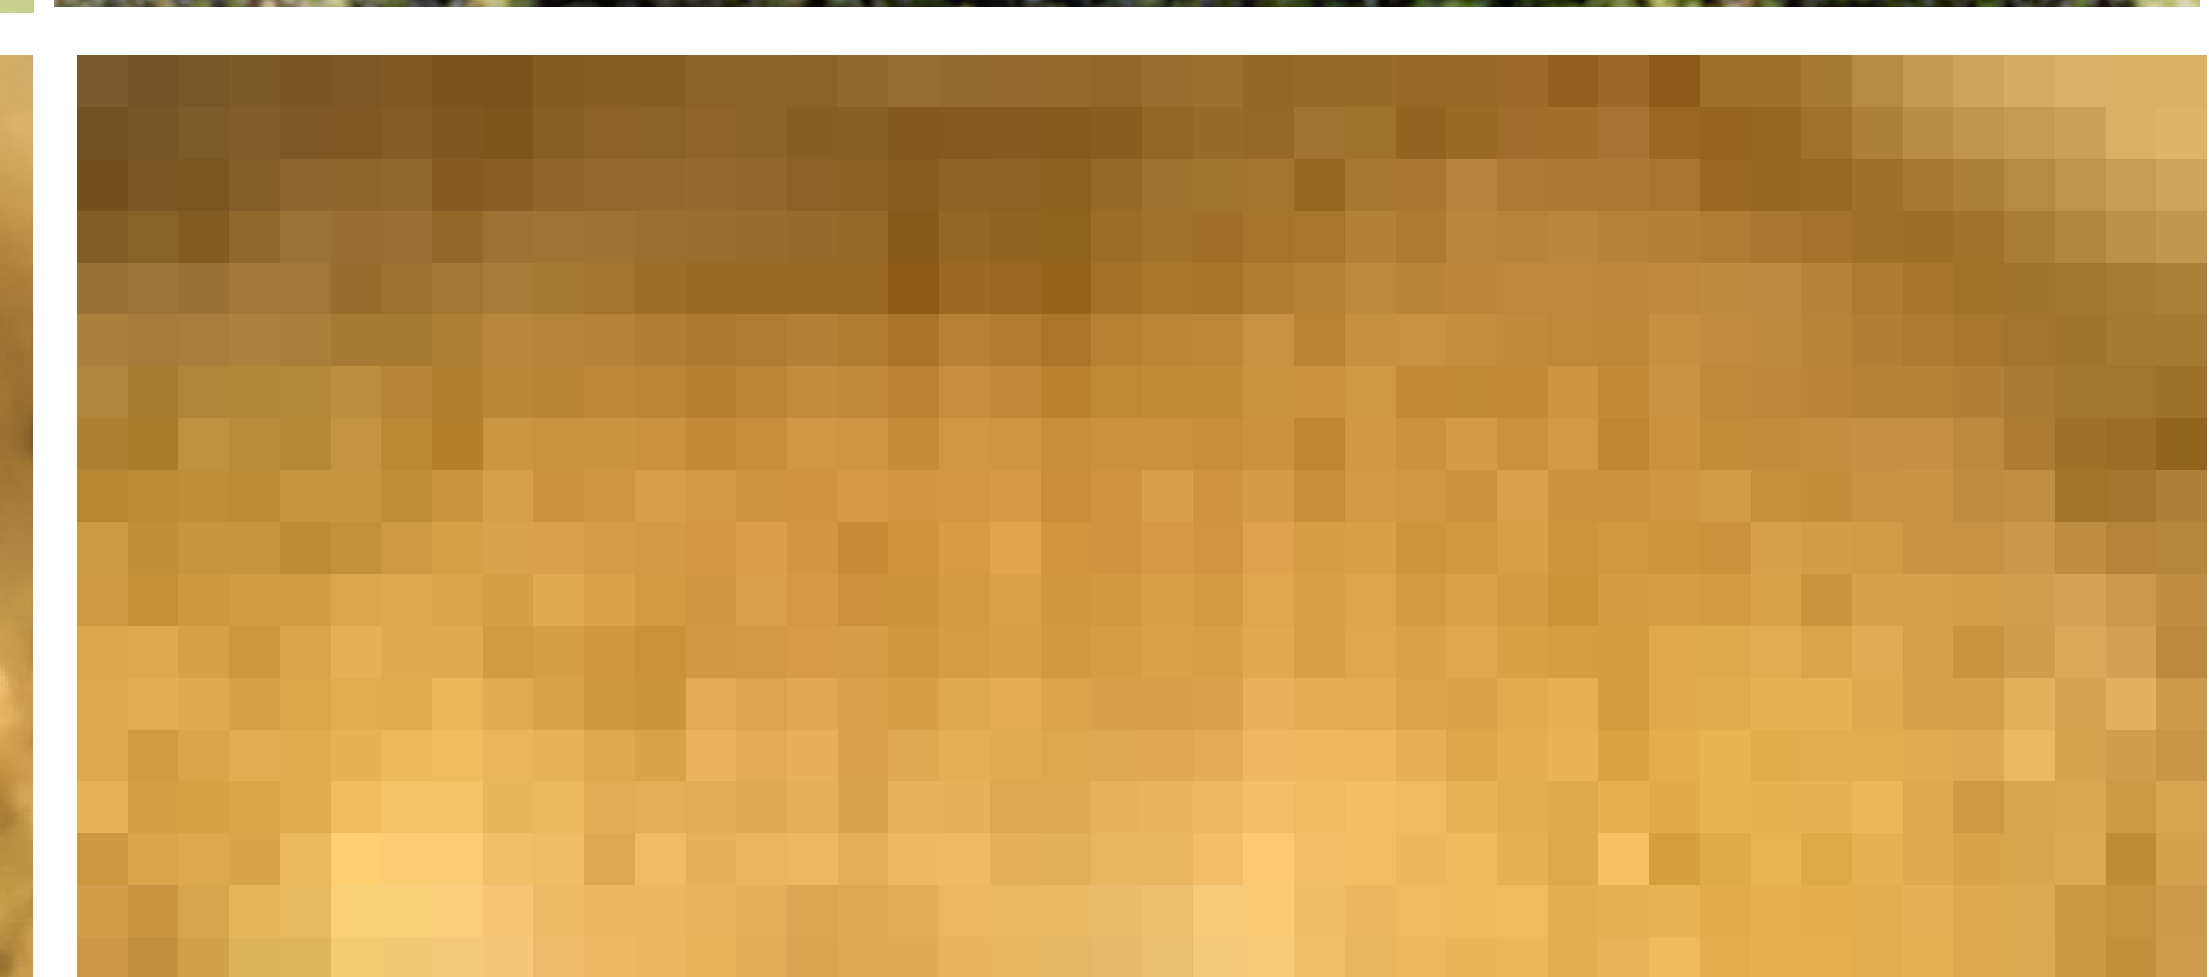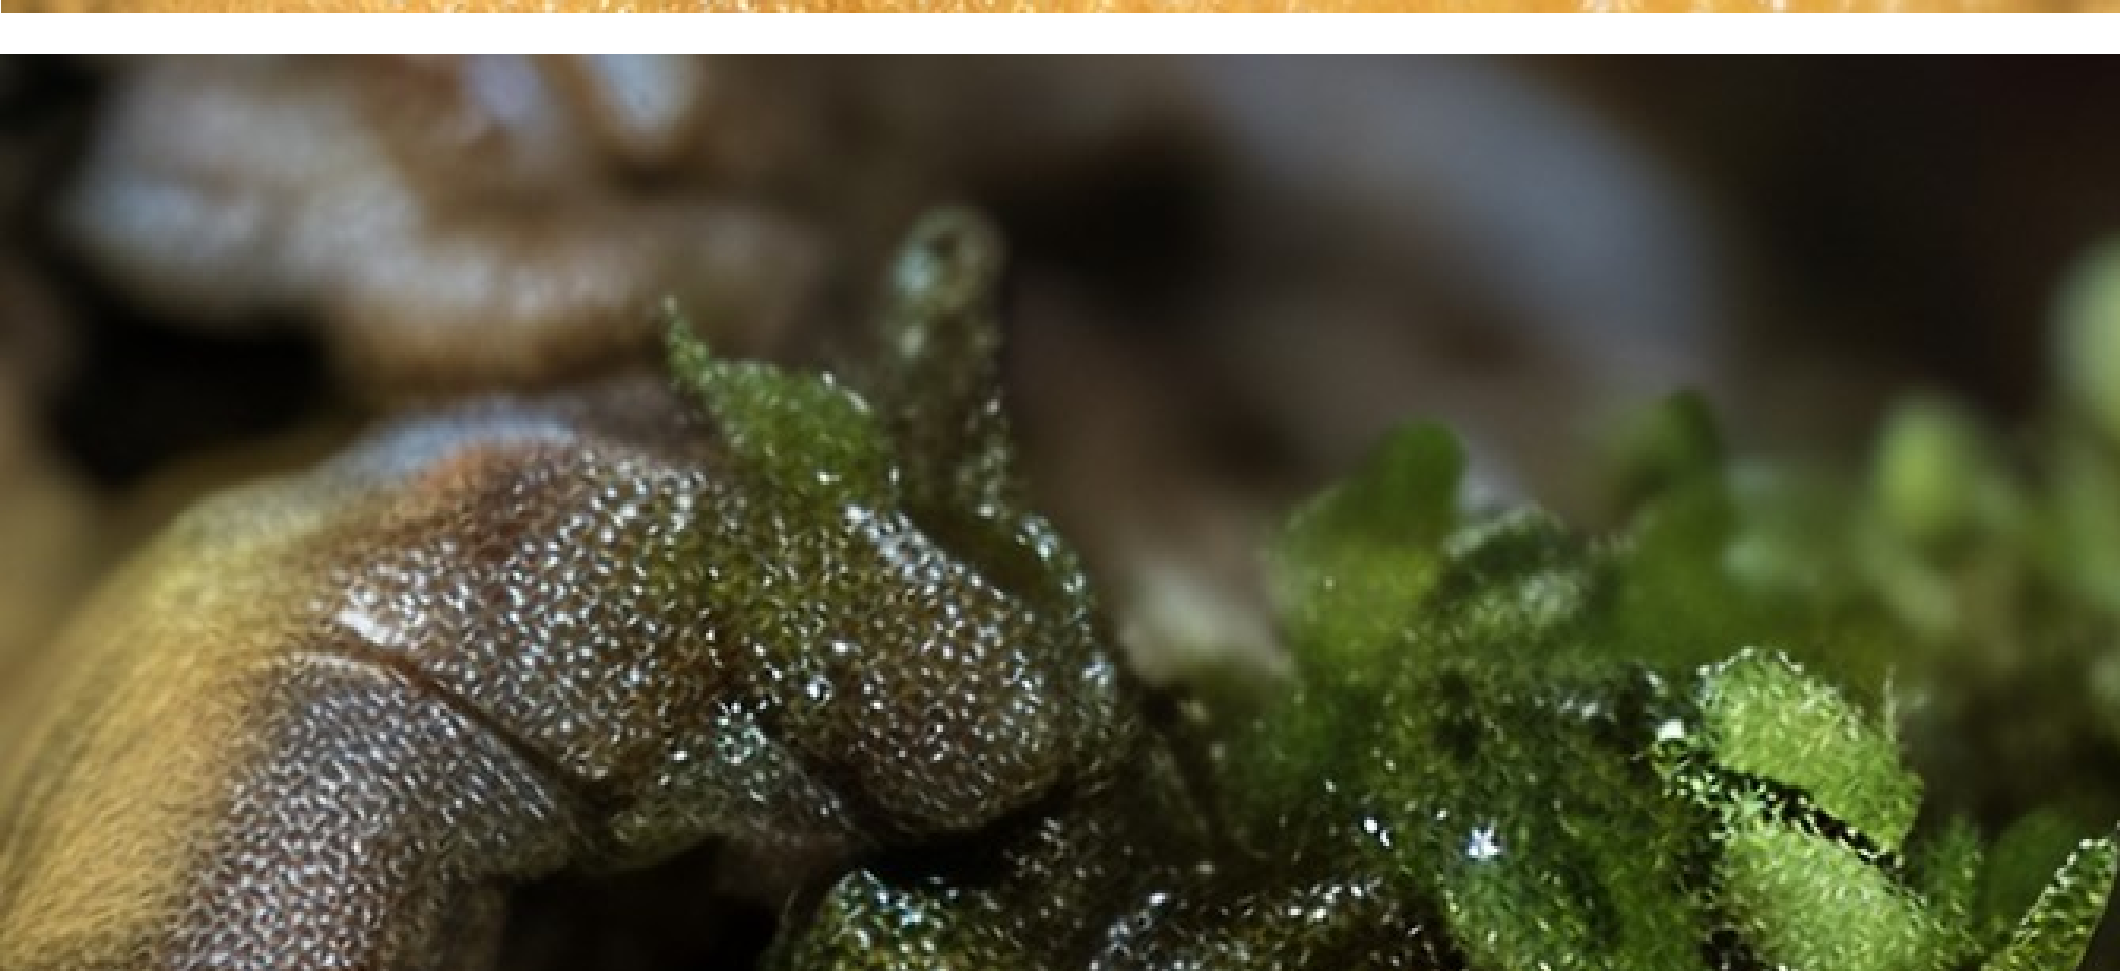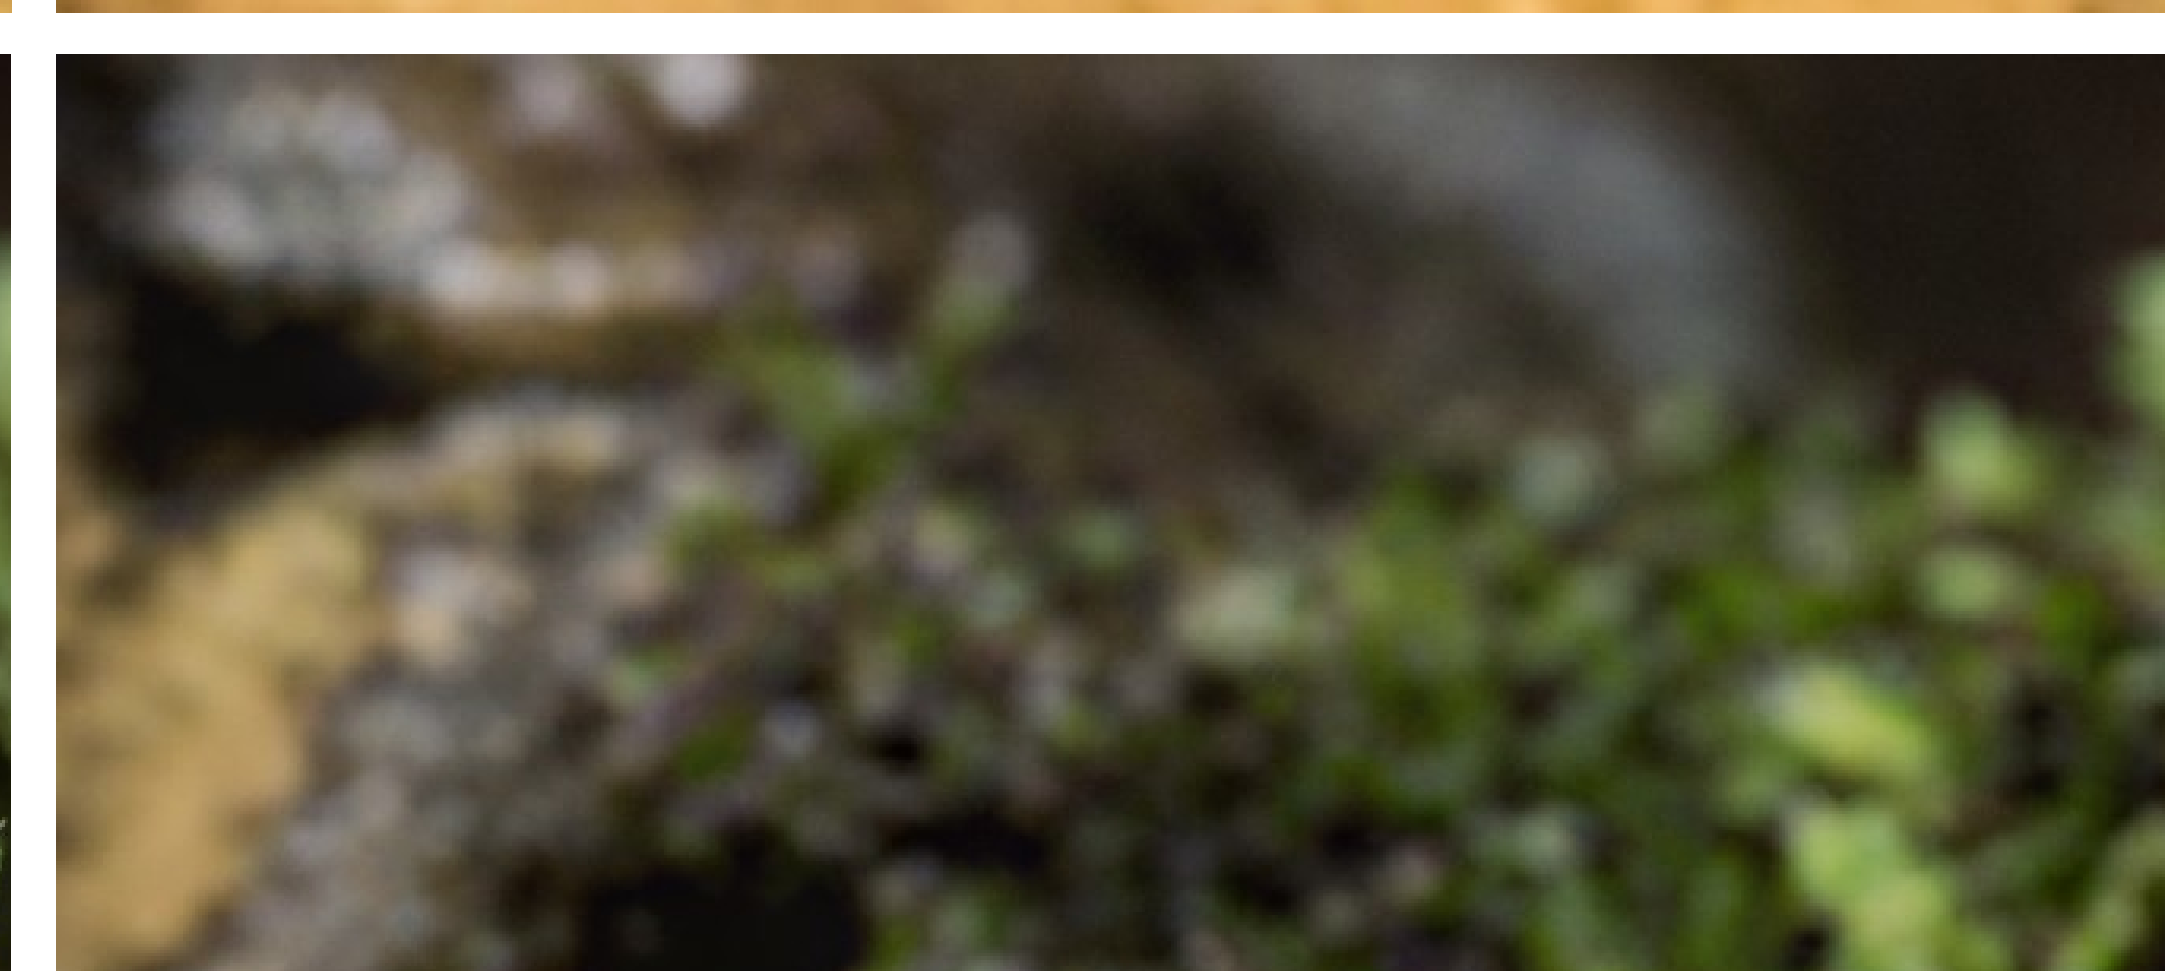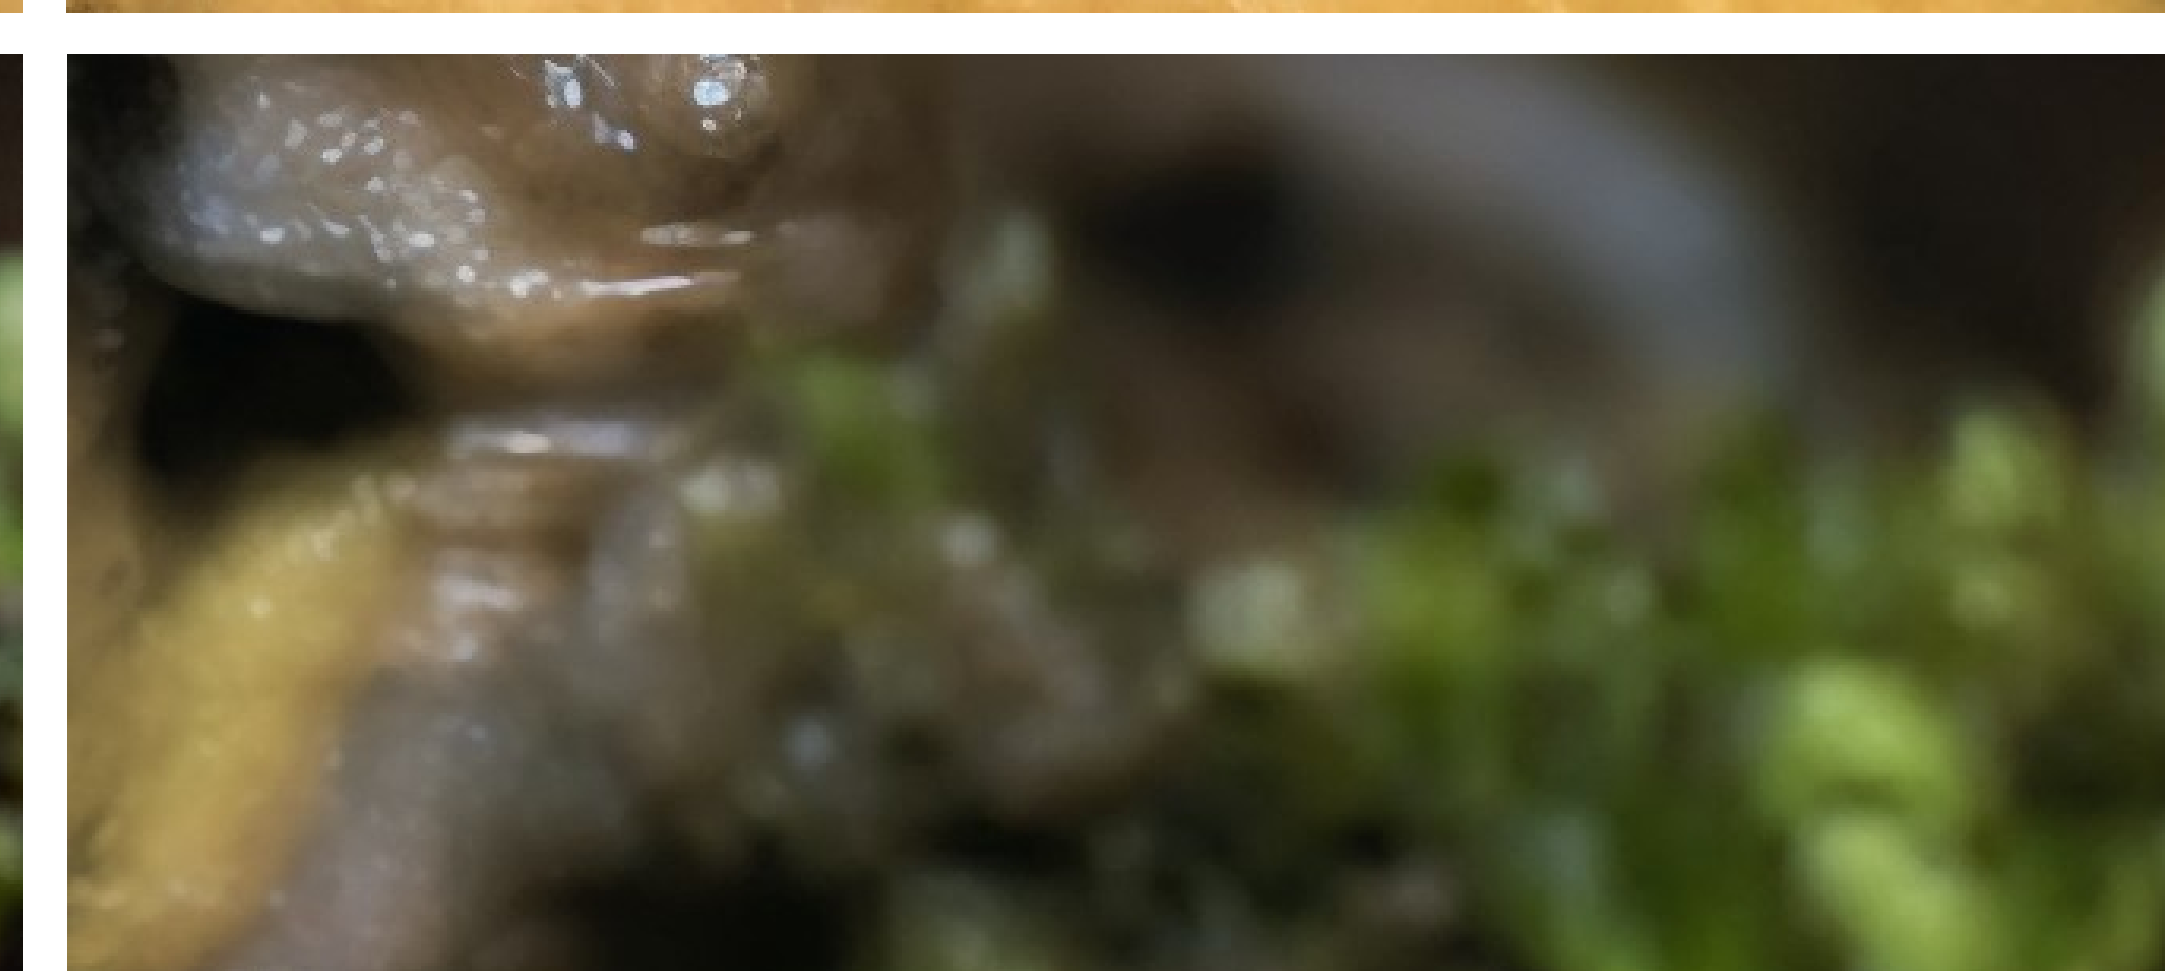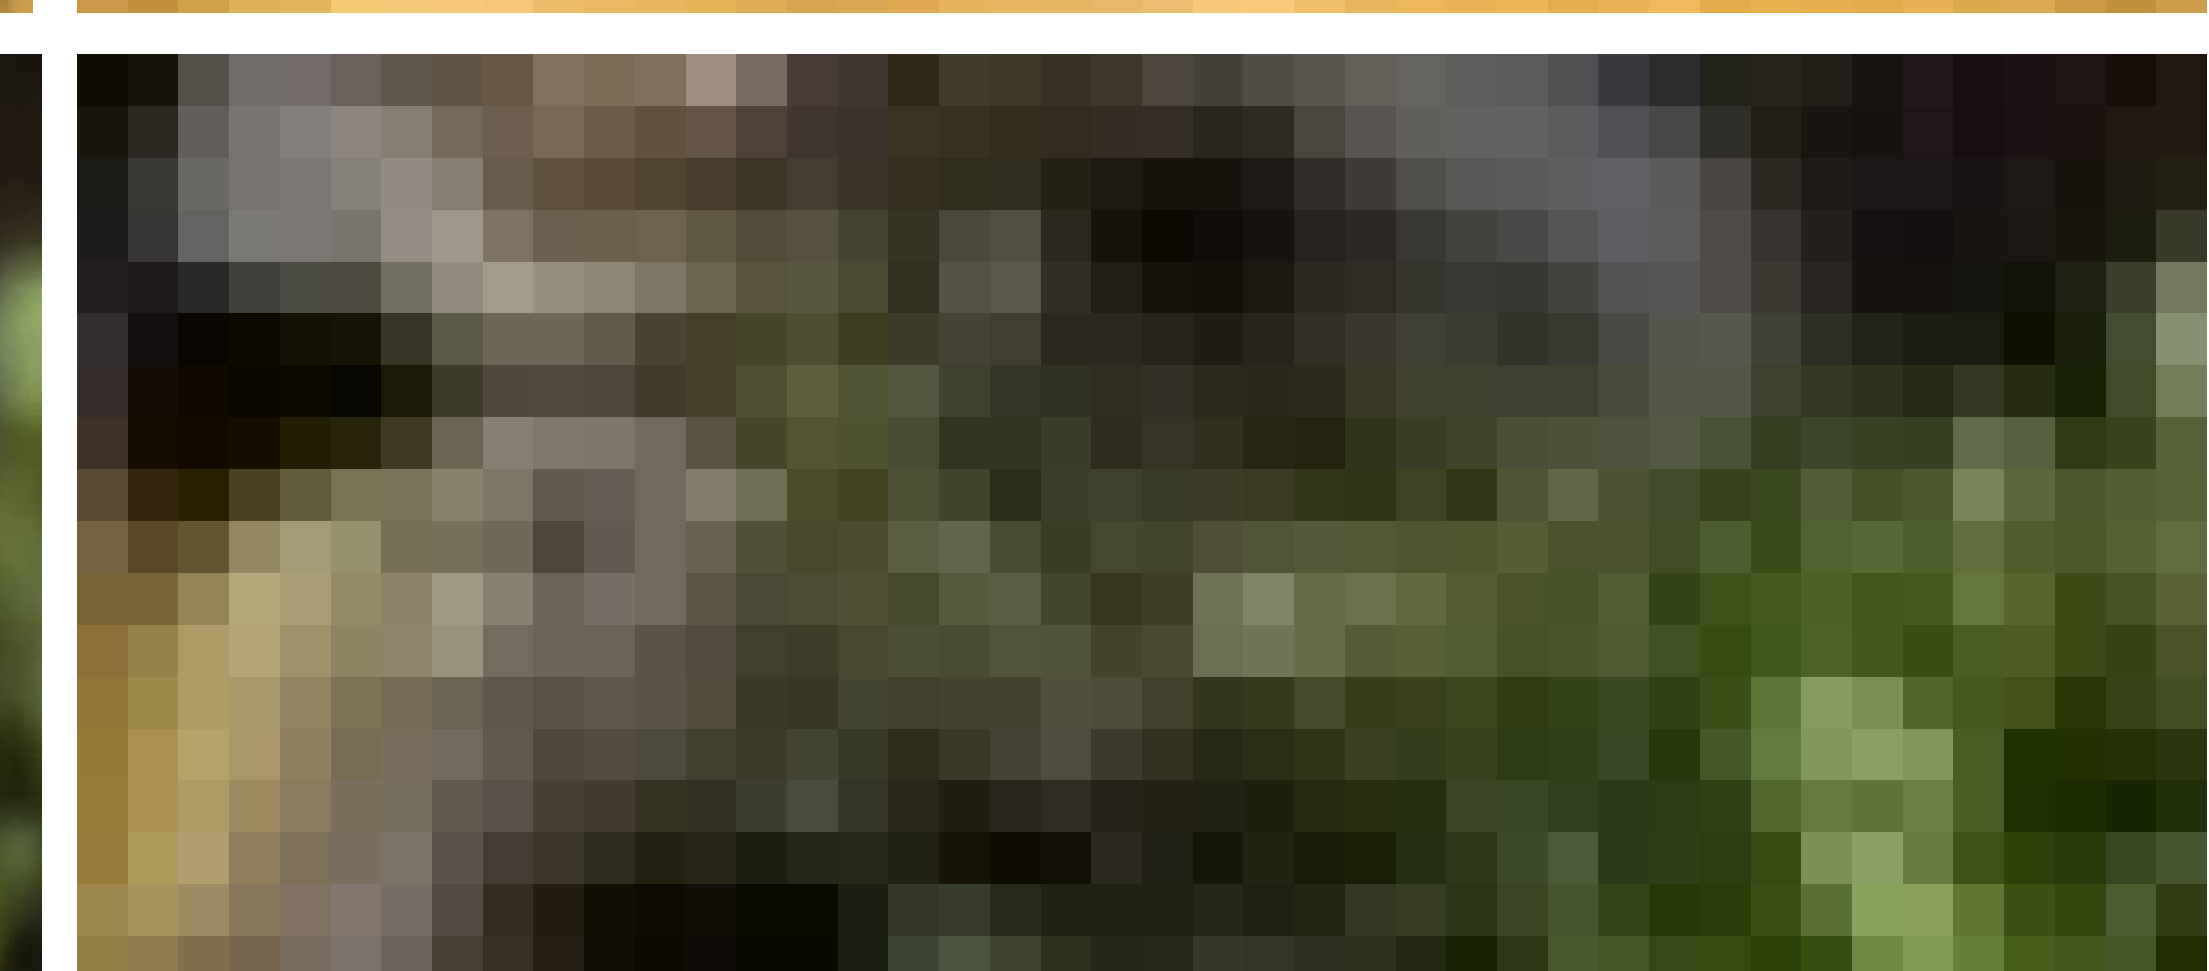

Ours

SUPIR

SeeSR

Input



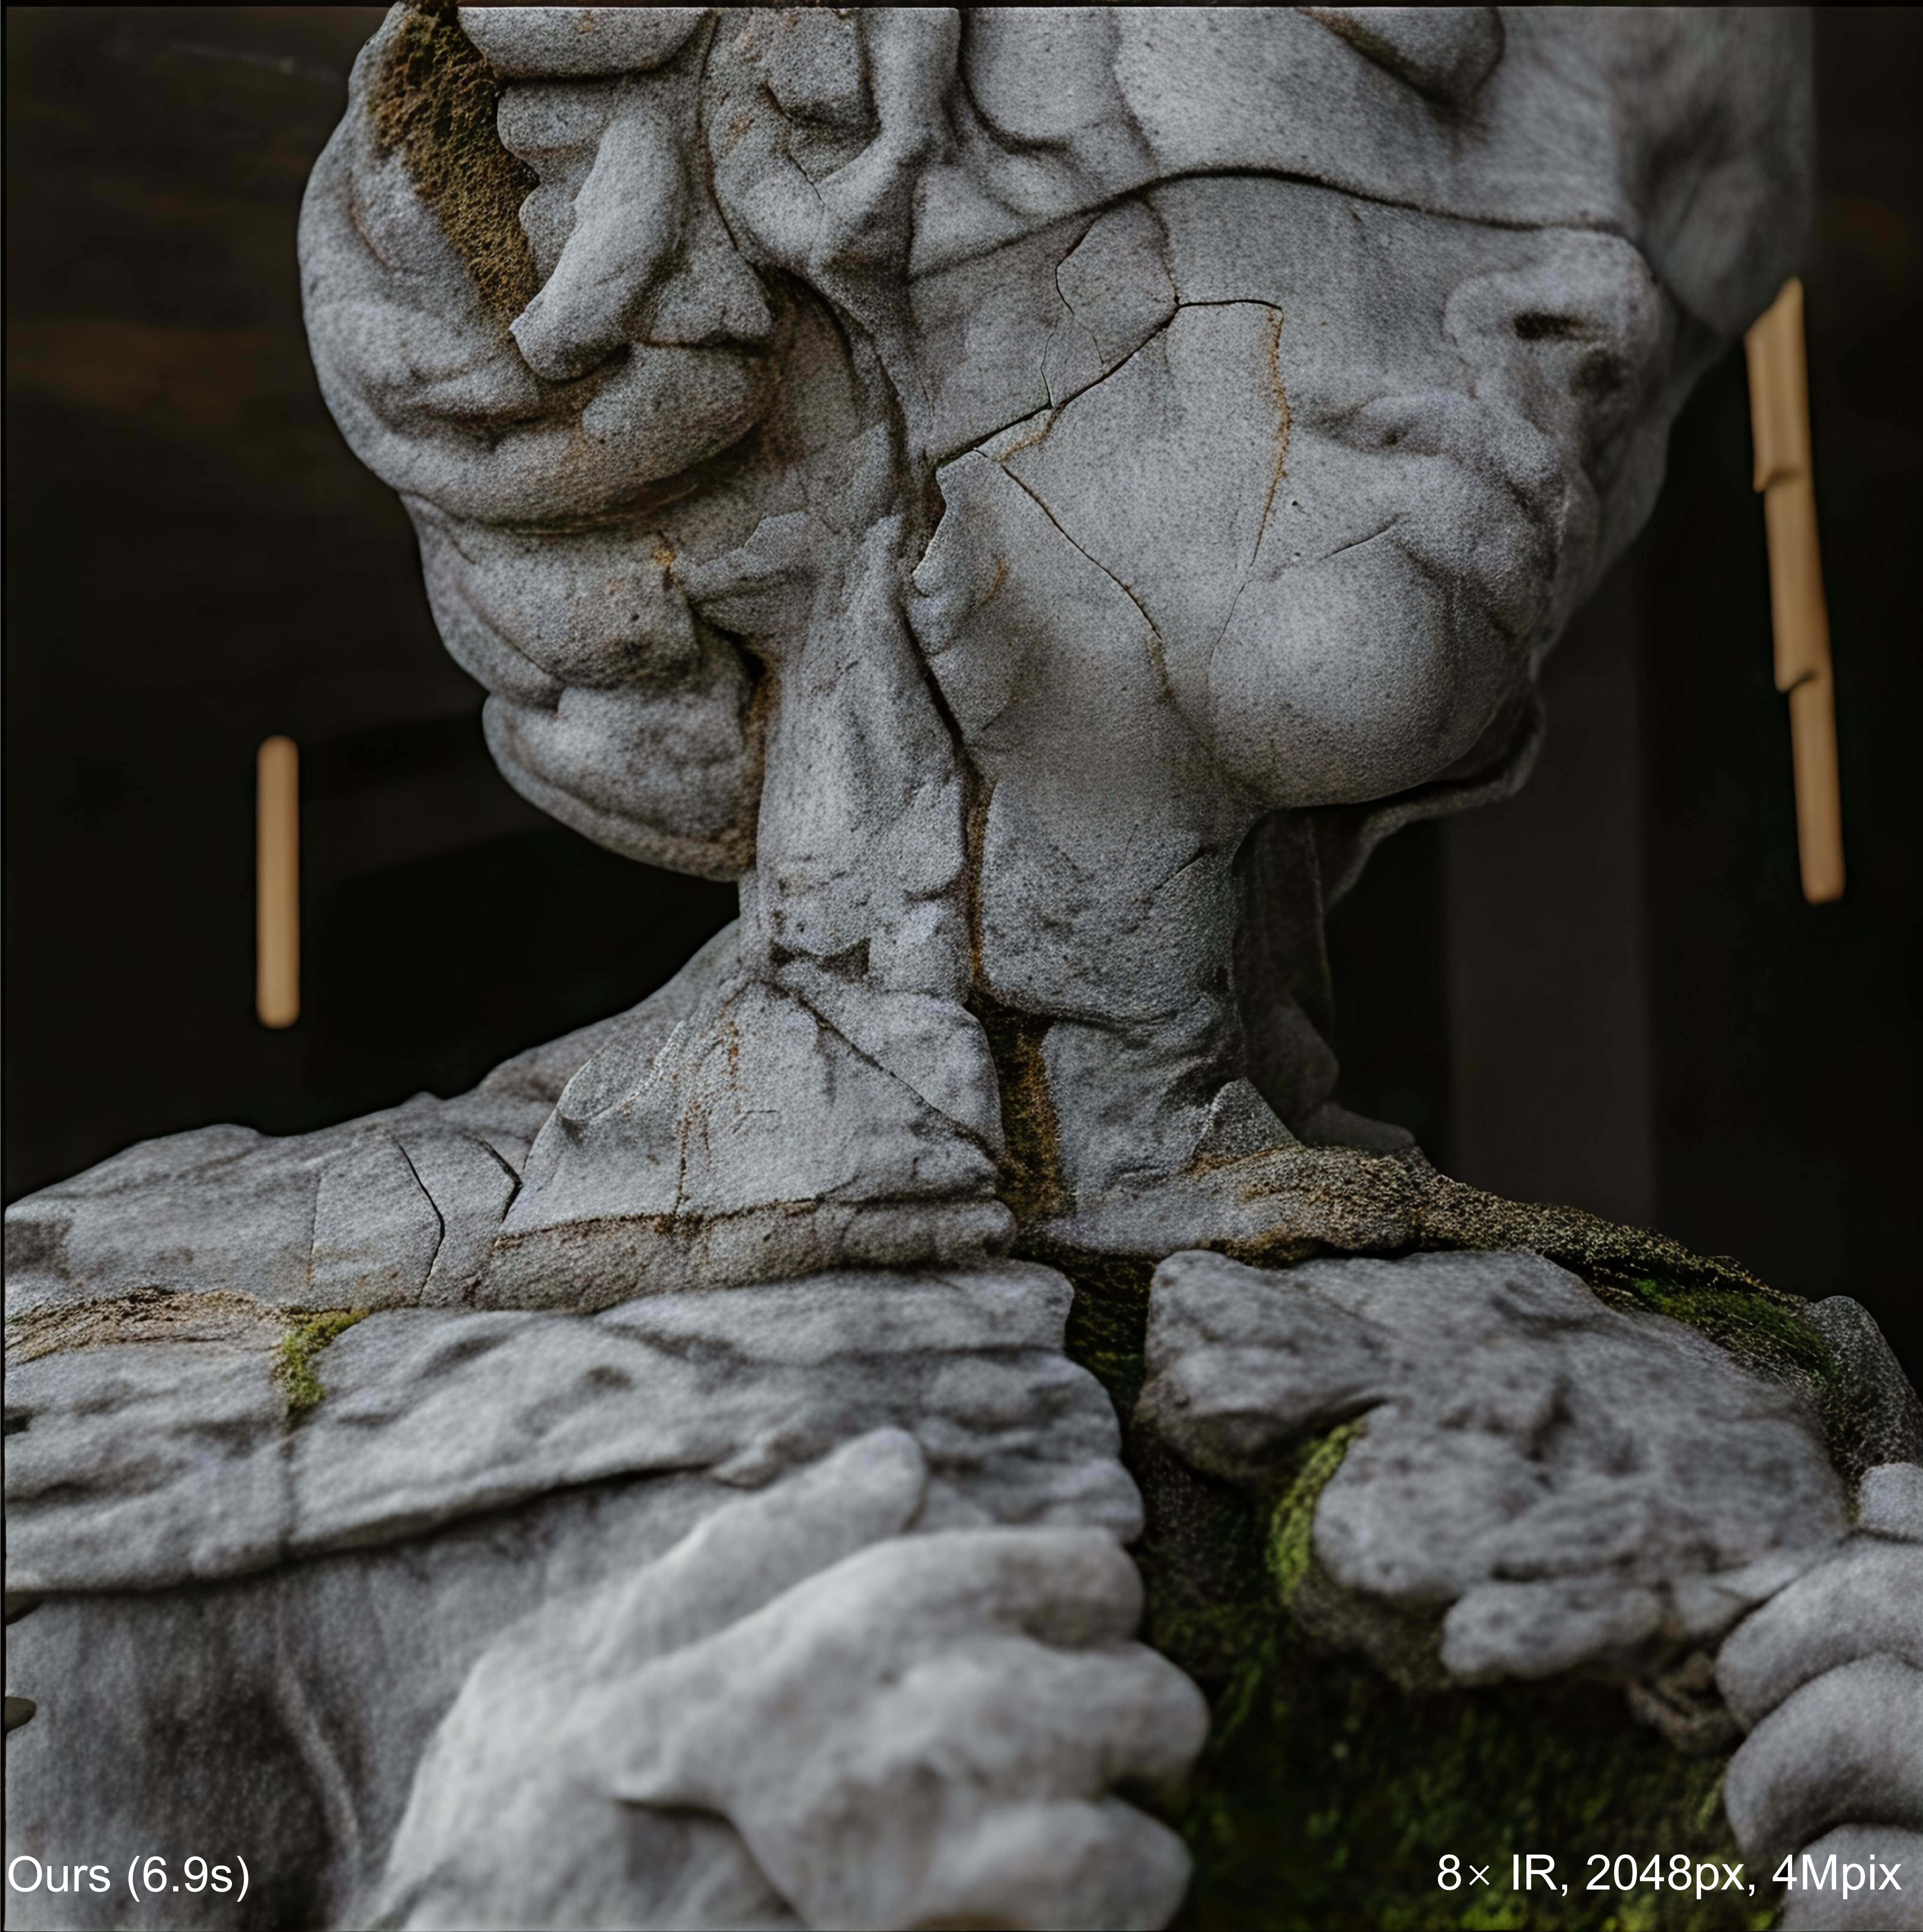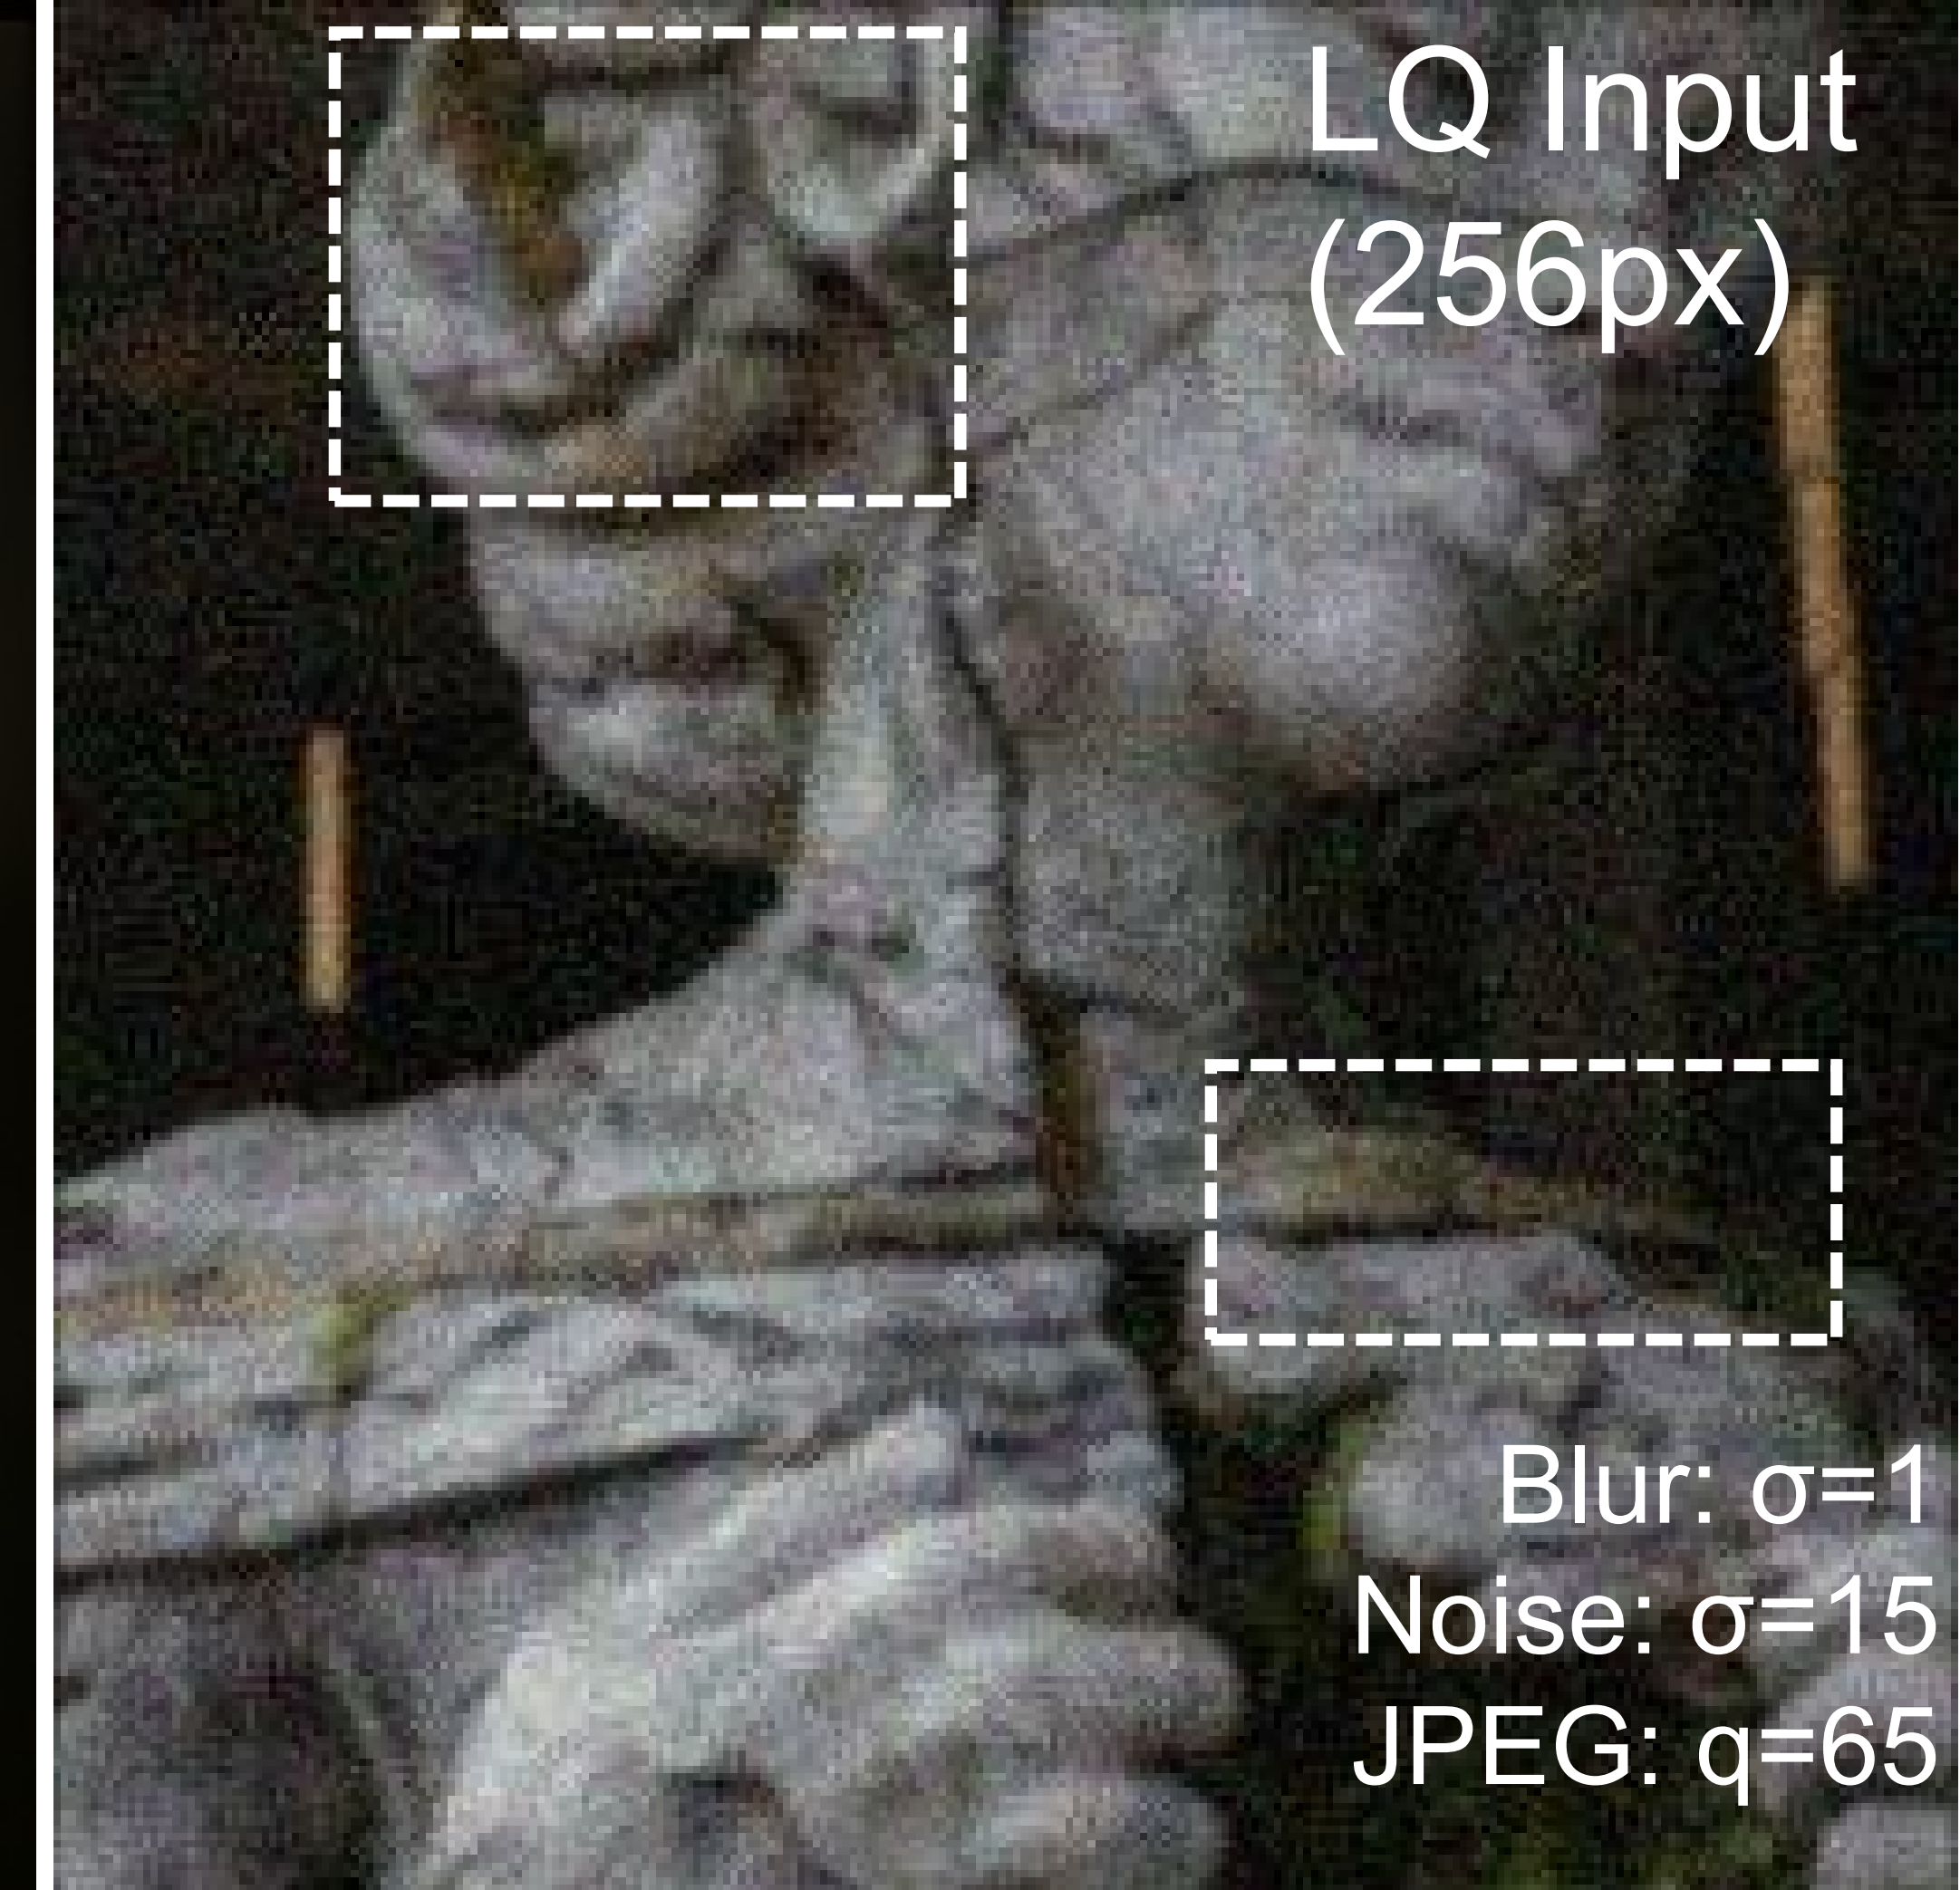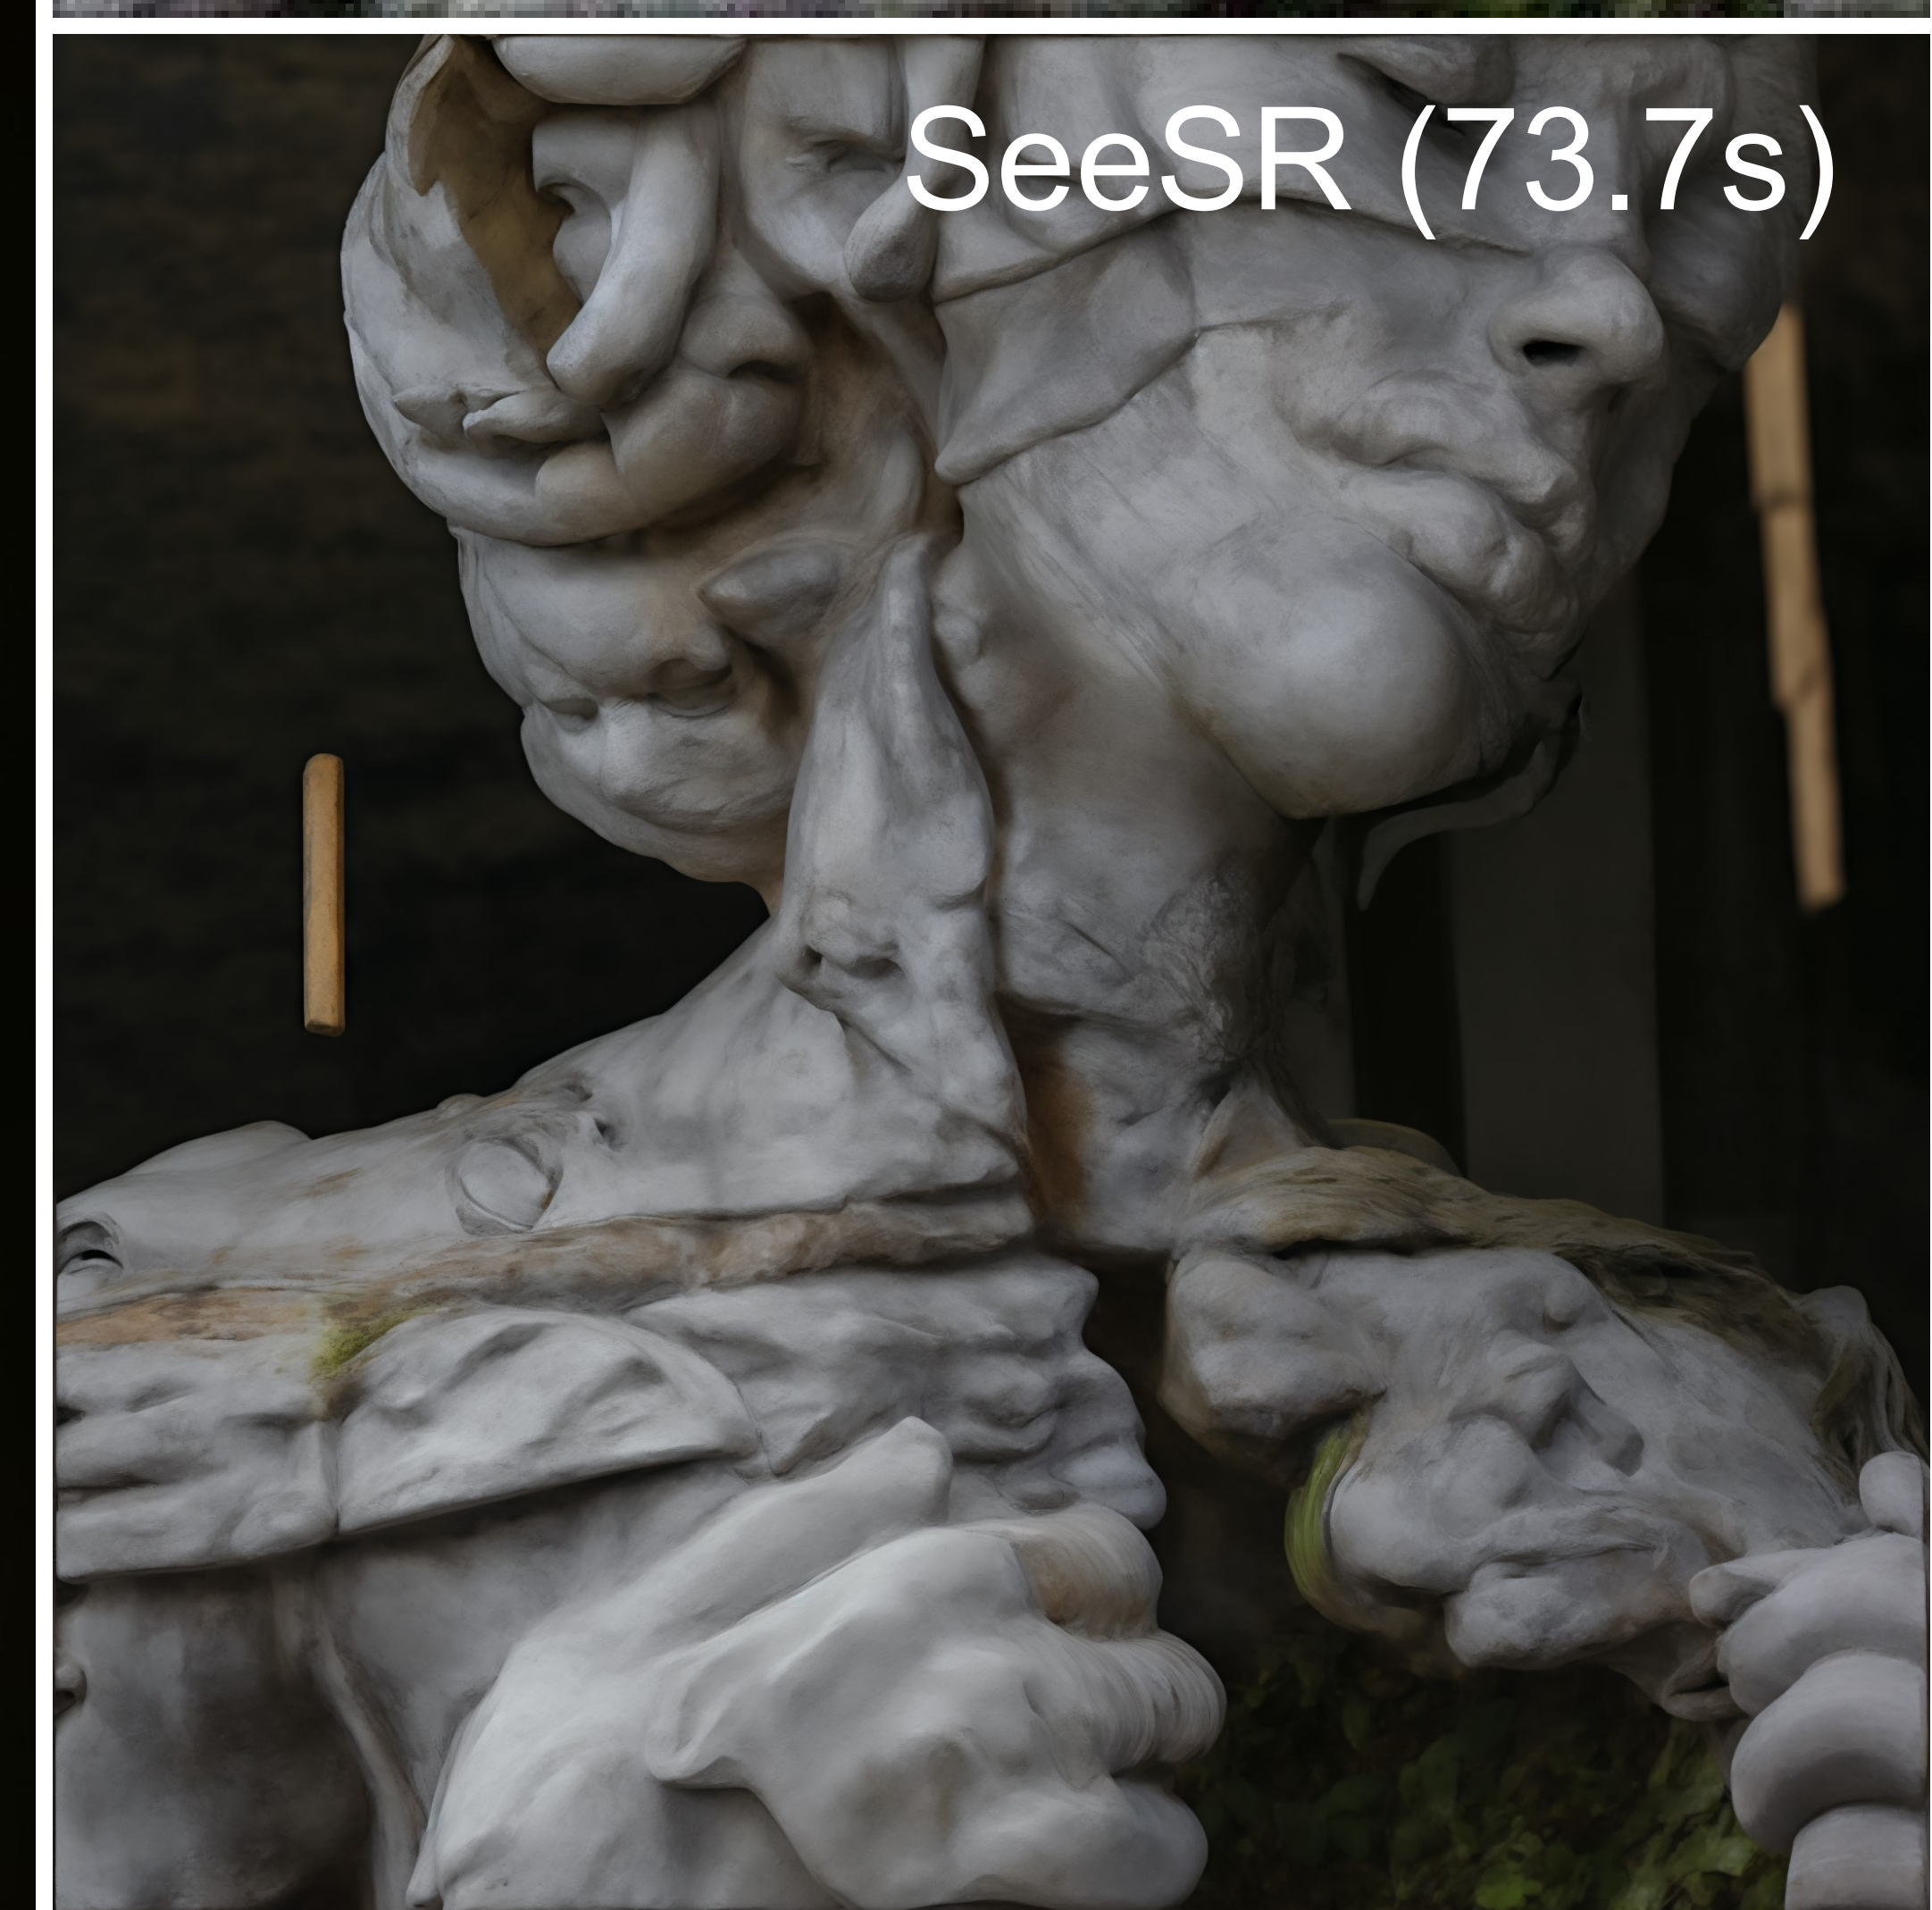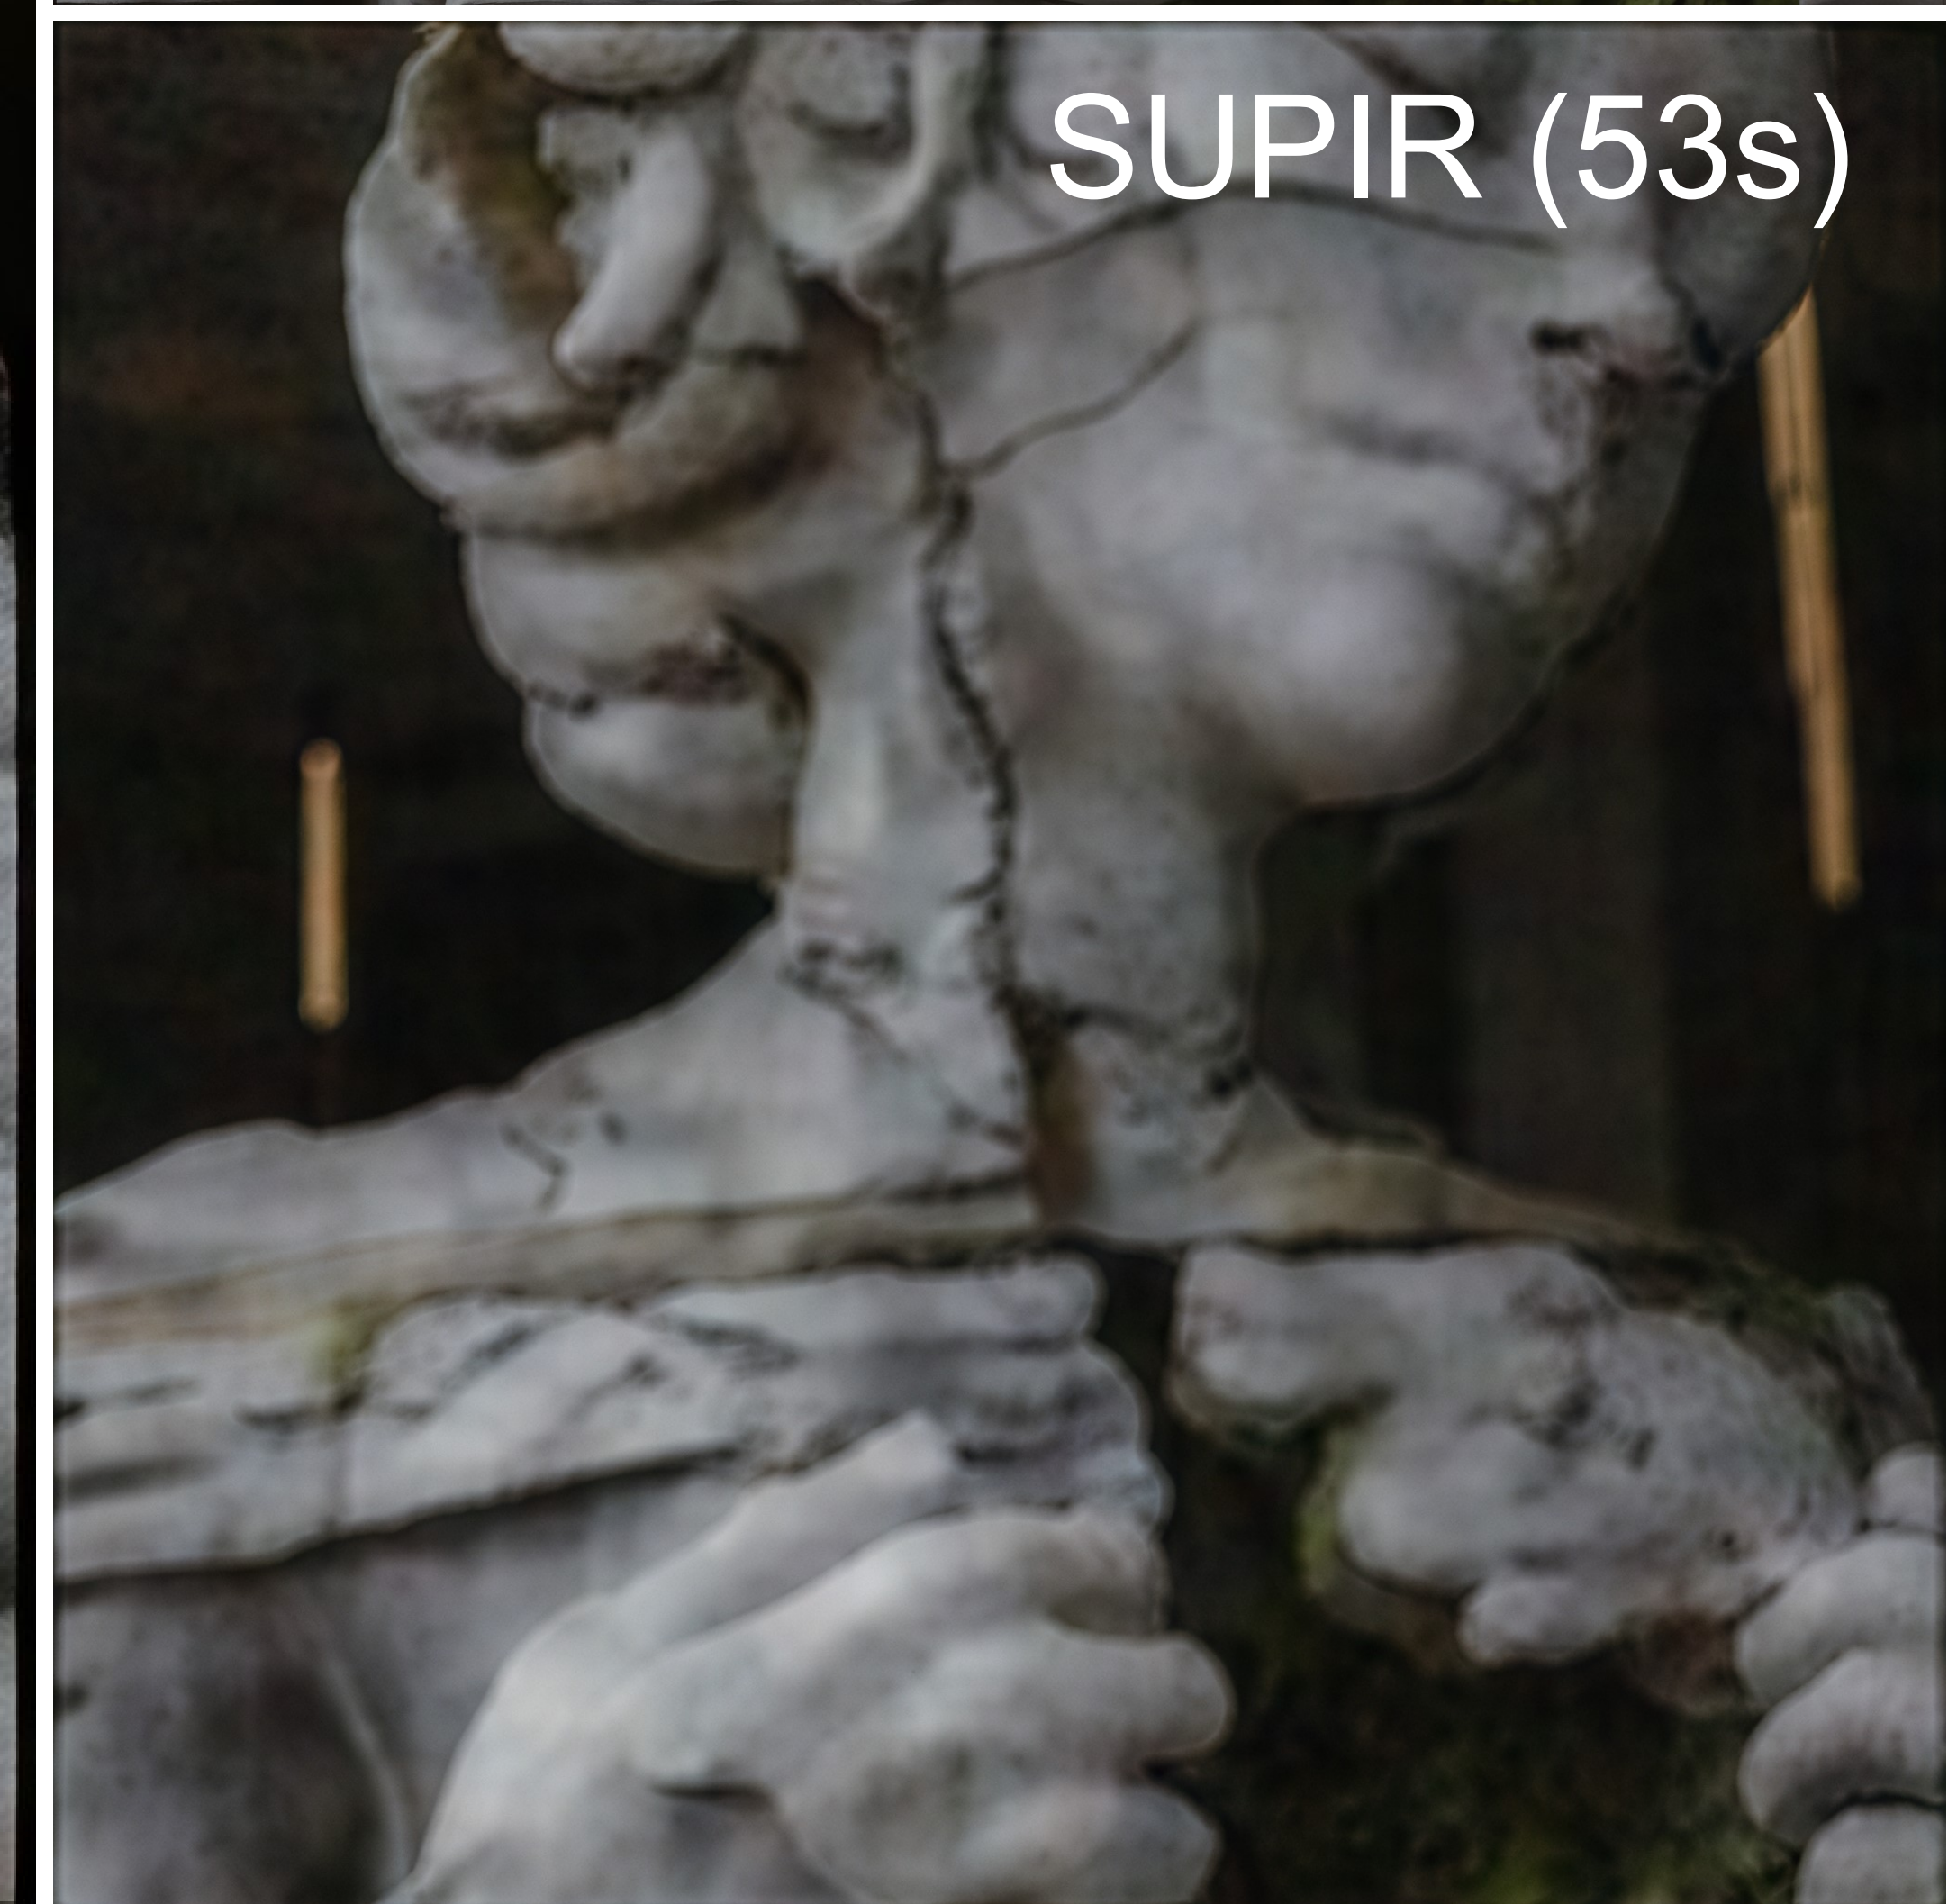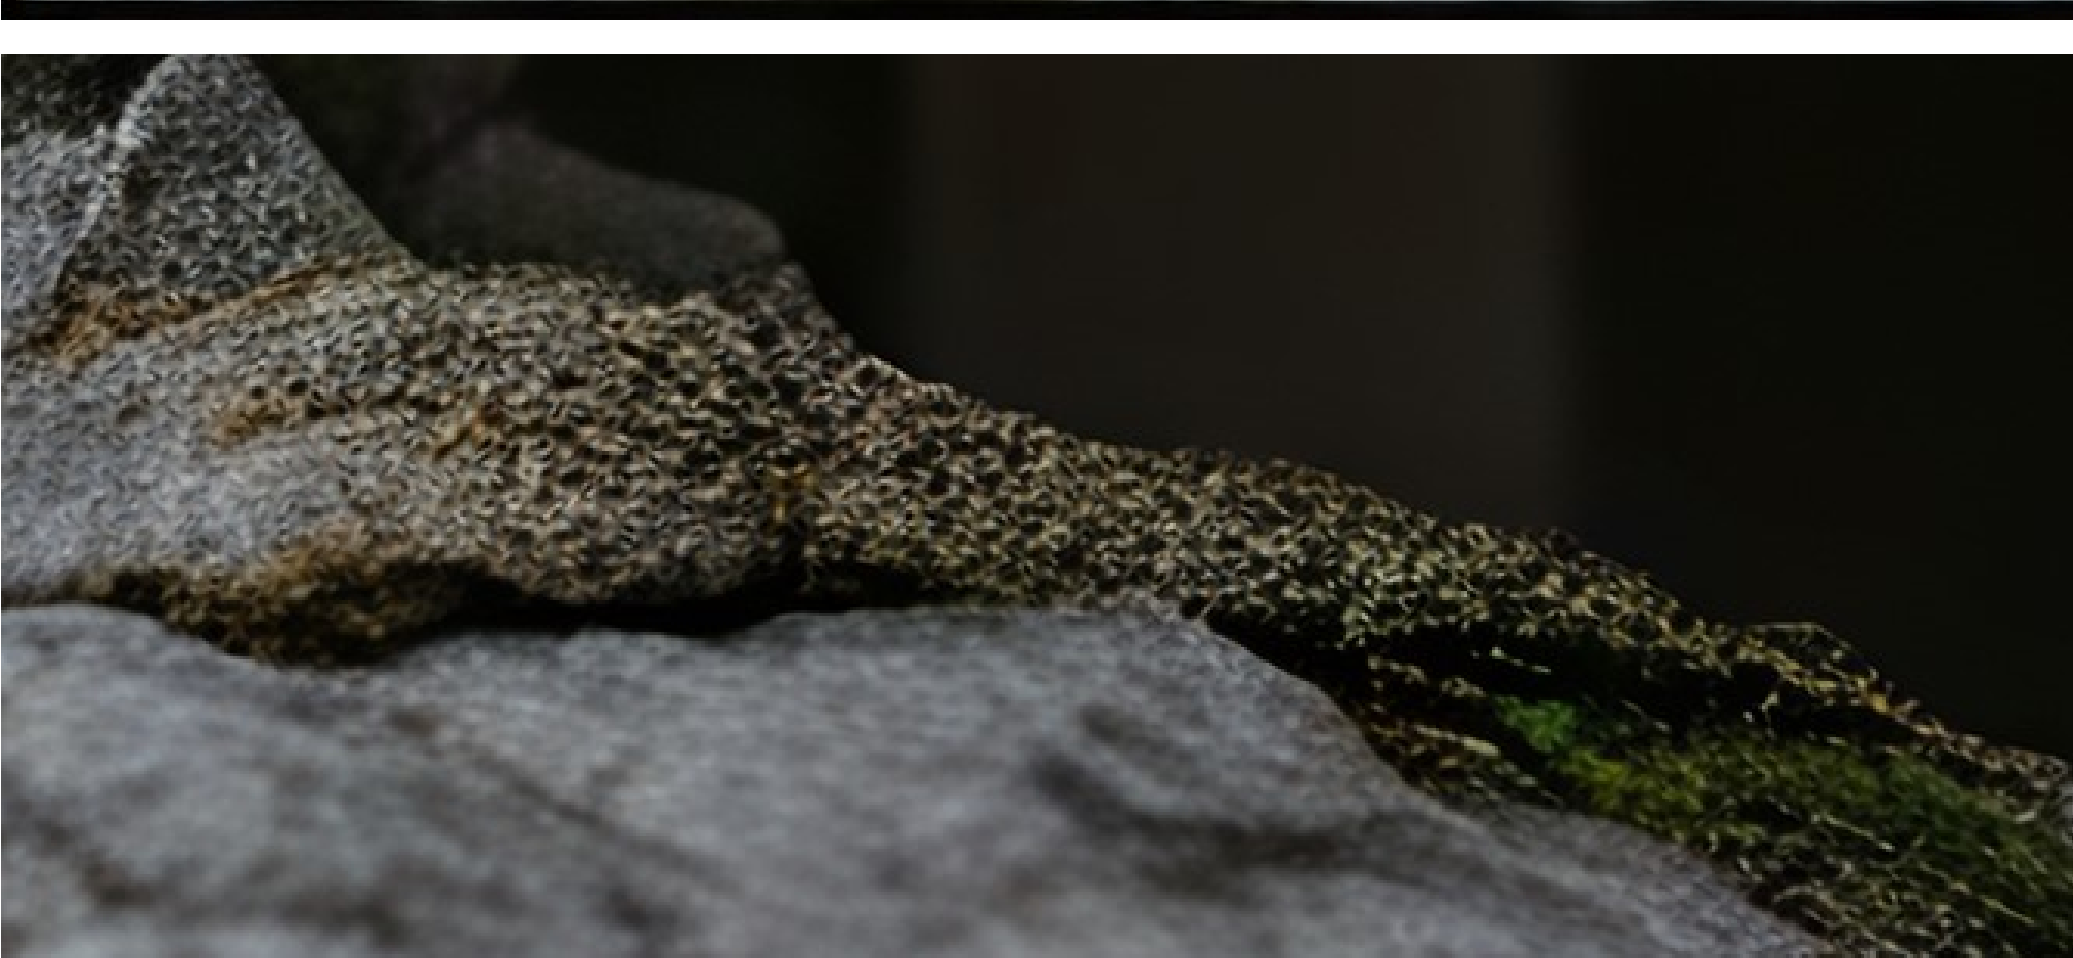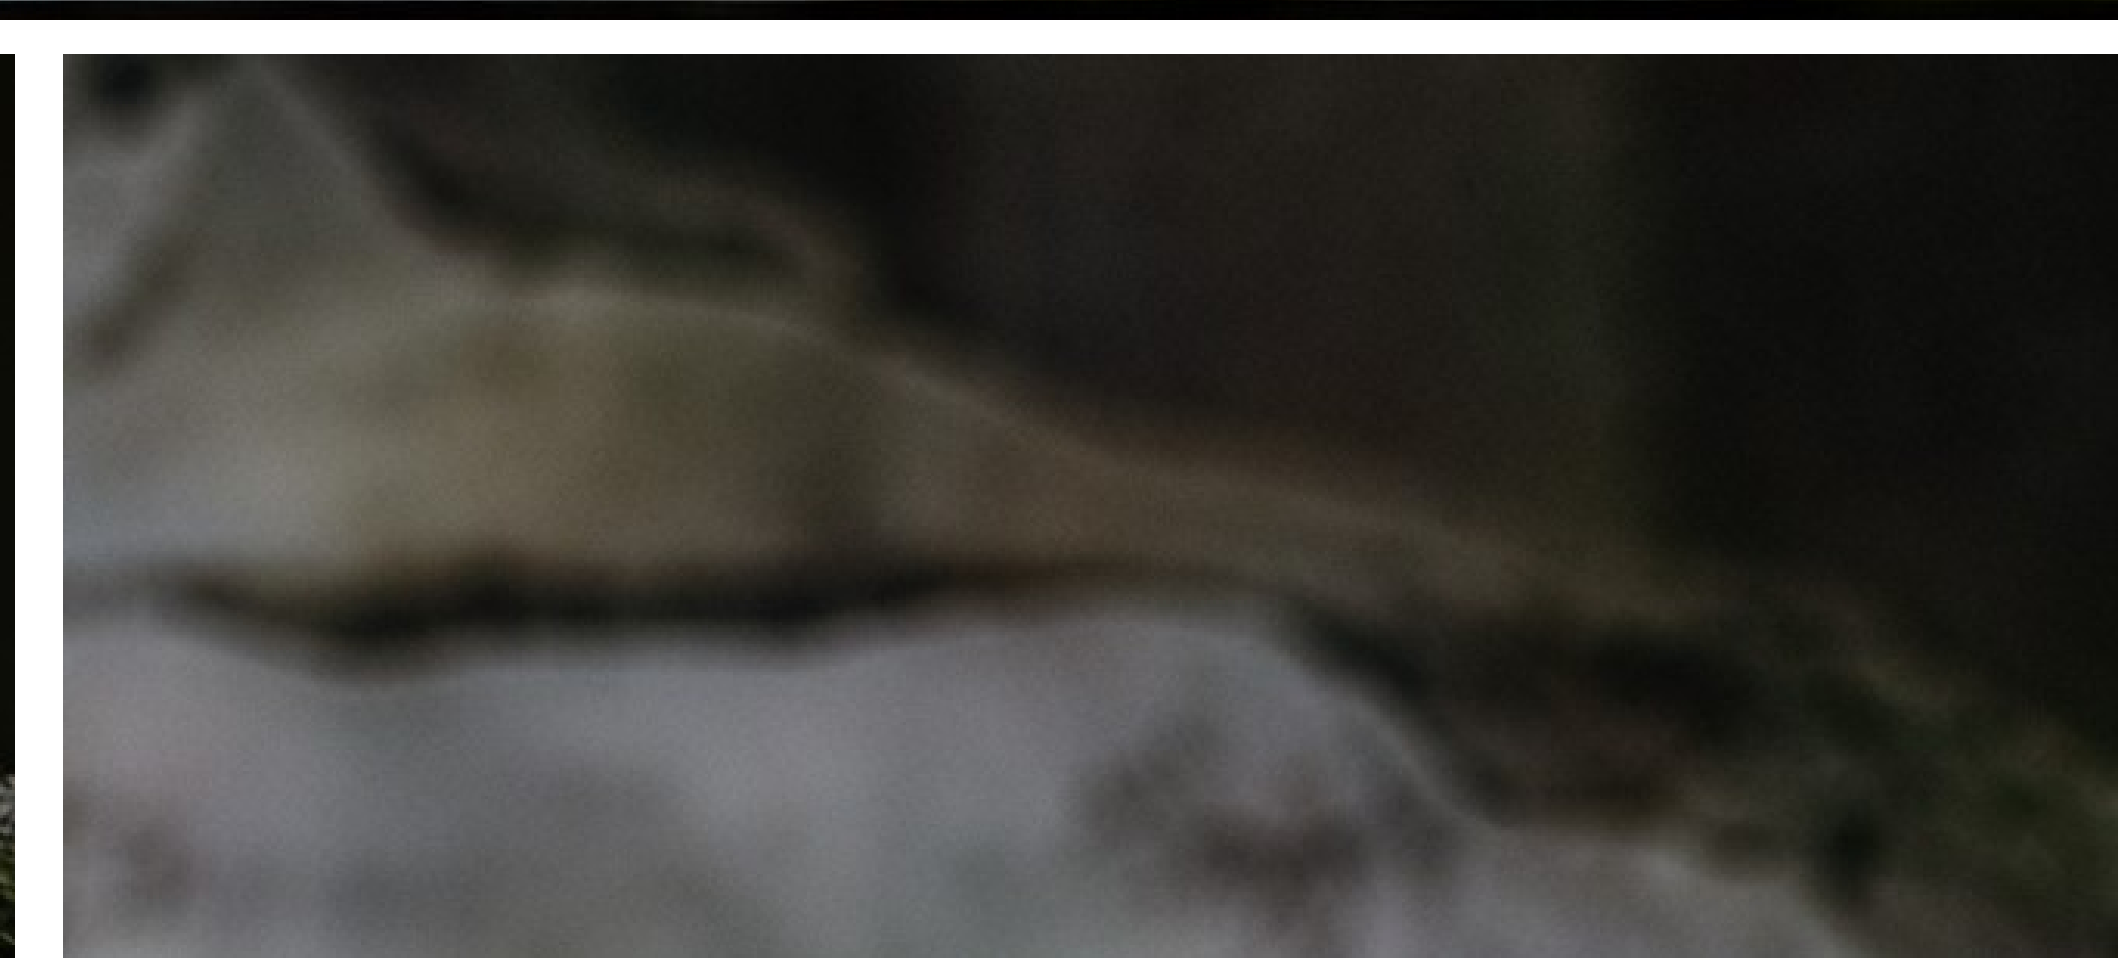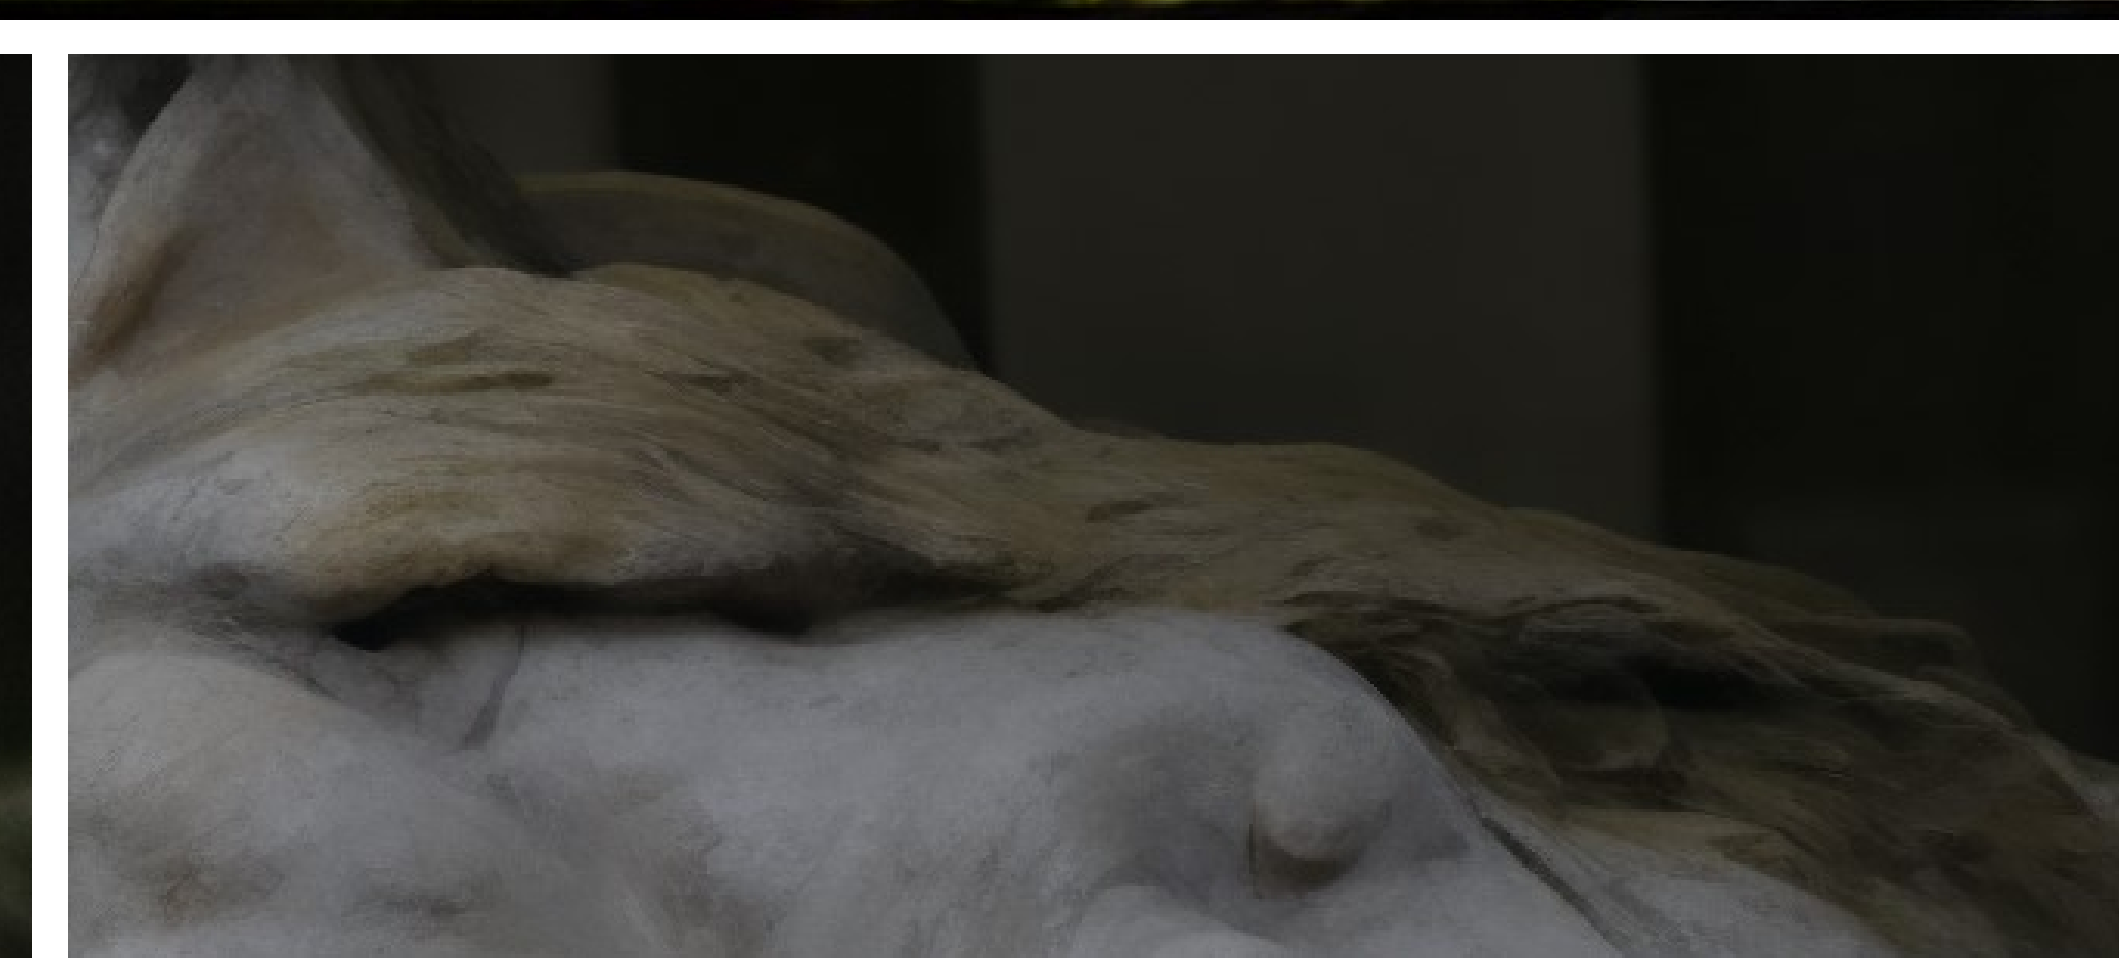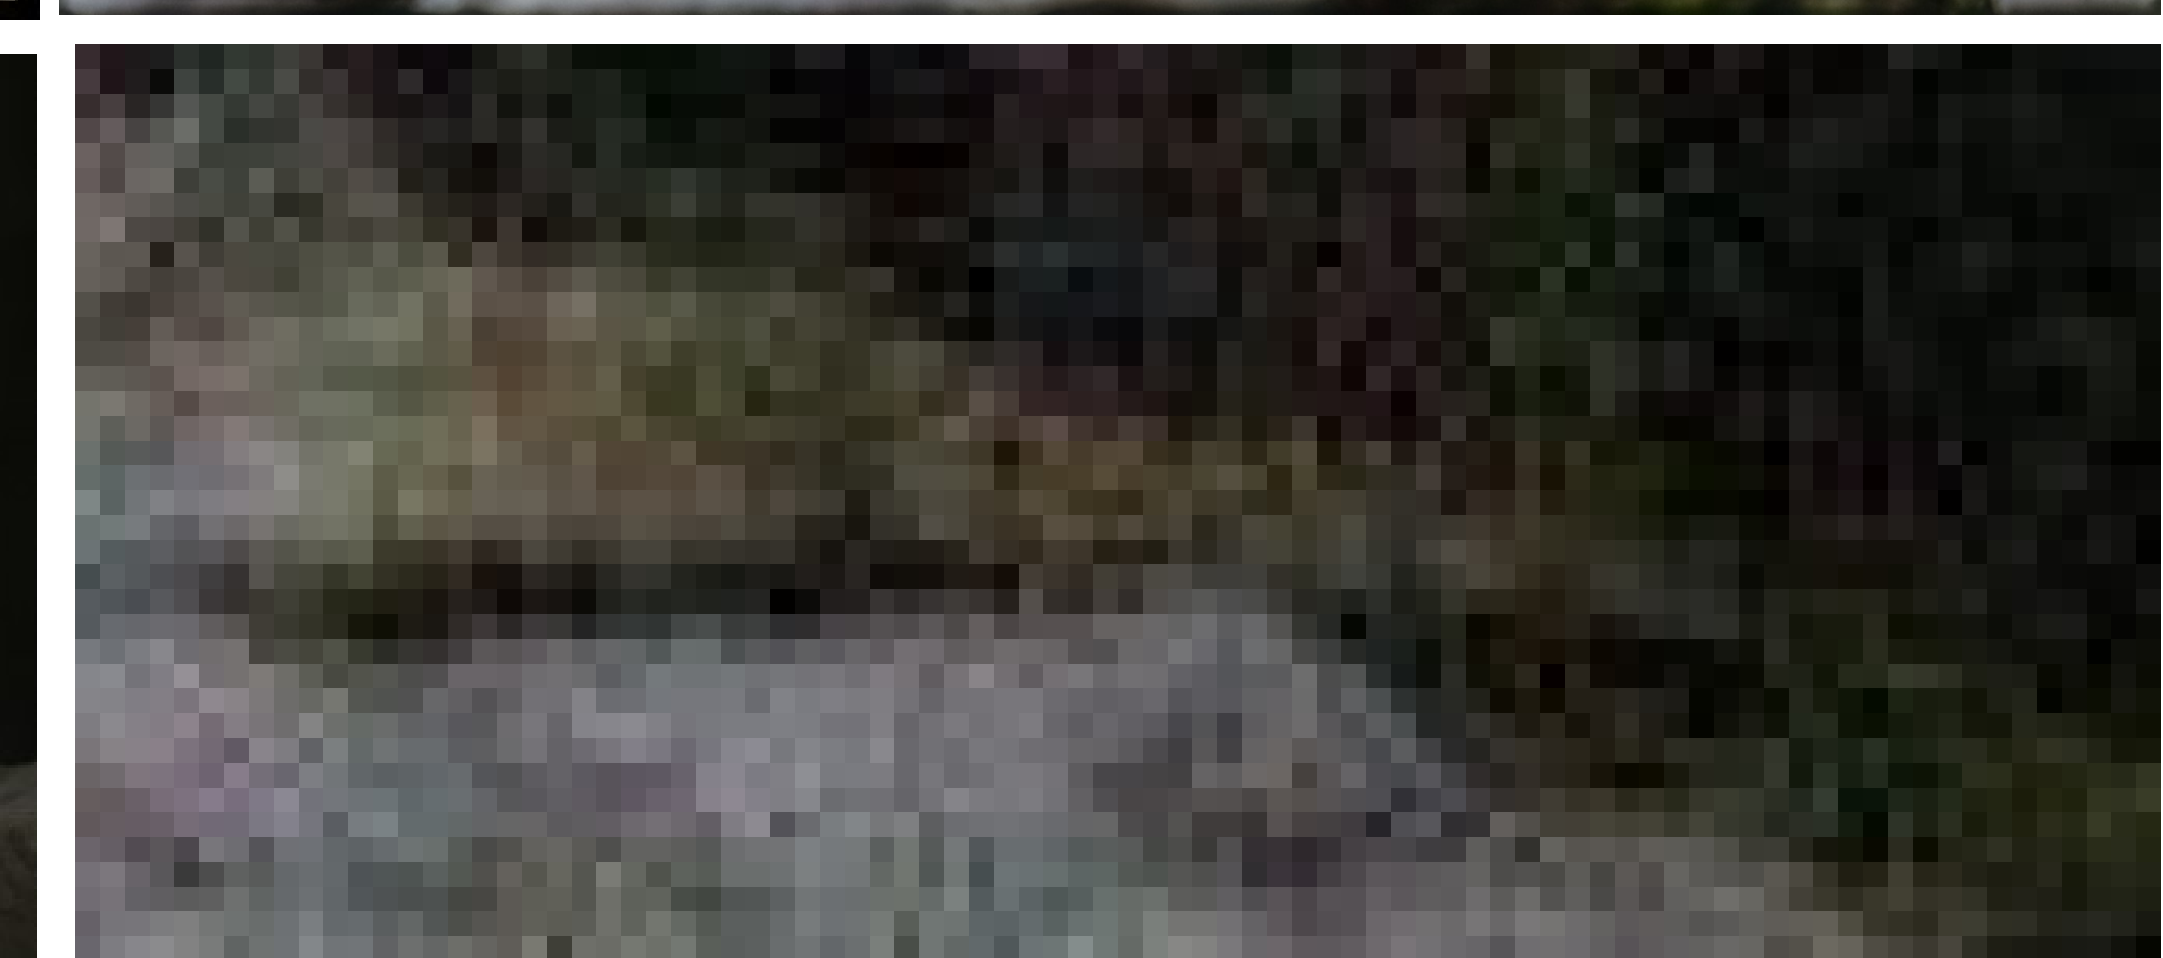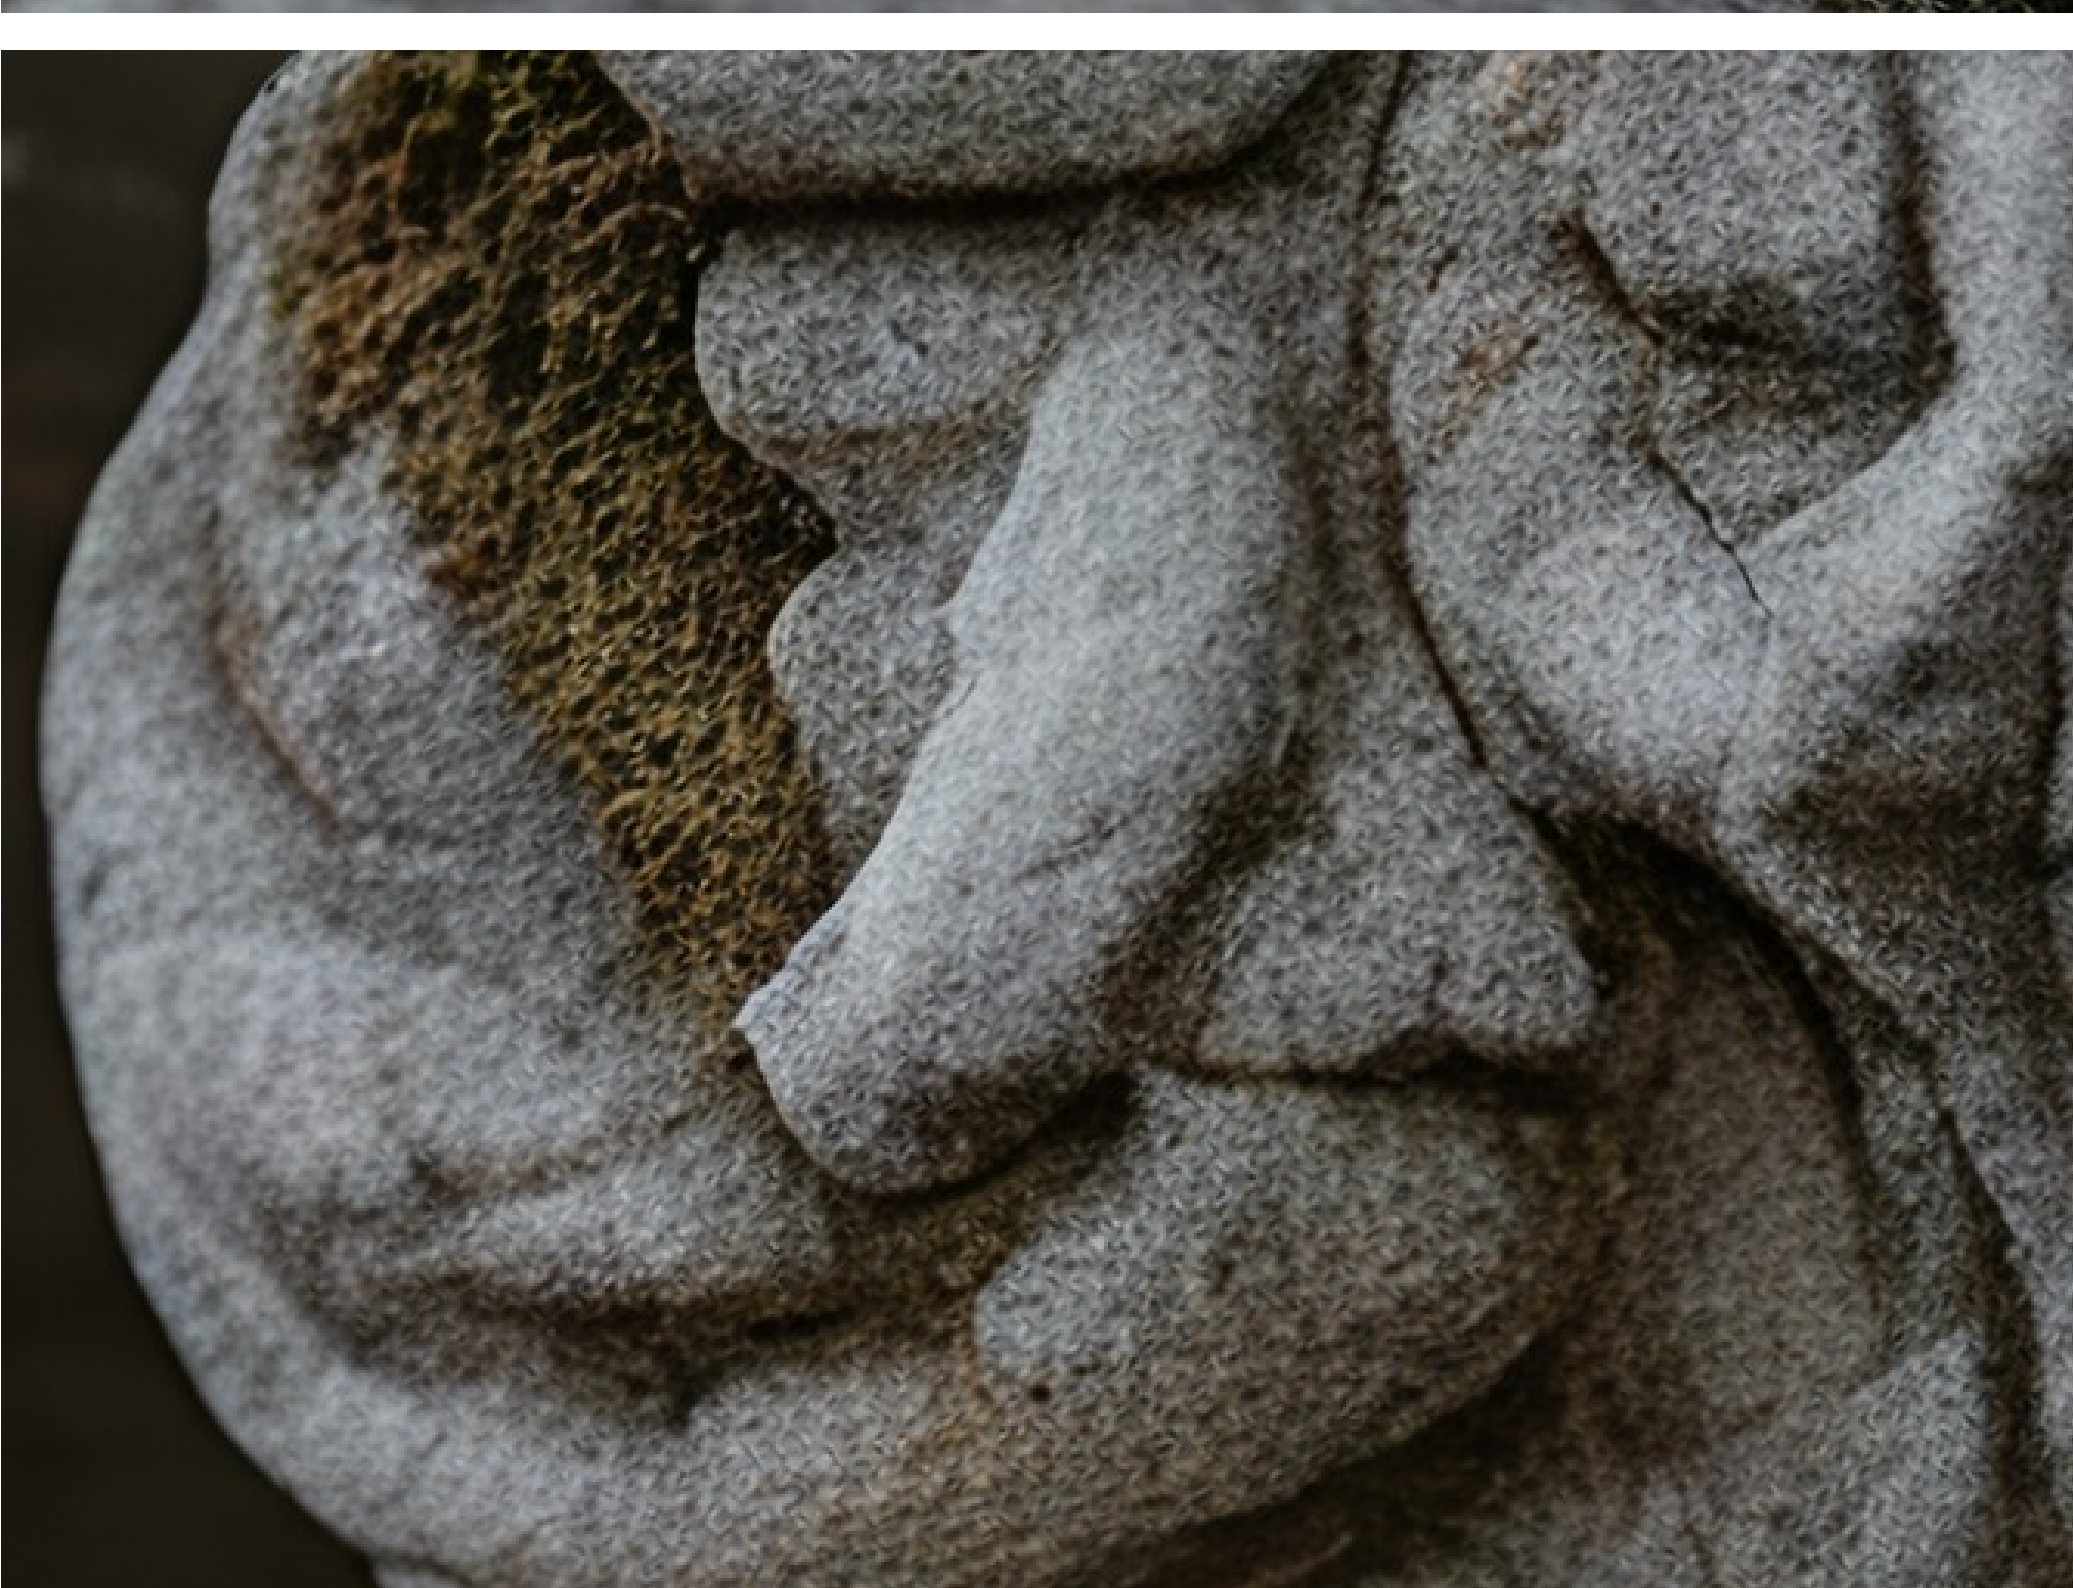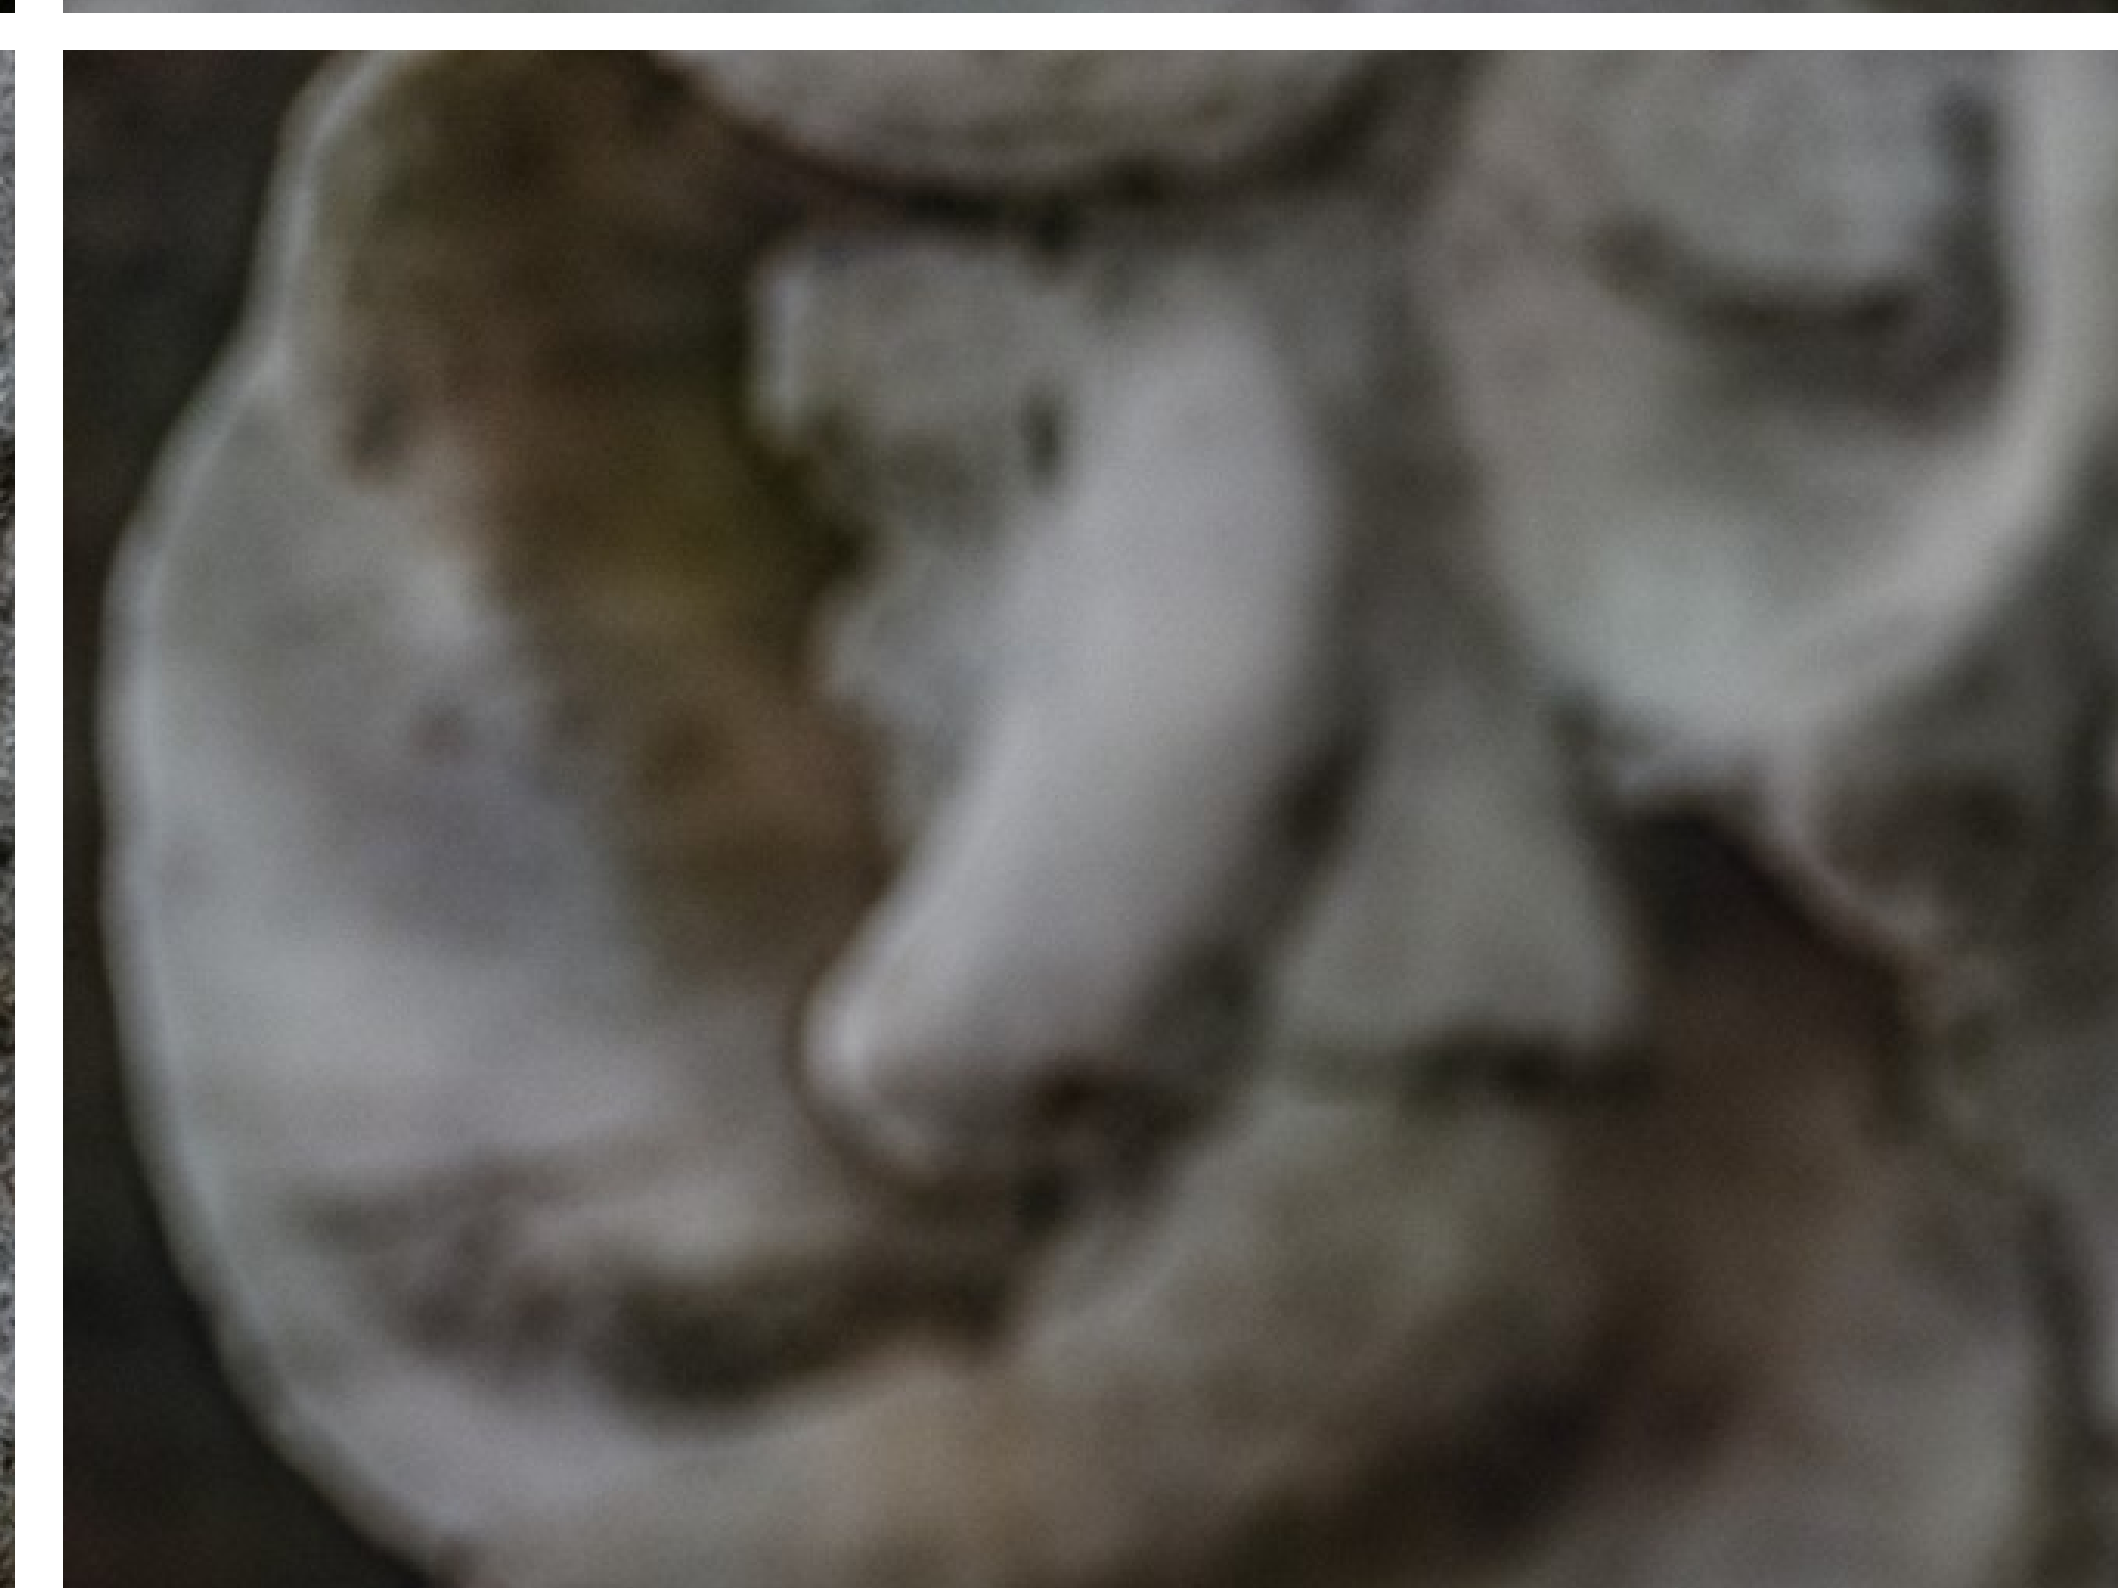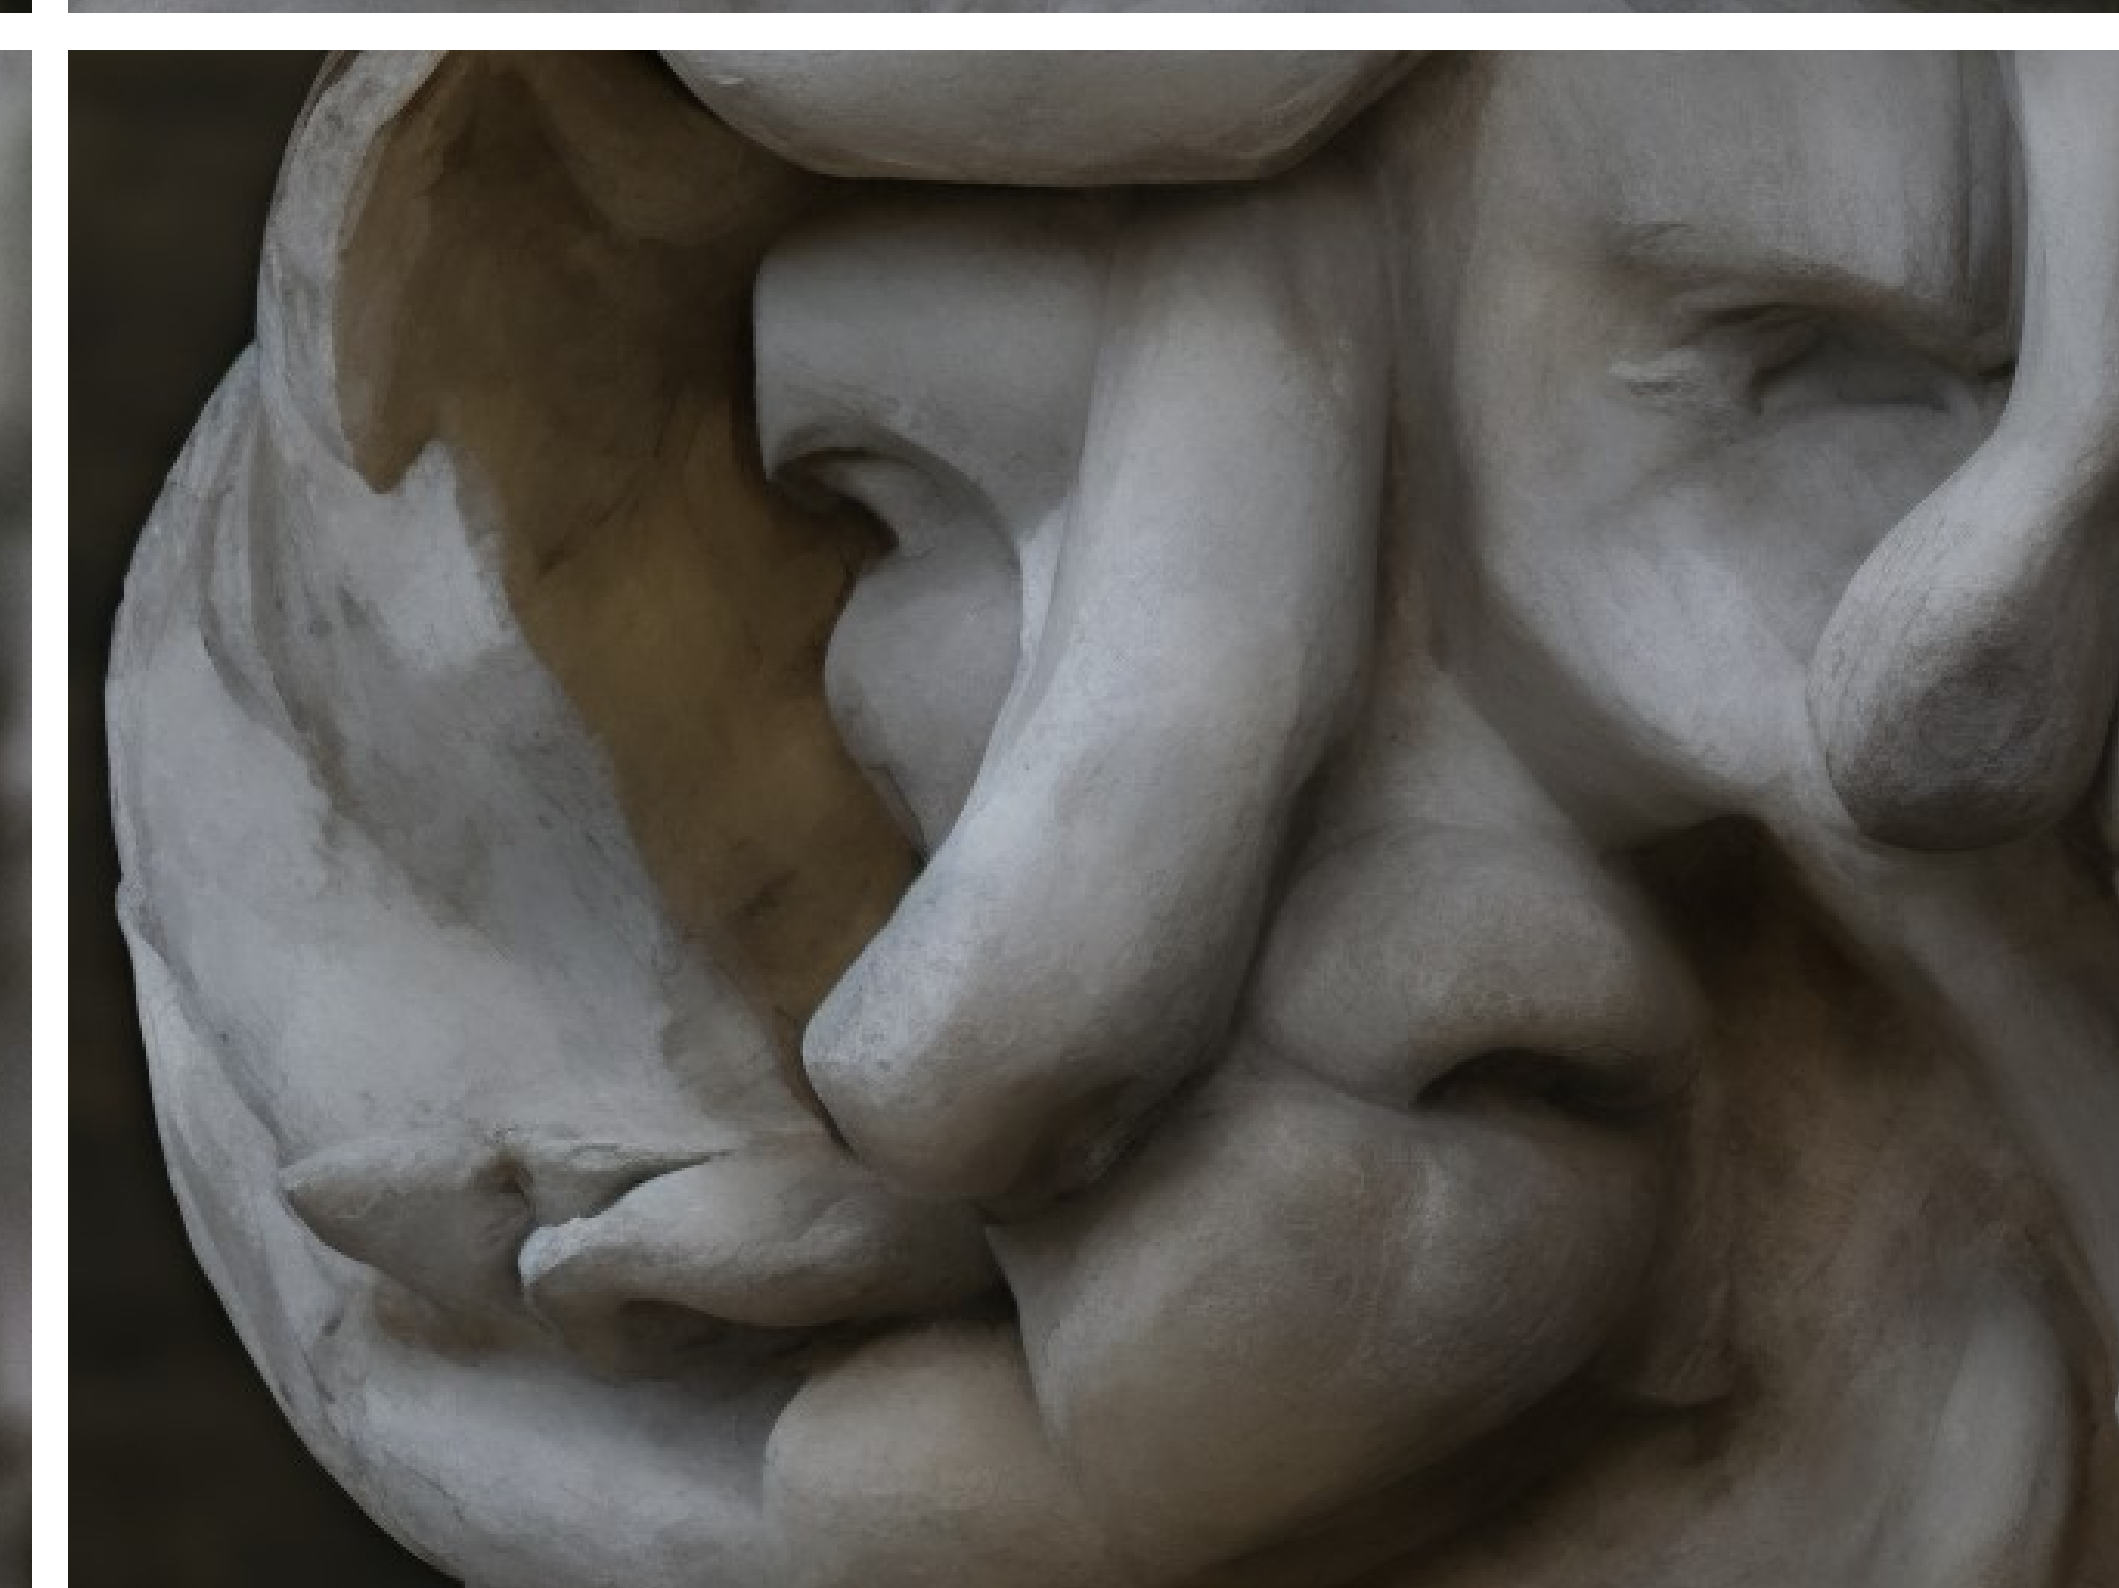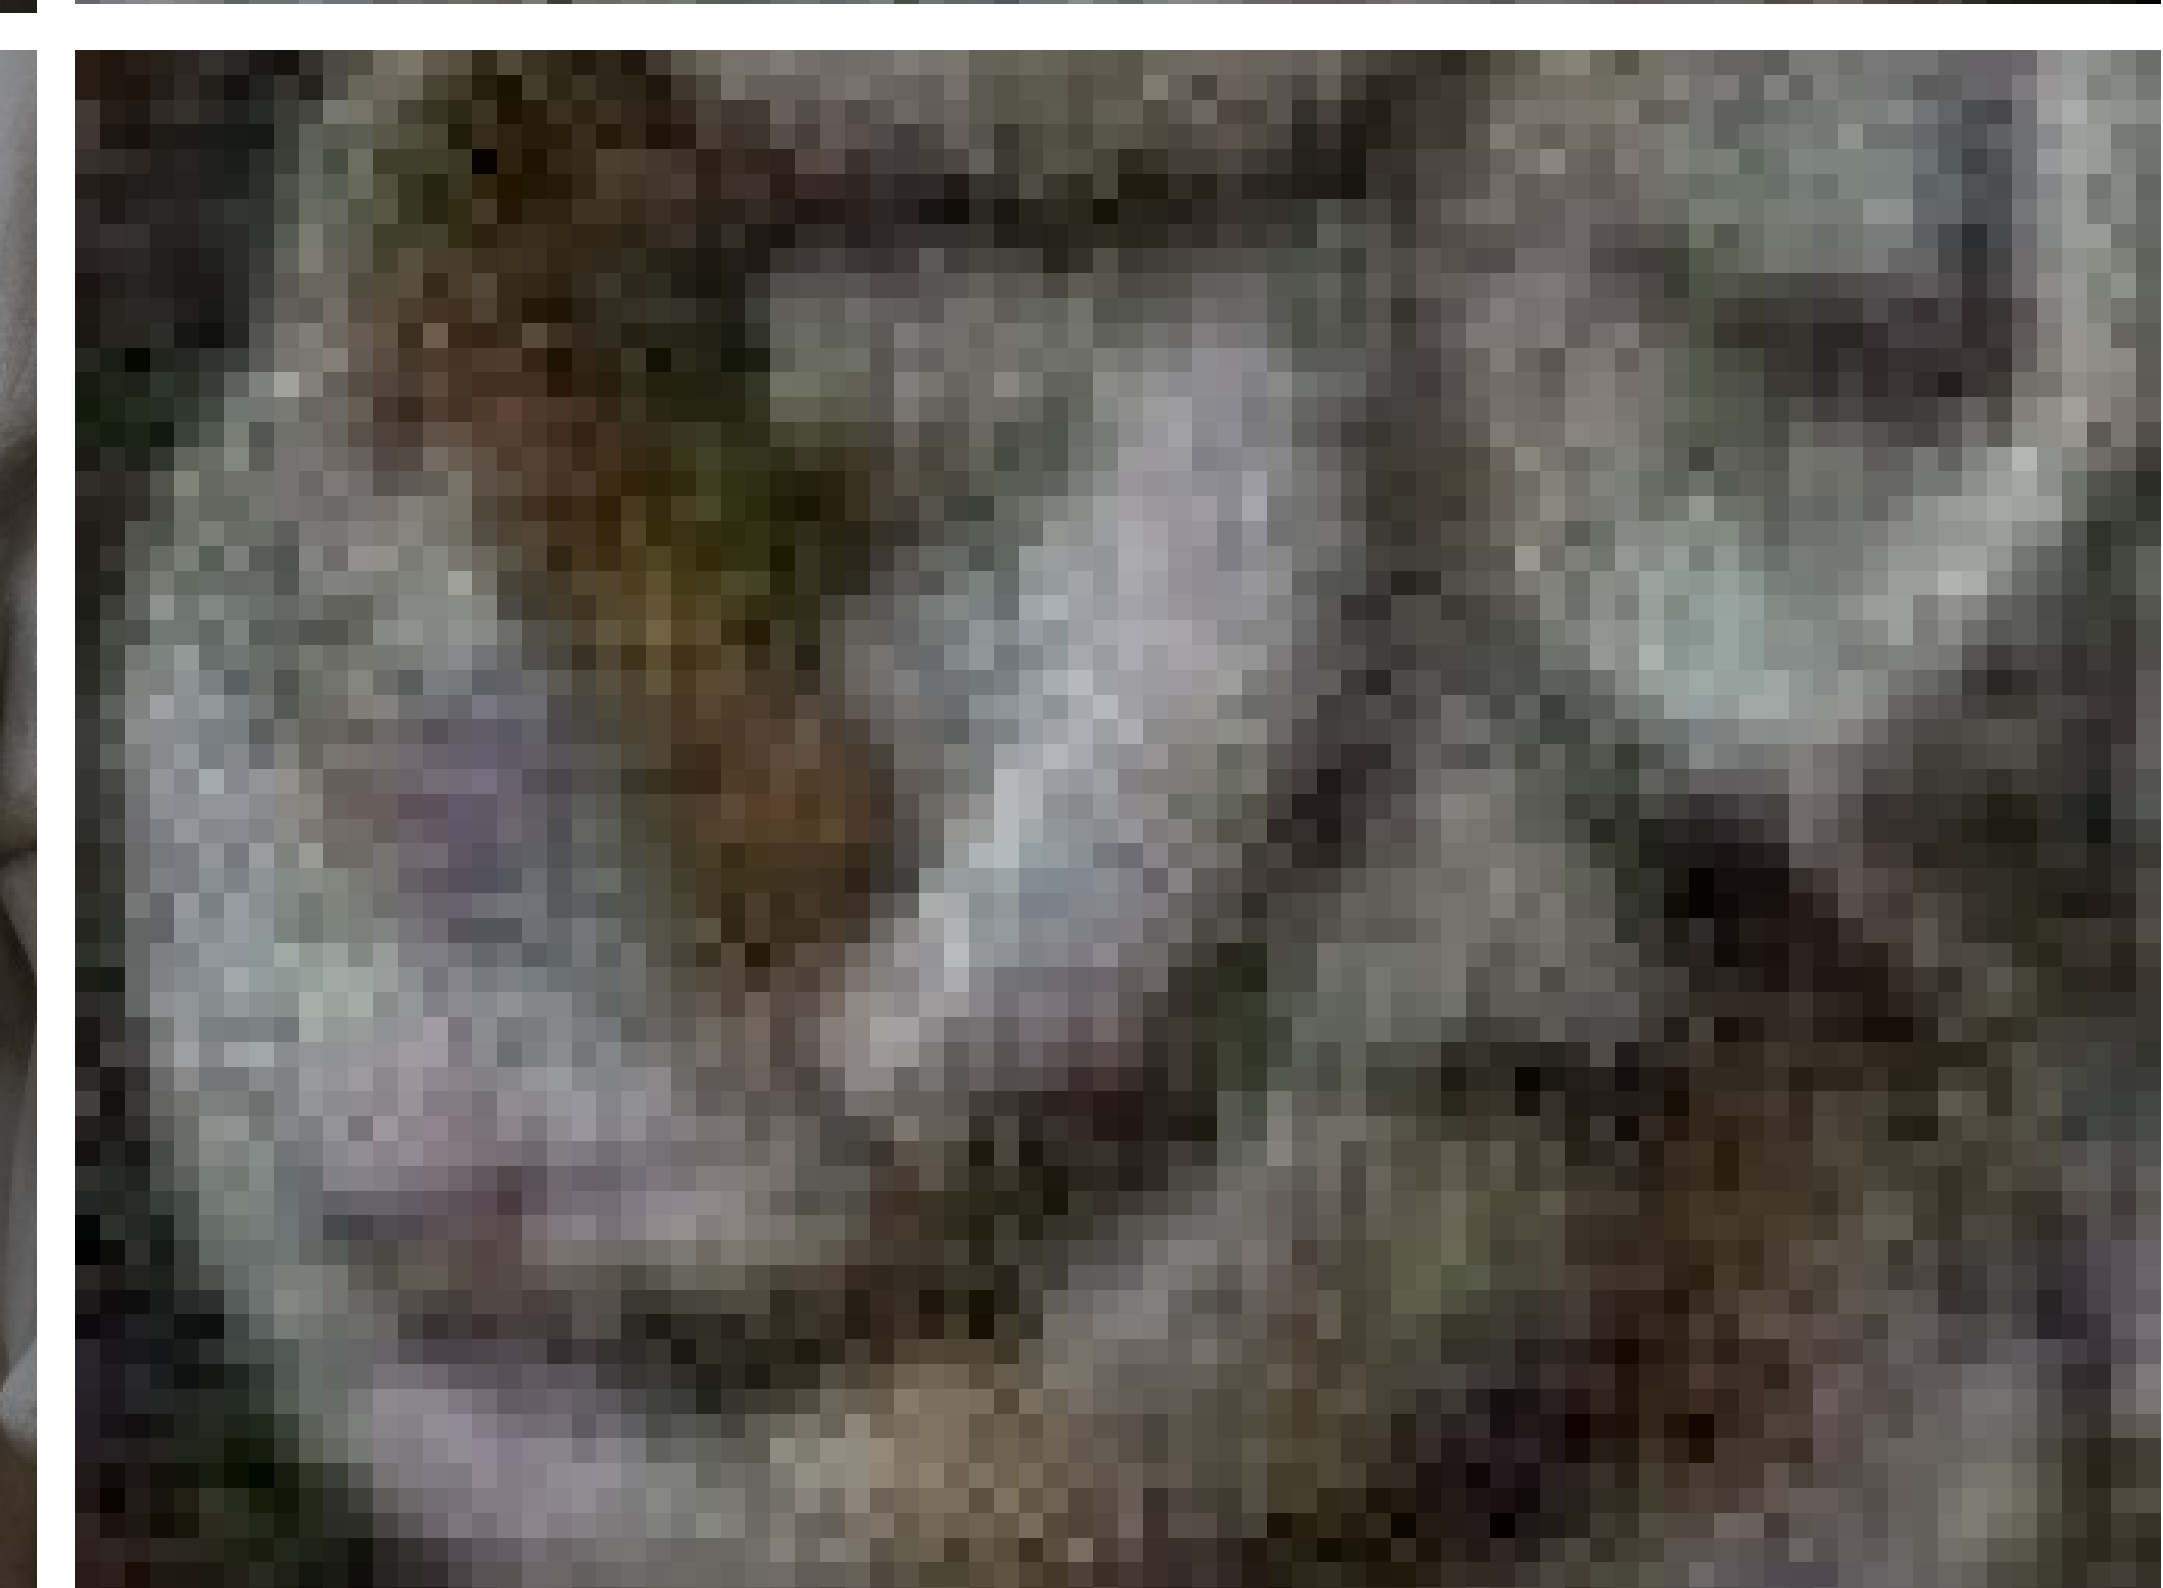

Ours

SUPIR

SeeSR

Input



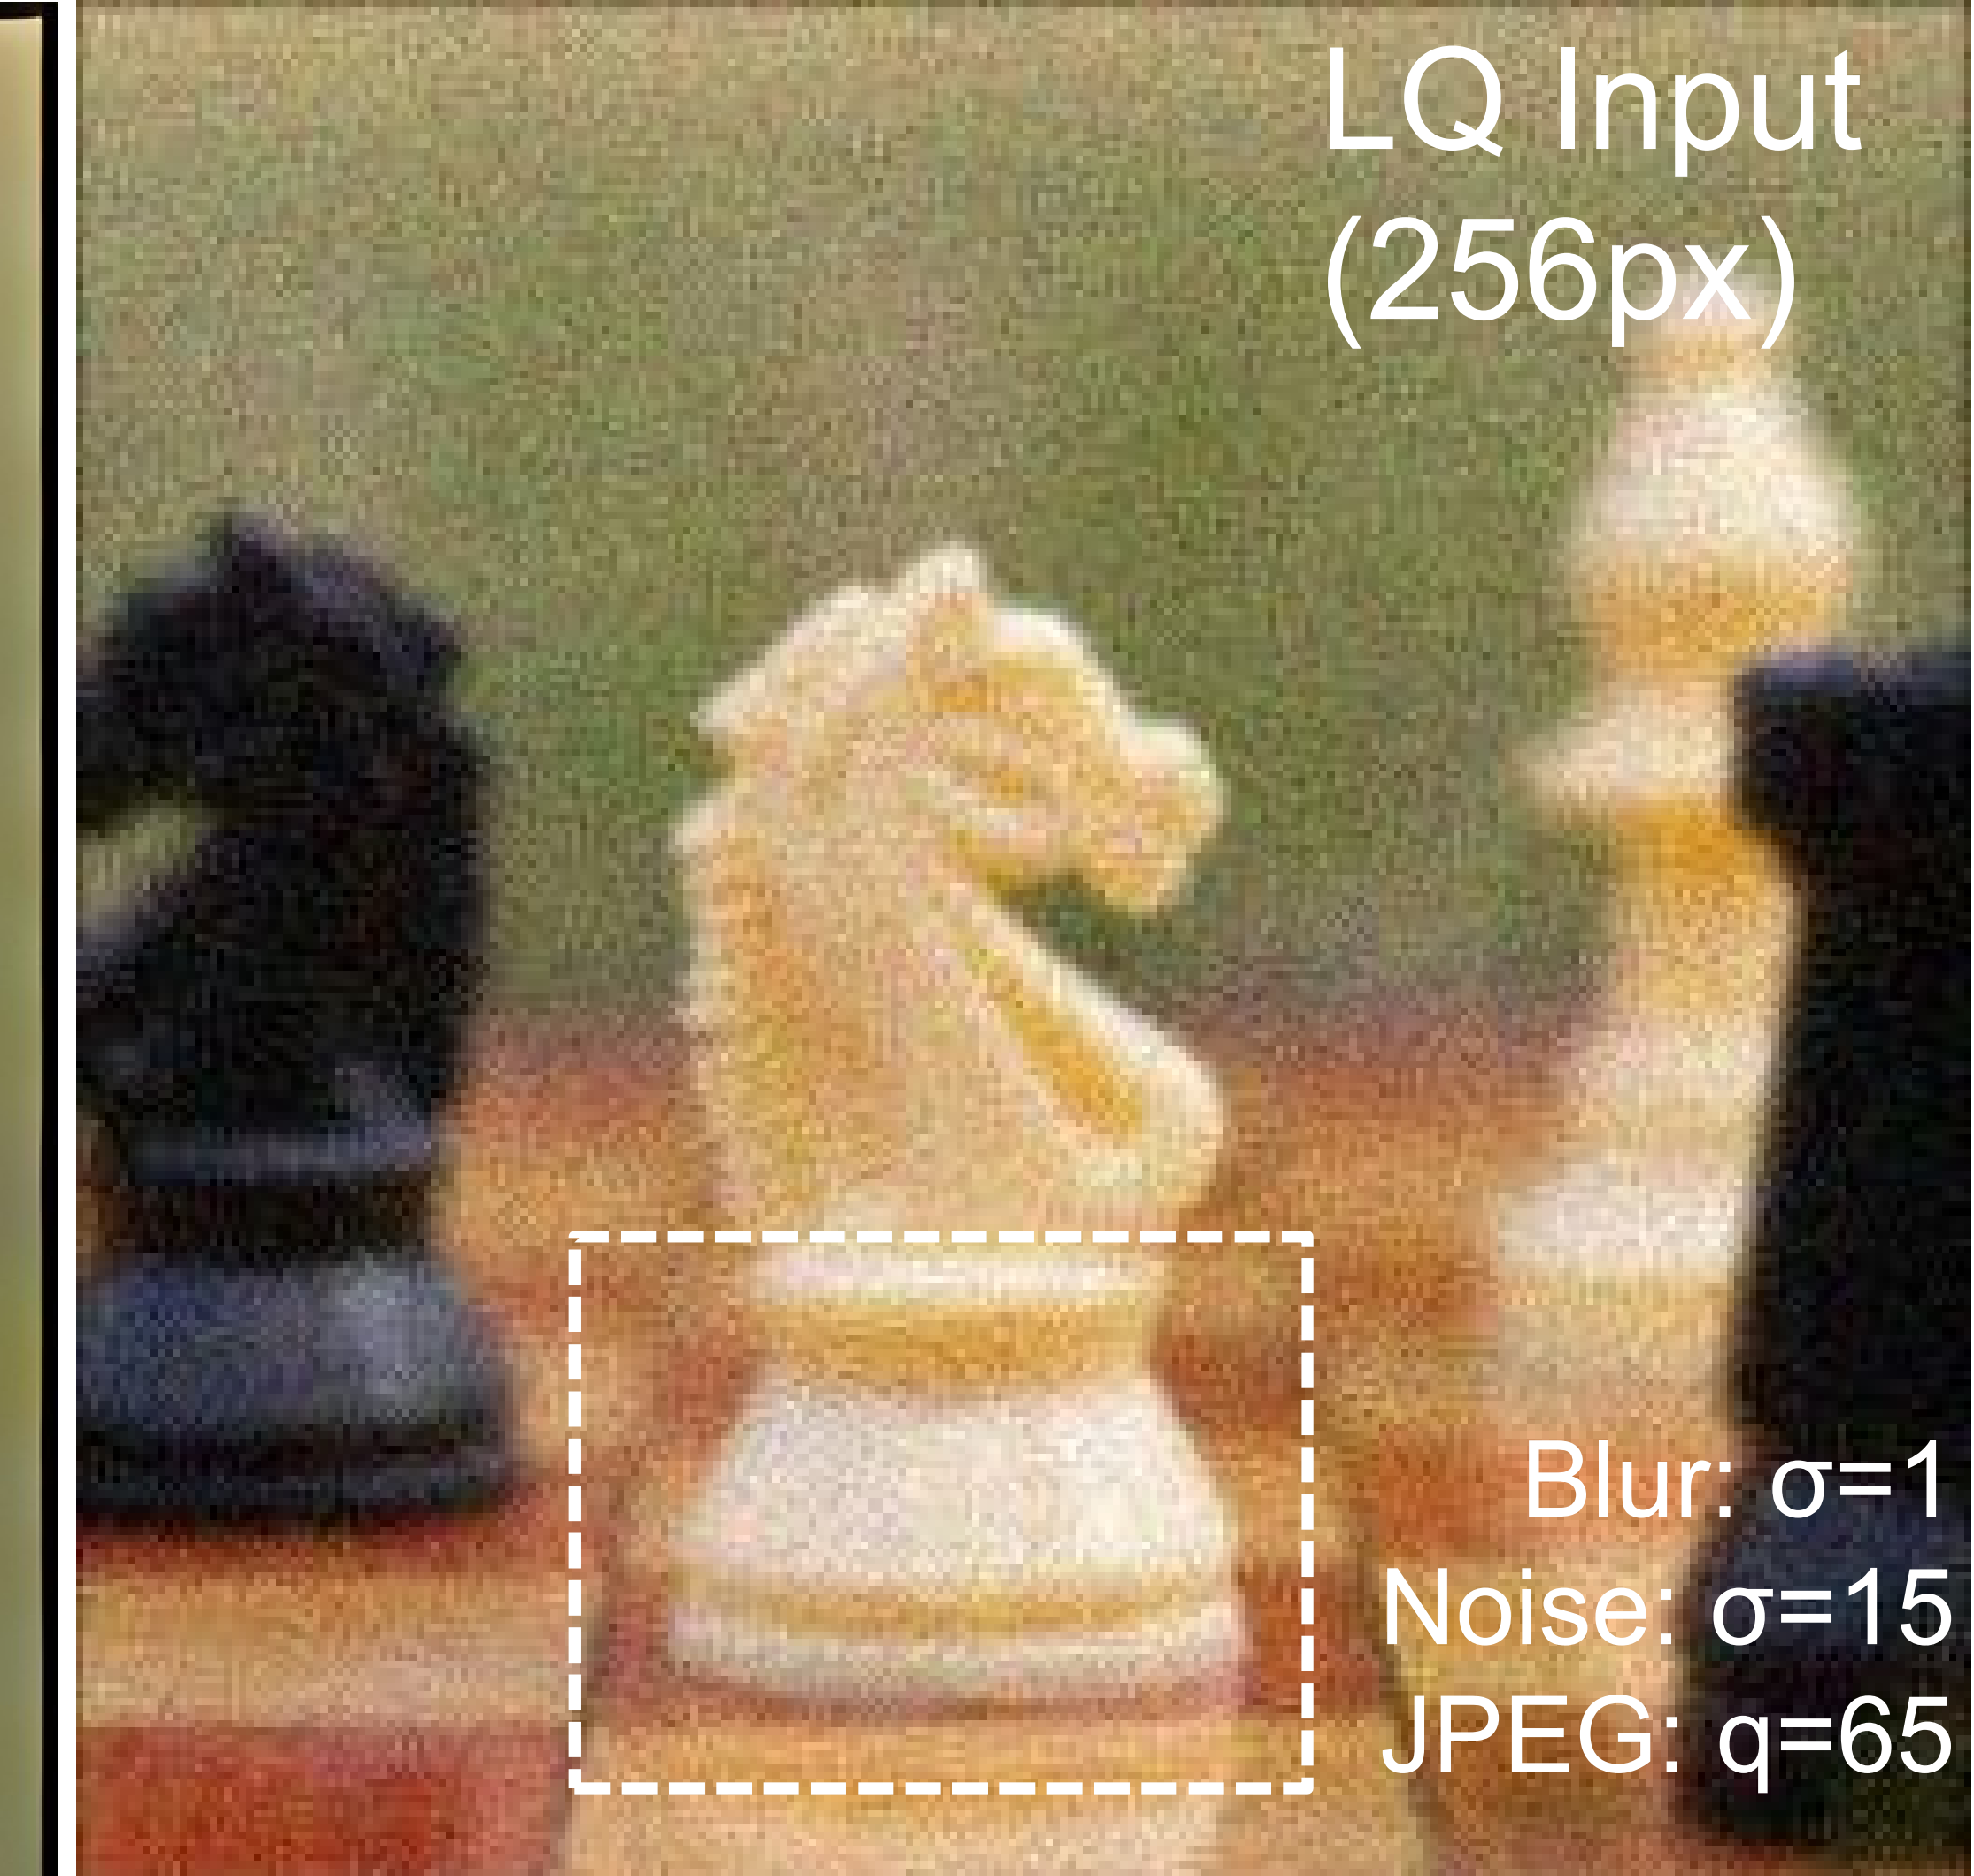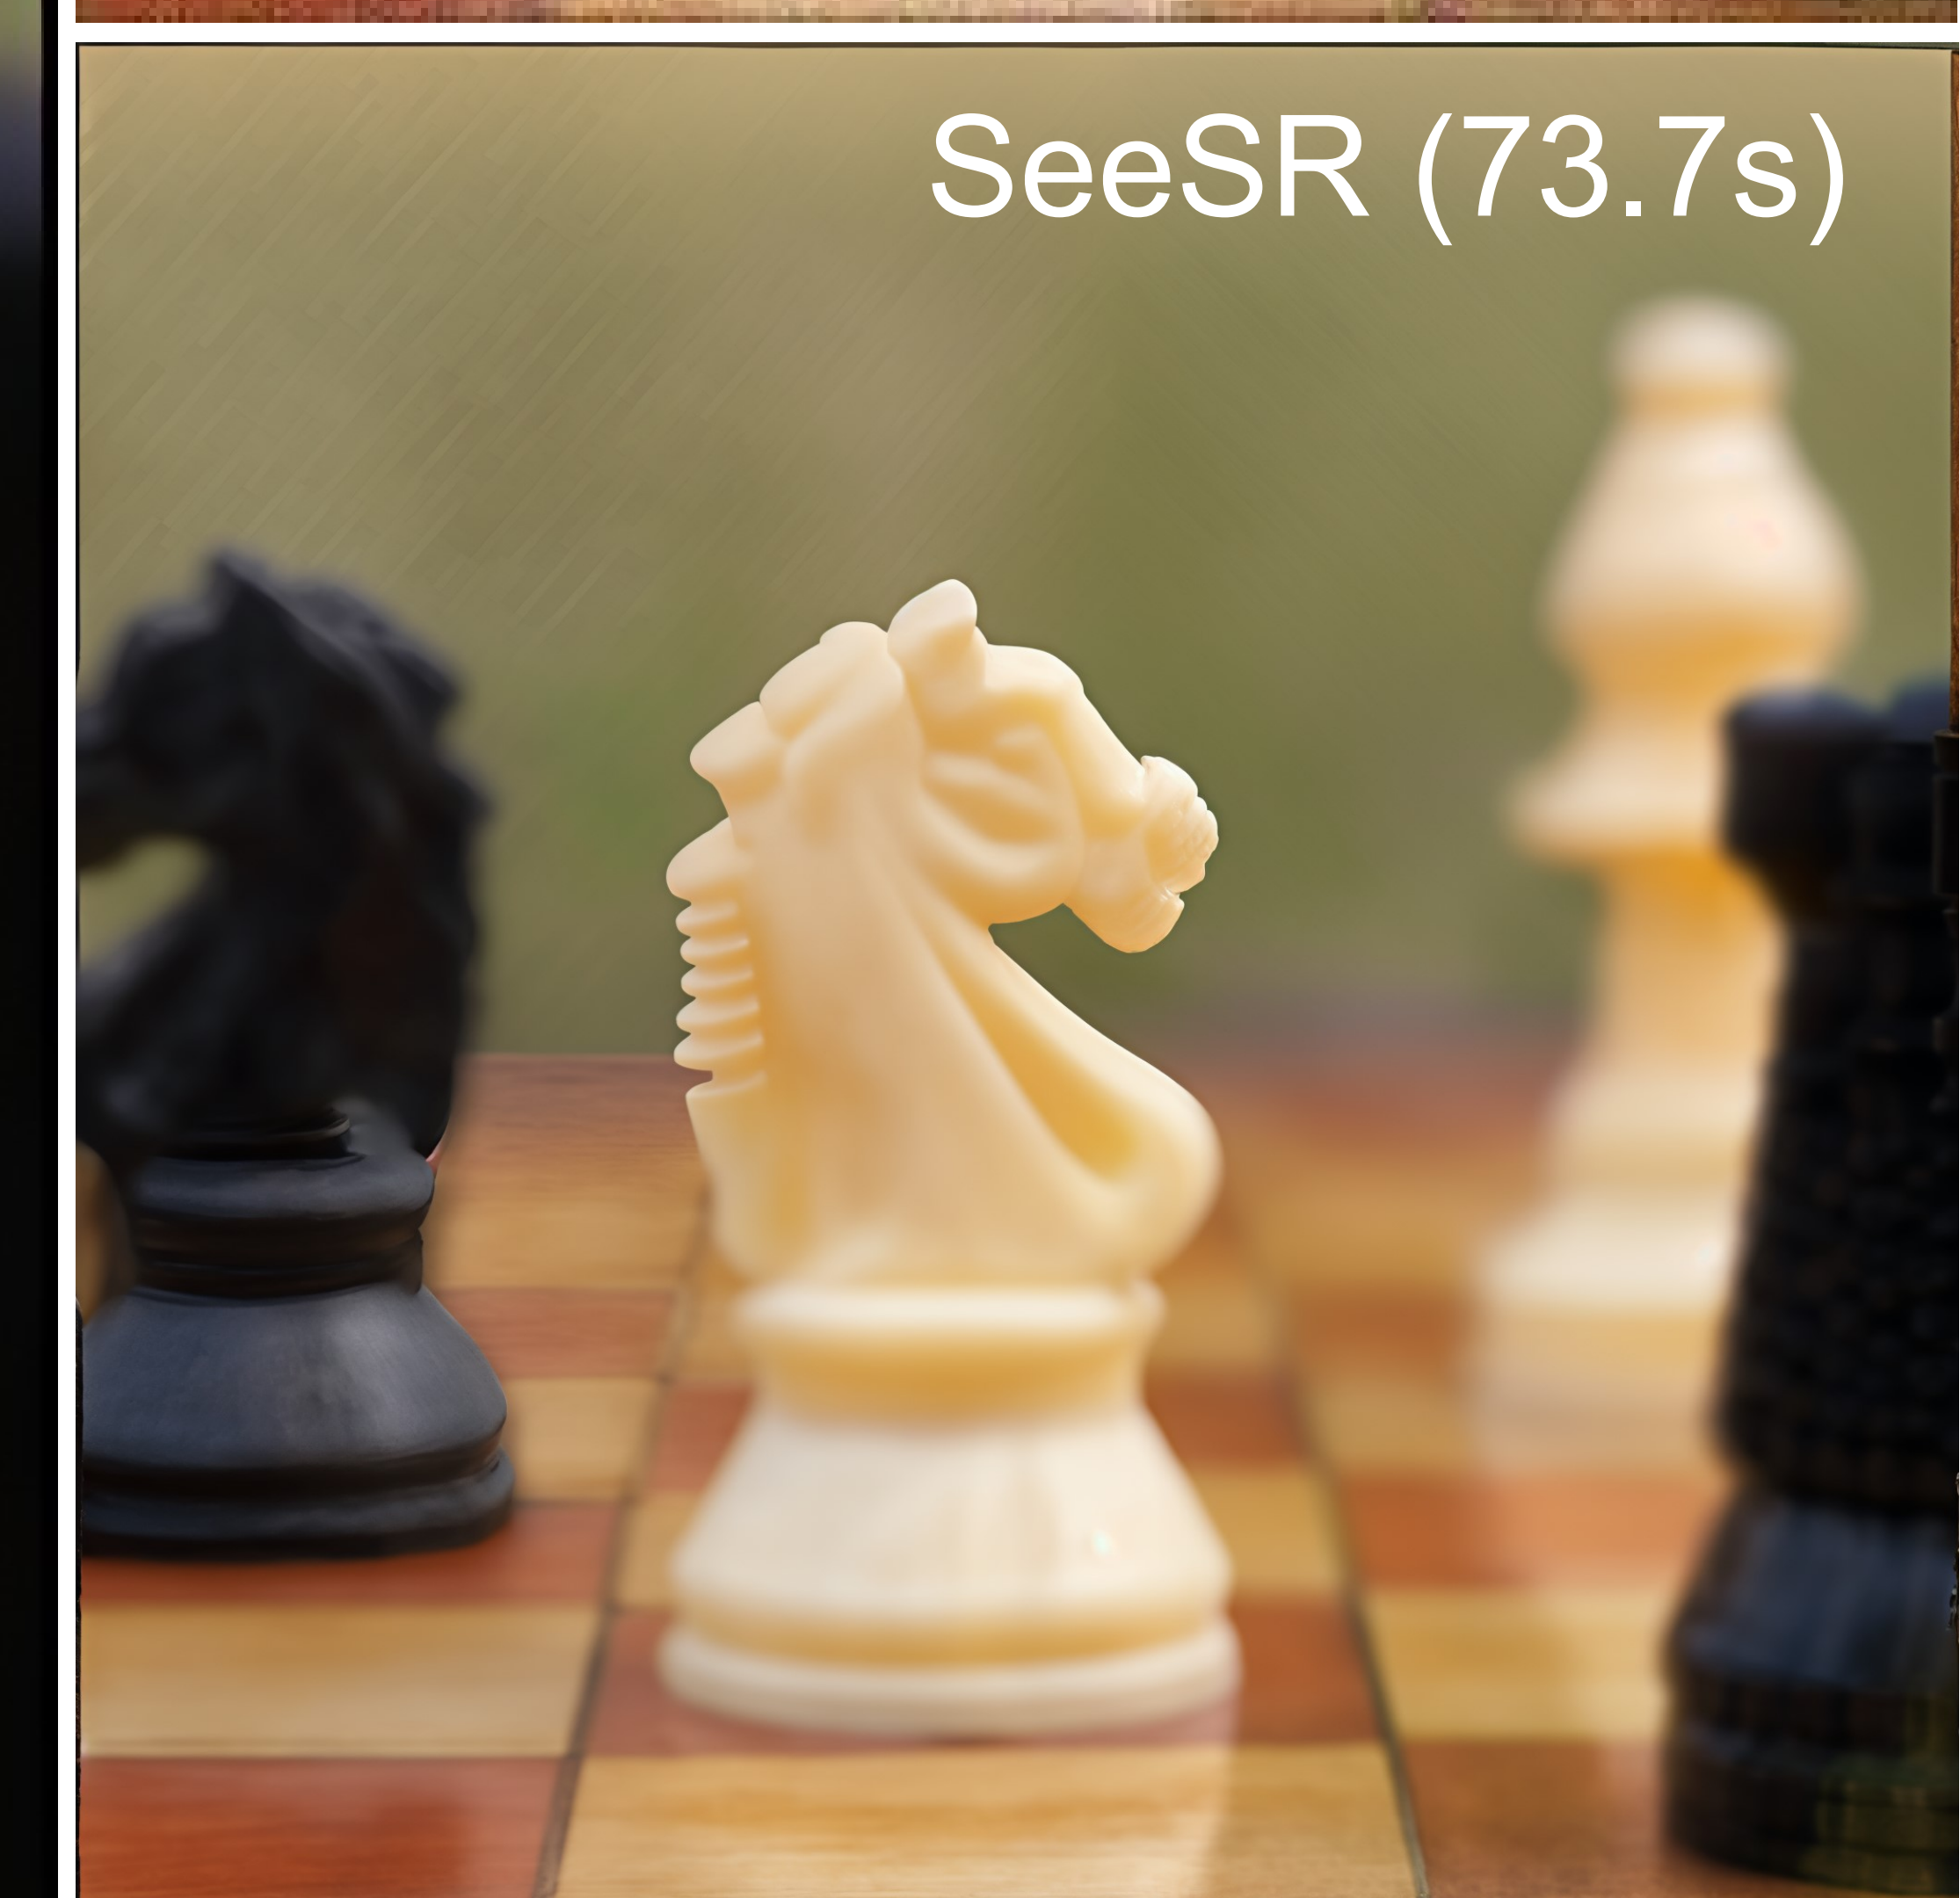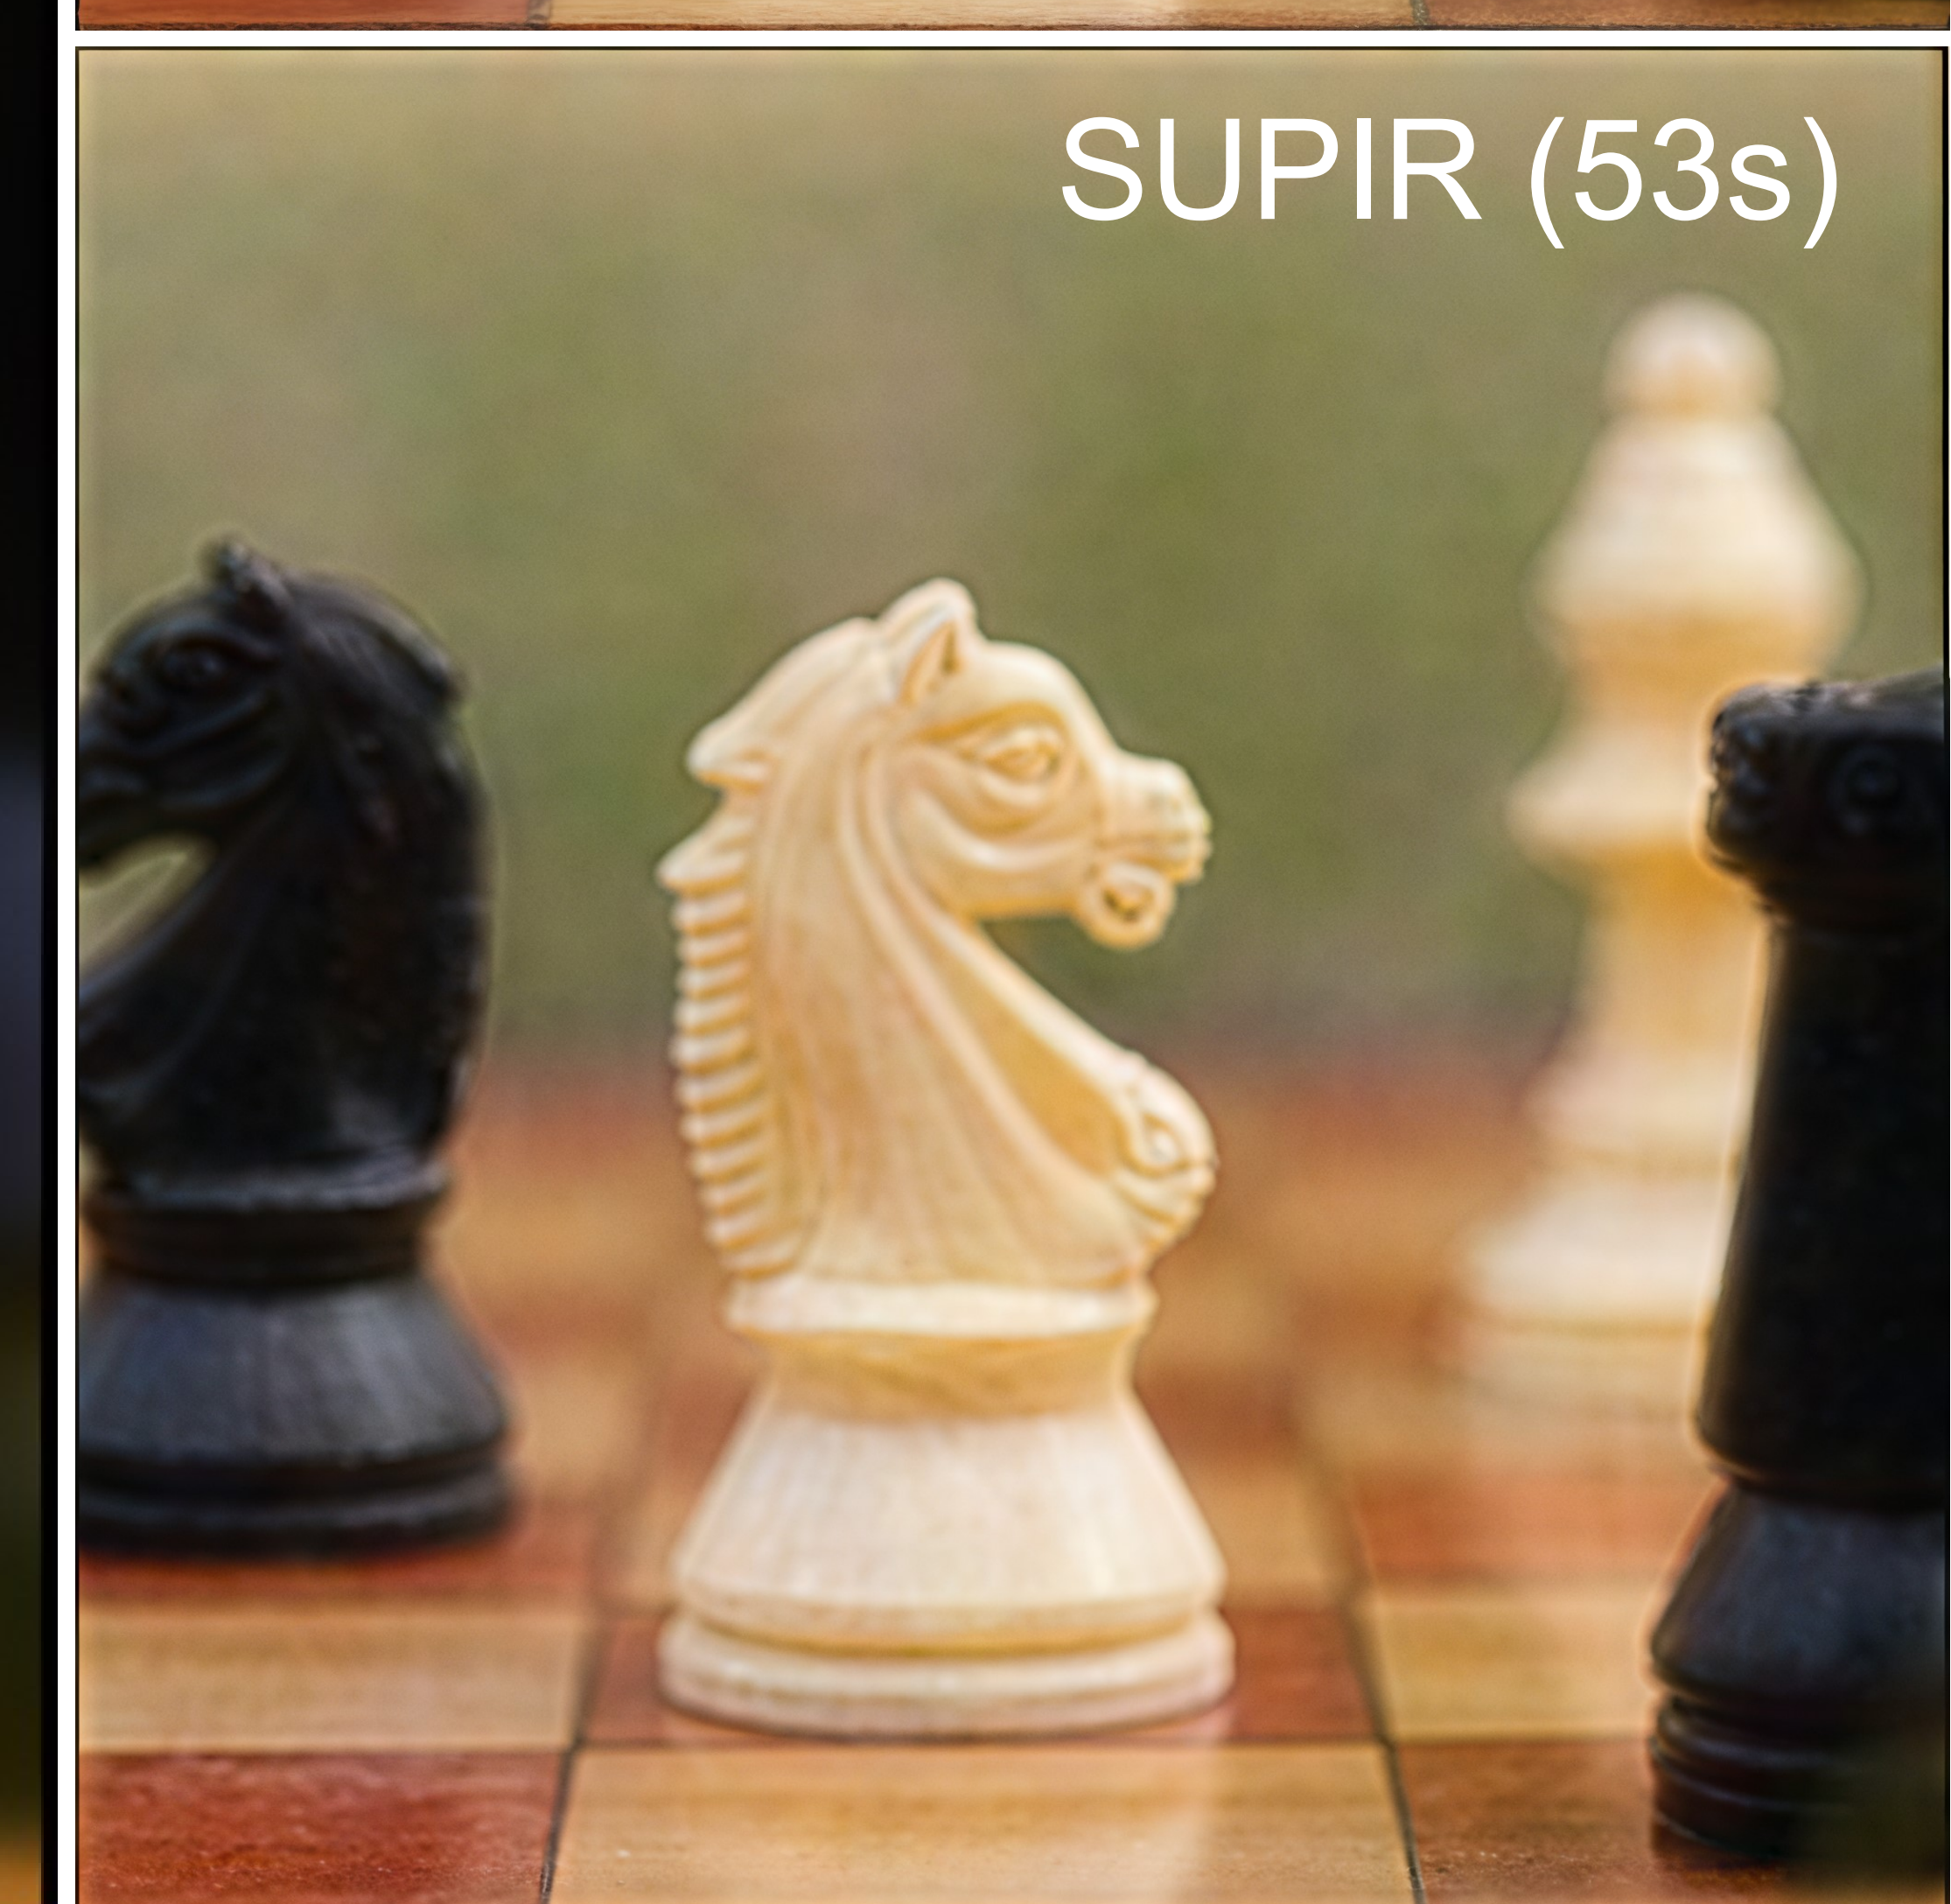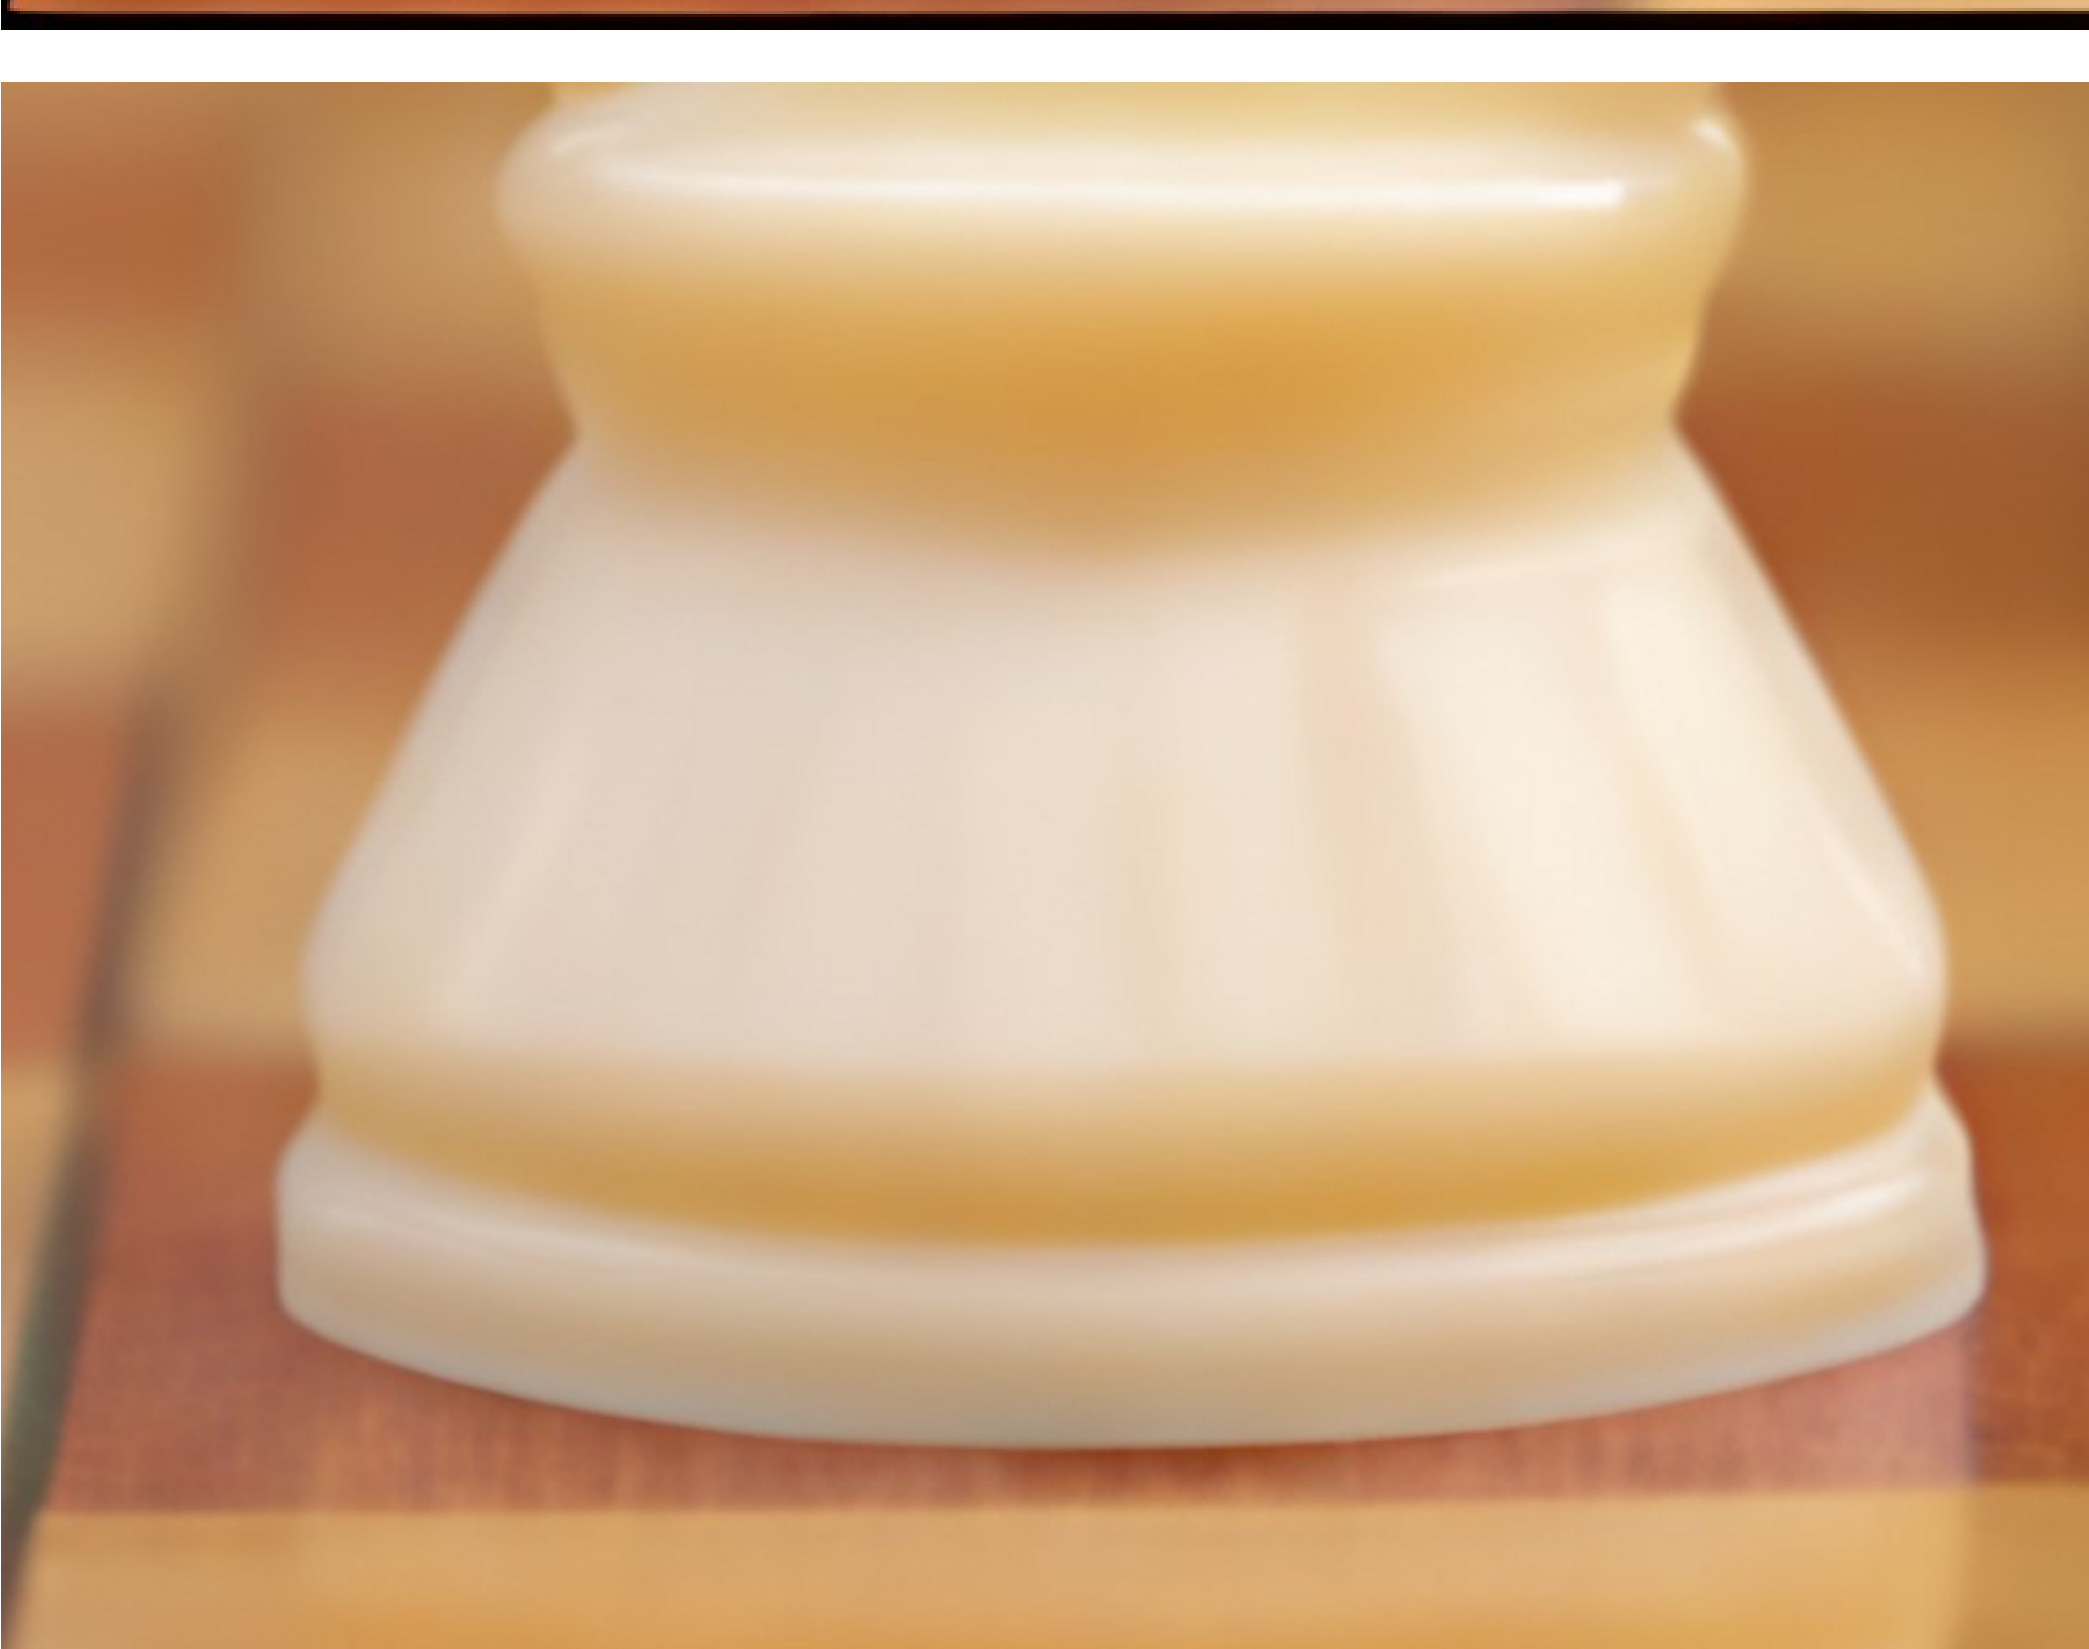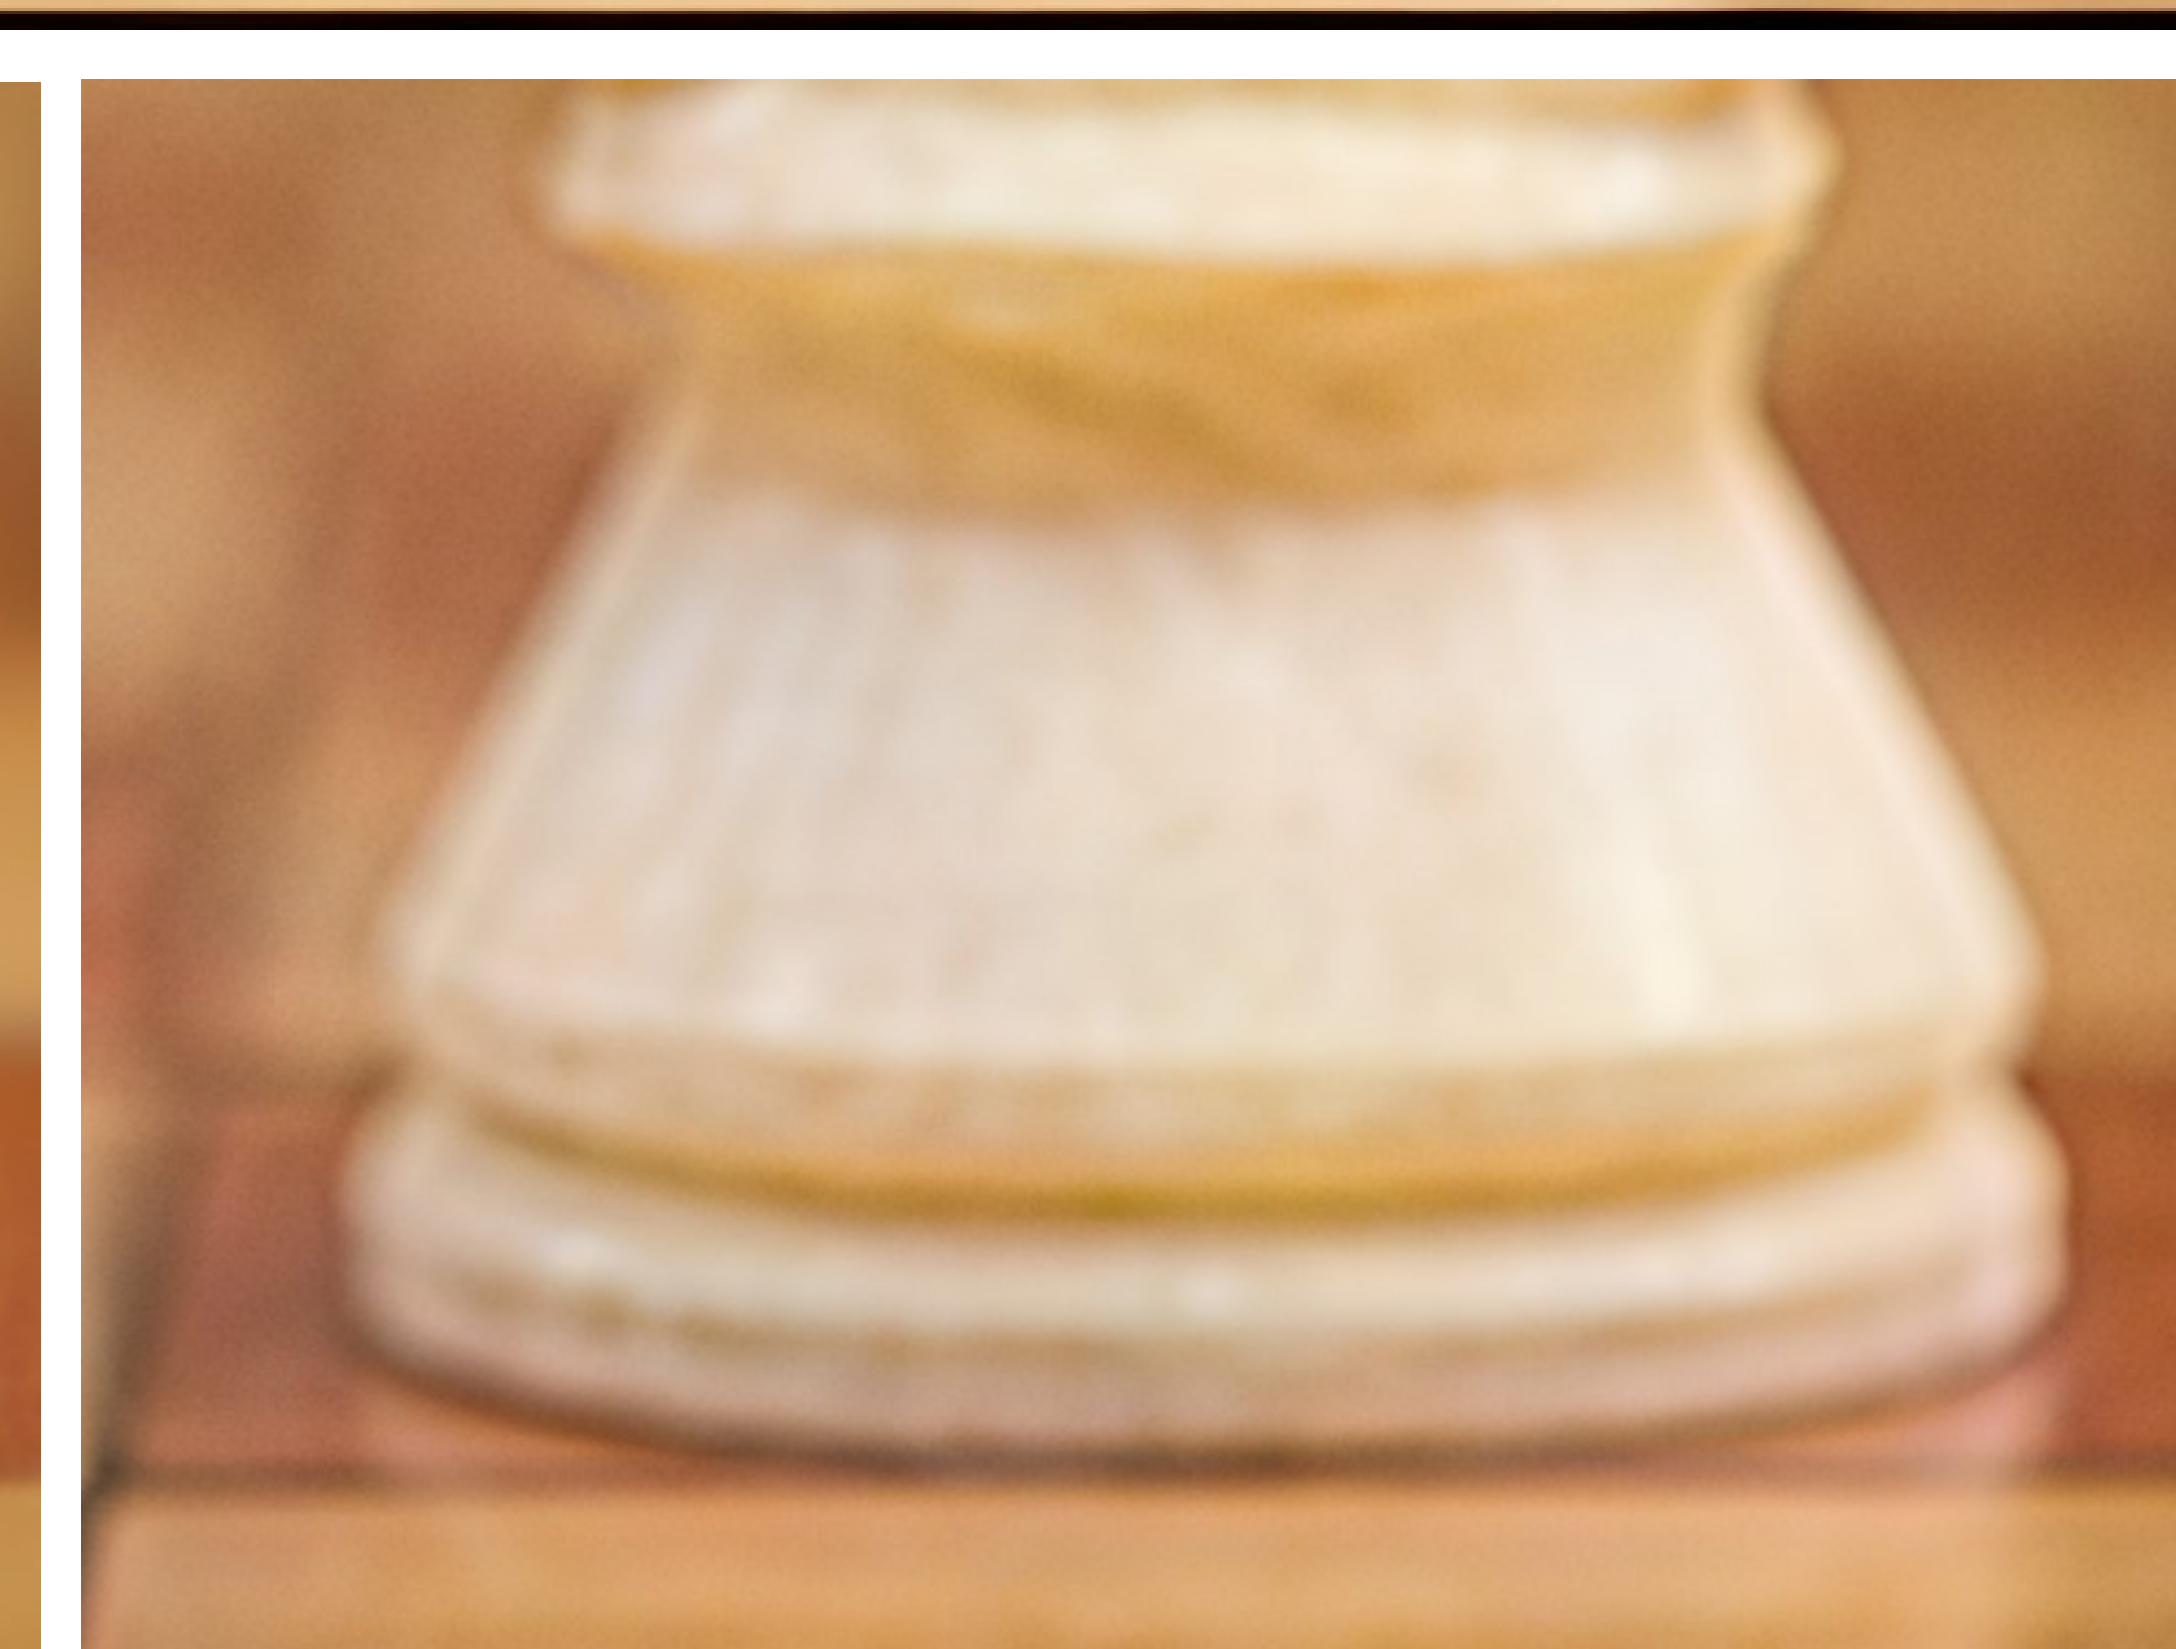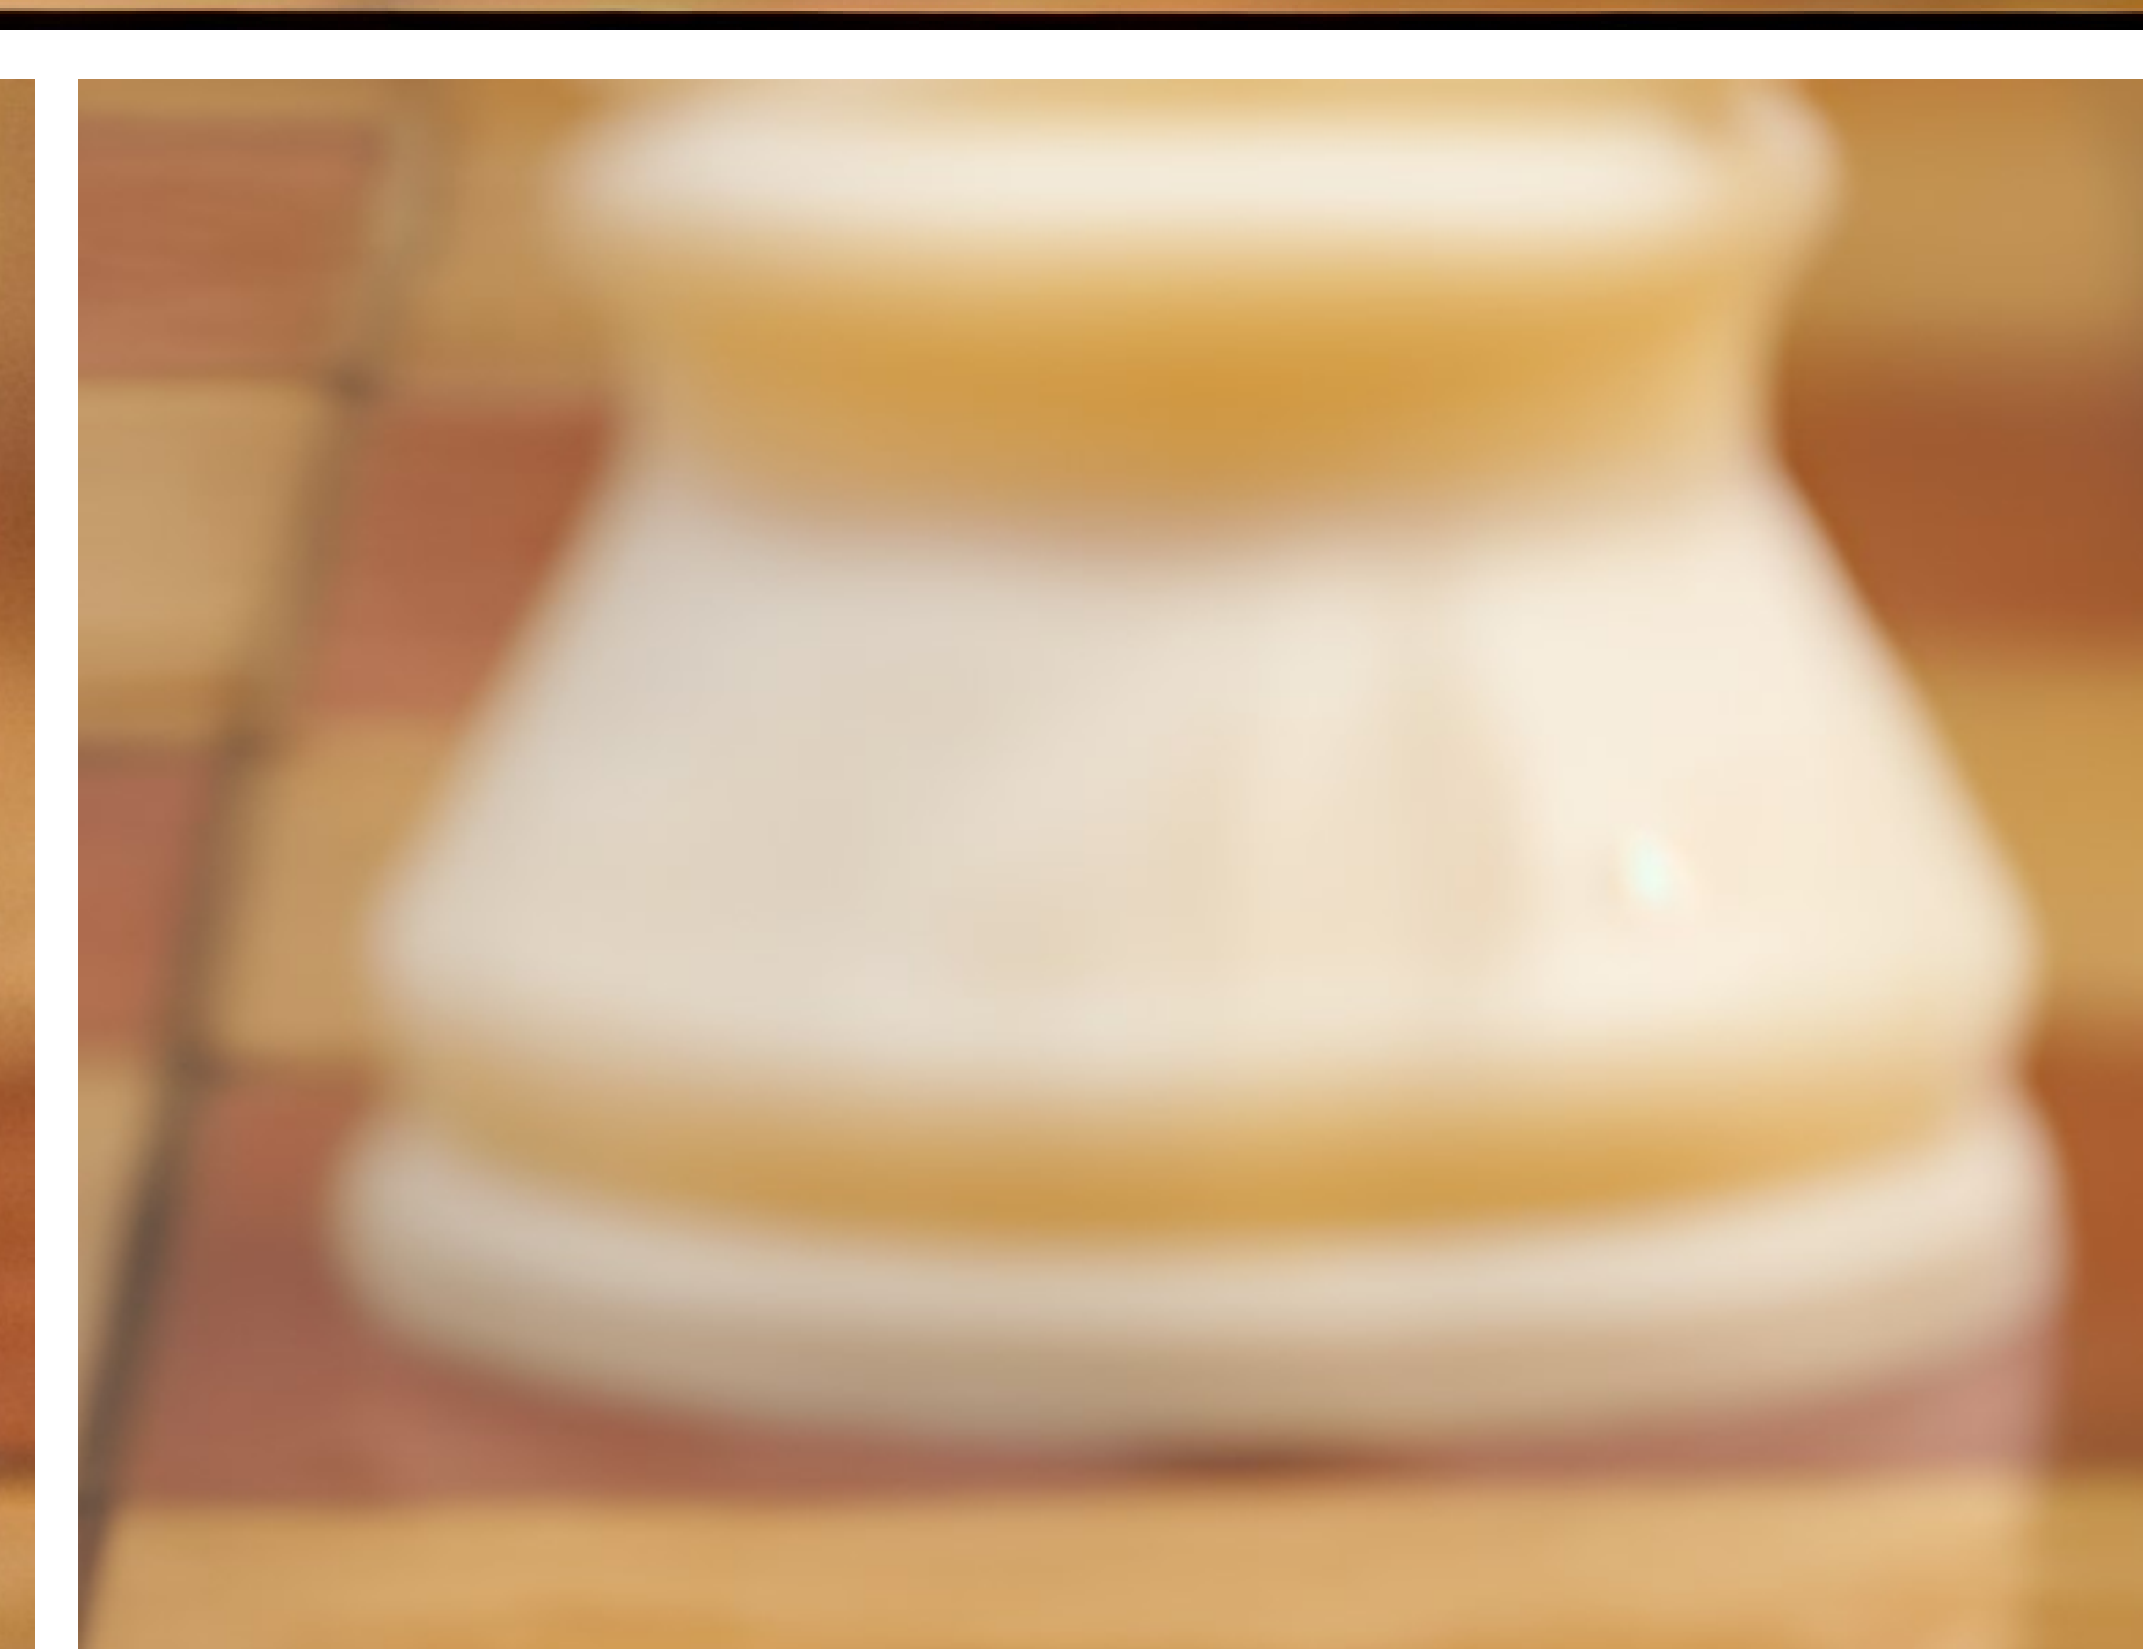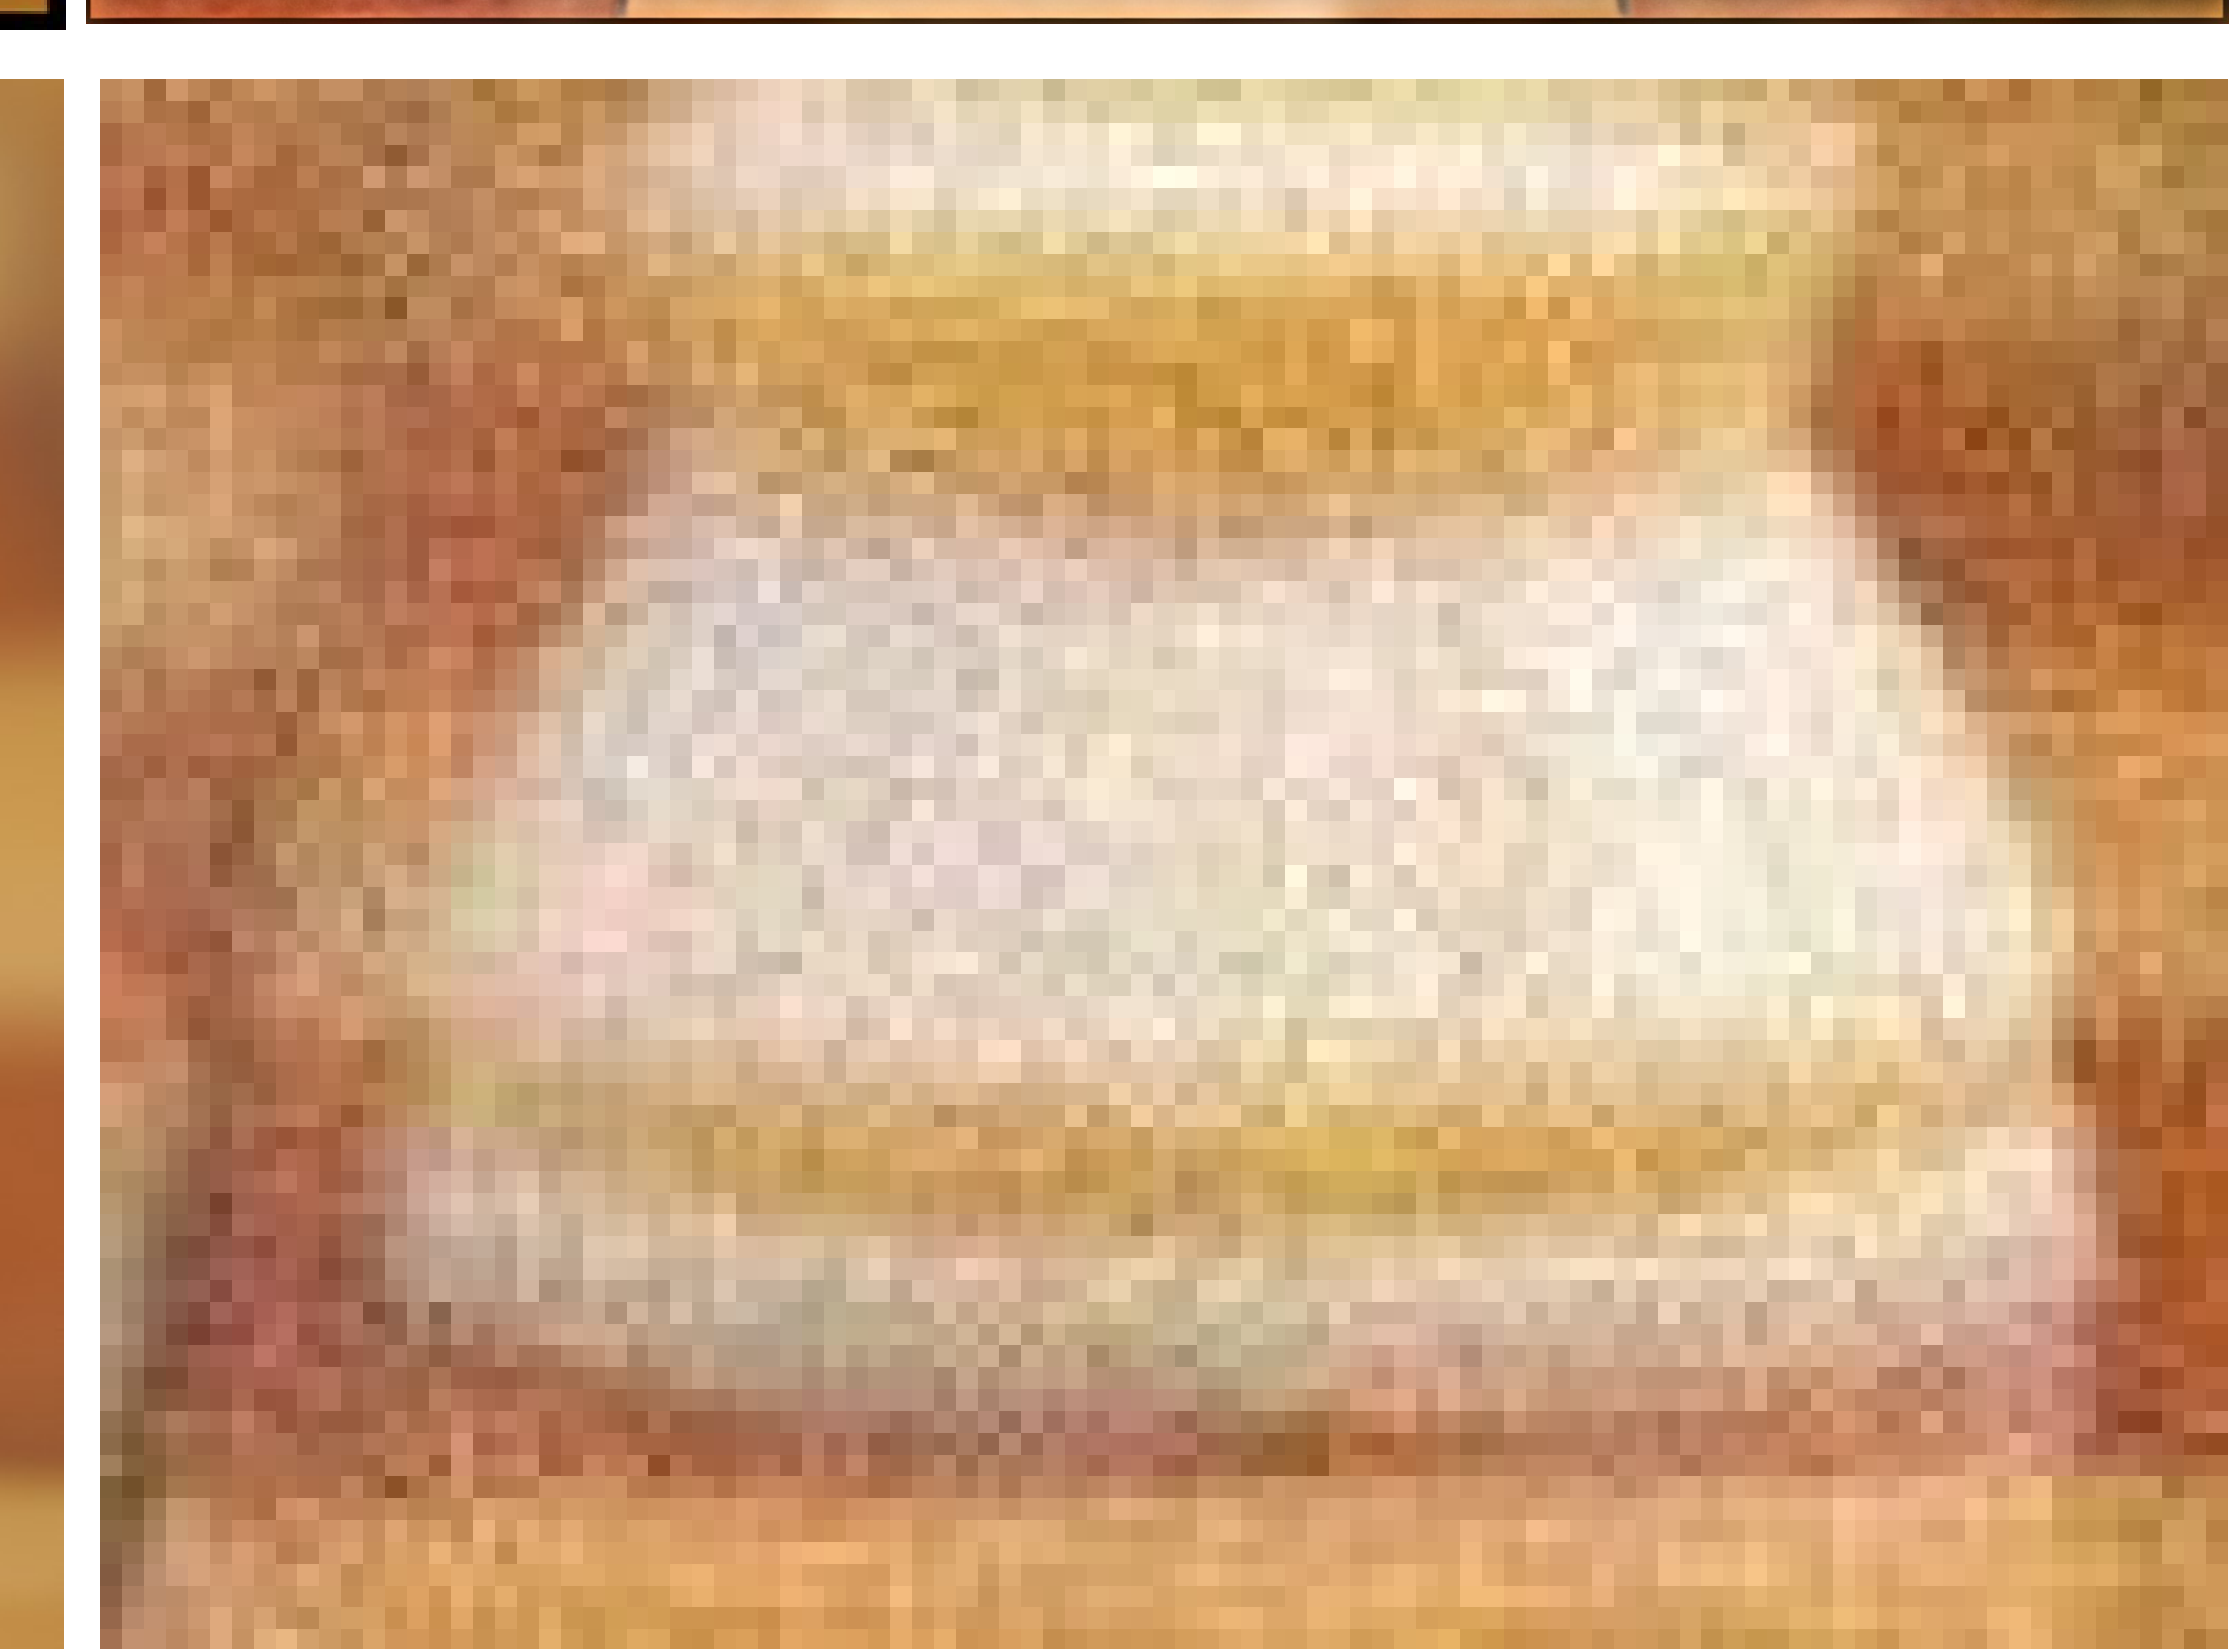





Ours (6.9s)

8× IR, 2048px, 4Mpix

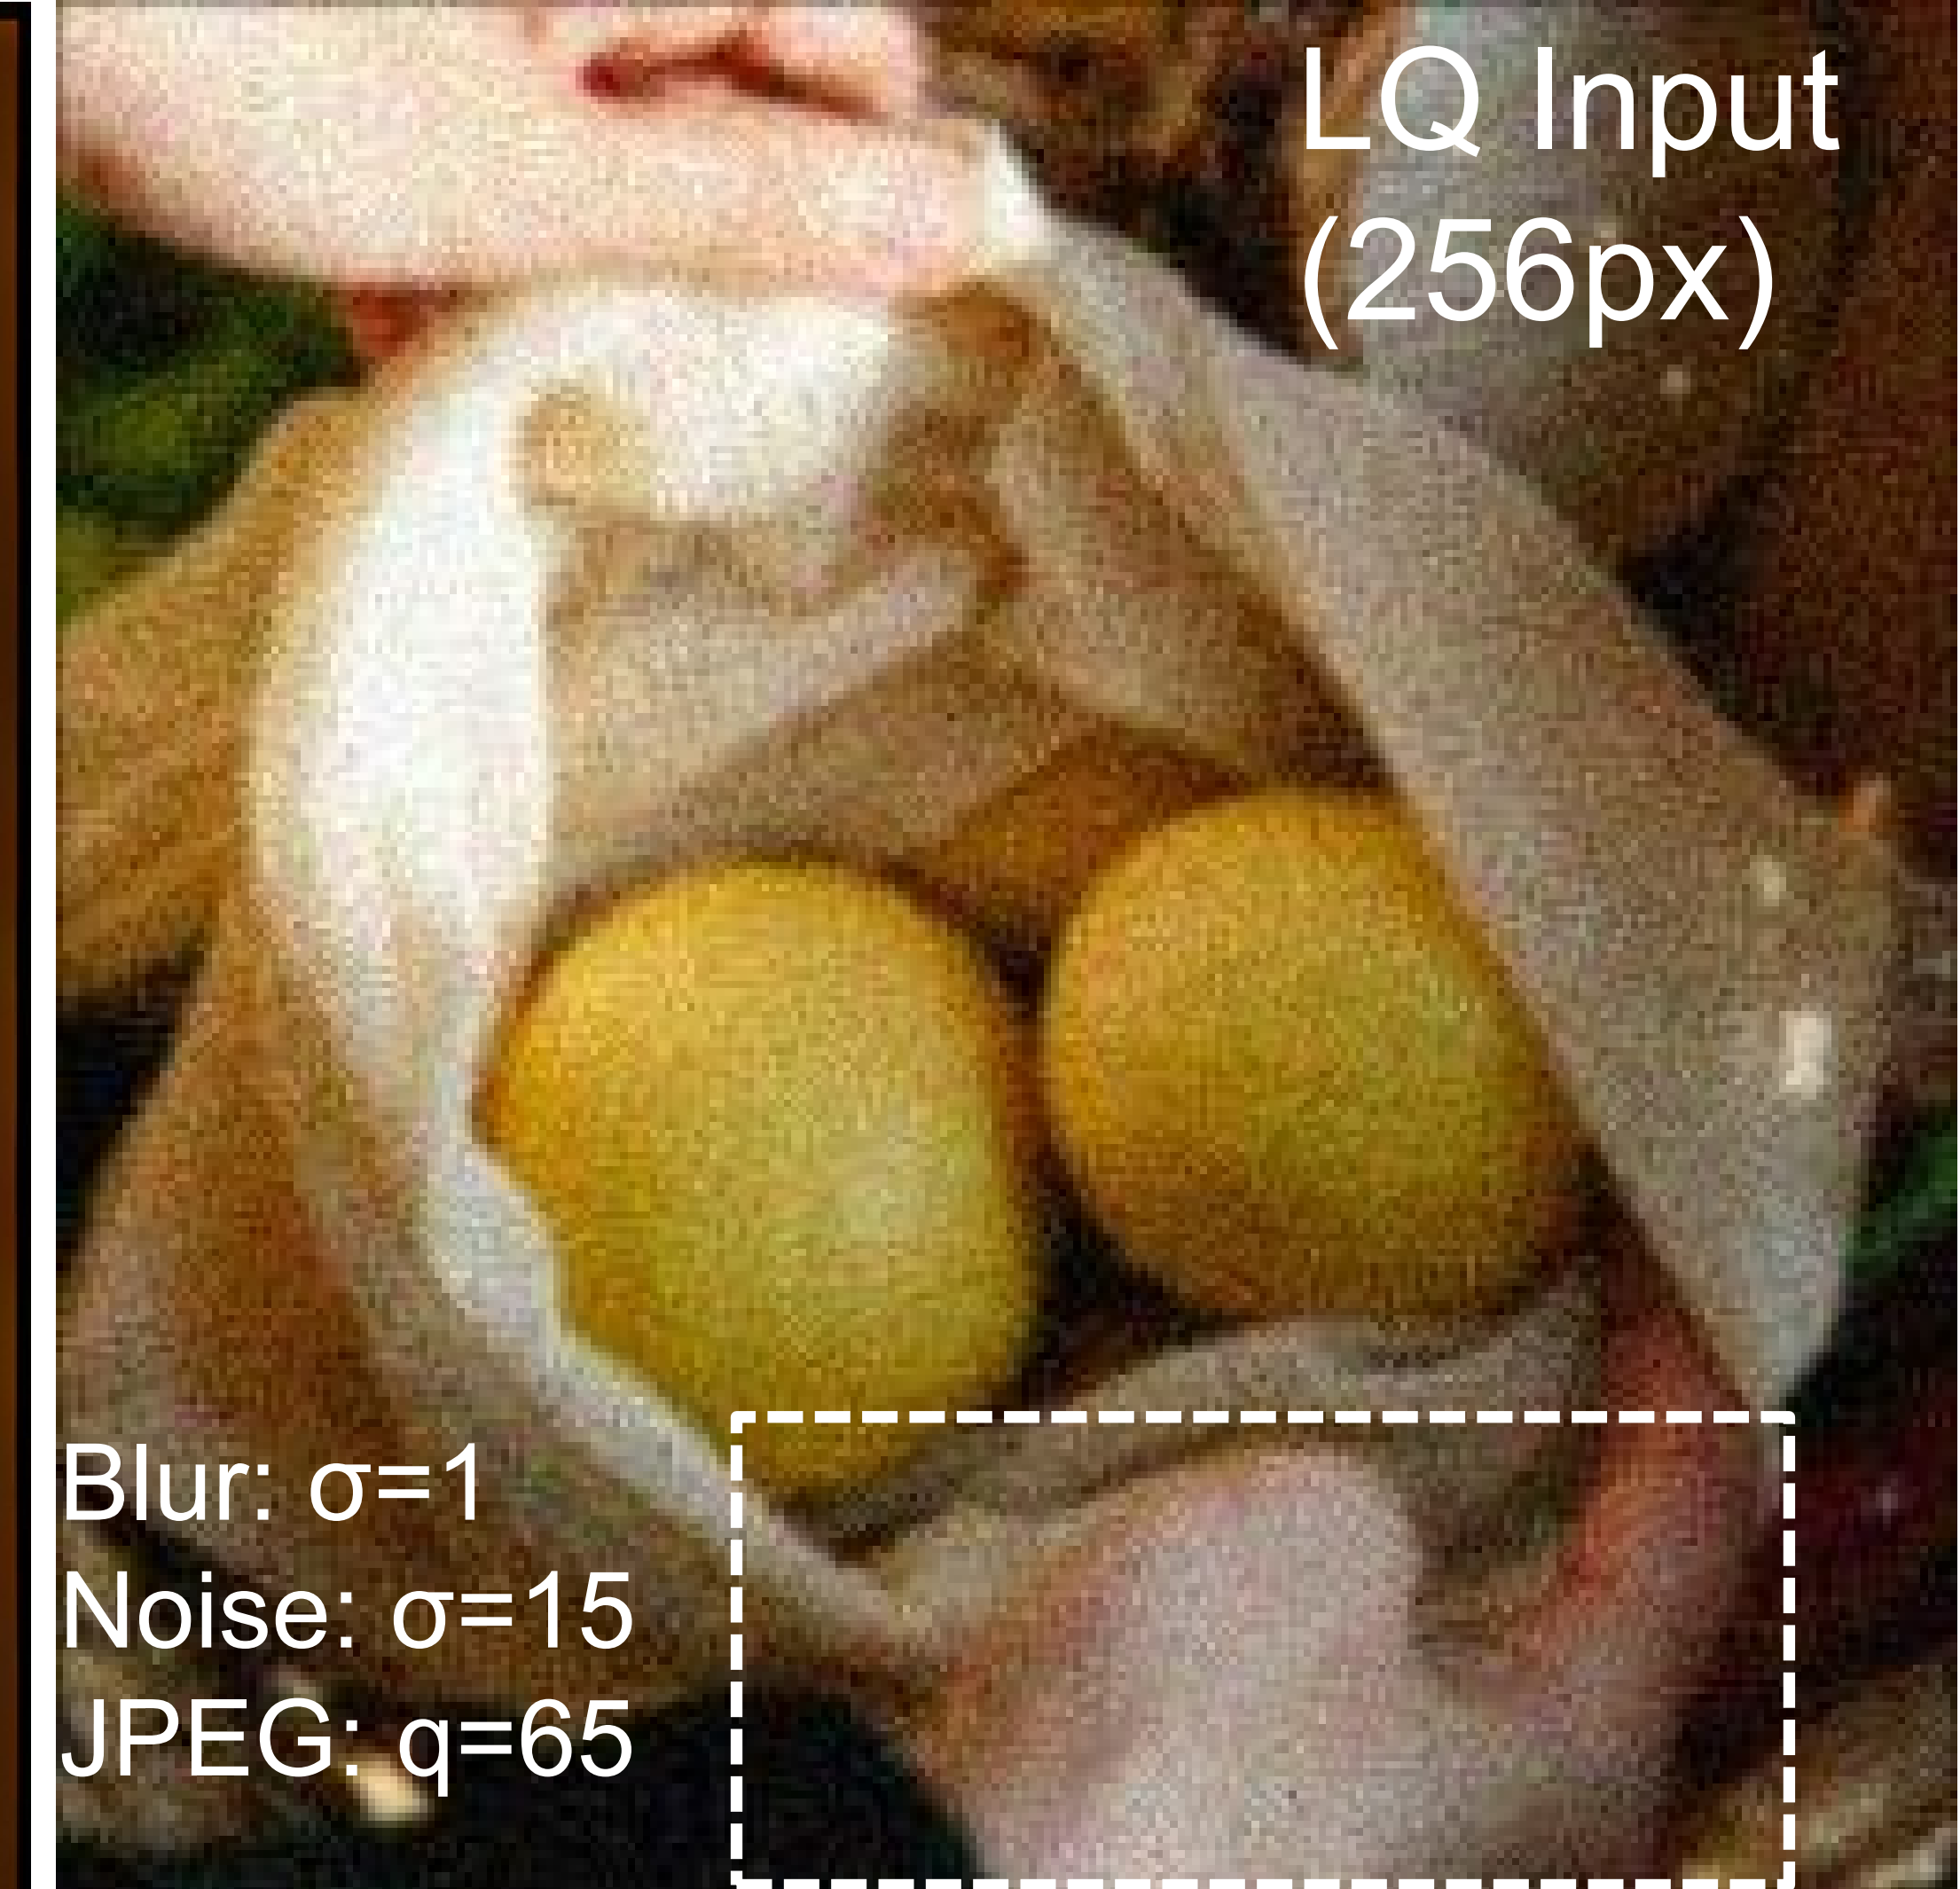

LQ Input  
(256px)

Blur:  $\sigma=1$   
Noise:  $\sigma=15$   
JPEG:  $q=65$

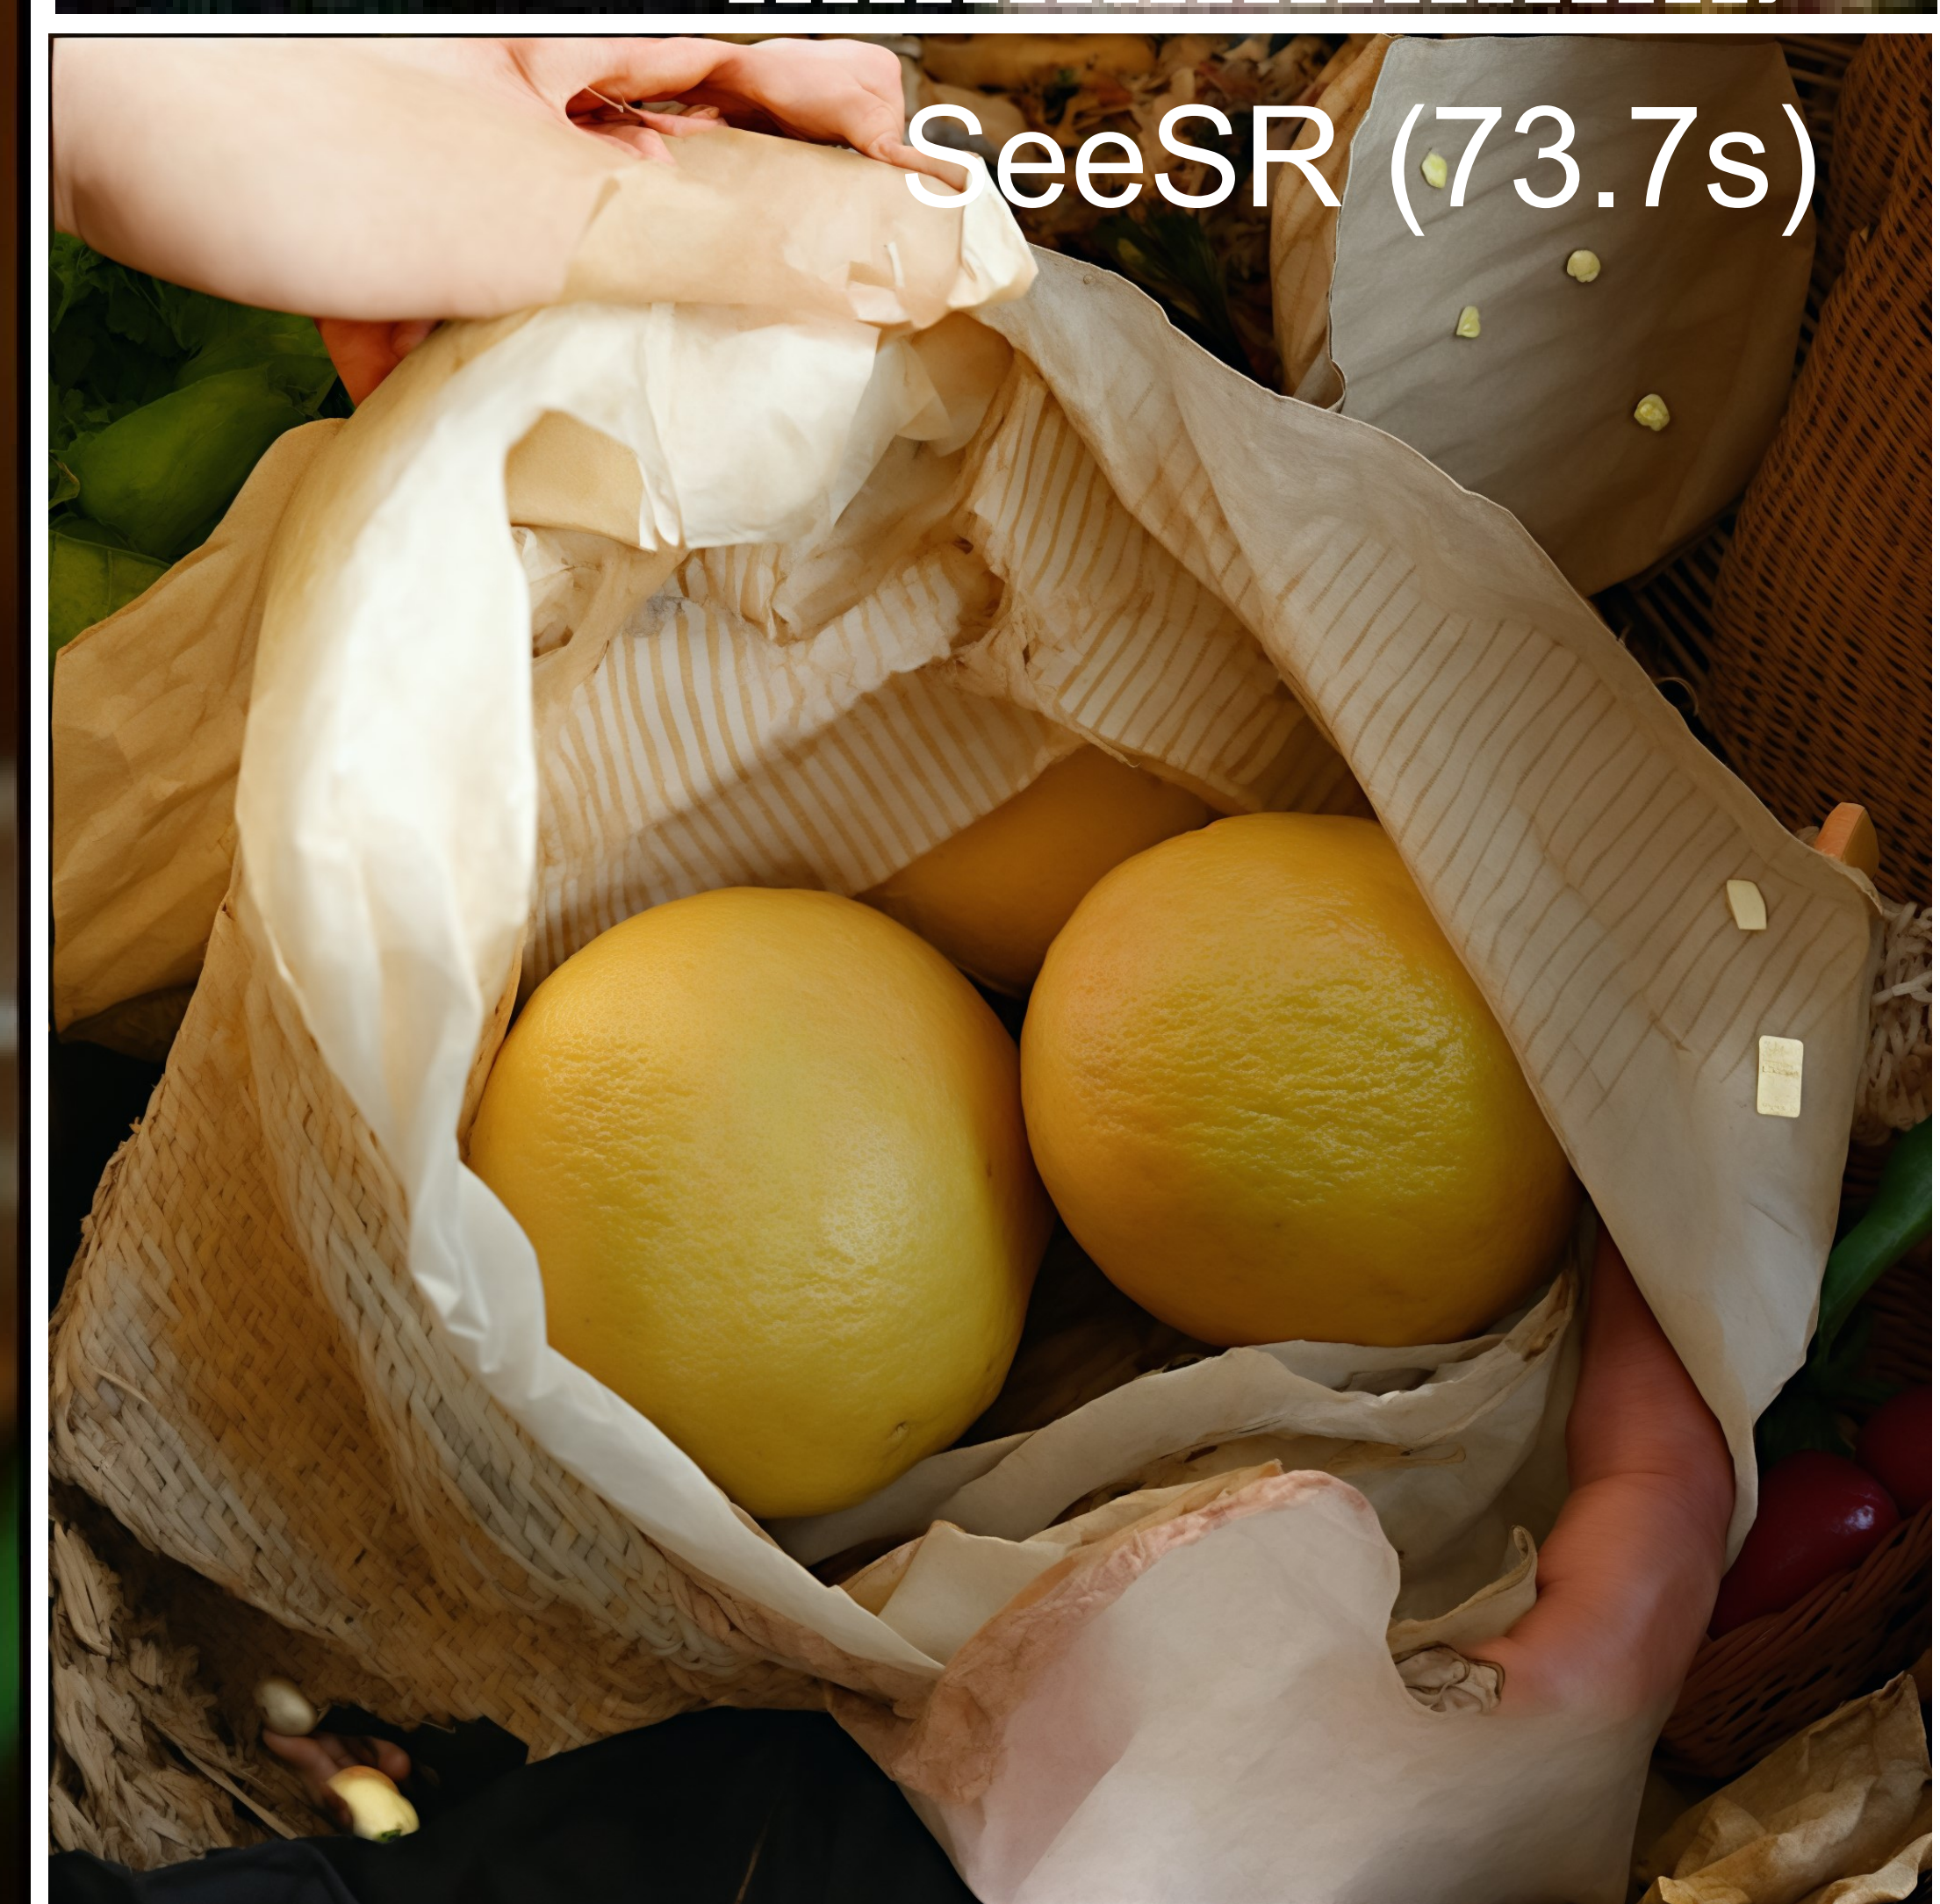

SeeSR (73.7s)

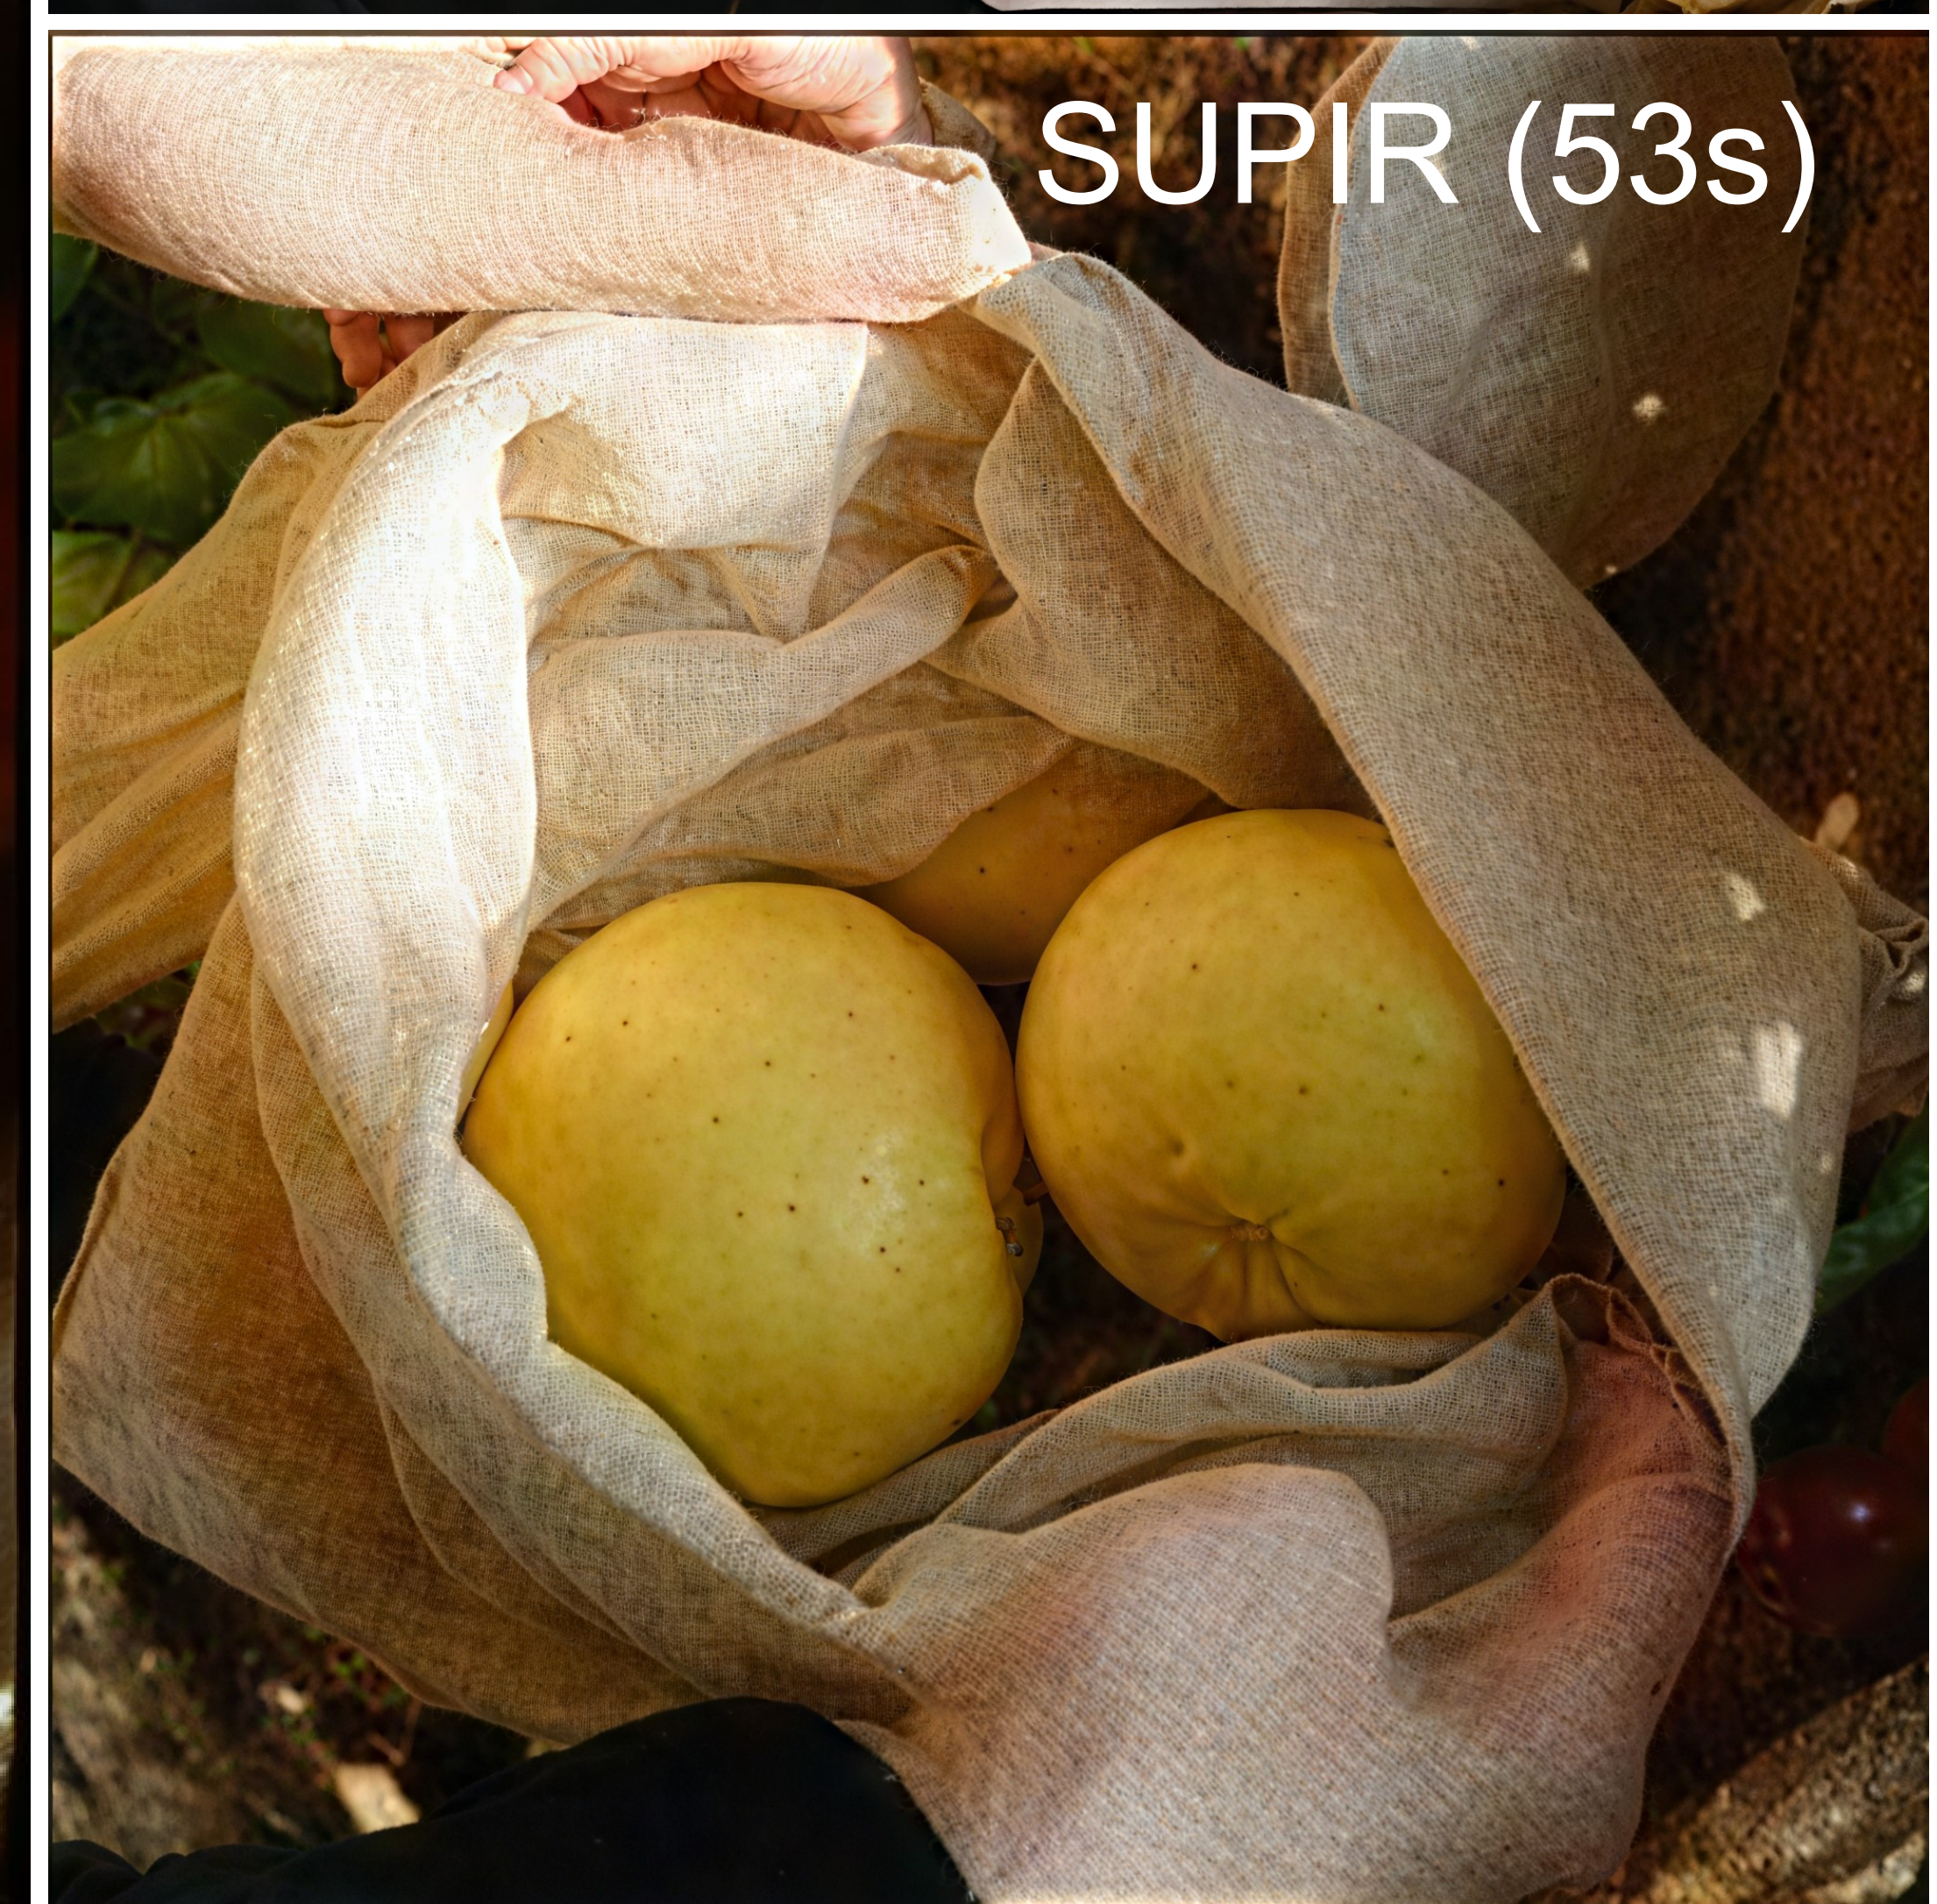

SUPIR (53s)

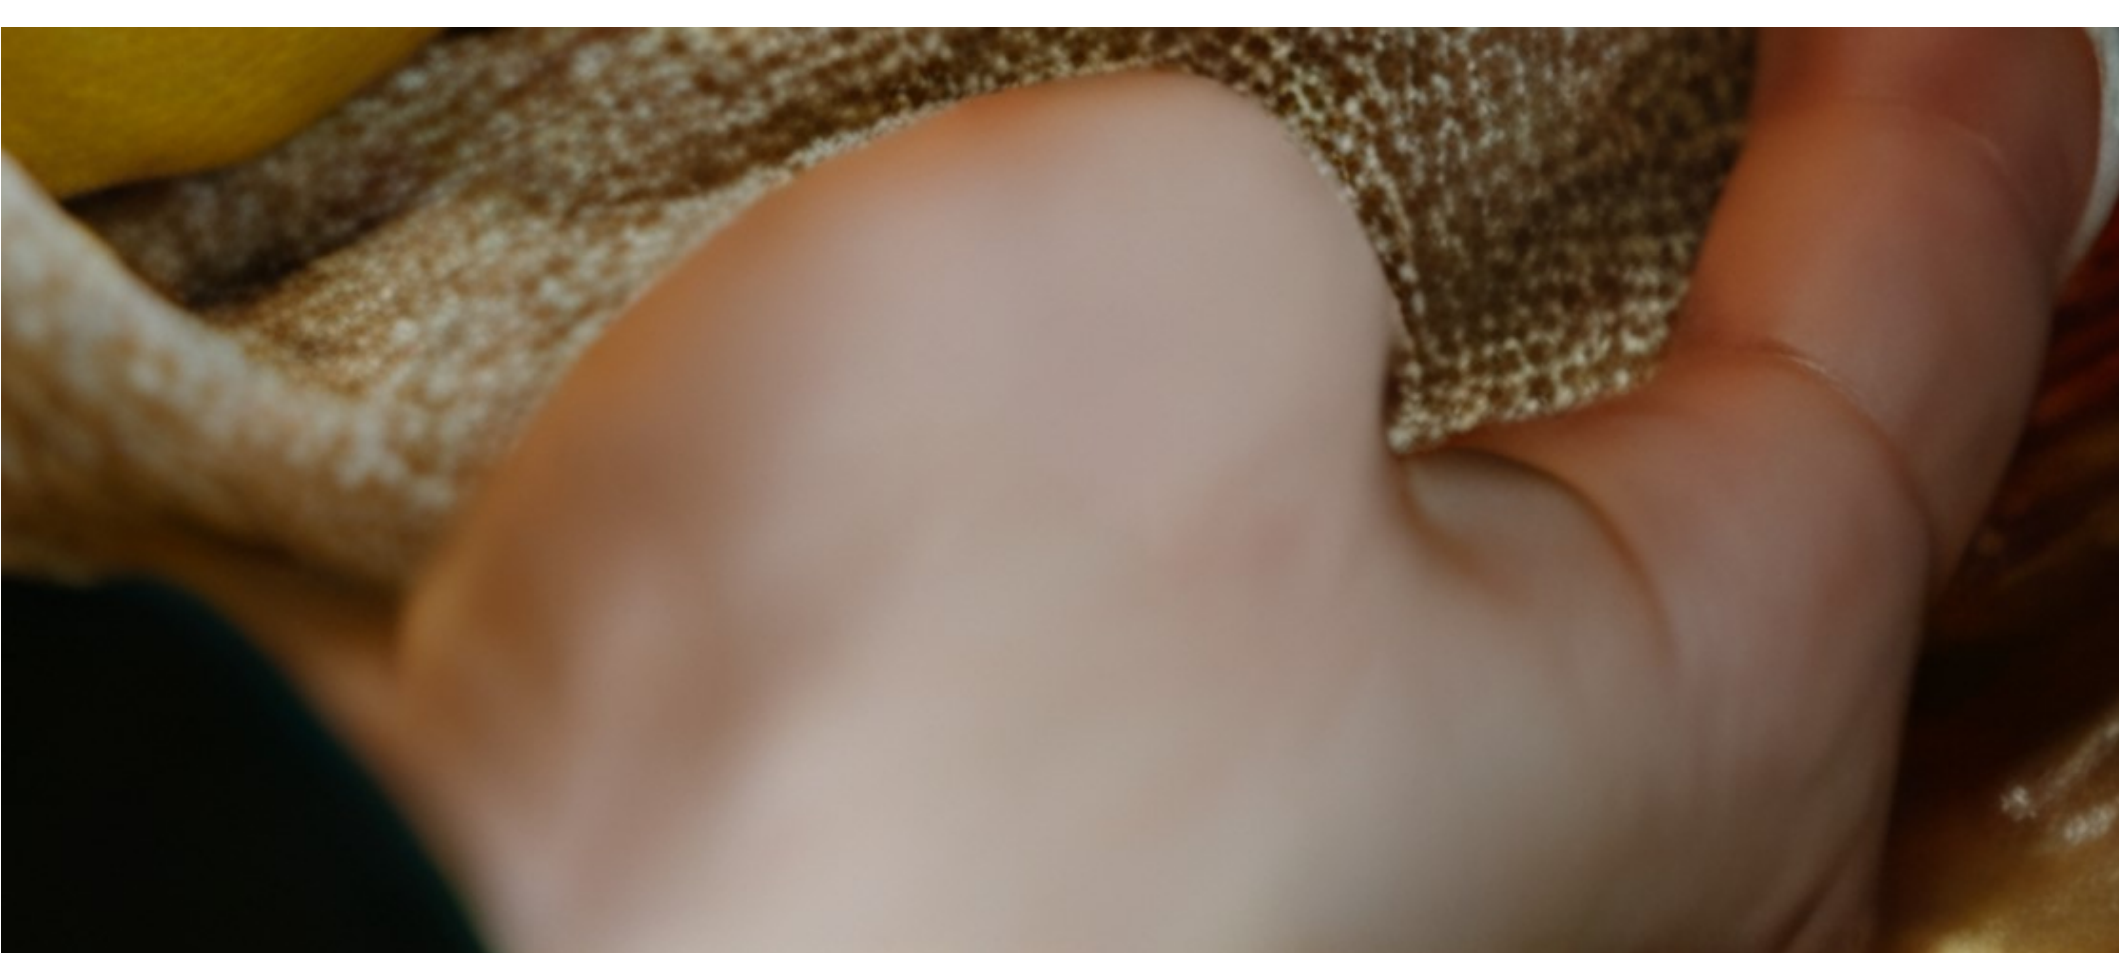

Ours

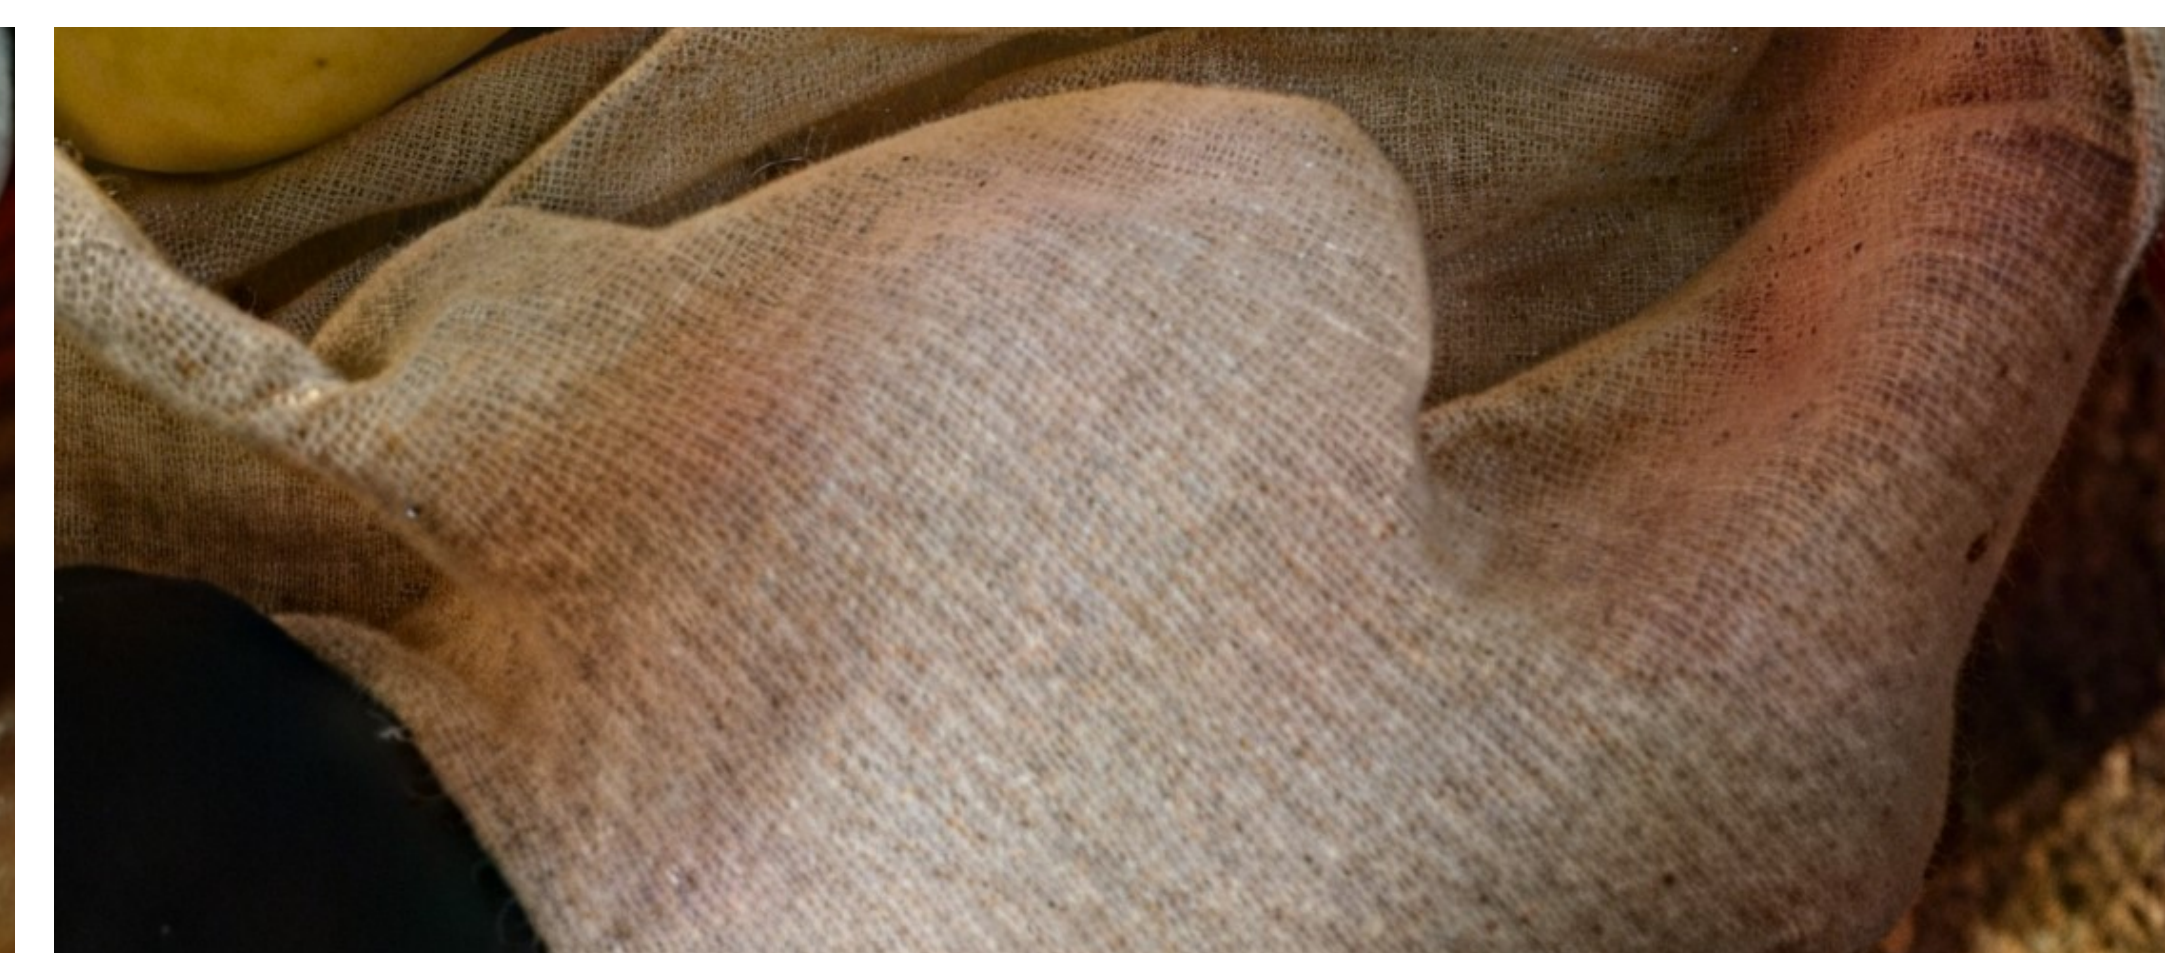

SUPIR

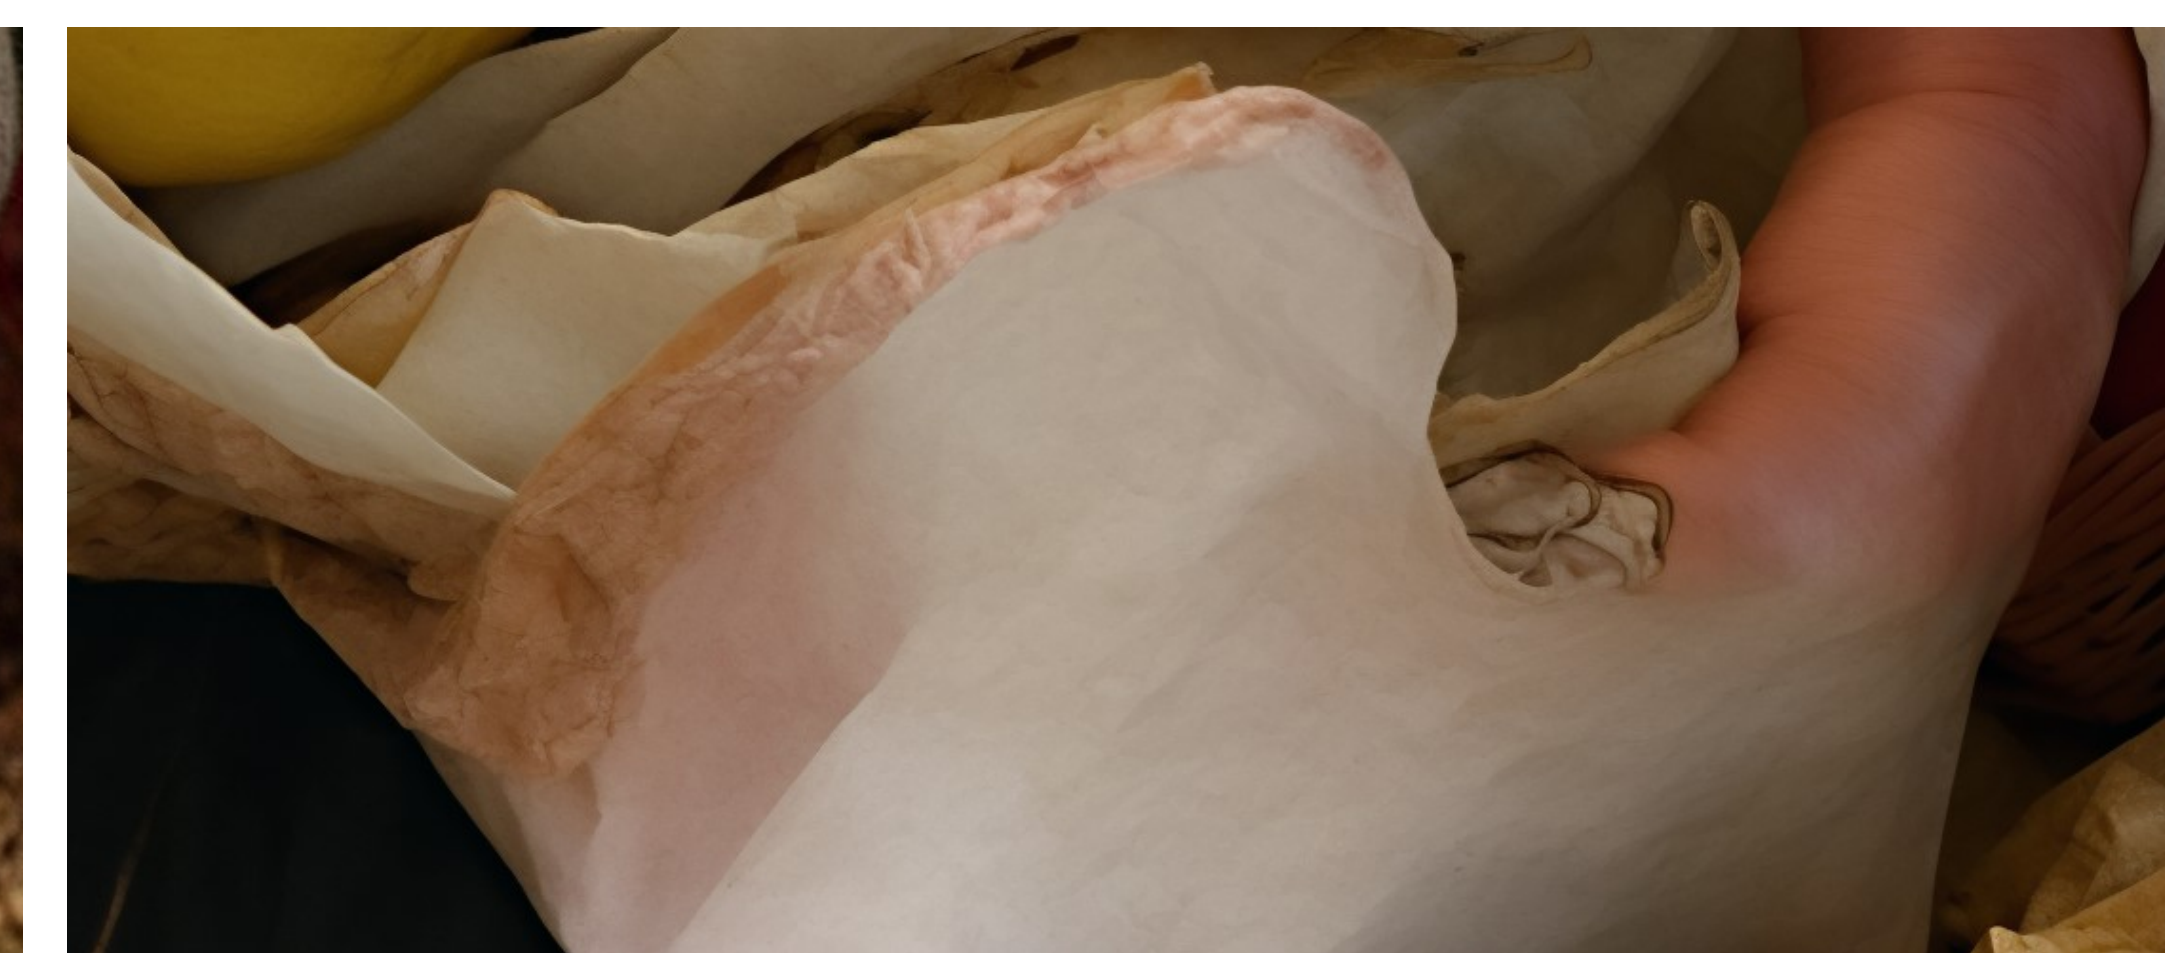

SeeSR

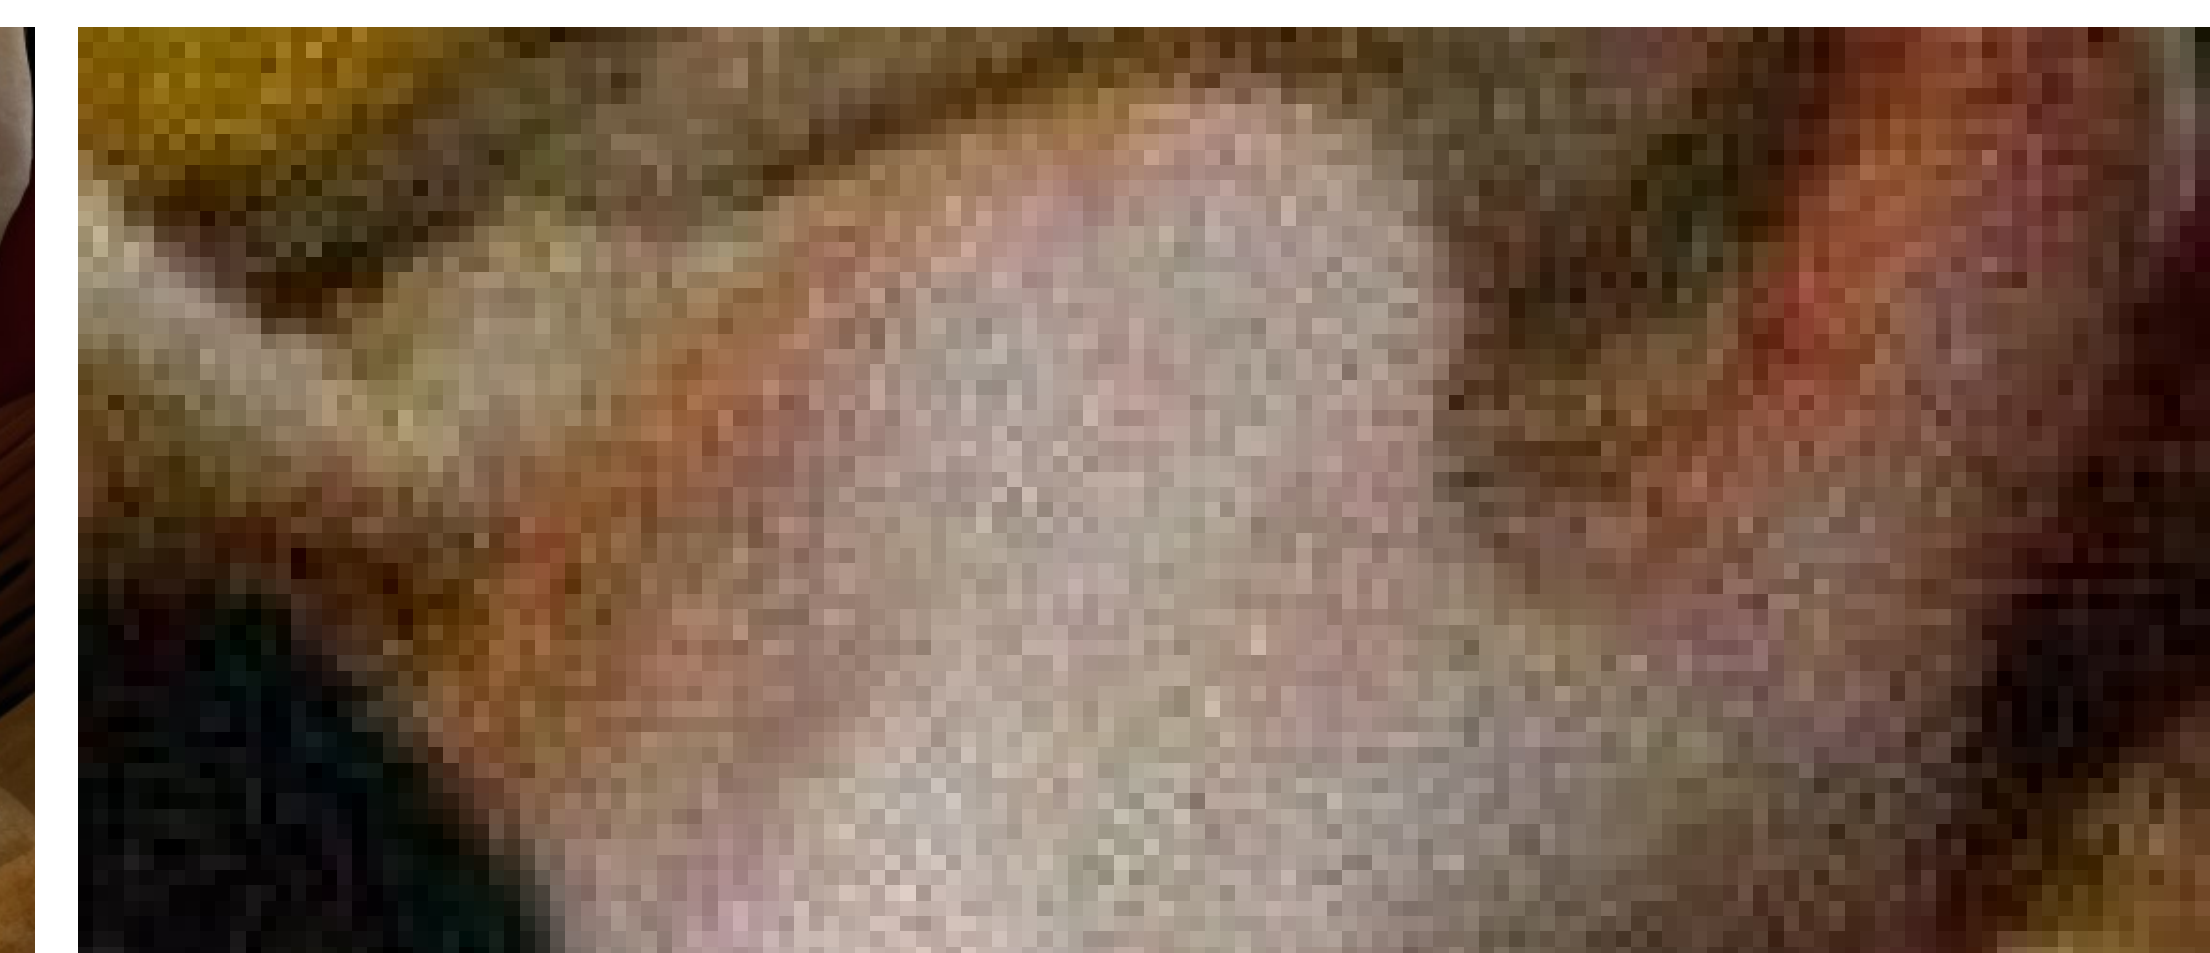

Input
