# Supplementary material for: ZipIR: Latent Pyramid Diffusion Transformer for High-Resolution Image Restoration
Source: arXiv:2504.08591 source file (2025-04-11)
Supplement: Supplementary file 4 [file ultrahigh-crop.pdf]

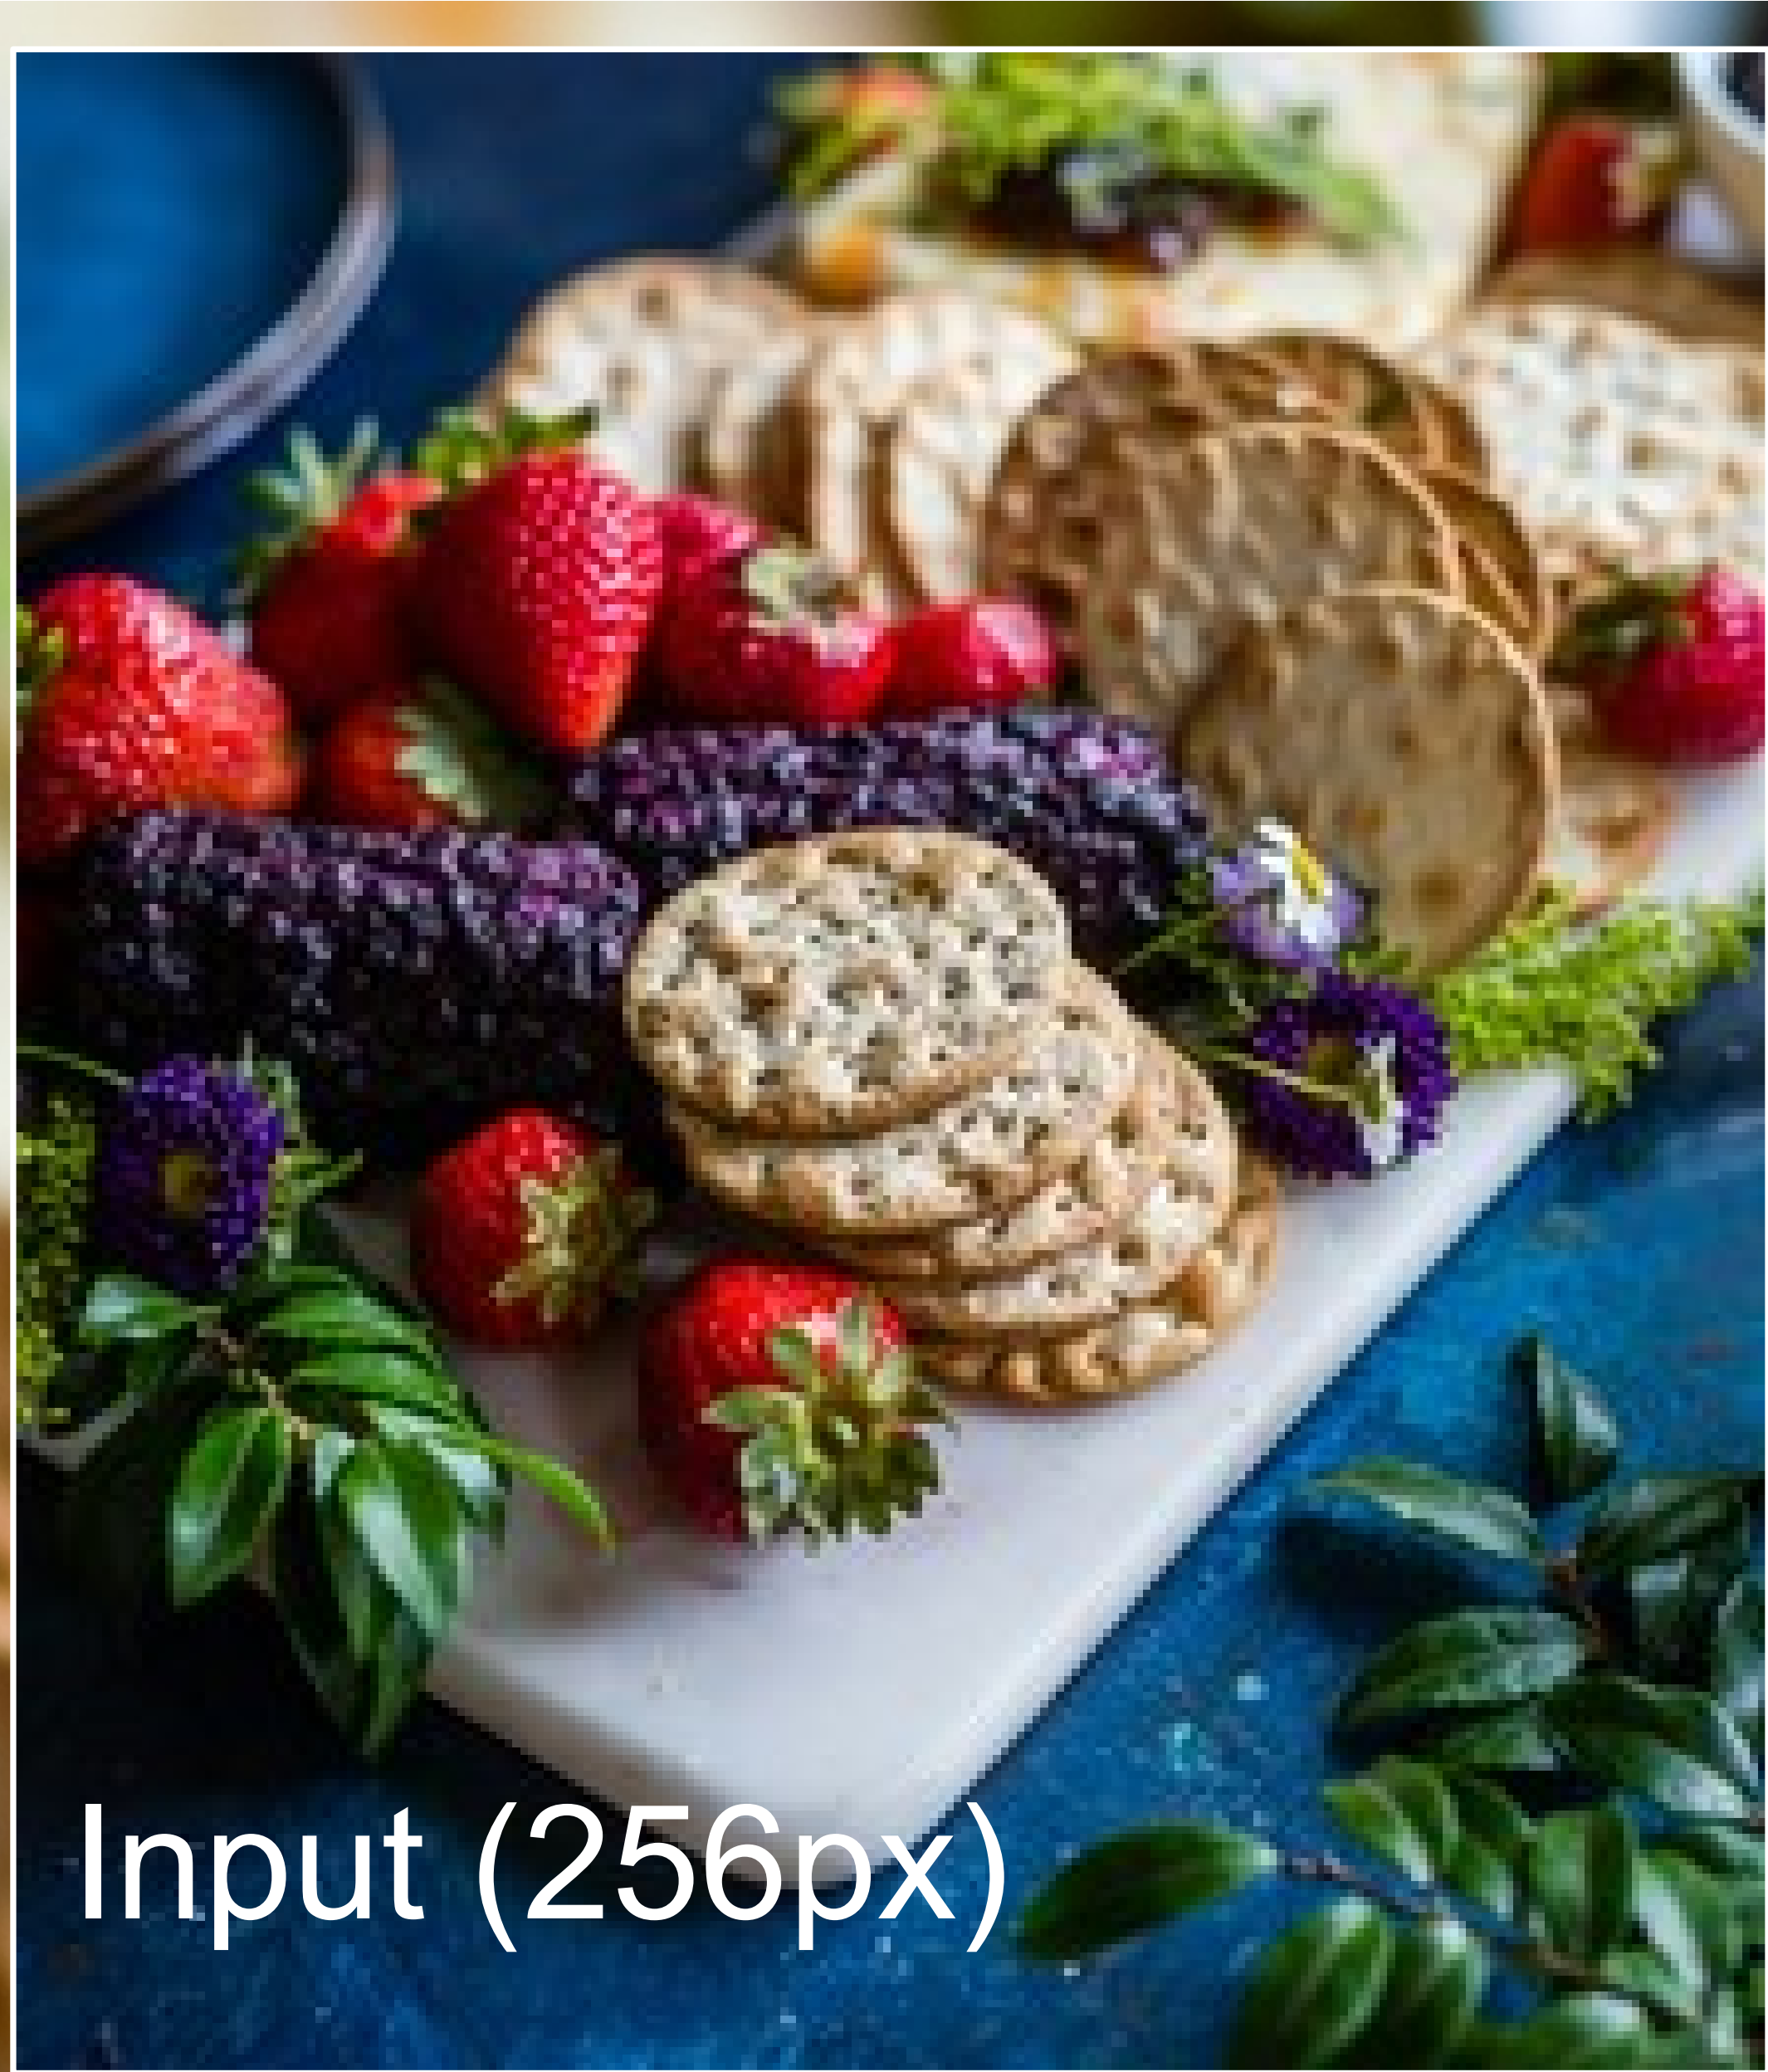

Input (256px)

ZipIR (Ours)

4096px, 16Mpix, 16× SR



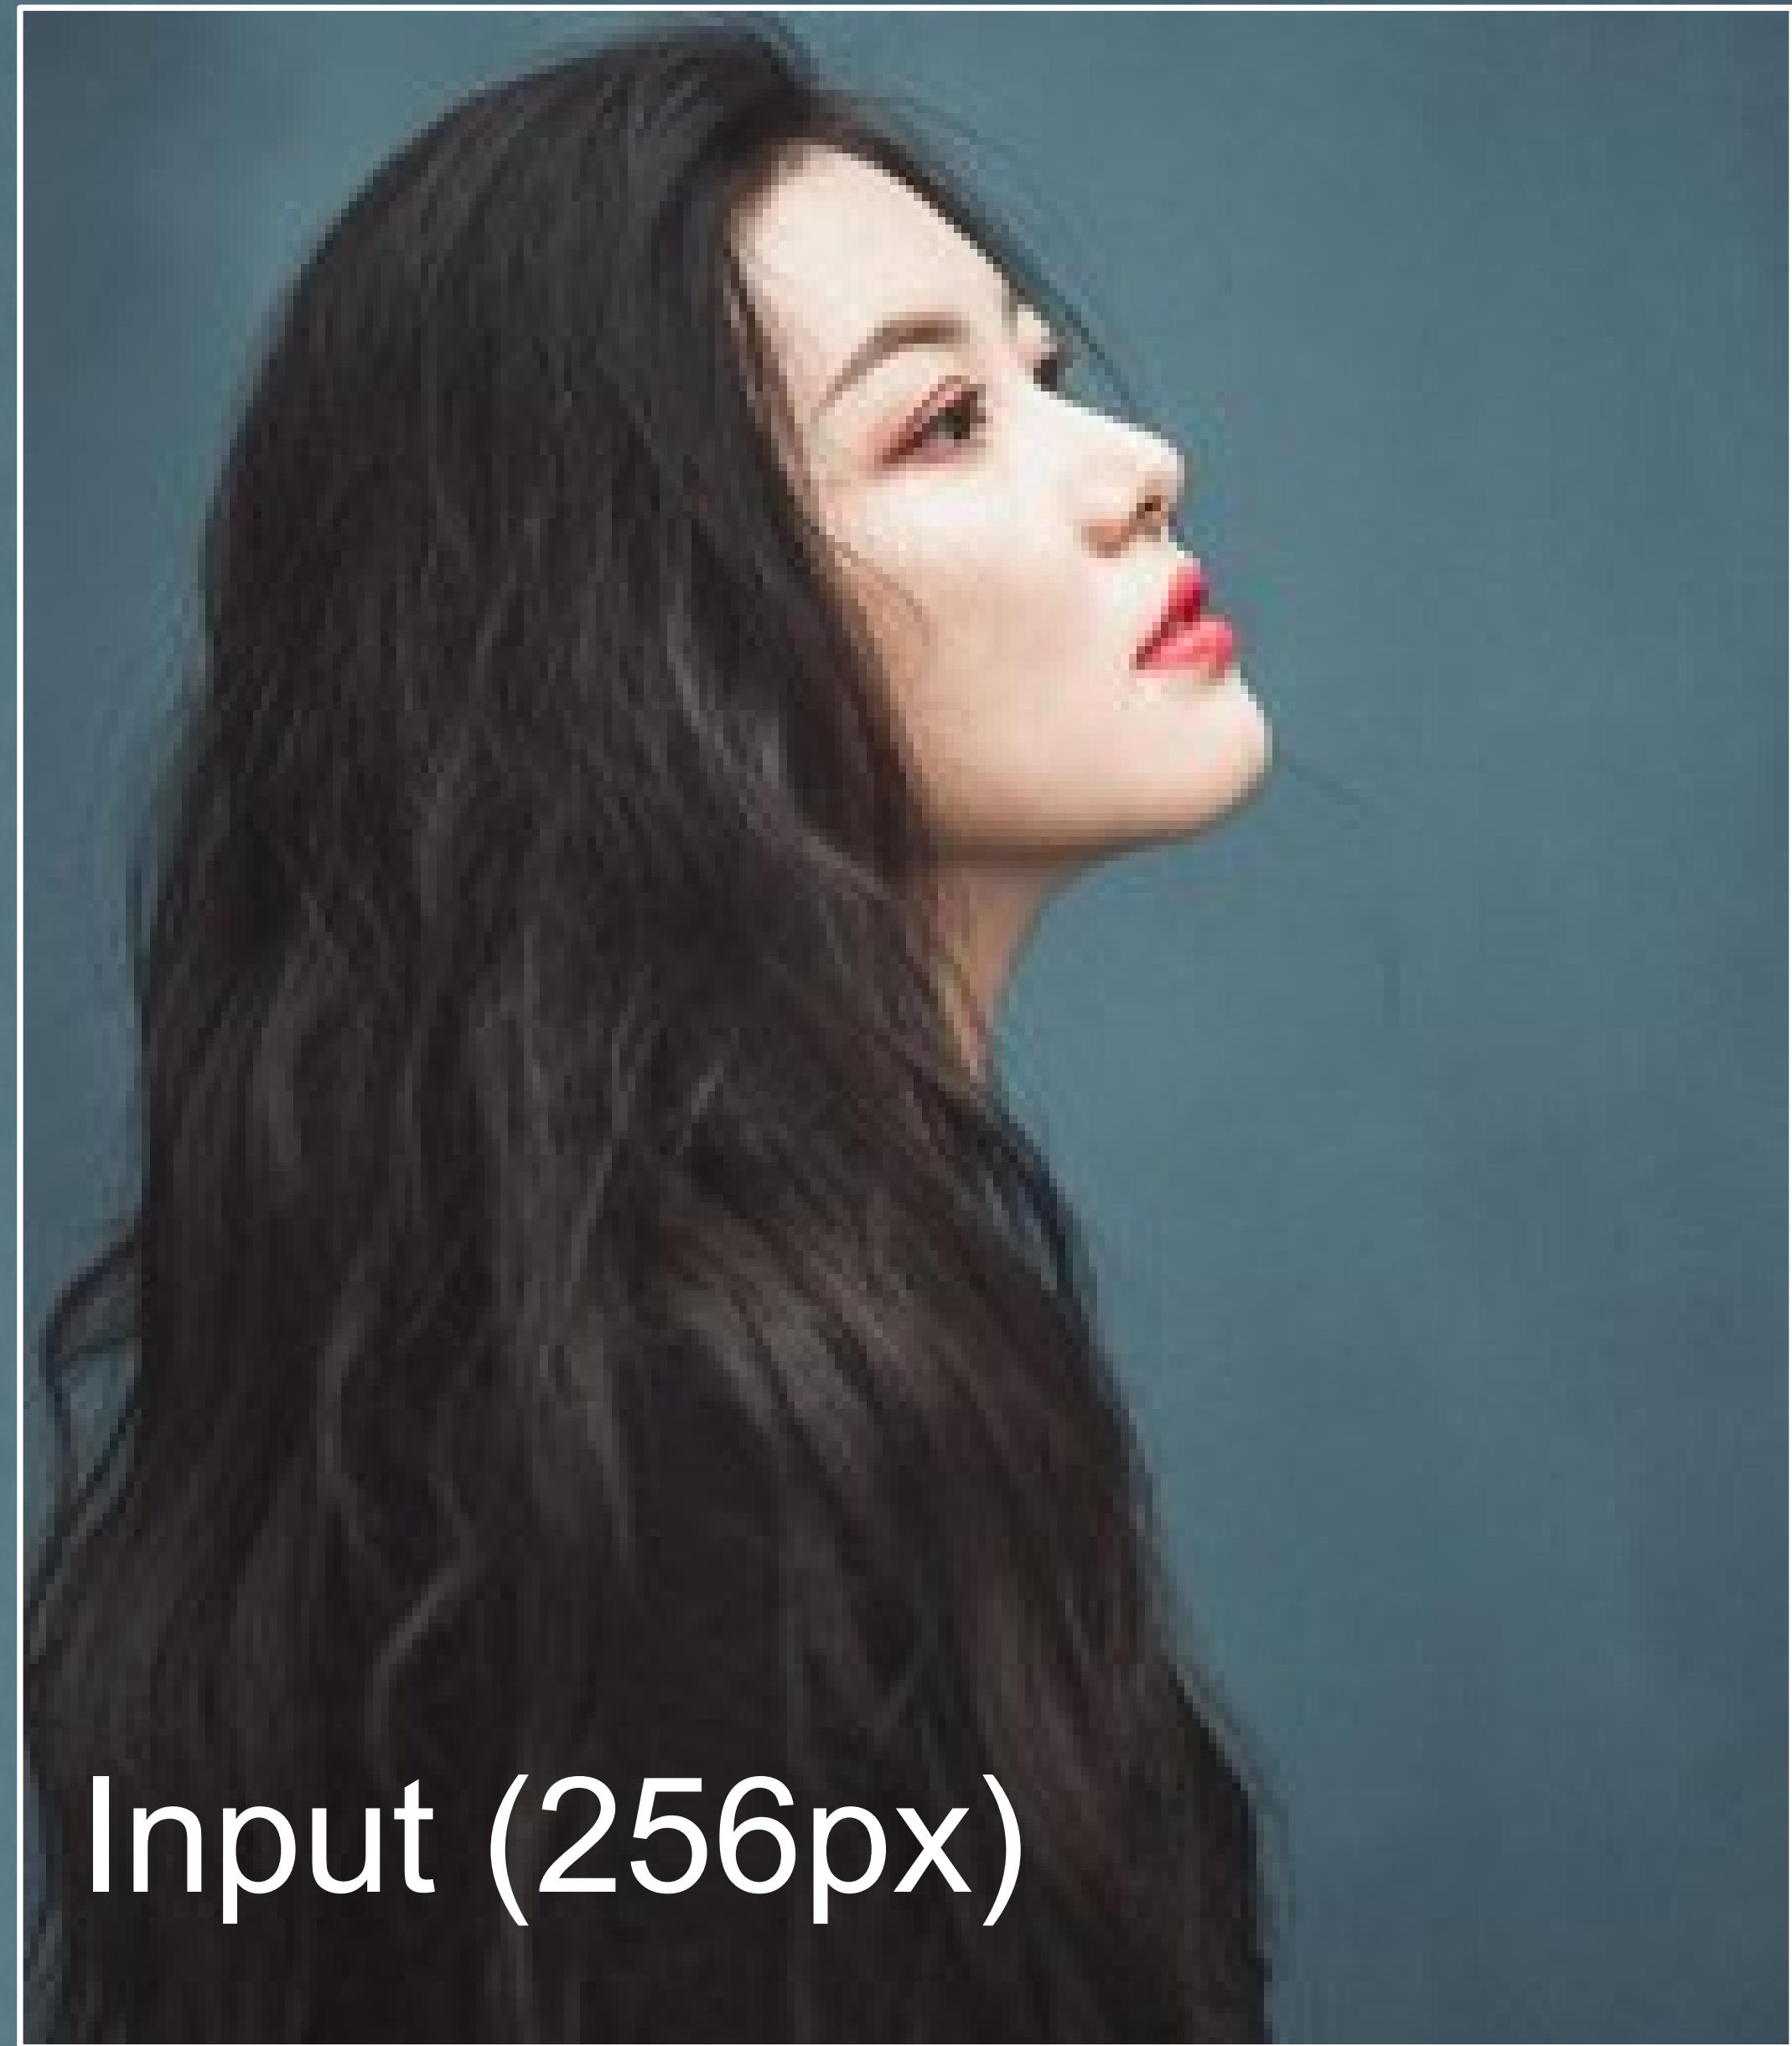

Input (256px)

ZipIR (Ours)

4096px, 16Mpix, 16× SR



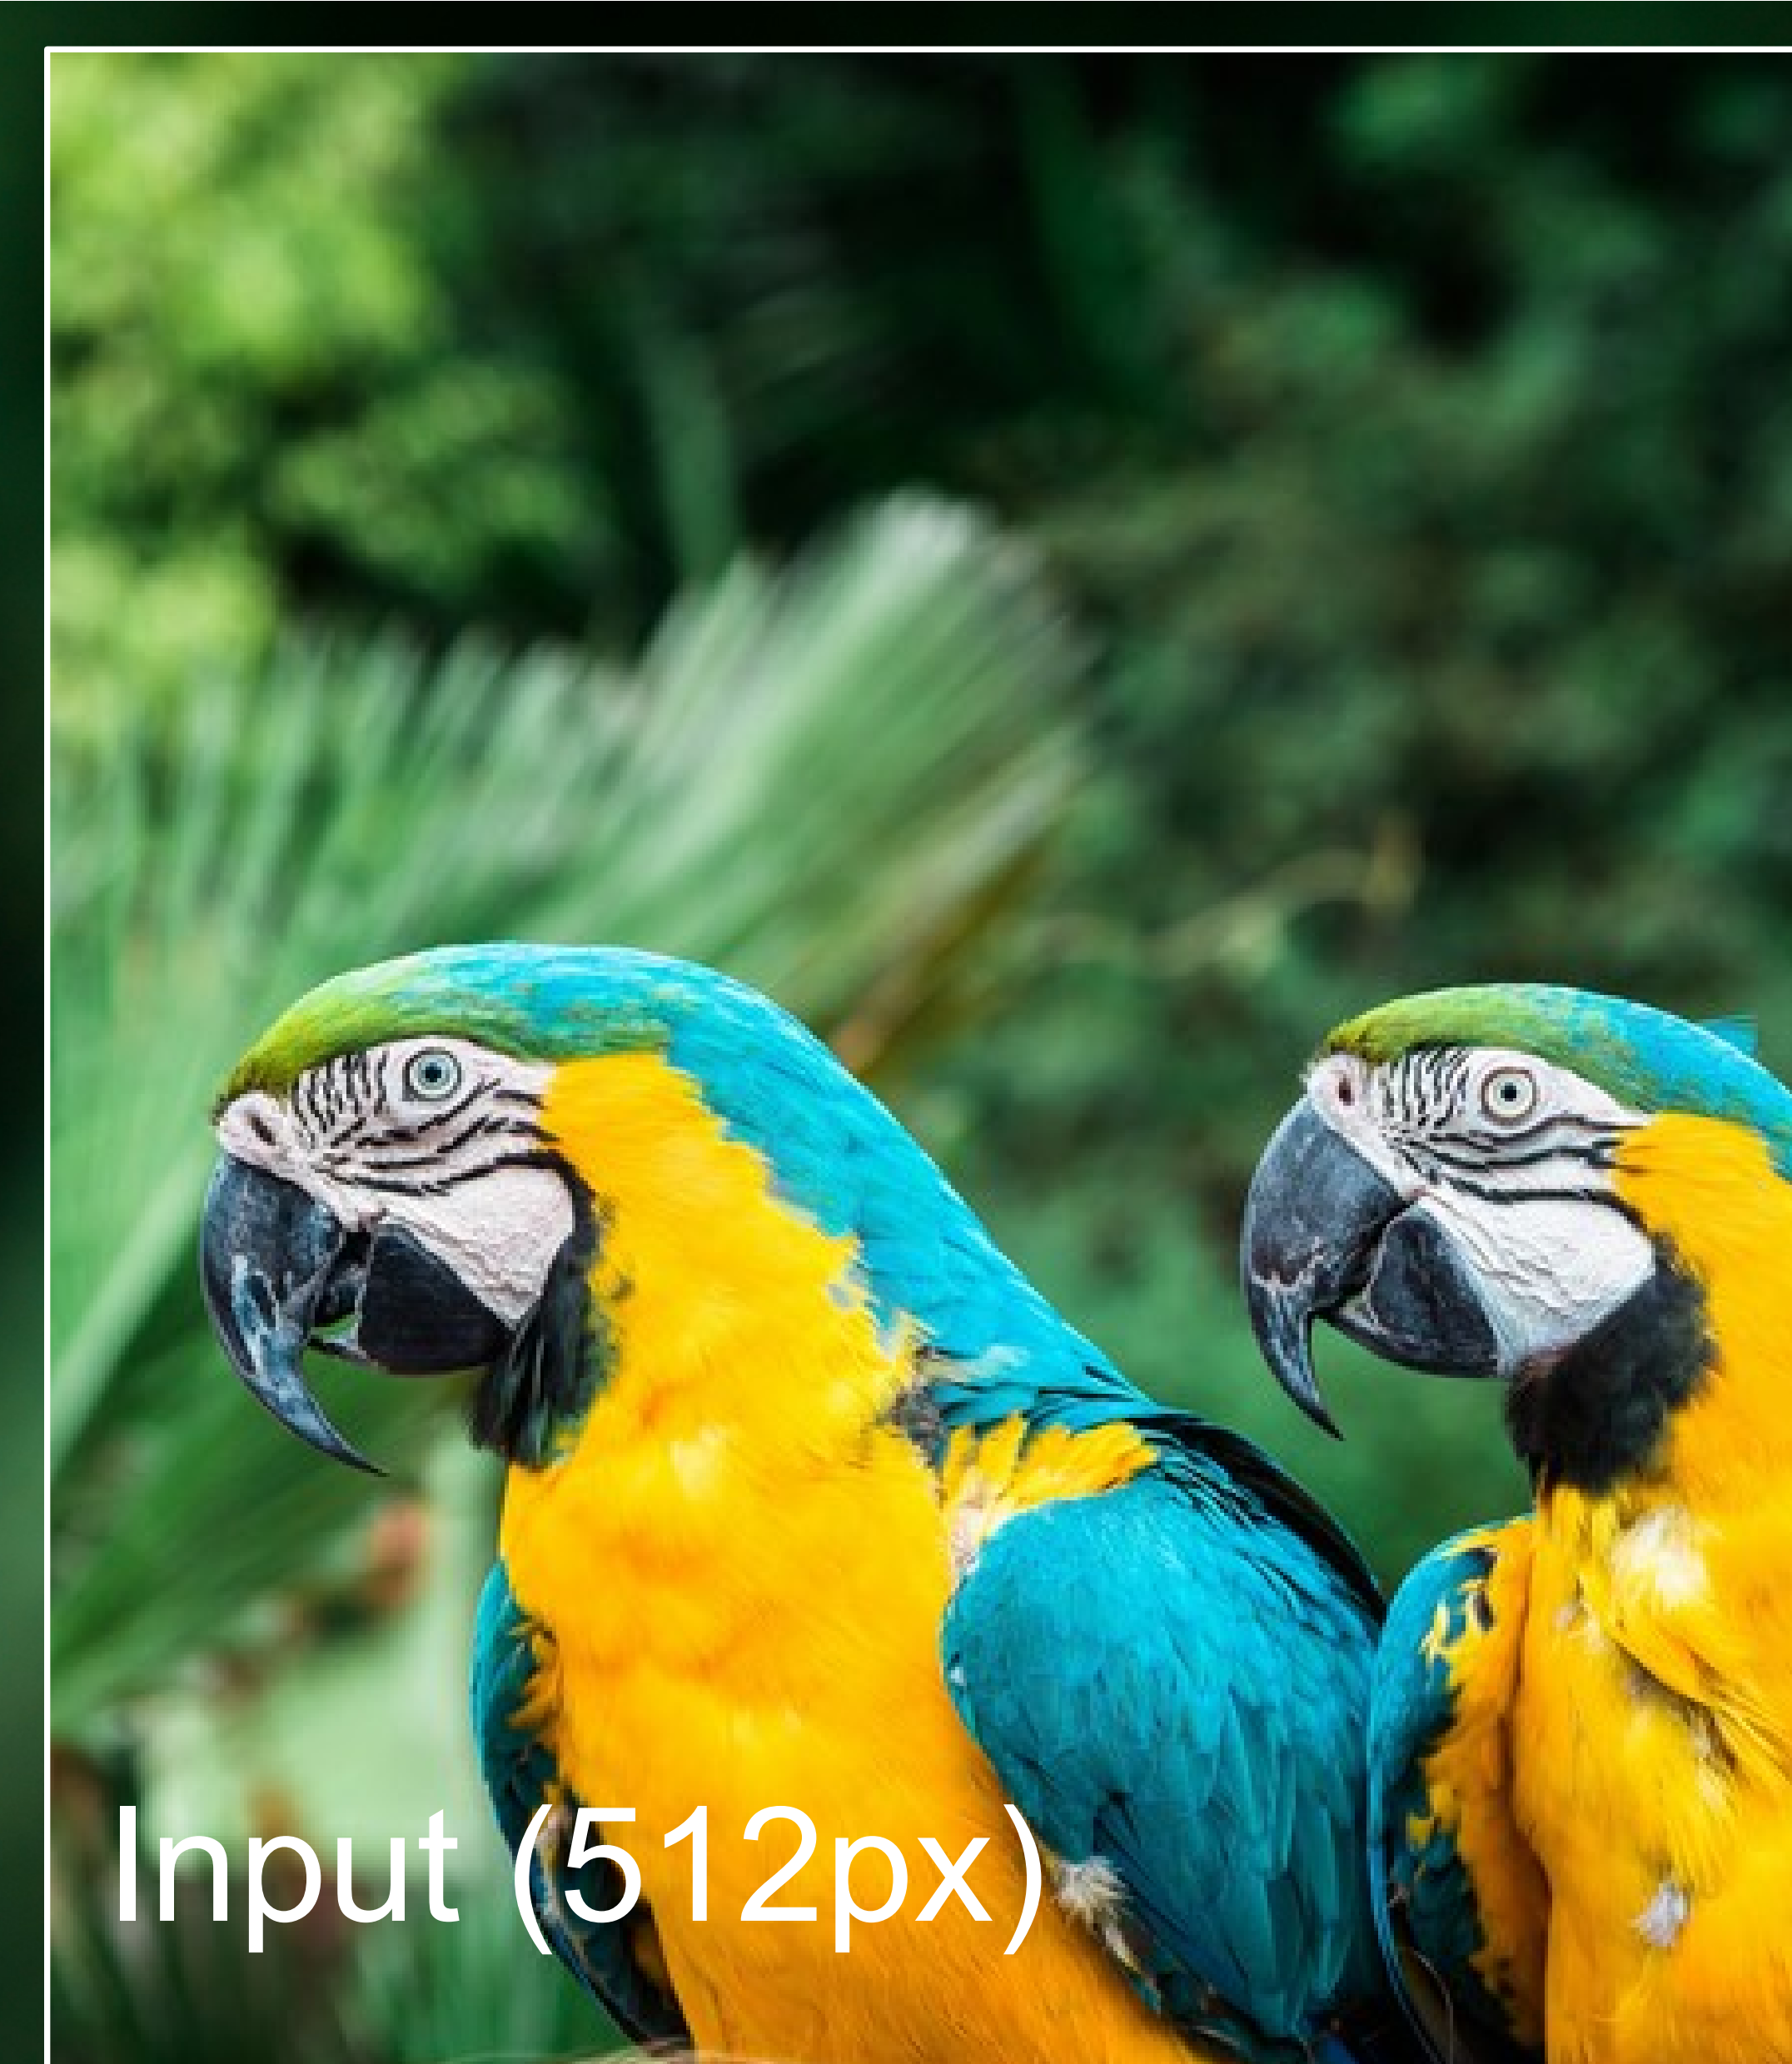

ZipIR (Ours)

8192px, 67Mpix, 16x SR
